# Supplementary material for: The Subarcsecond Mid-Infrared View of Local Active Galactic Nuclei. IV. The L- and M-band Imaging Atlas
Source: arXiv:2101.07006 source file (2021-04-14)
Supplement: Supplementary file 2 [file supplementaryv2.tex]

\documentclass[../submission2.tex]{subfiles}

\begin{document}

\begin{figure*}
\centering
\subfloat{\includegraphics[width=0.25\hsize]{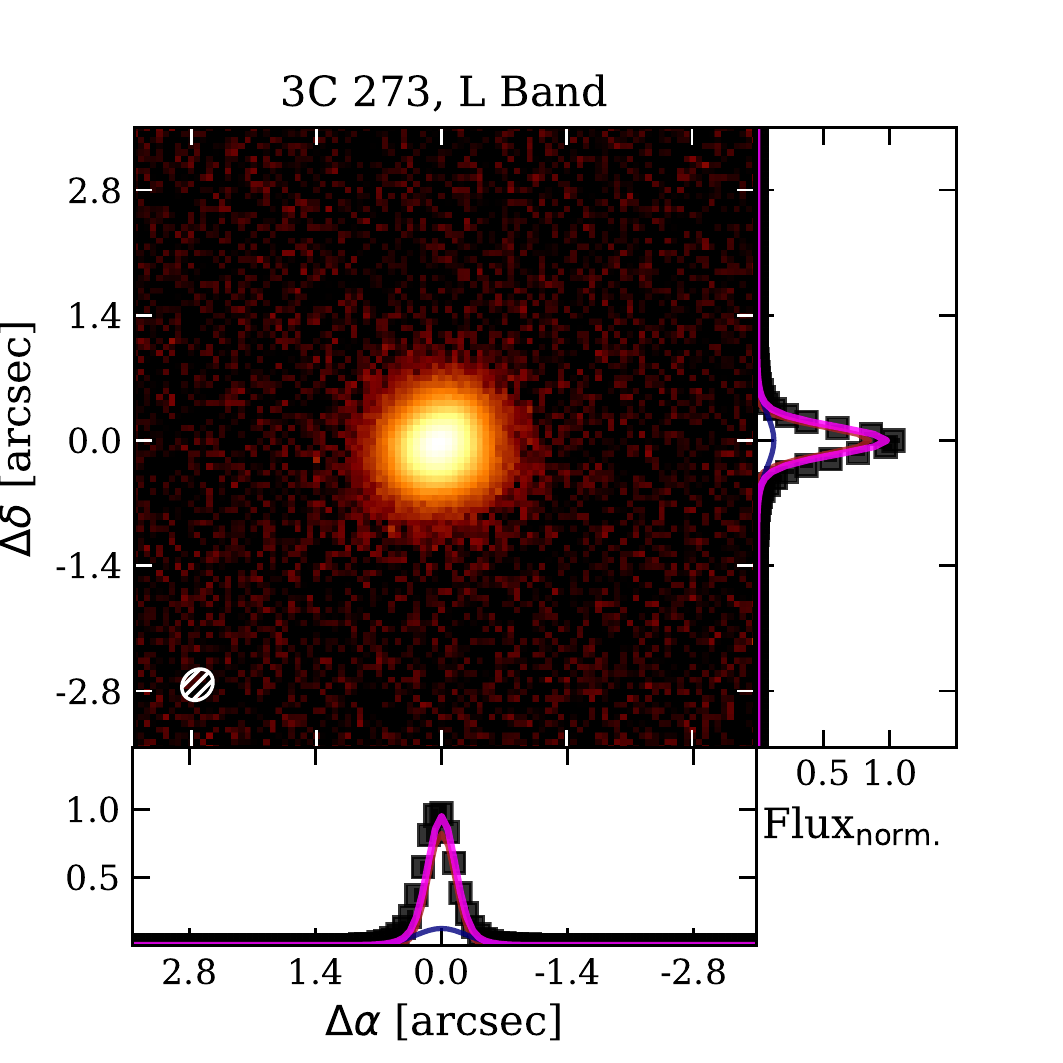}}
\subfloat{\includegraphics[width=0.25\hsize]{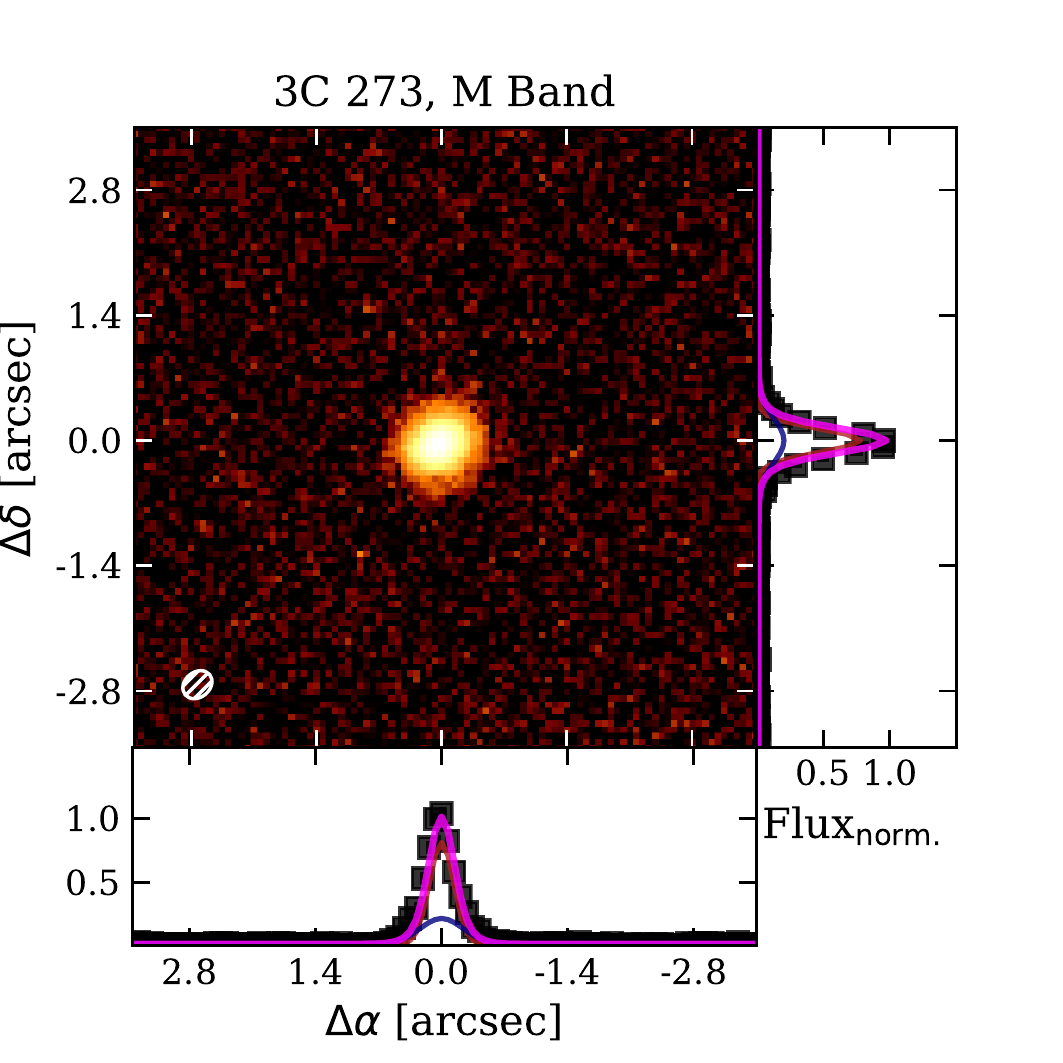}}
\subfloat{\includegraphics[width=0.25\hsize]{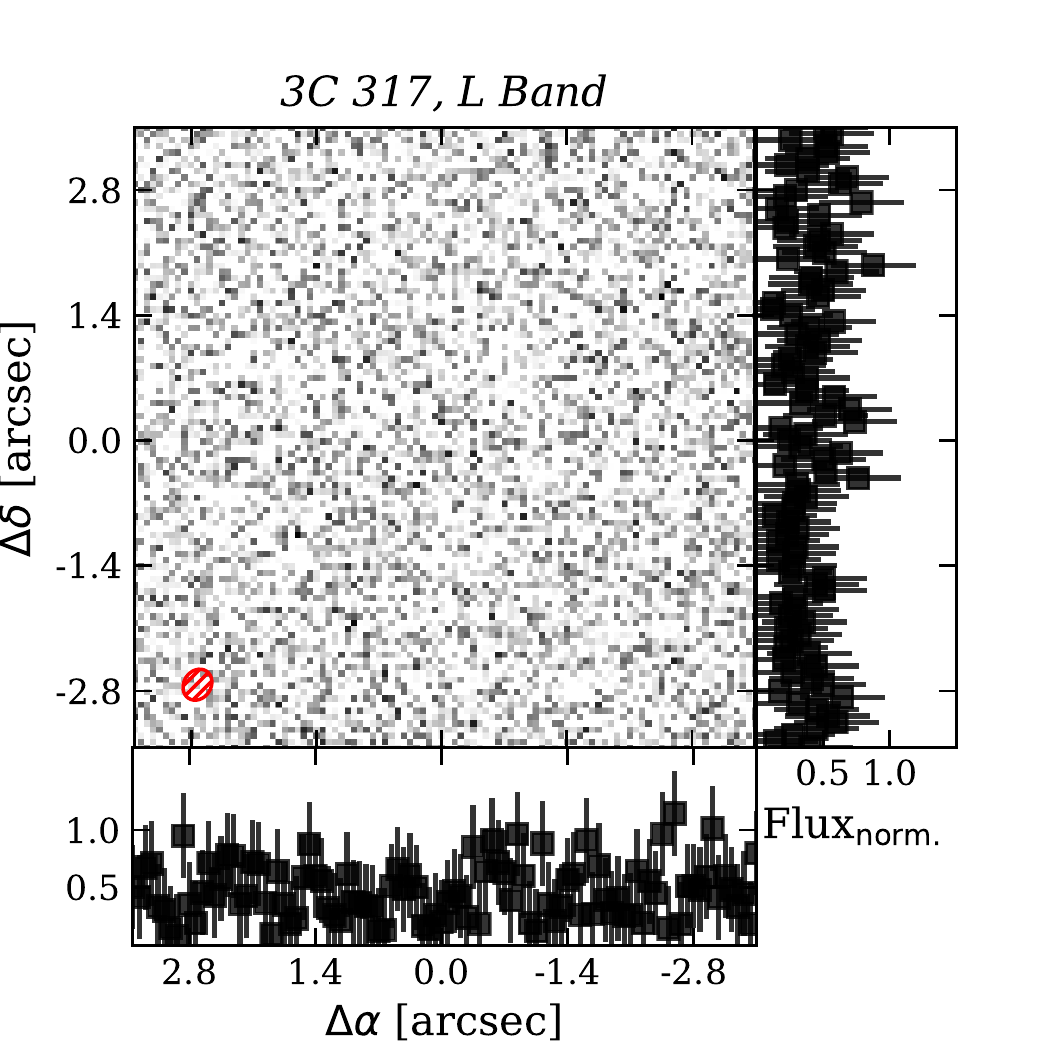}}
\subfloat{\includegraphics[width=0.25\hsize]{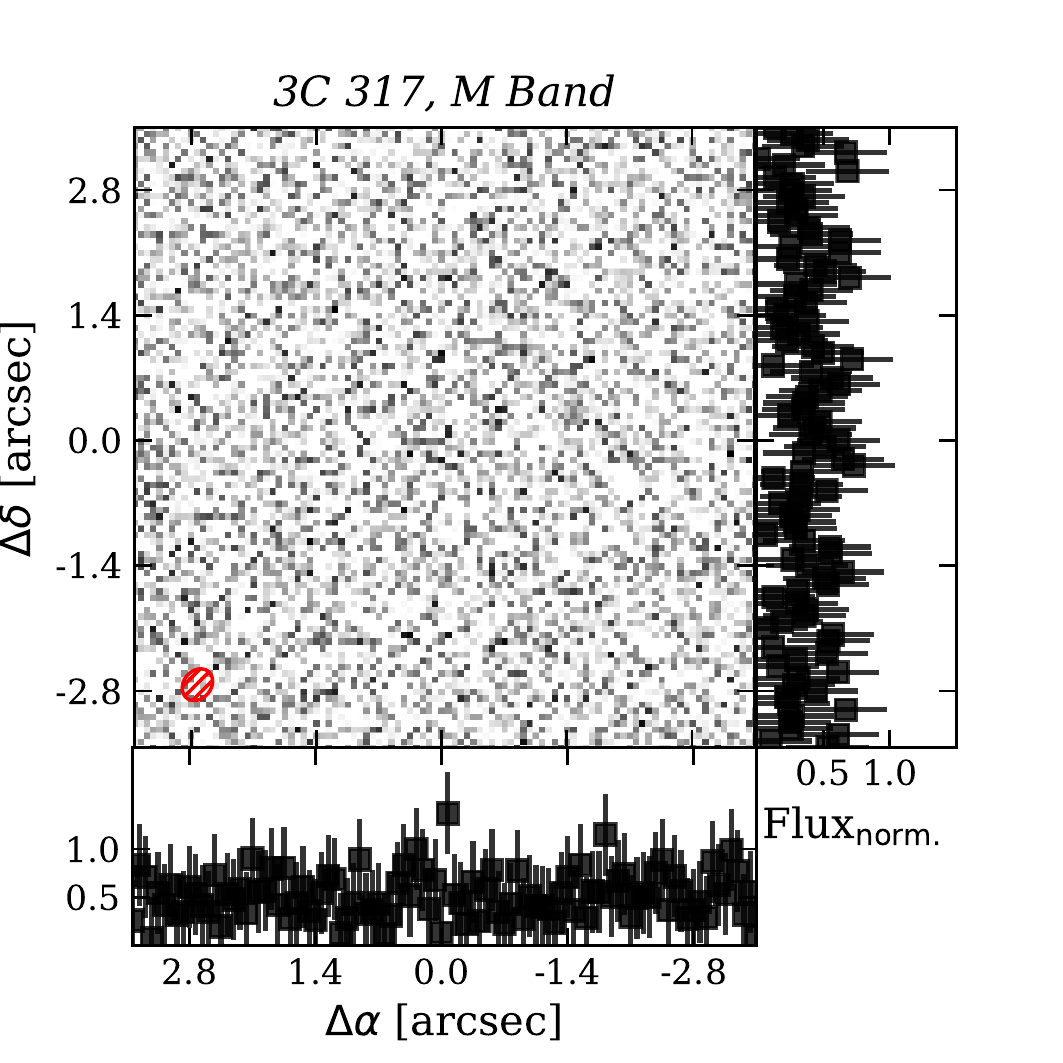}} \\
\subfloat{\includegraphics[width=0.25\hsize]{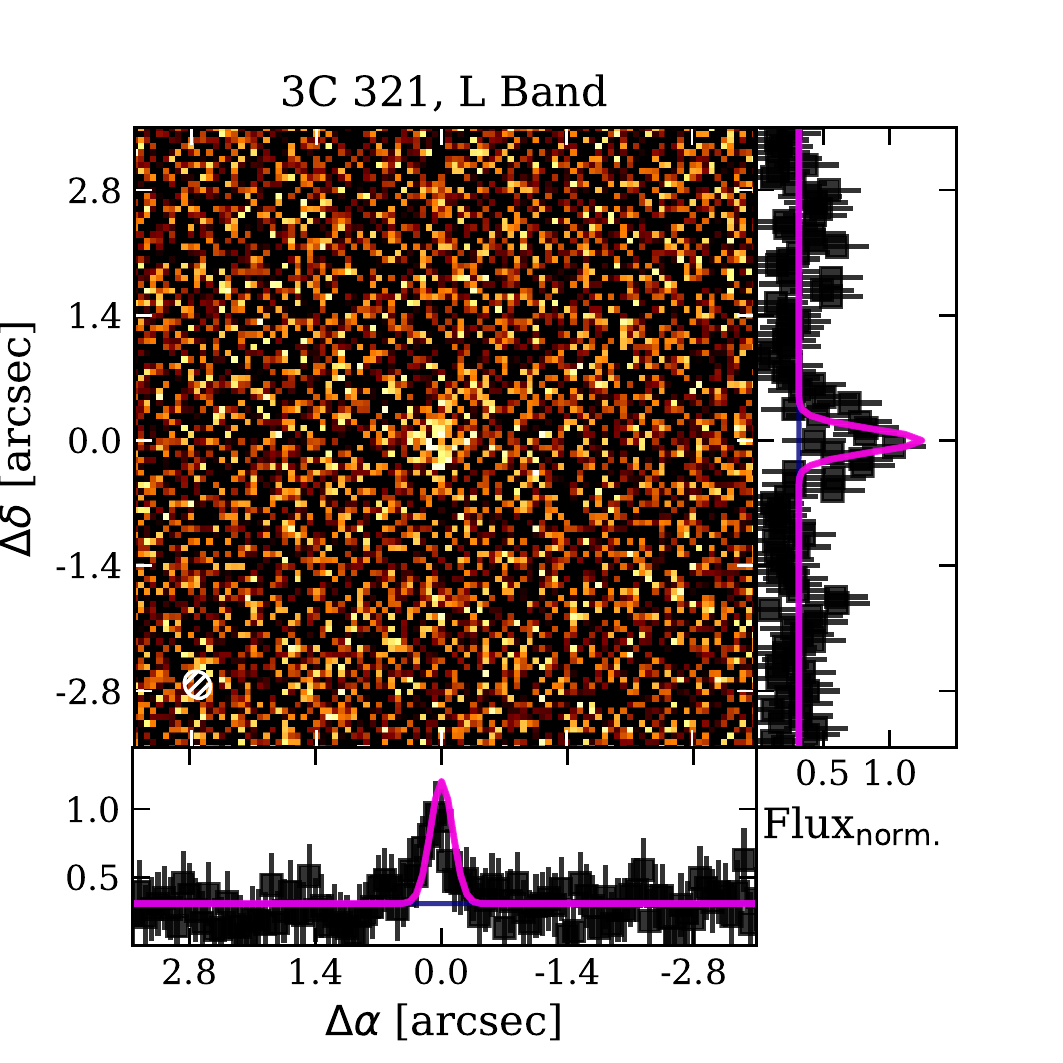}}
\subfloat{\includegraphics[width=0.25\hsize]{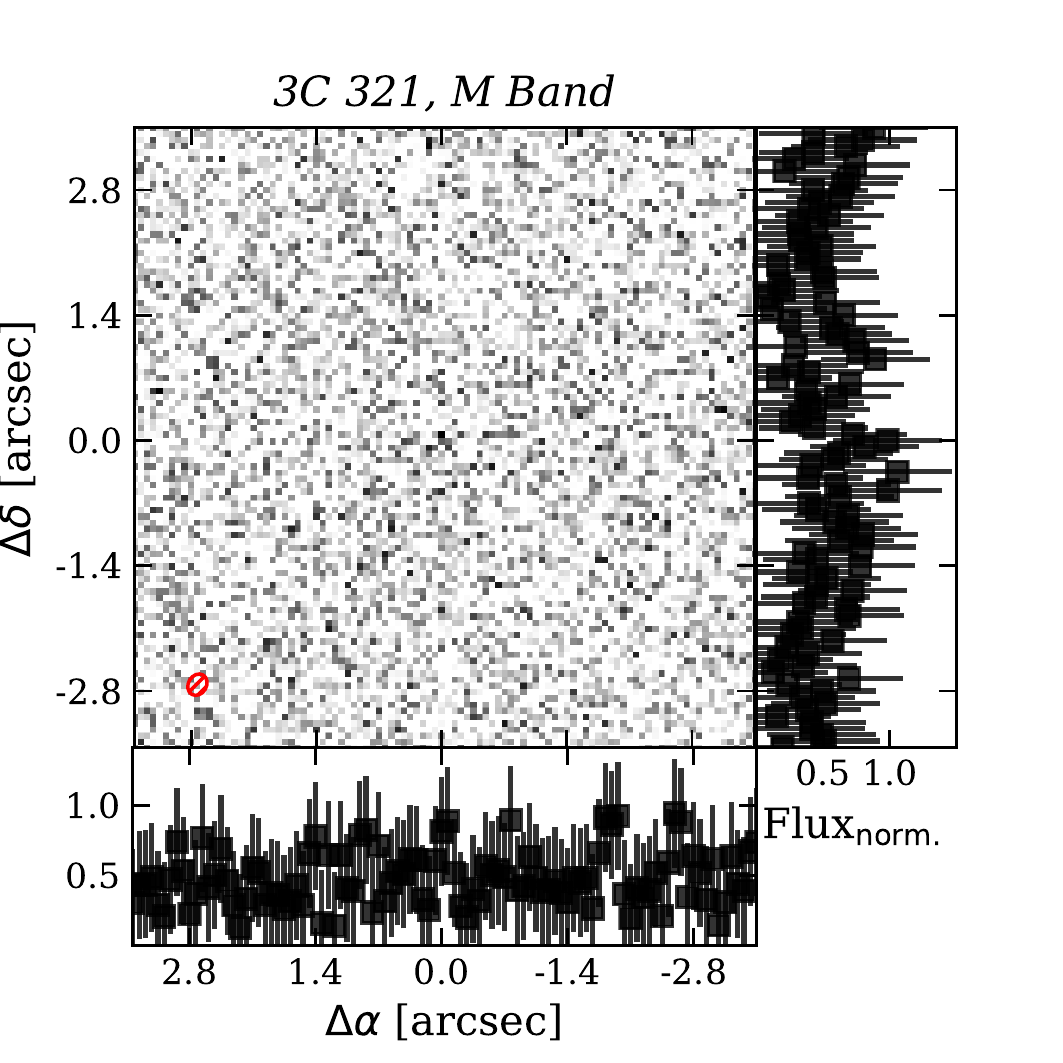}}
\subfloat{\includegraphics[width=0.25\hsize]{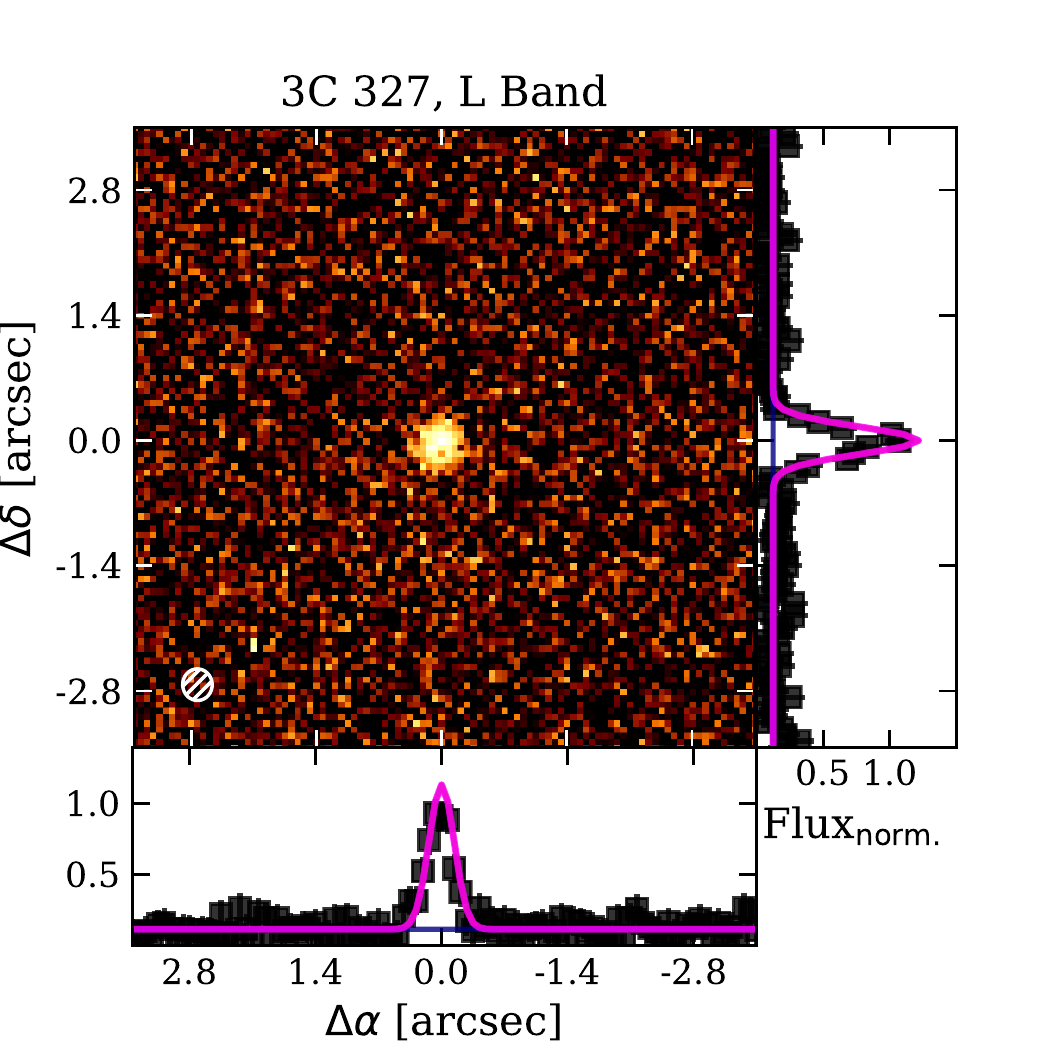}}
\subfloat{\includegraphics[width=0.25\hsize]{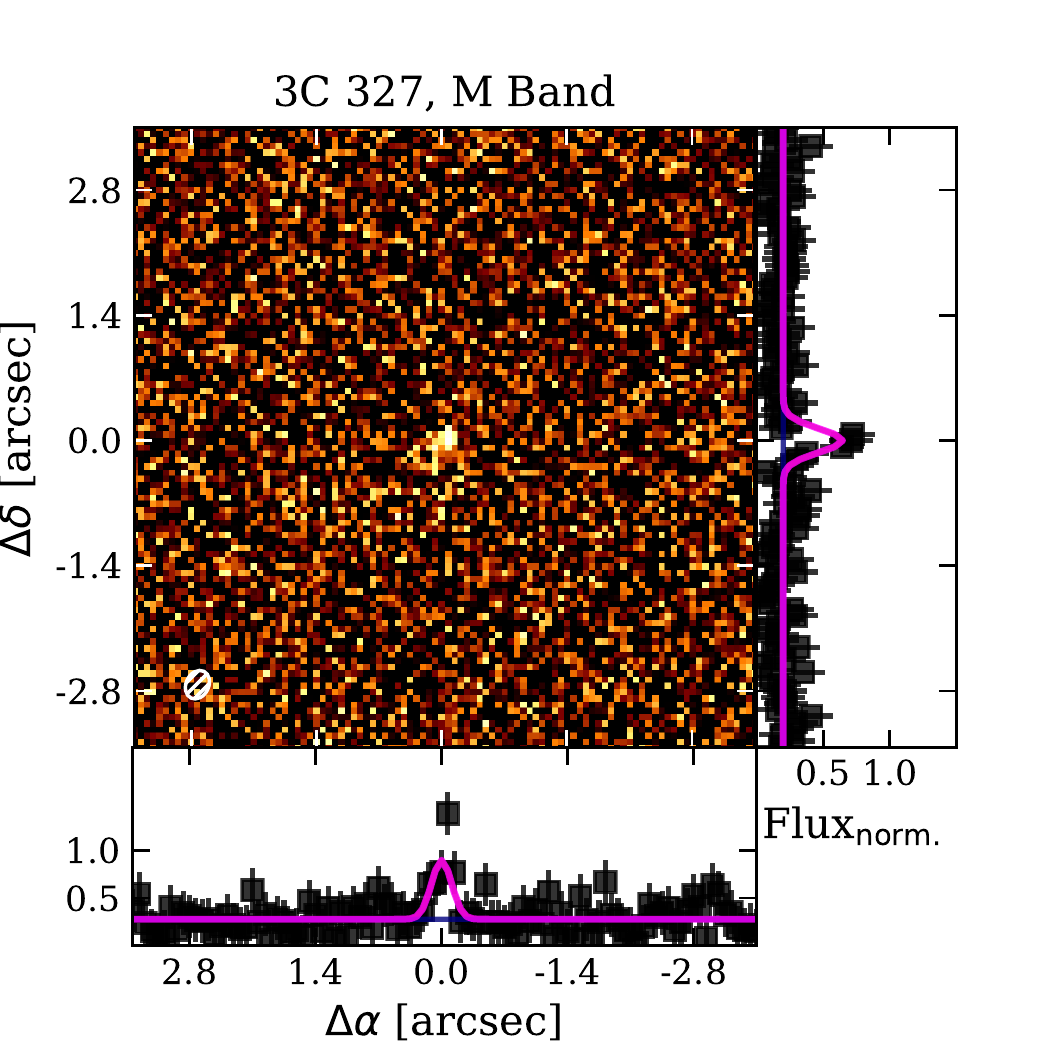}} \\
\subfloat{\includegraphics[width=0.25\hsize]{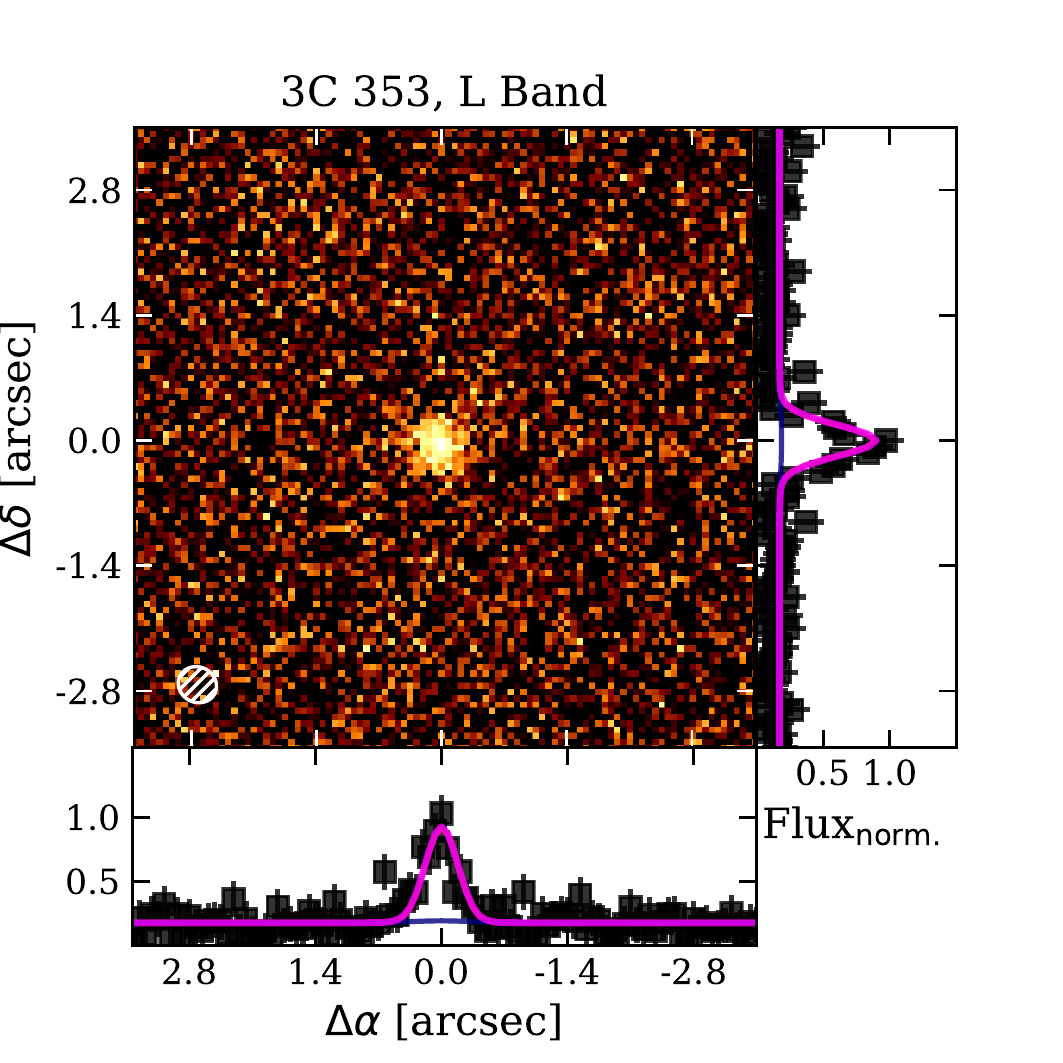}}
\subfloat{\includegraphics[width=0.25\hsize]{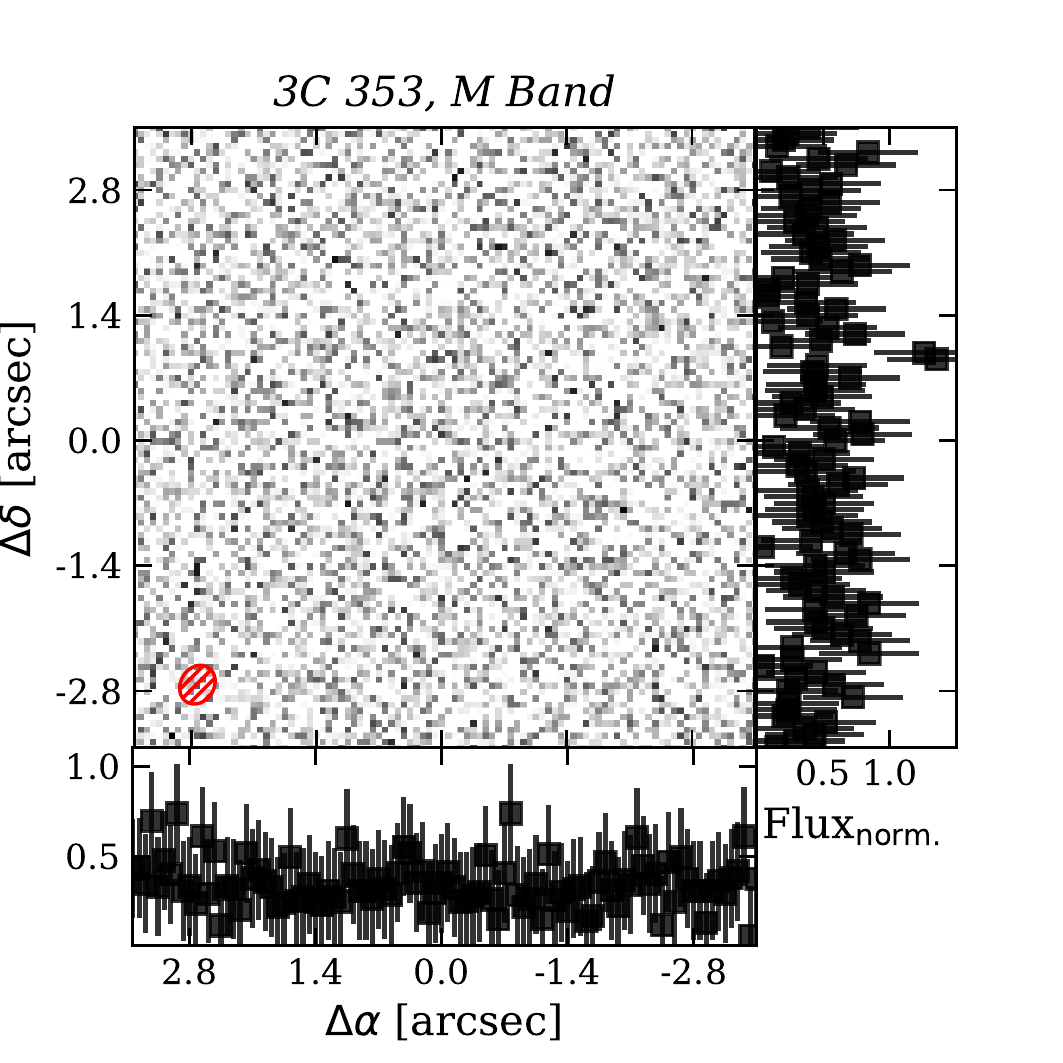}}
\subfloat{\includegraphics[width=0.25\hsize]{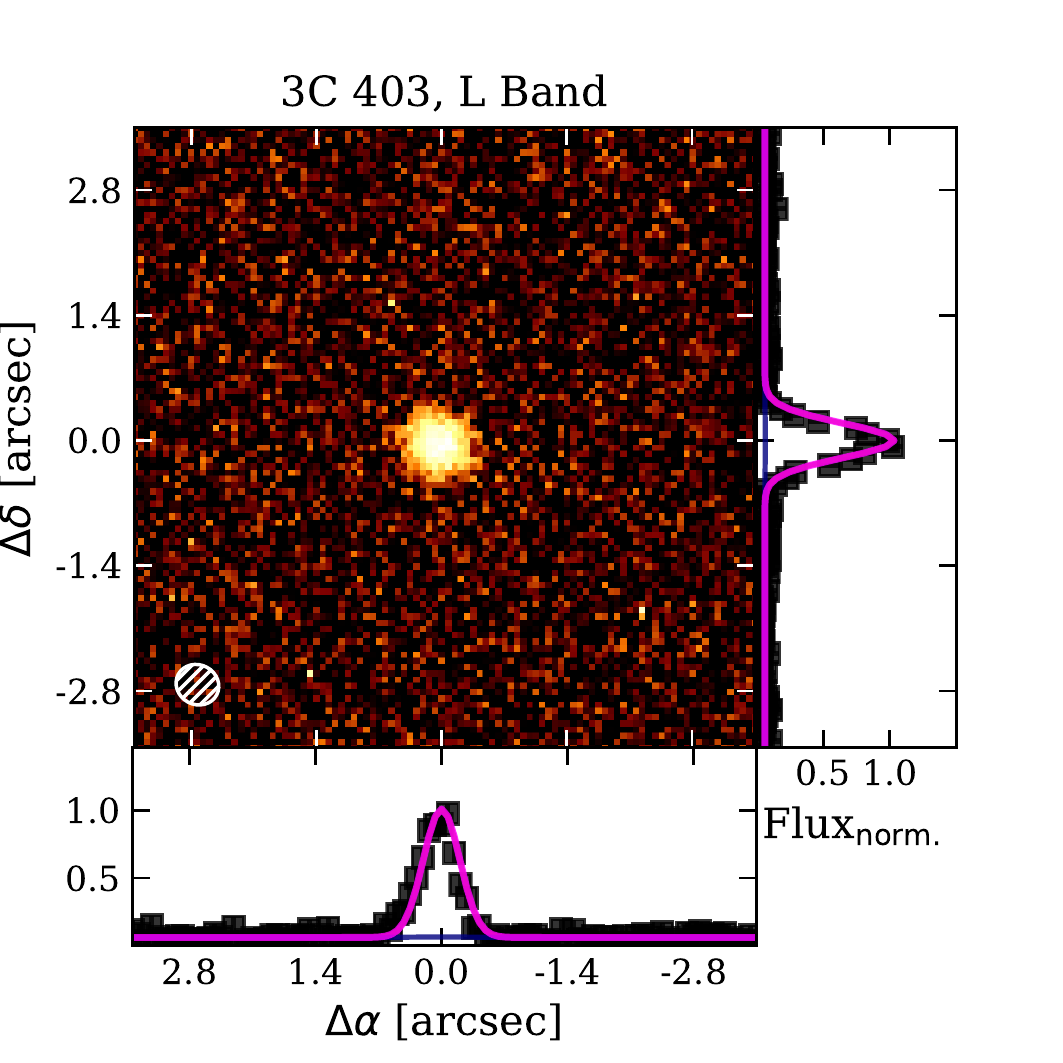}}
\subfloat{\includegraphics[width=0.25\hsize]{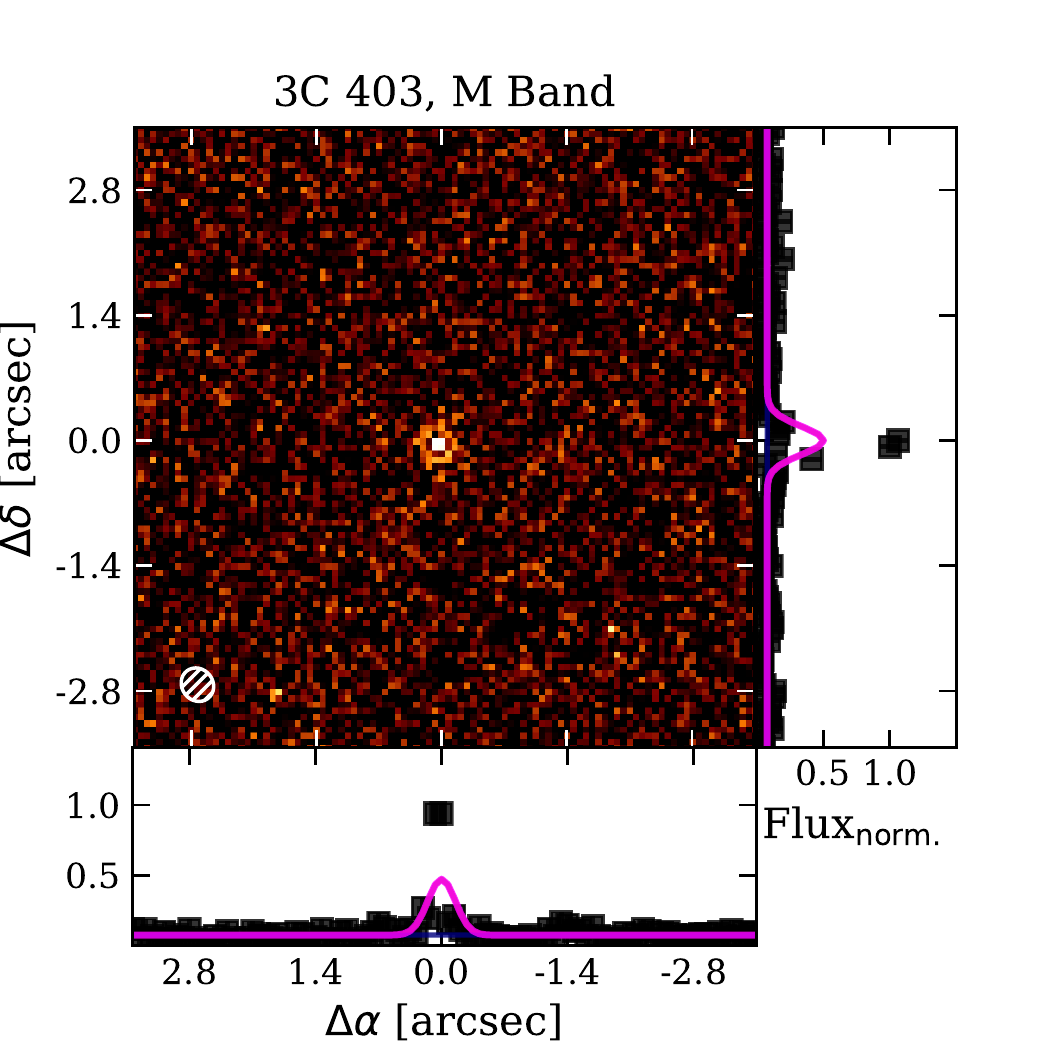}} \\
\subfloat{\includegraphics[width=0.25\hsize]{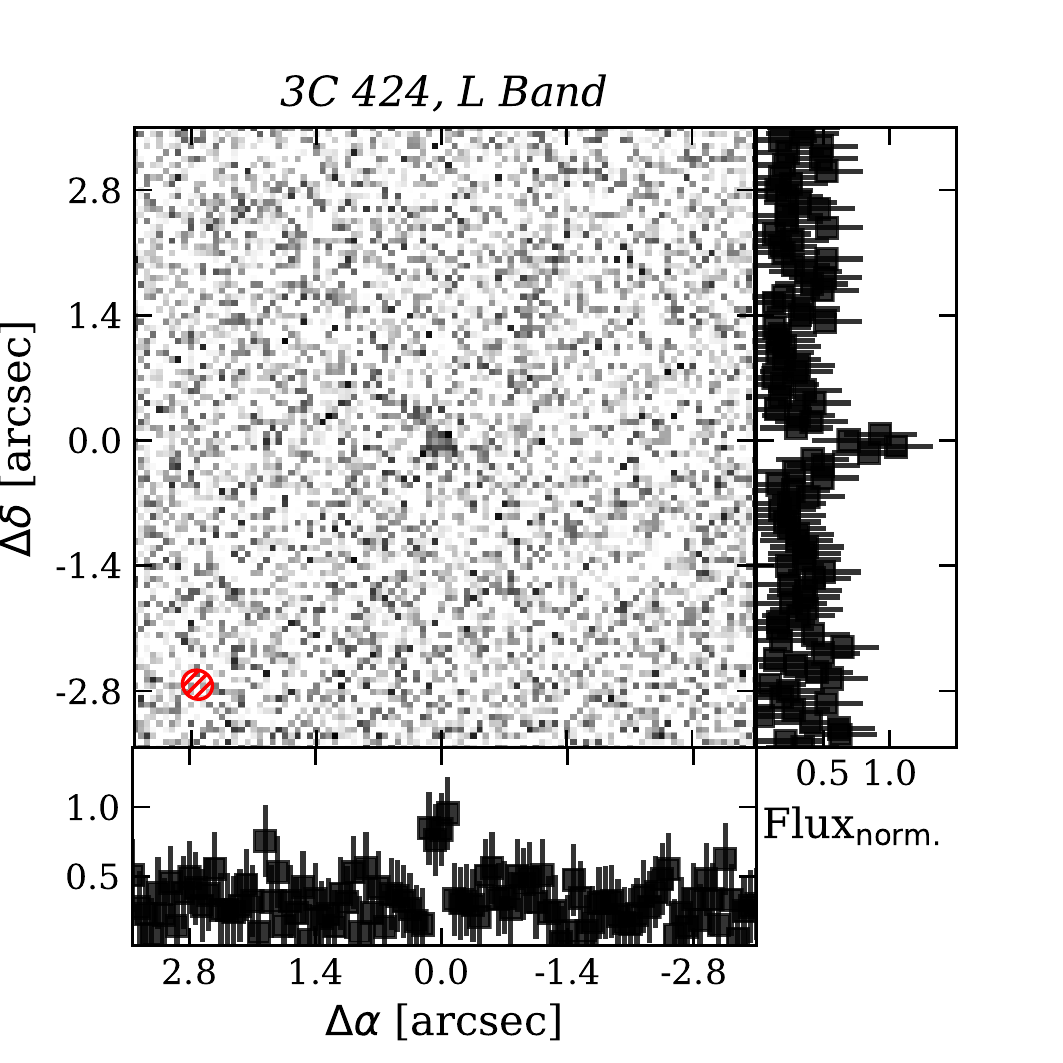}}
\subfloat{\includegraphics[width=0.25\hsize]{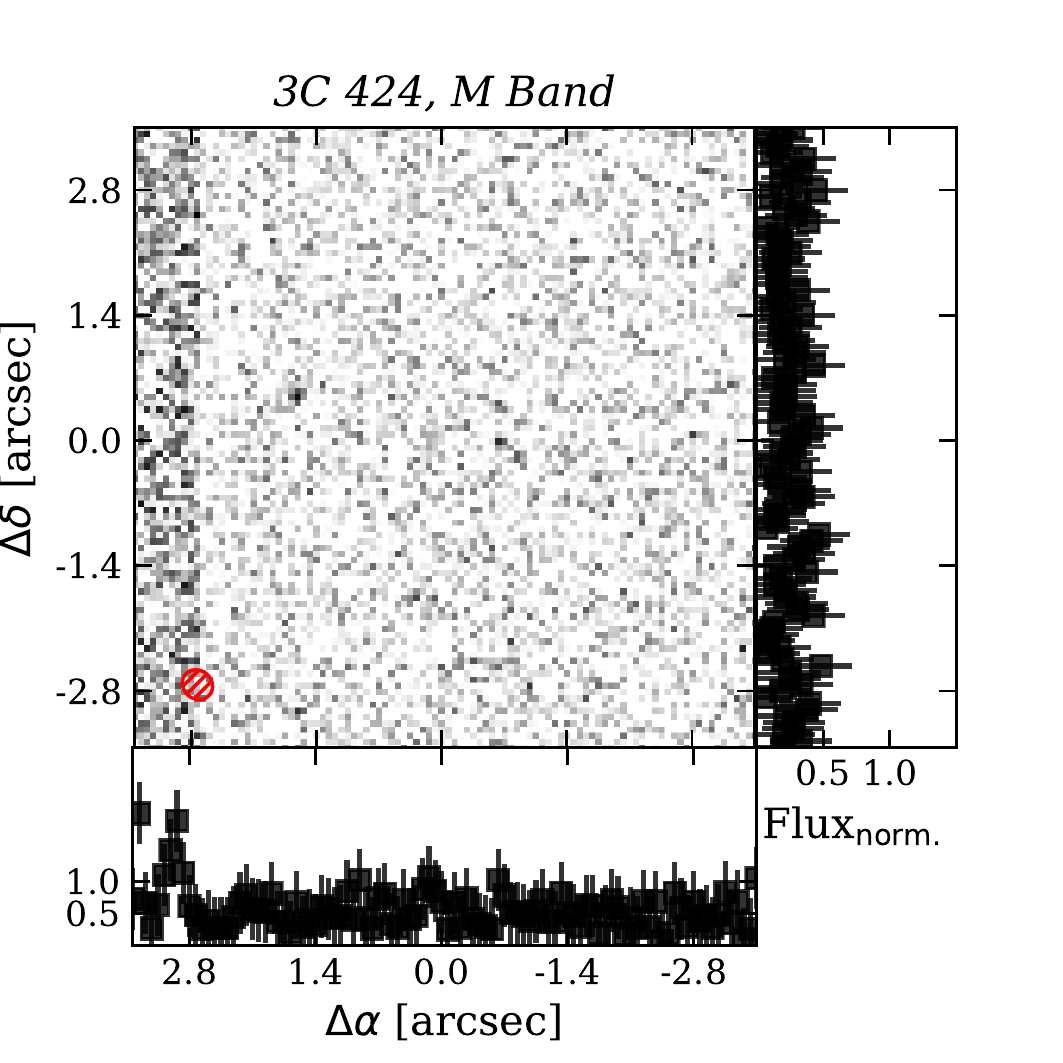}}
\subfloat{\includegraphics[width=0.25\hsize]{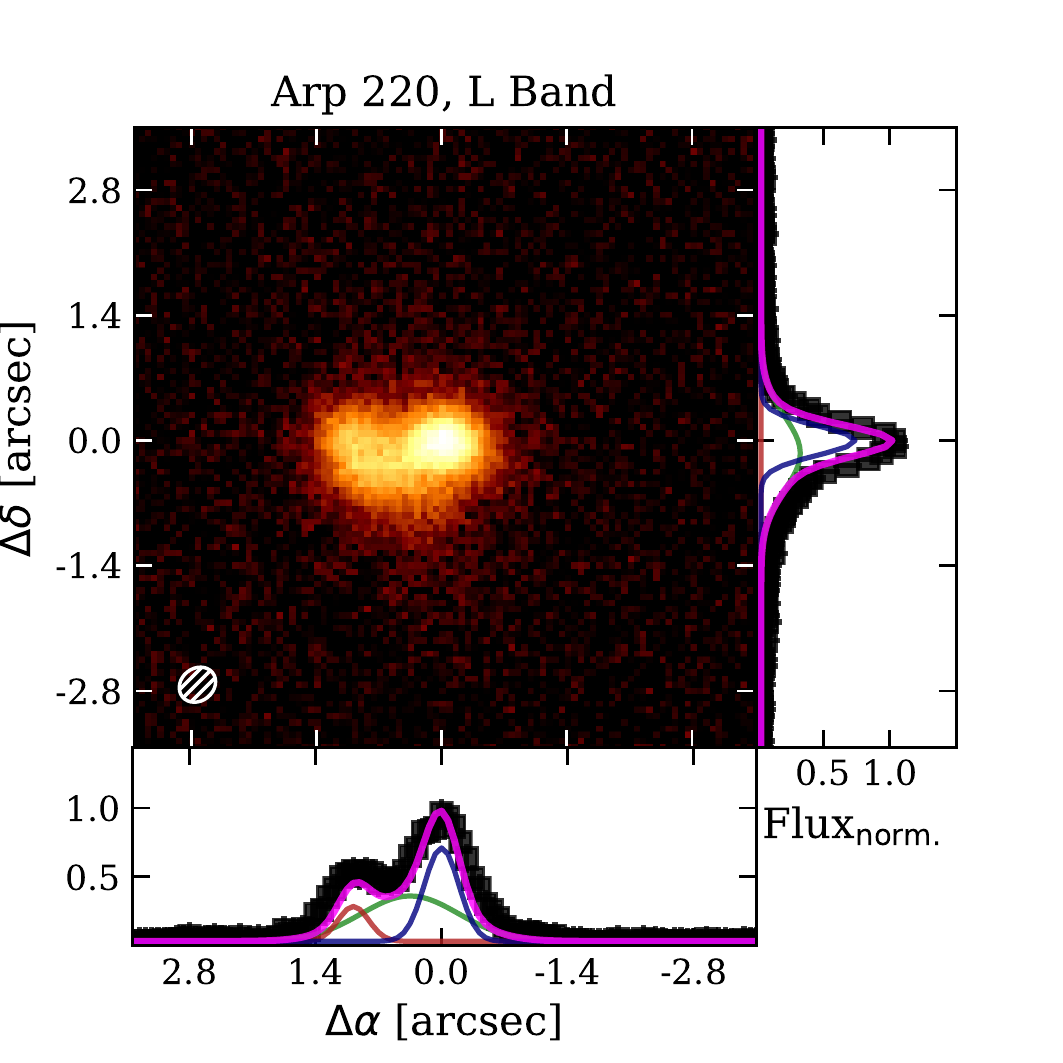}}
\subfloat{\includegraphics[width=0.25\hsize]{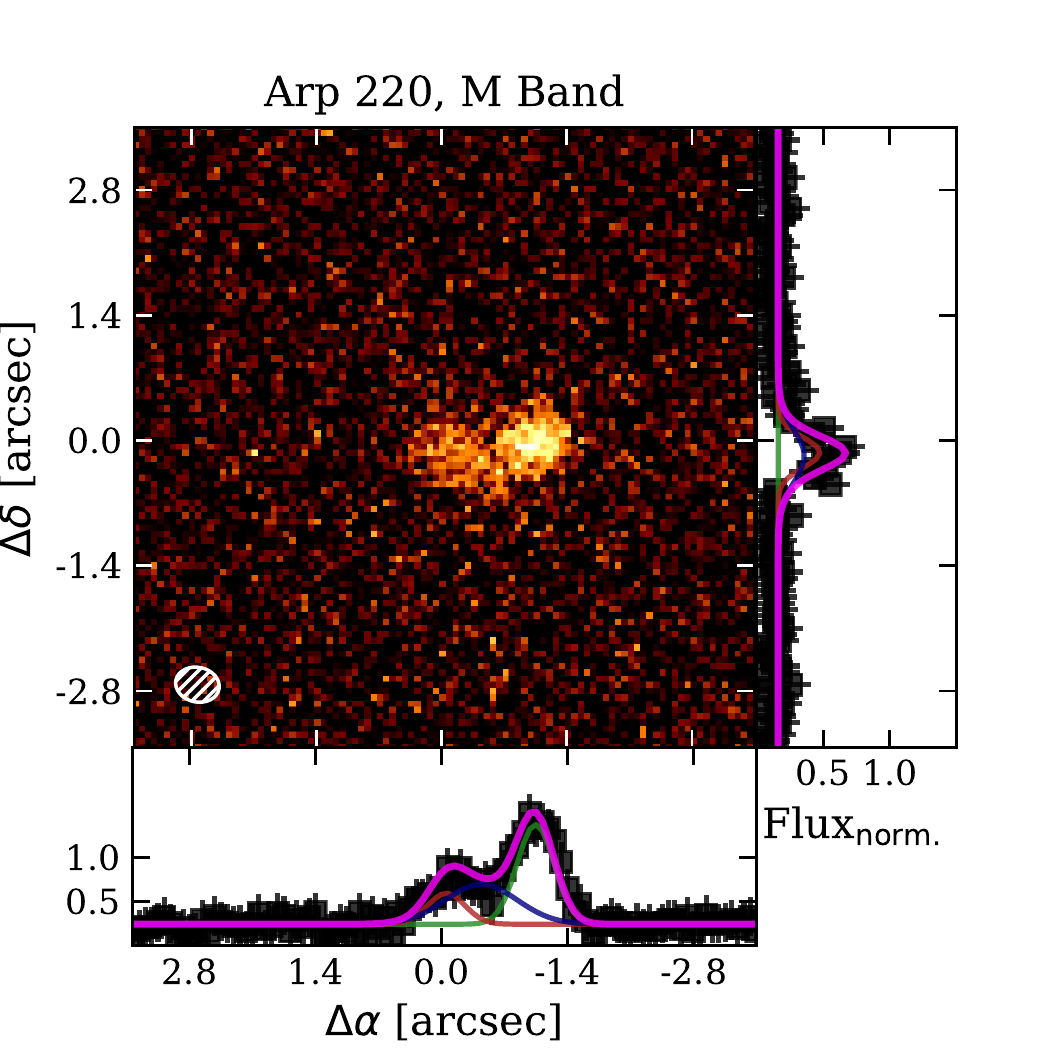}} \\
\subfloat{\includegraphics[width=0.25\hsize]{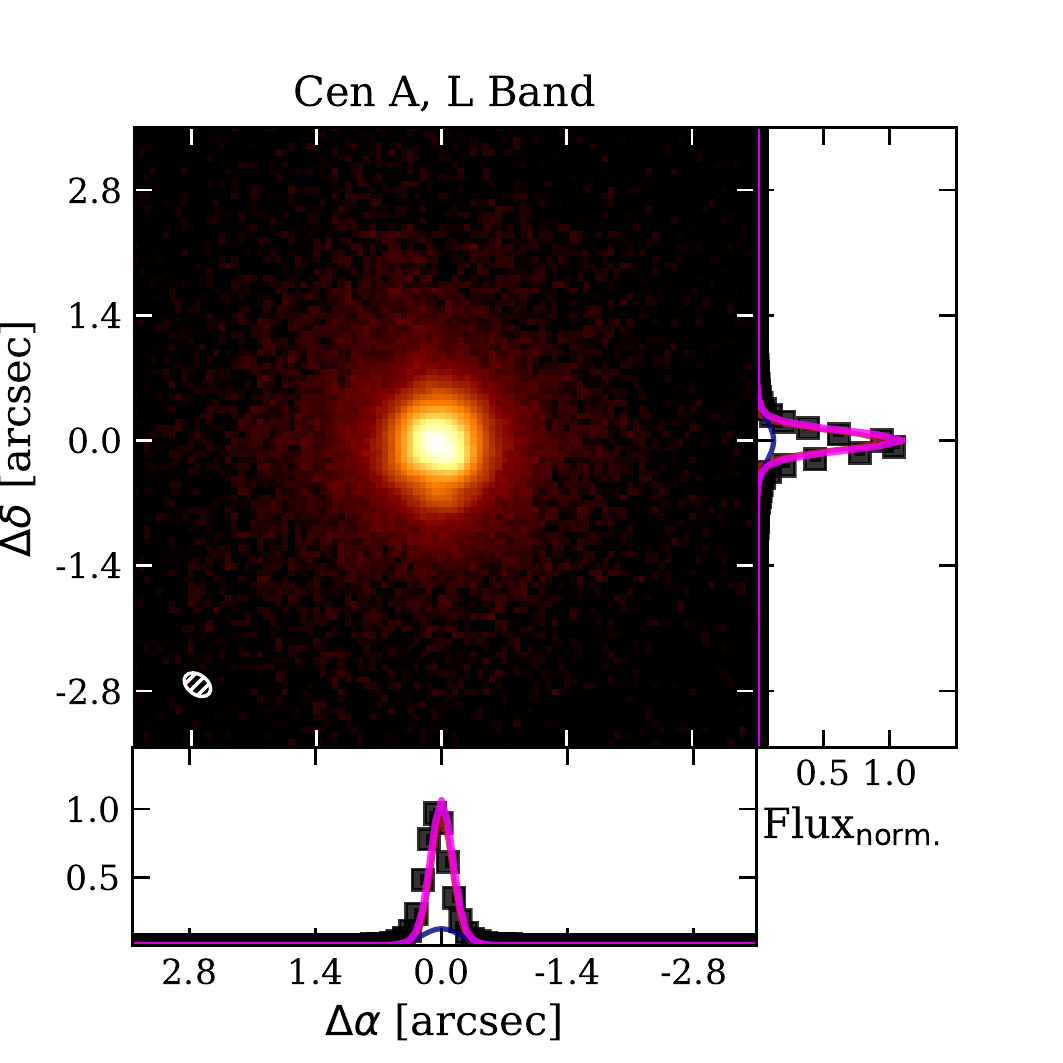}}
\subfloat{\includegraphics[width=0.25\hsize]{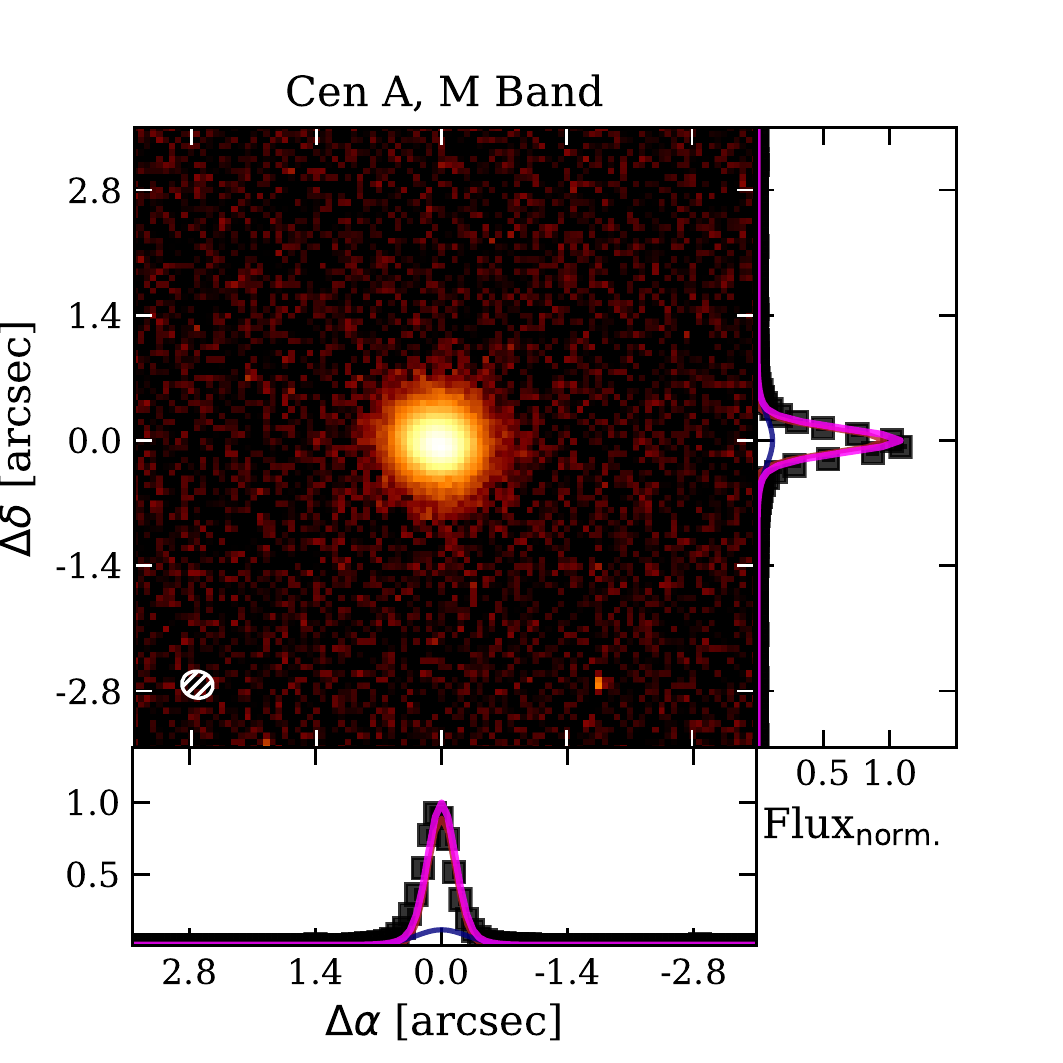}}
\subfloat{\includegraphics[width=0.25\hsize]{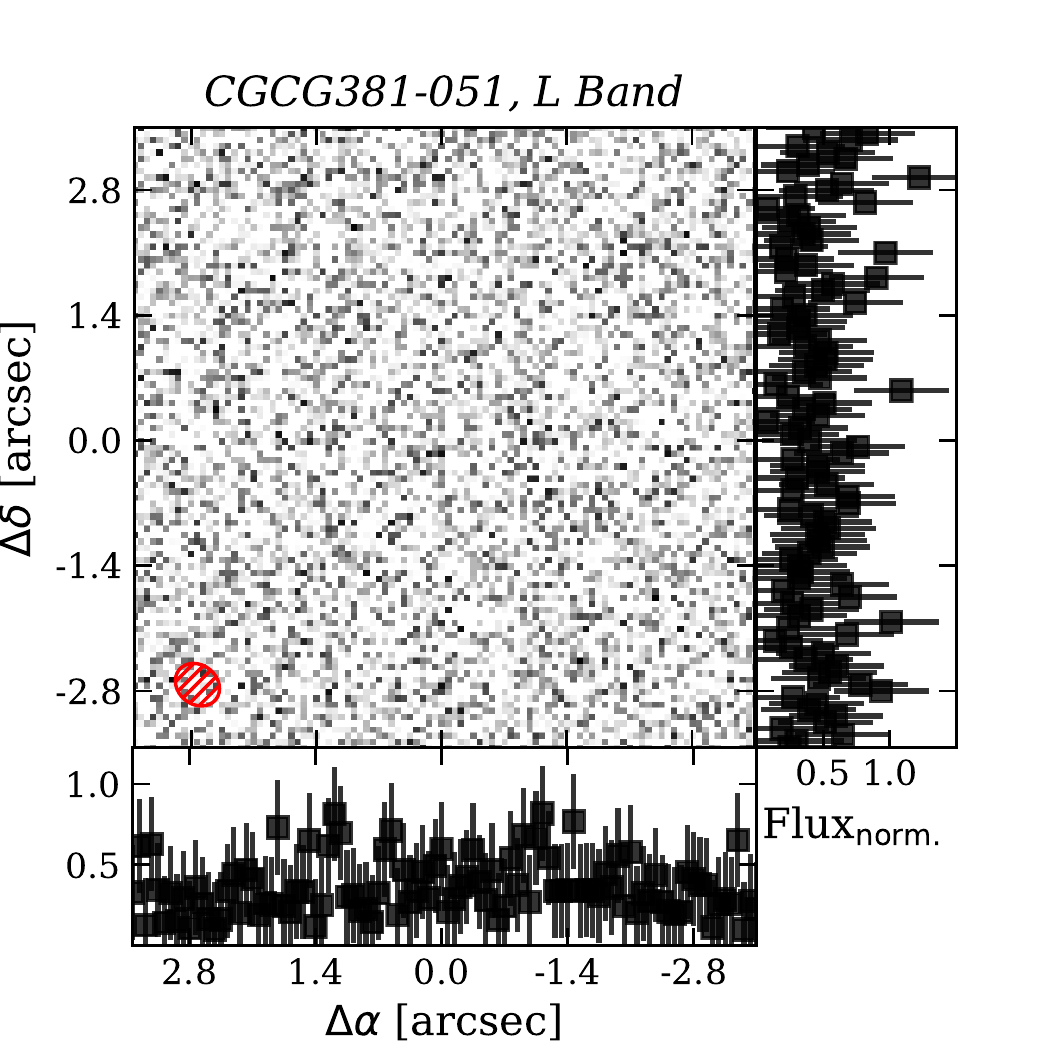}}
\subfloat{\includegraphics[width=0.25\hsize]{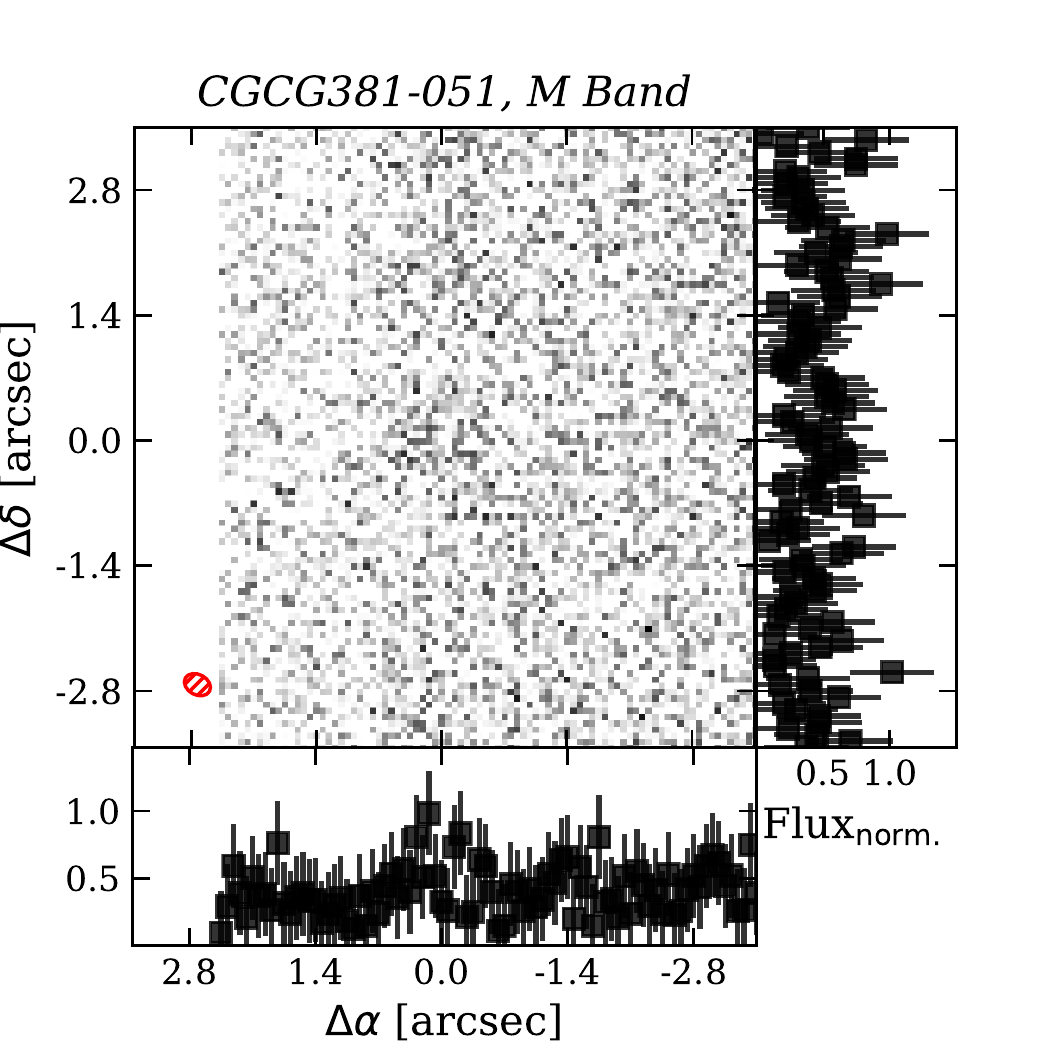}} \\
\caption{ As Fig \ref{fig:cutouts_one} but for all sources.}
\end{figure*}
\begin{figure*}
\subfloat{\includegraphics[width=0.25\hsize]{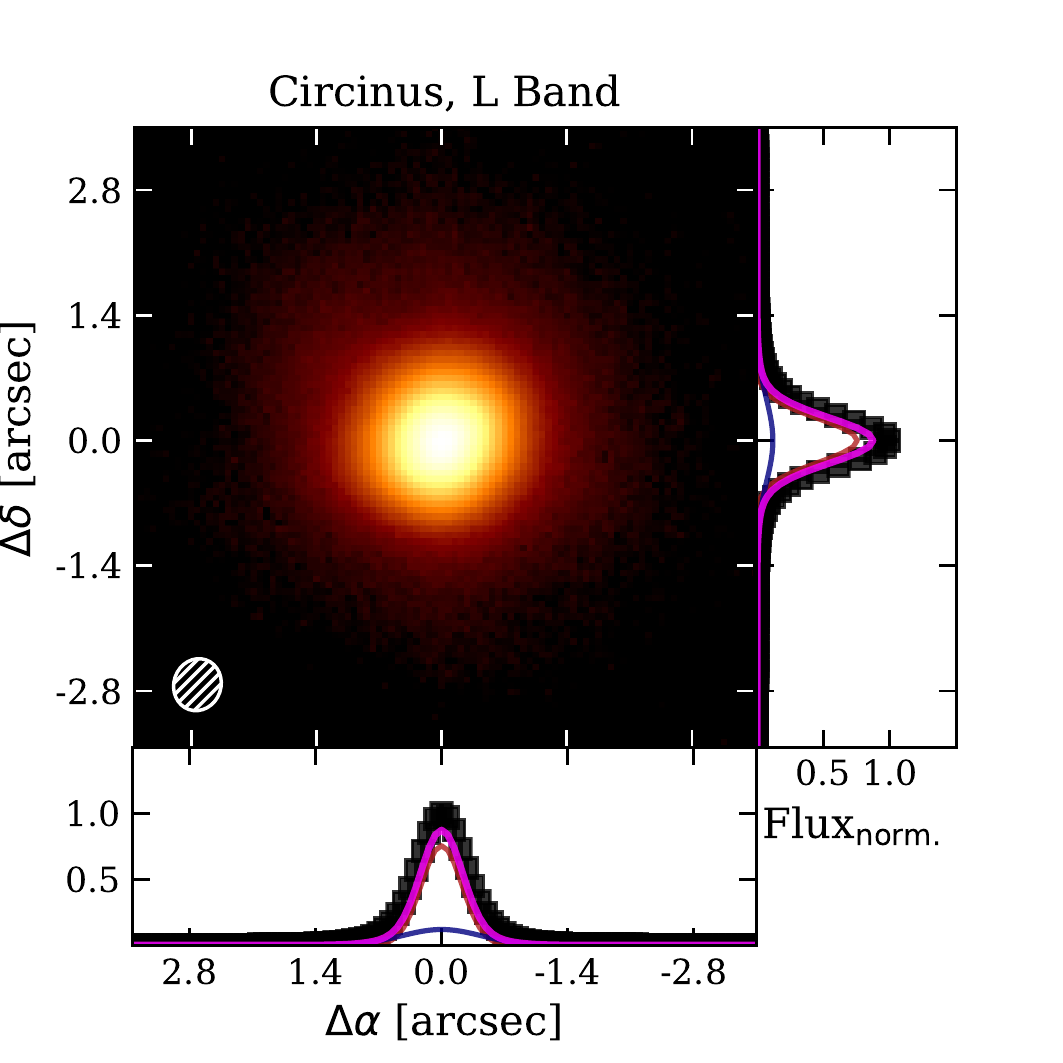}}
\subfloat{\includegraphics[width=0.25\hsize]{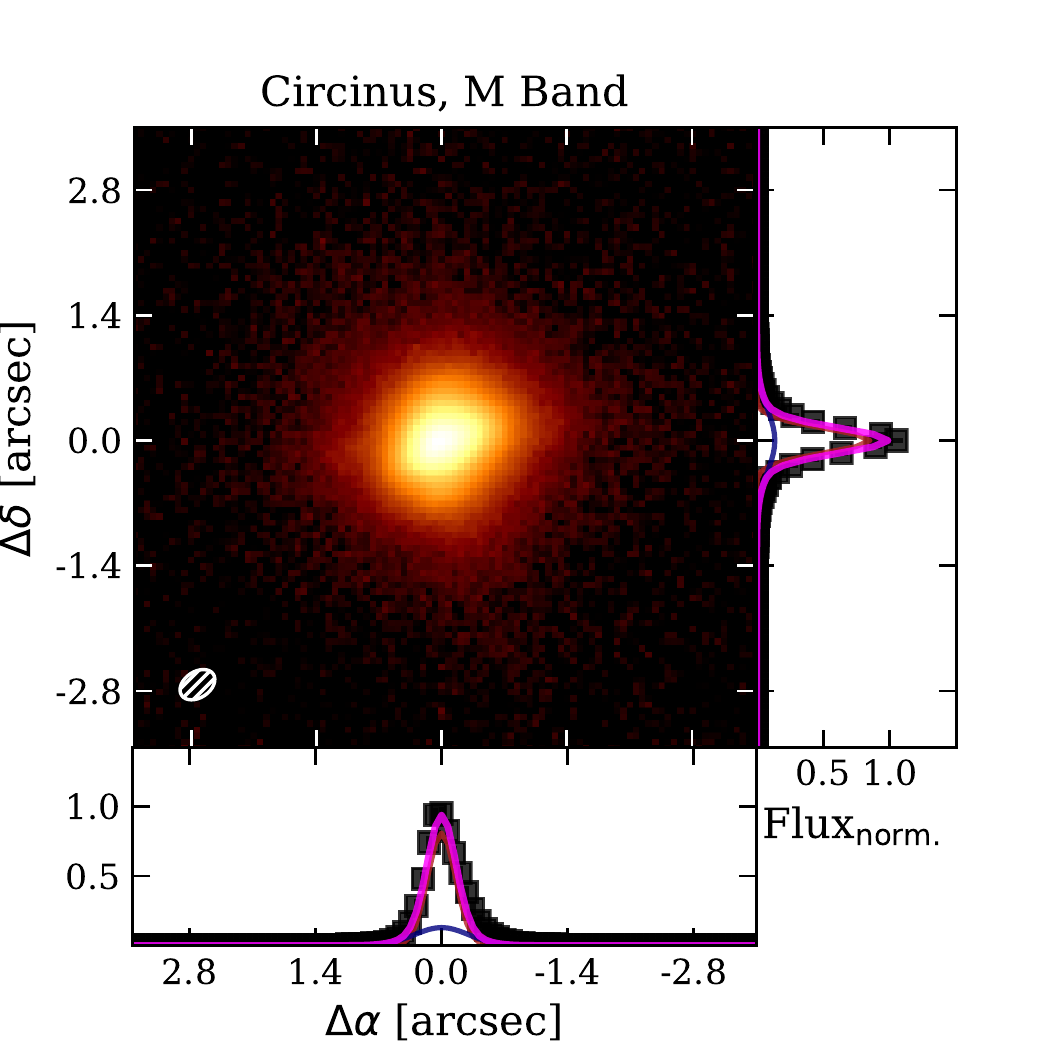}}
\subfloat{\includegraphics[width=0.25\hsize]{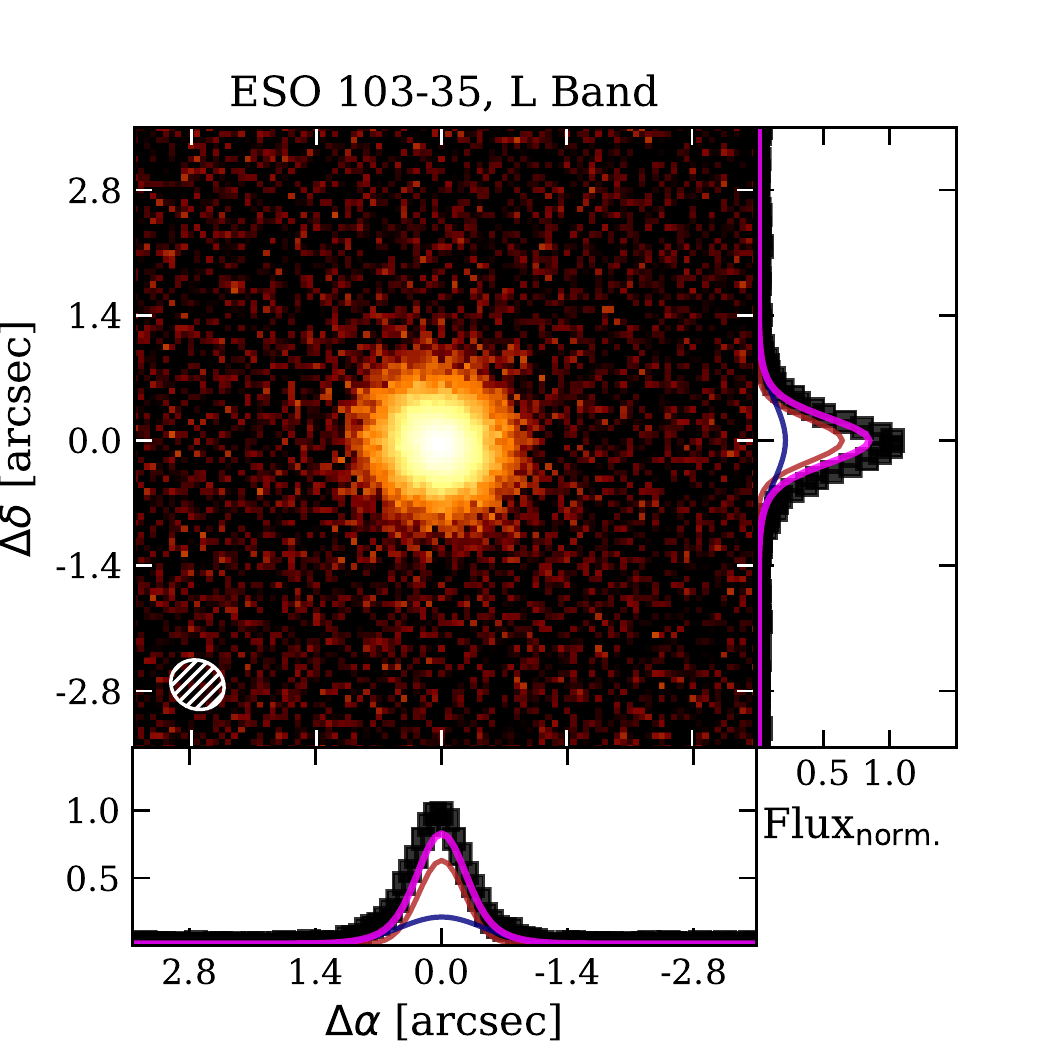}}
\subfloat{\includegraphics[width=0.25\hsize]{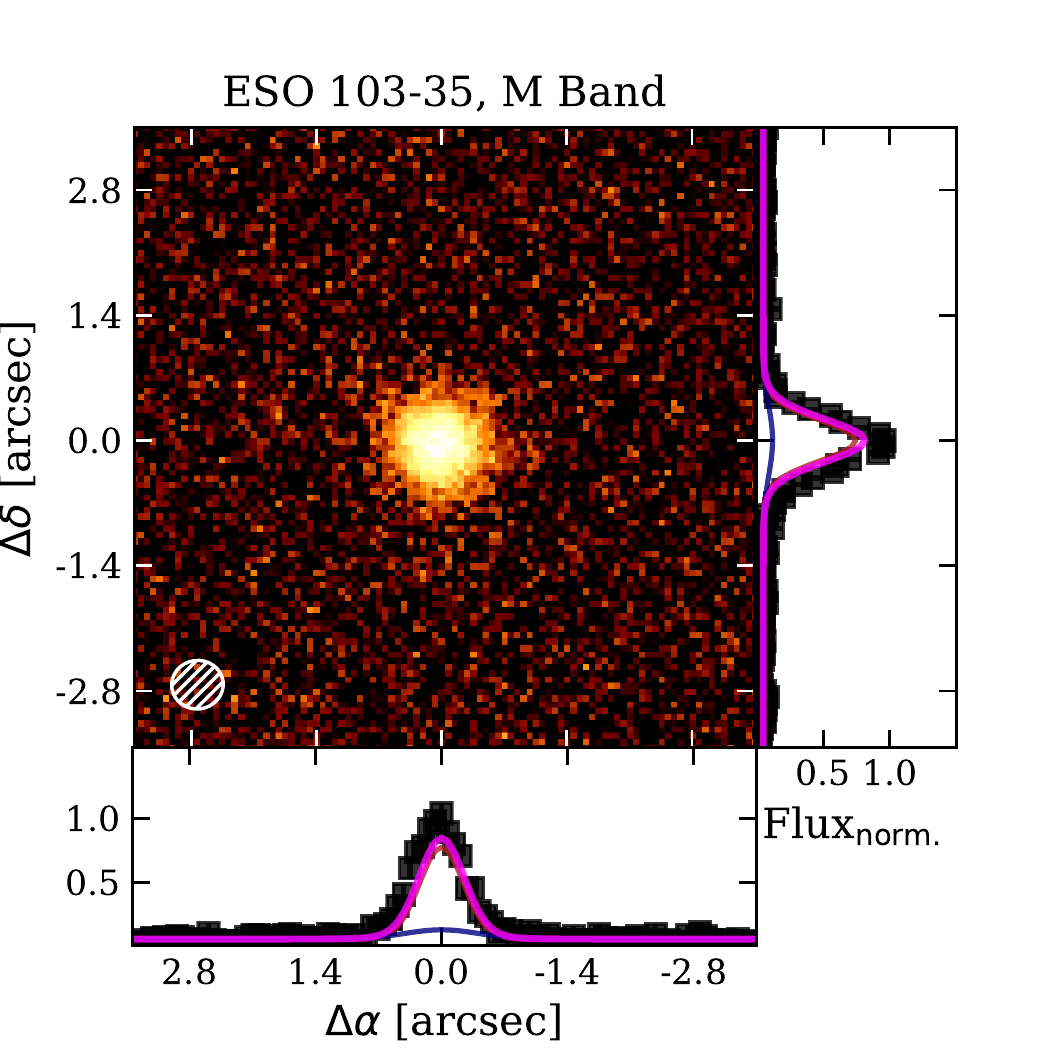}} \\
\subfloat{\includegraphics[width=0.25\hsize]{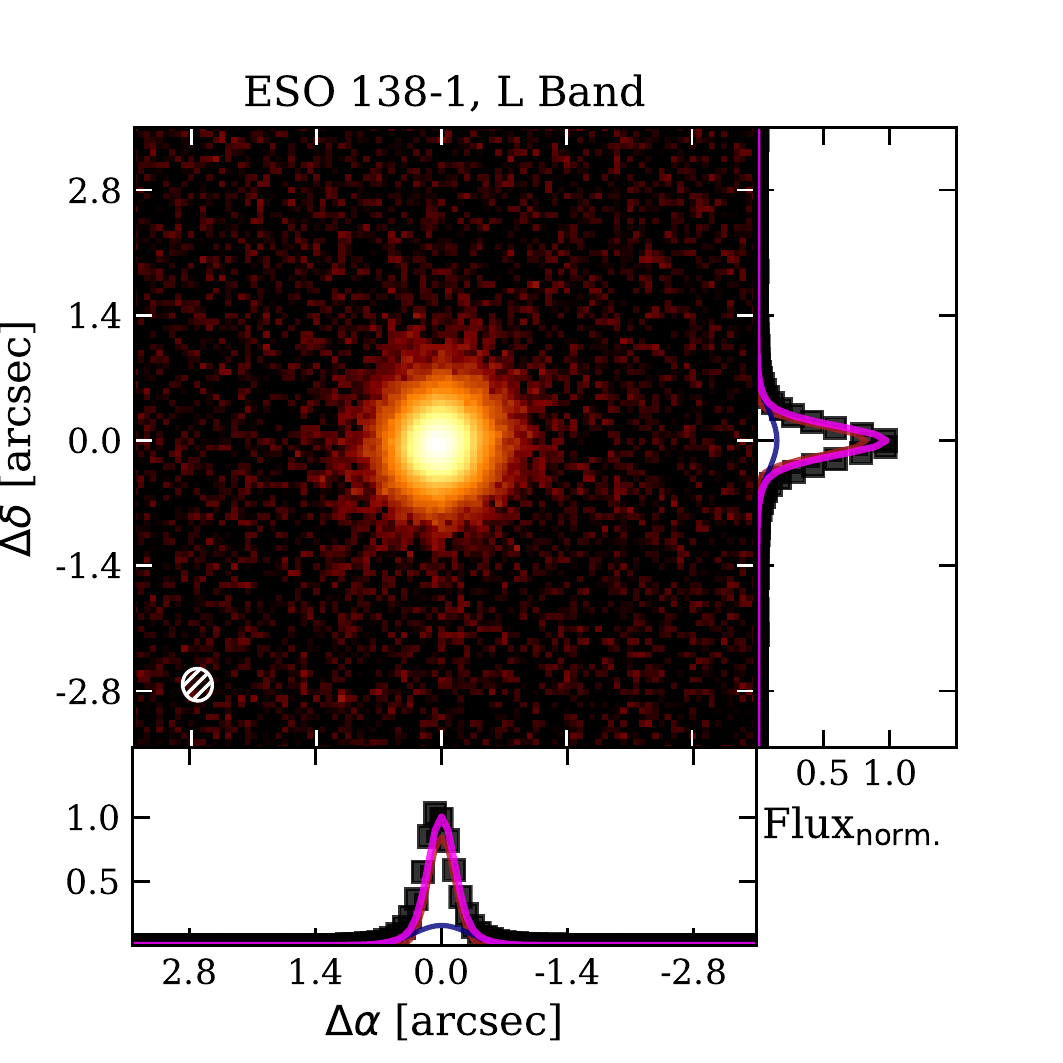}}
\subfloat{\includegraphics[width=0.25\hsize]{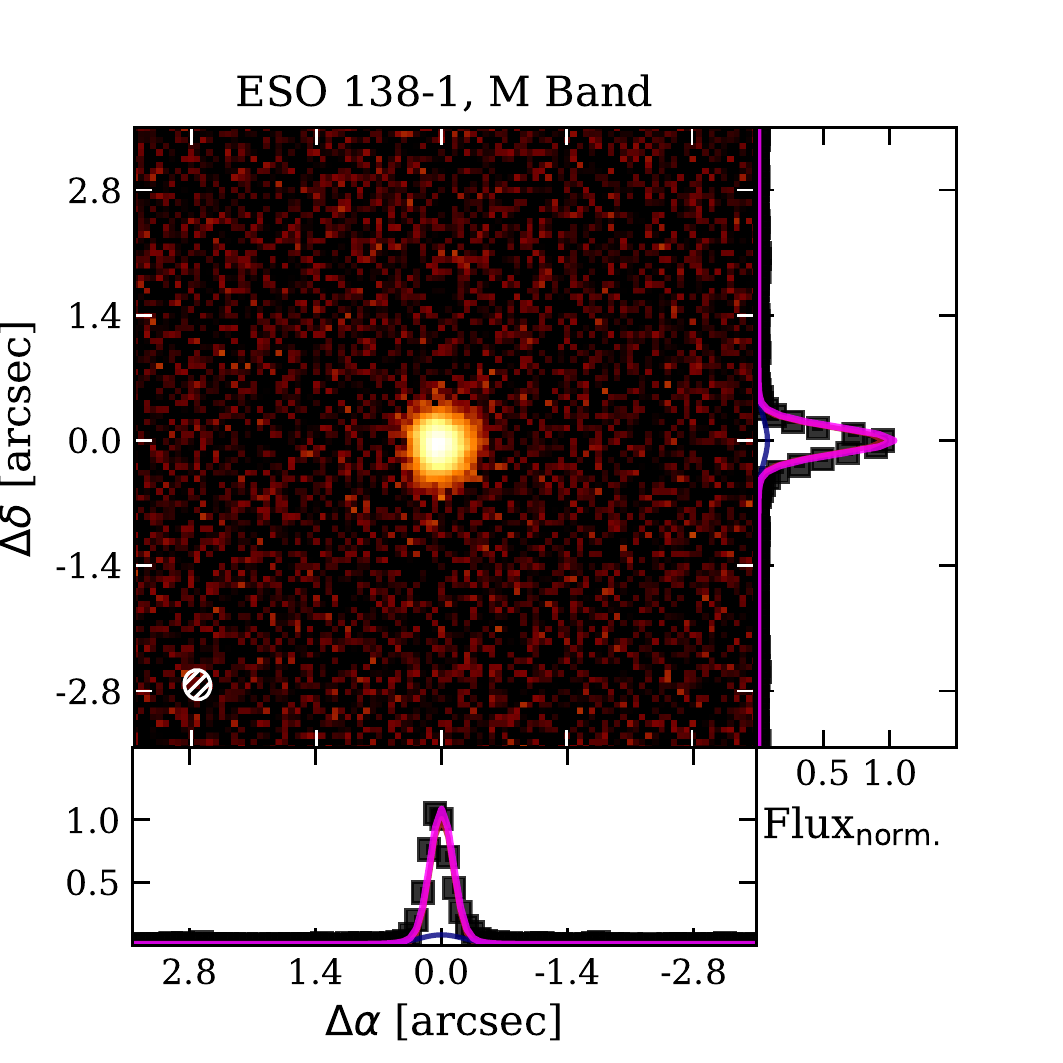}}
\subfloat{\includegraphics[width=0.25\hsize]{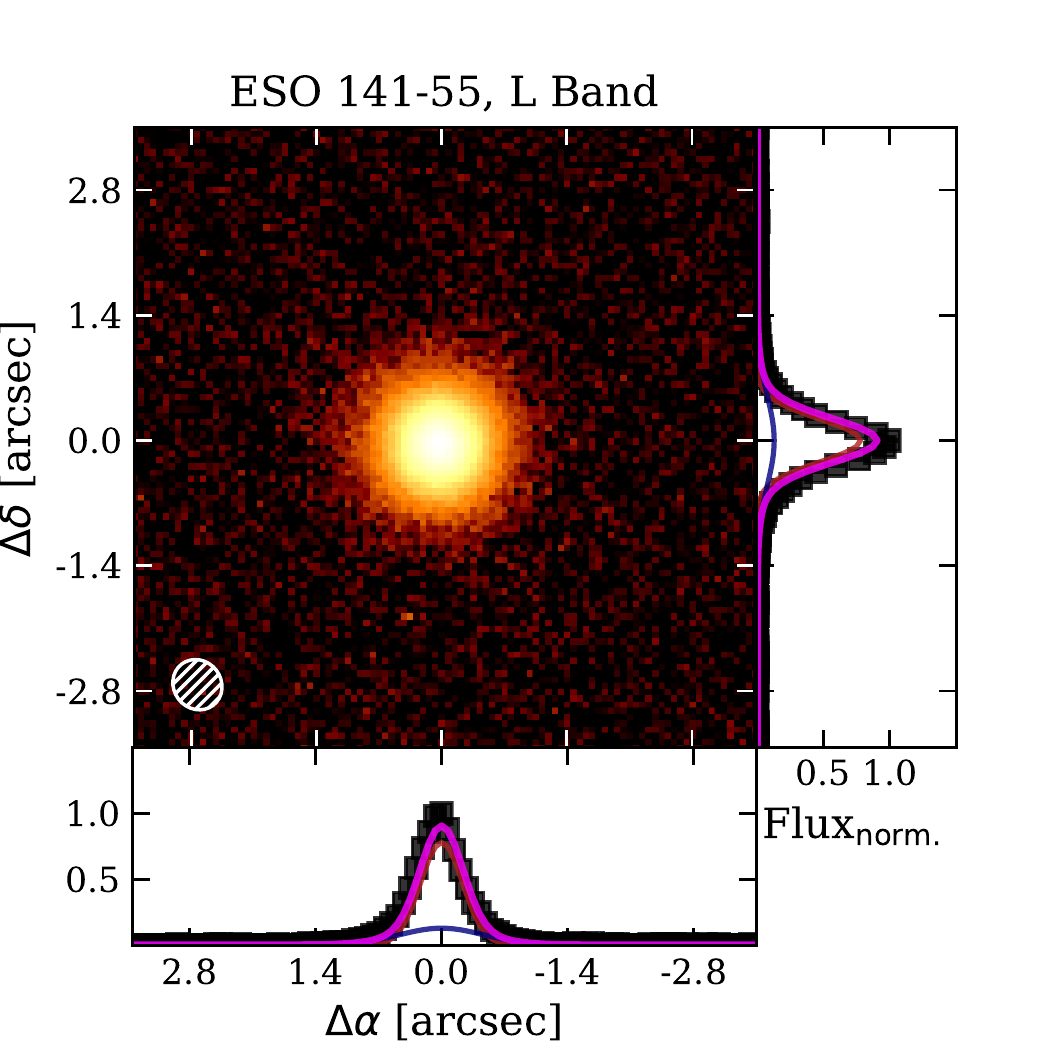}}
\subfloat{\includegraphics[width=0.25\hsize]{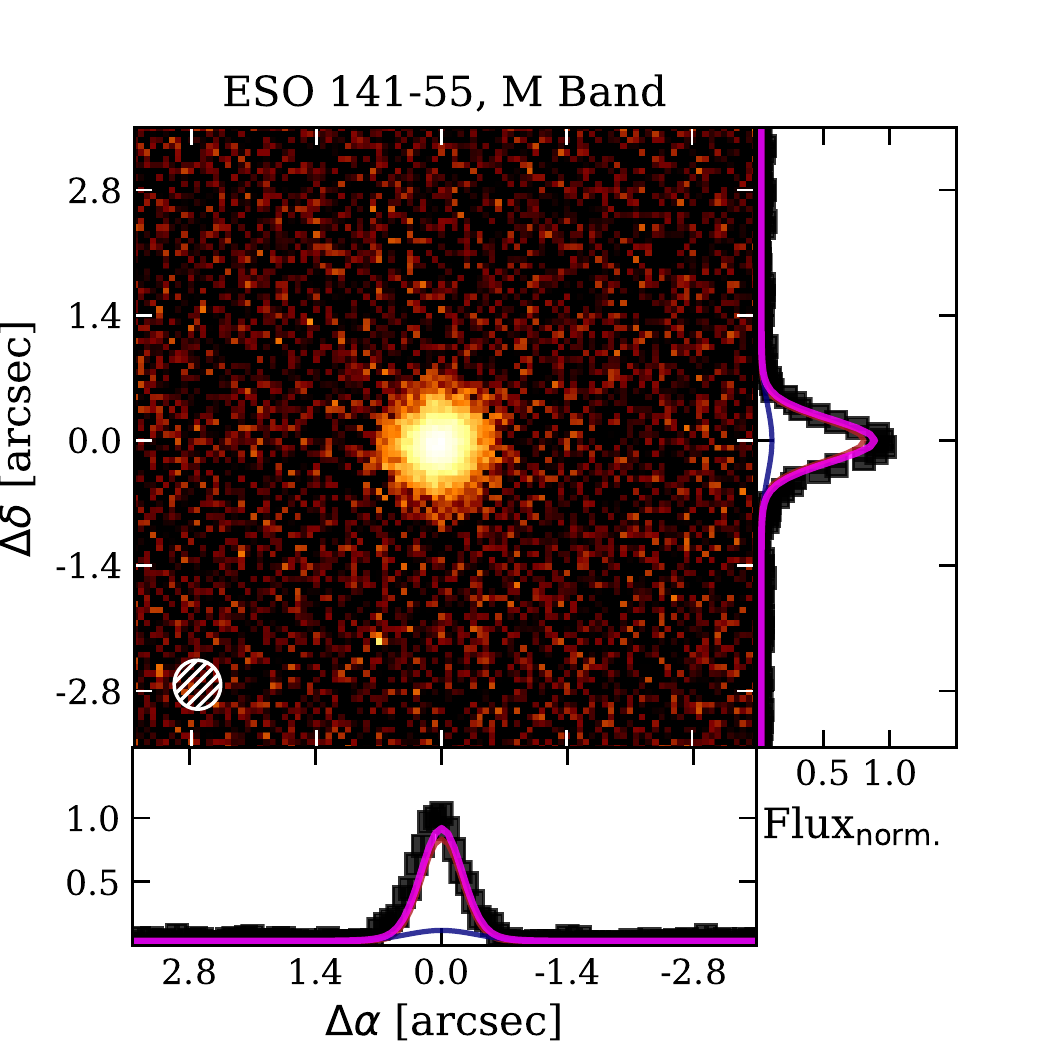}} \\
\subfloat{\includegraphics[width=0.25\hsize]{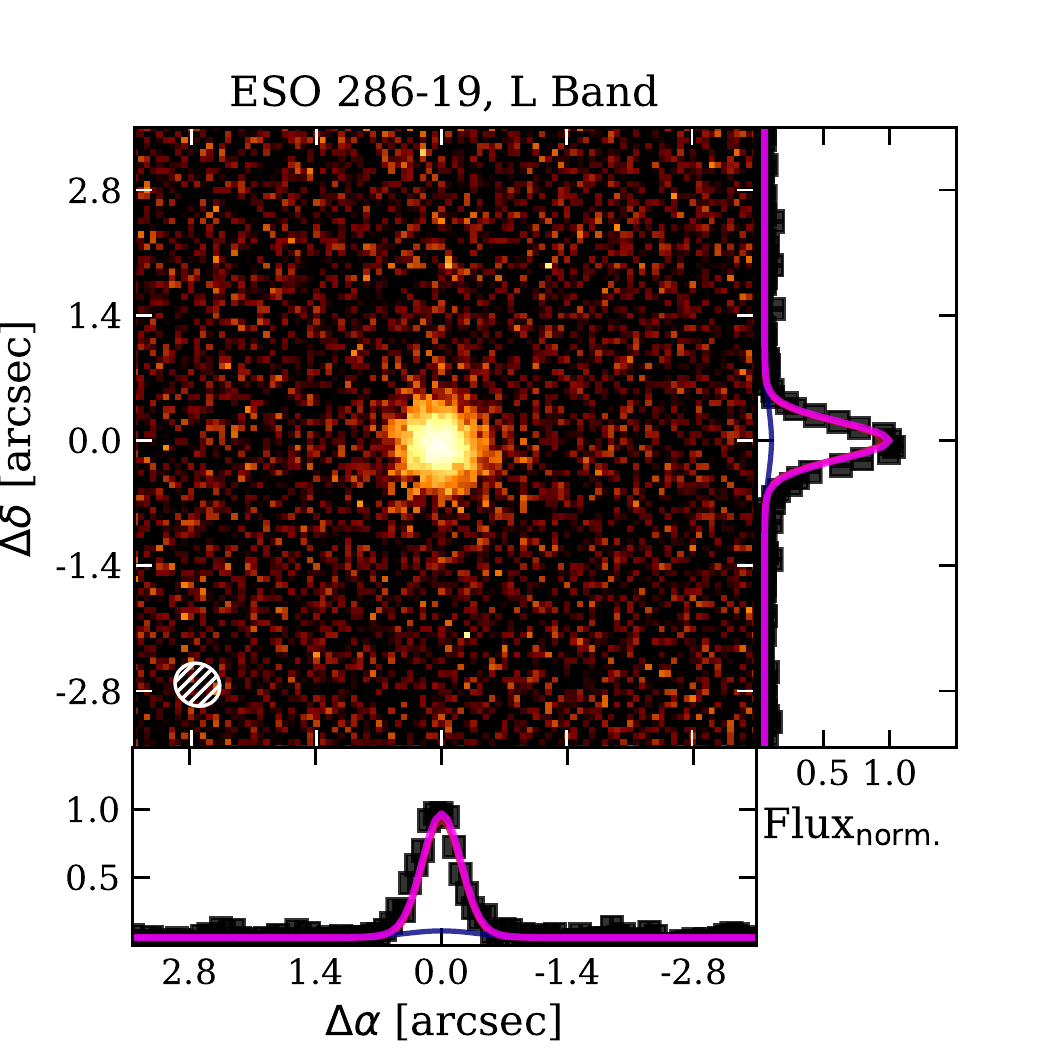}}
\subfloat{\includegraphics[width=0.25\hsize]{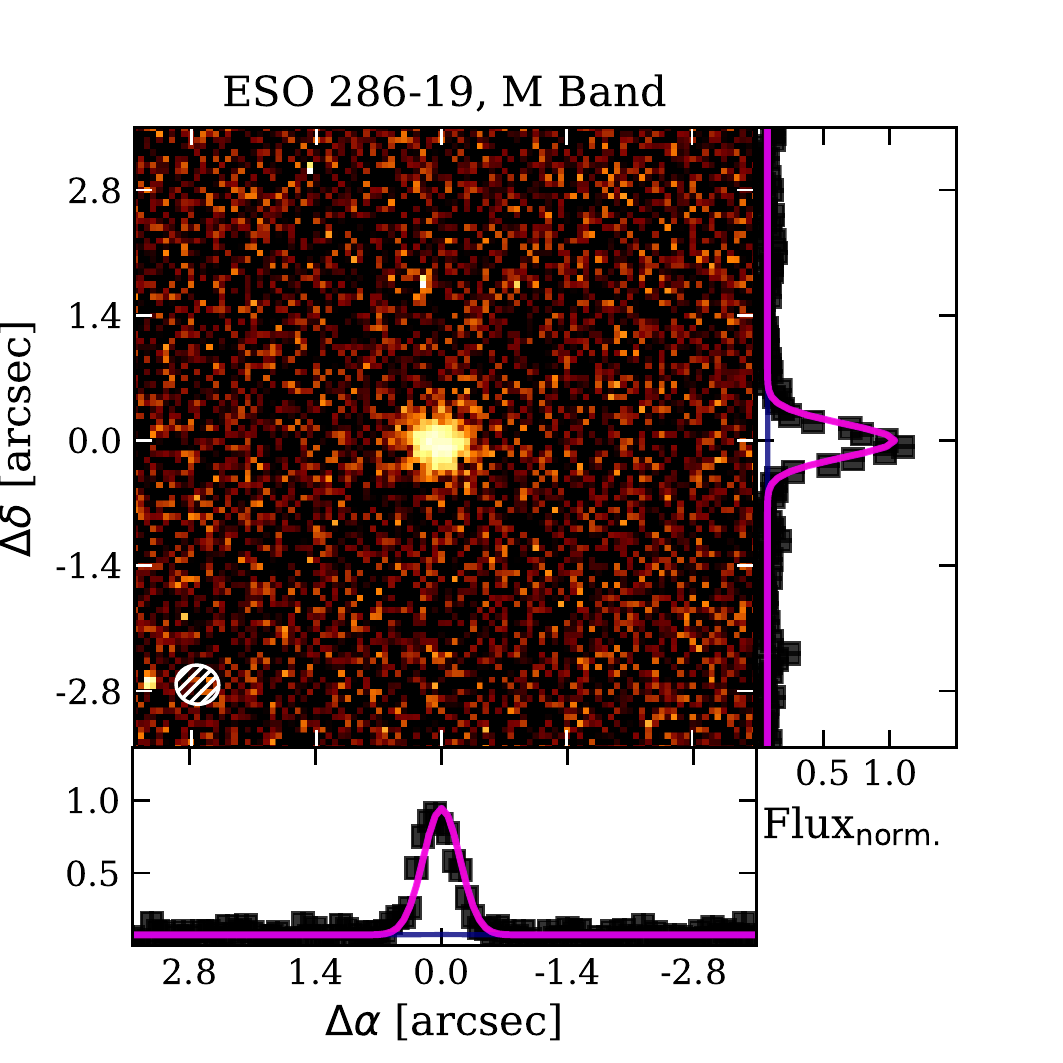}}
\subfloat{\includegraphics[width=0.25\hsize]{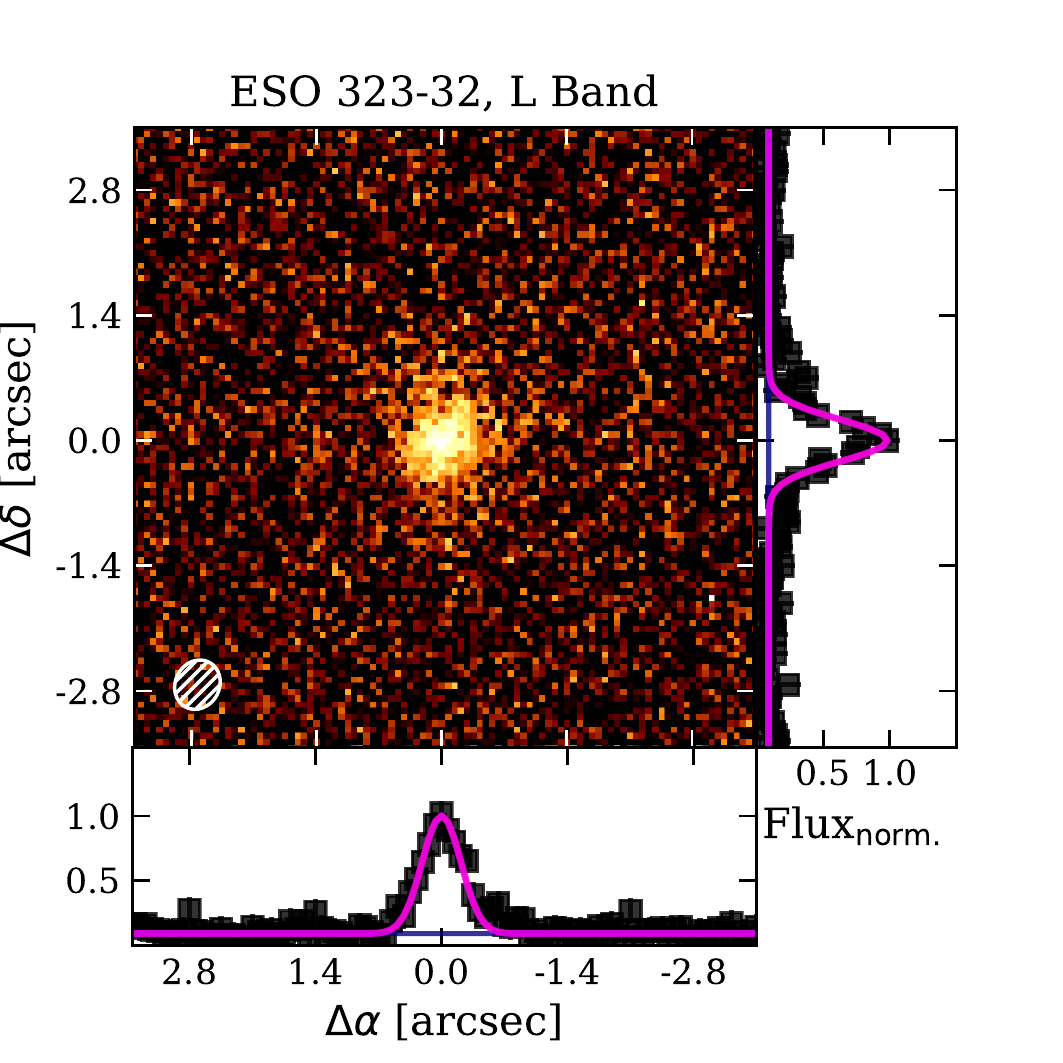}}
\subfloat{\includegraphics[width=0.25\hsize]{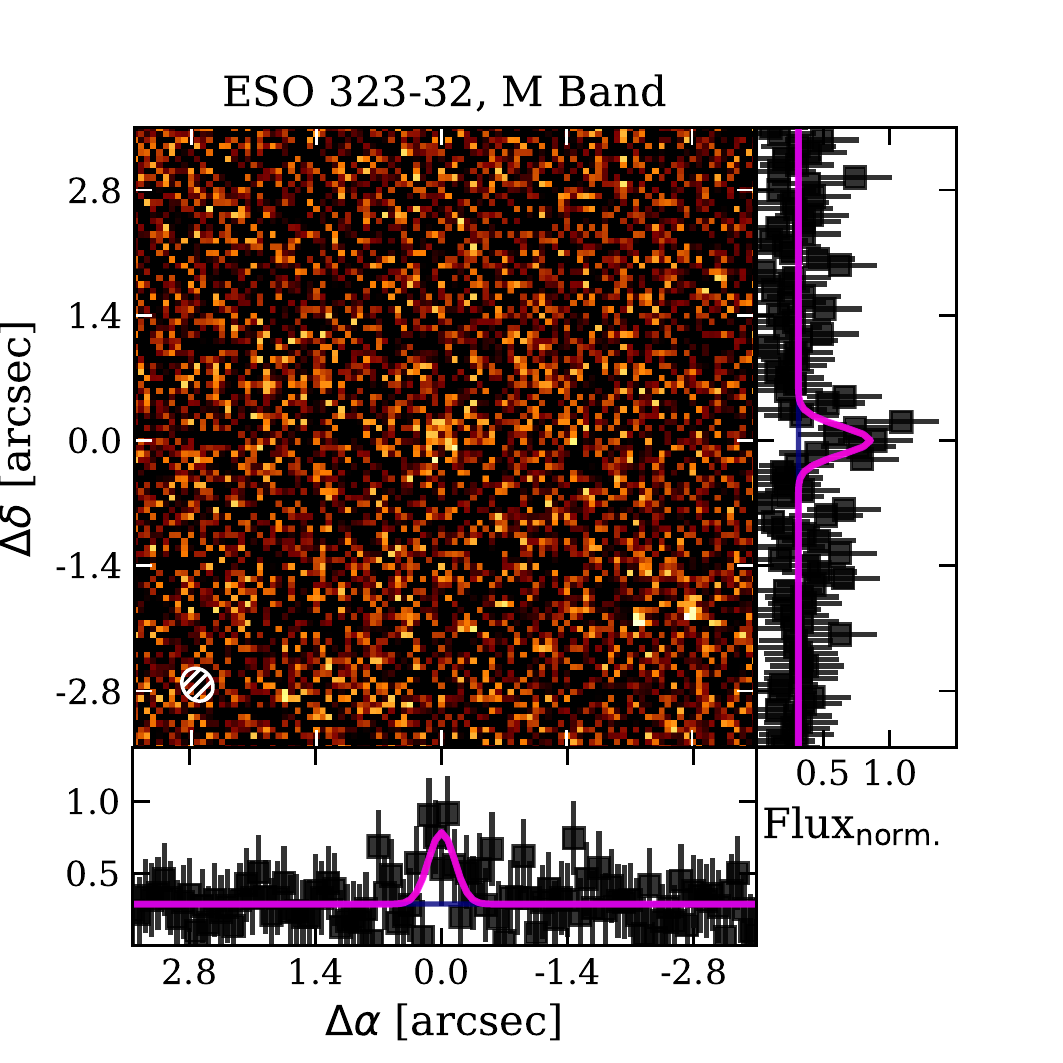}} \\
\subfloat{\includegraphics[width=0.25\hsize]{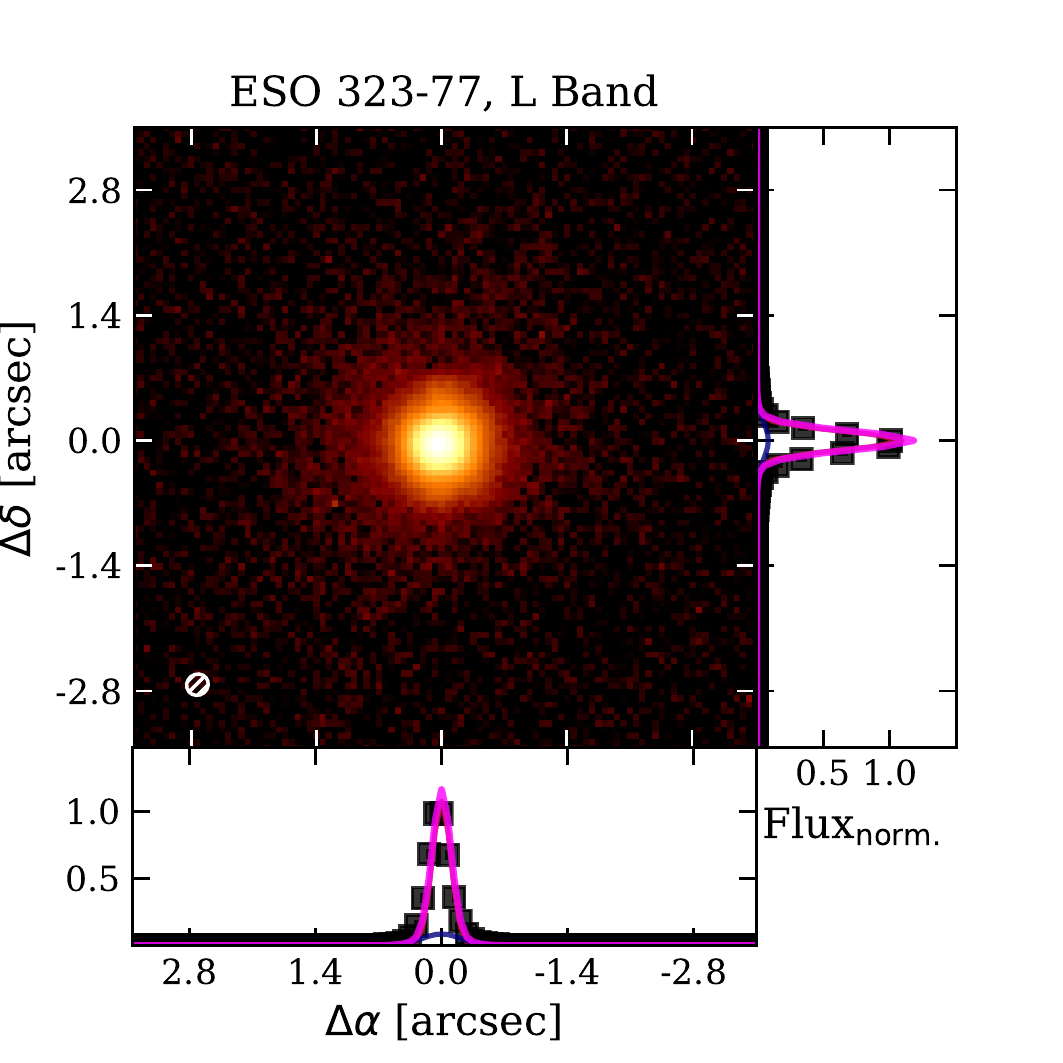}}
\subfloat{\includegraphics[width=0.25\hsize]{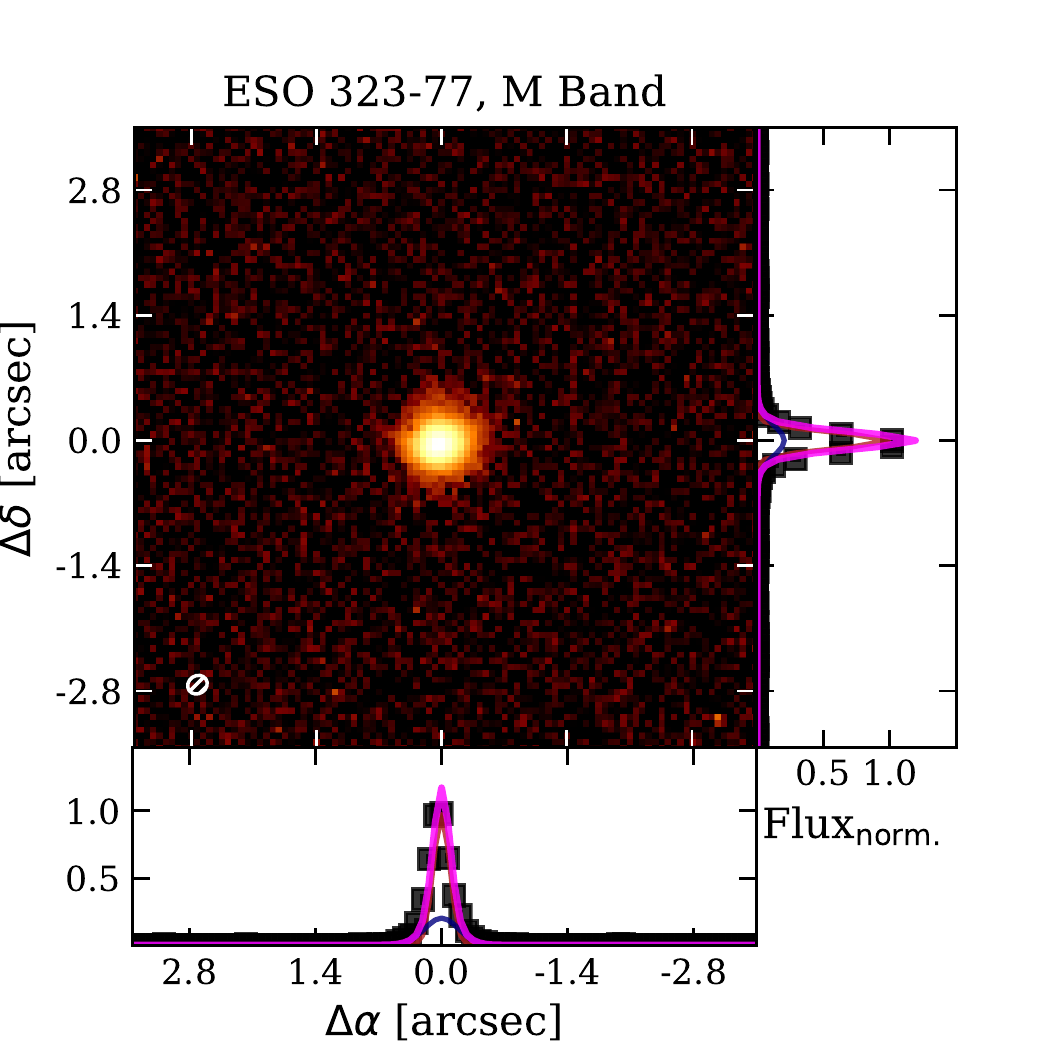}}
\subfloat{\includegraphics[width=0.25\hsize]{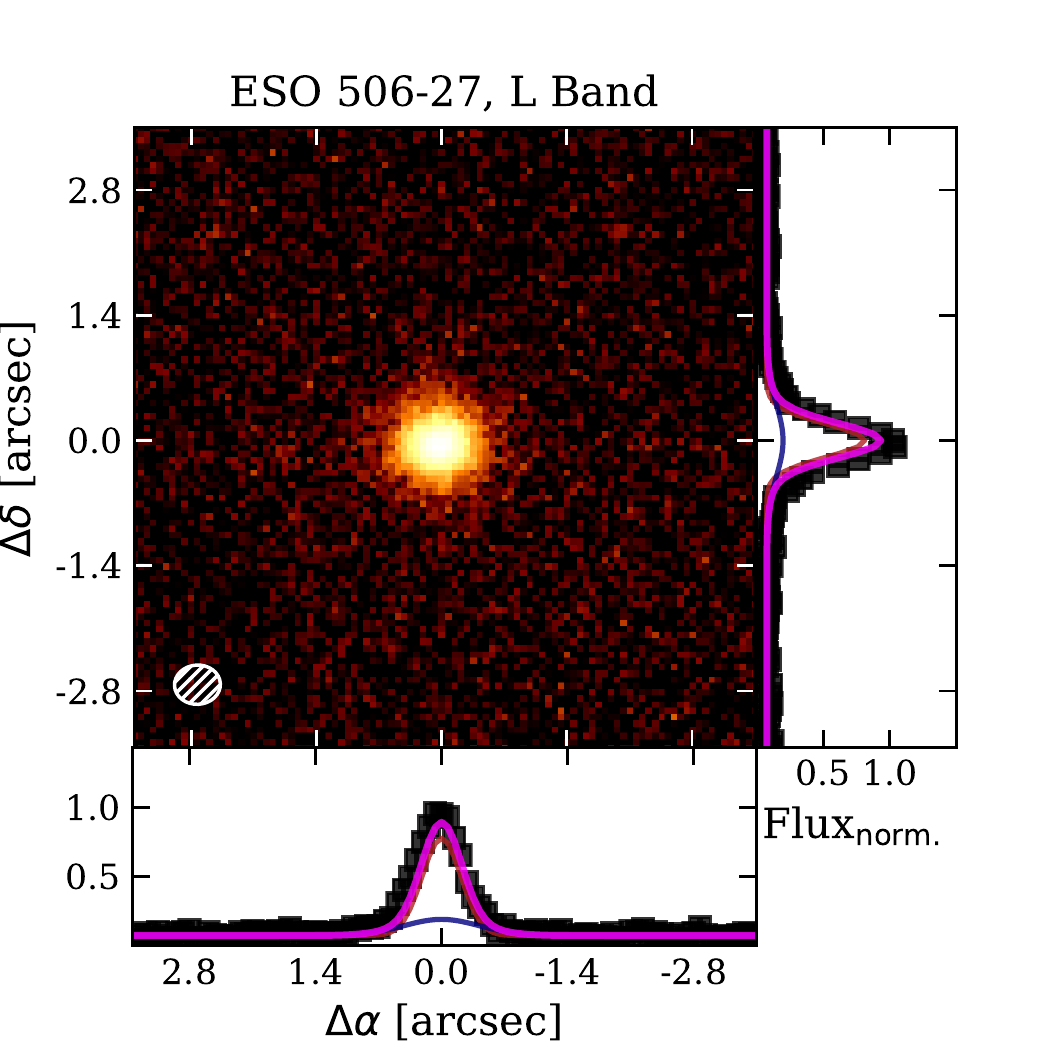}}
\subfloat{\includegraphics[width=0.25\hsize]{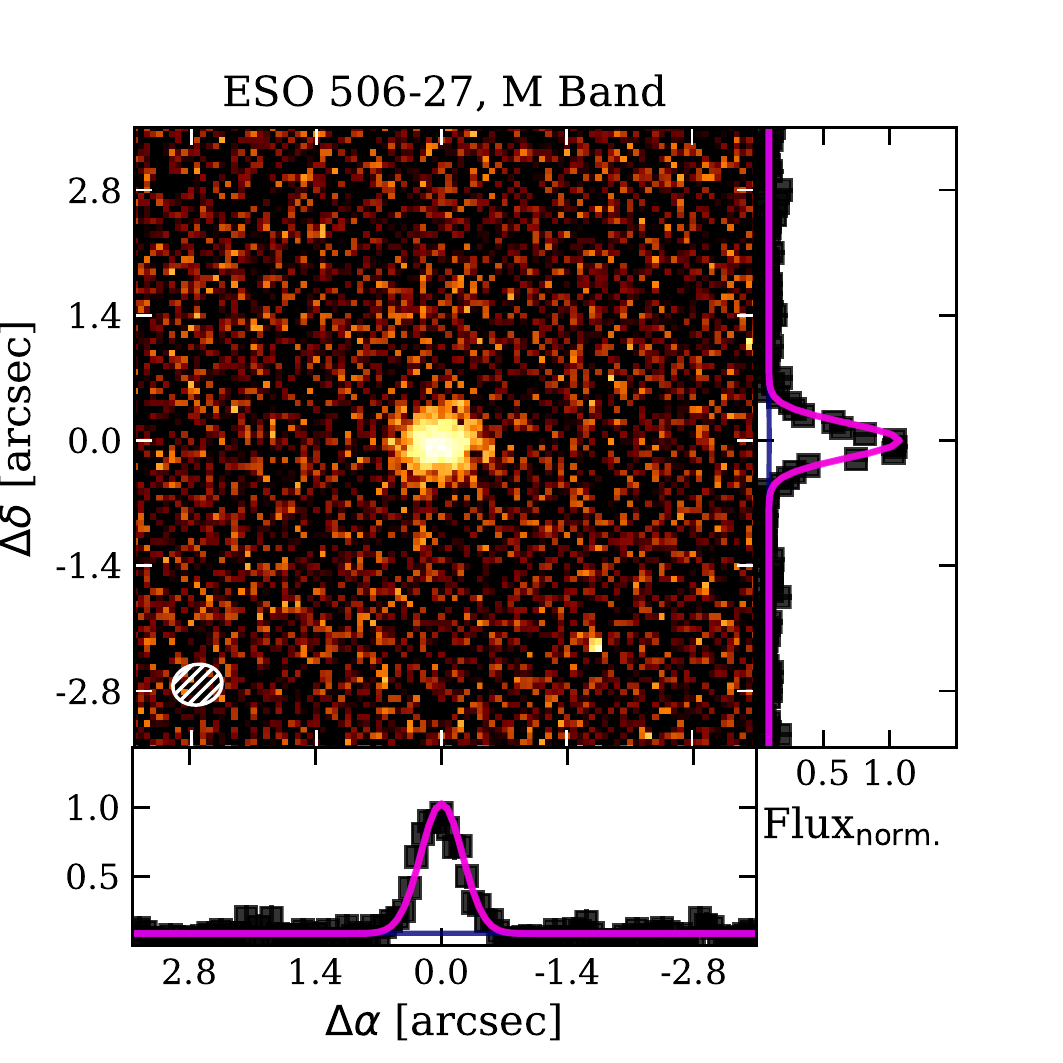}} \\
\subfloat{\includegraphics[width=0.25\hsize]{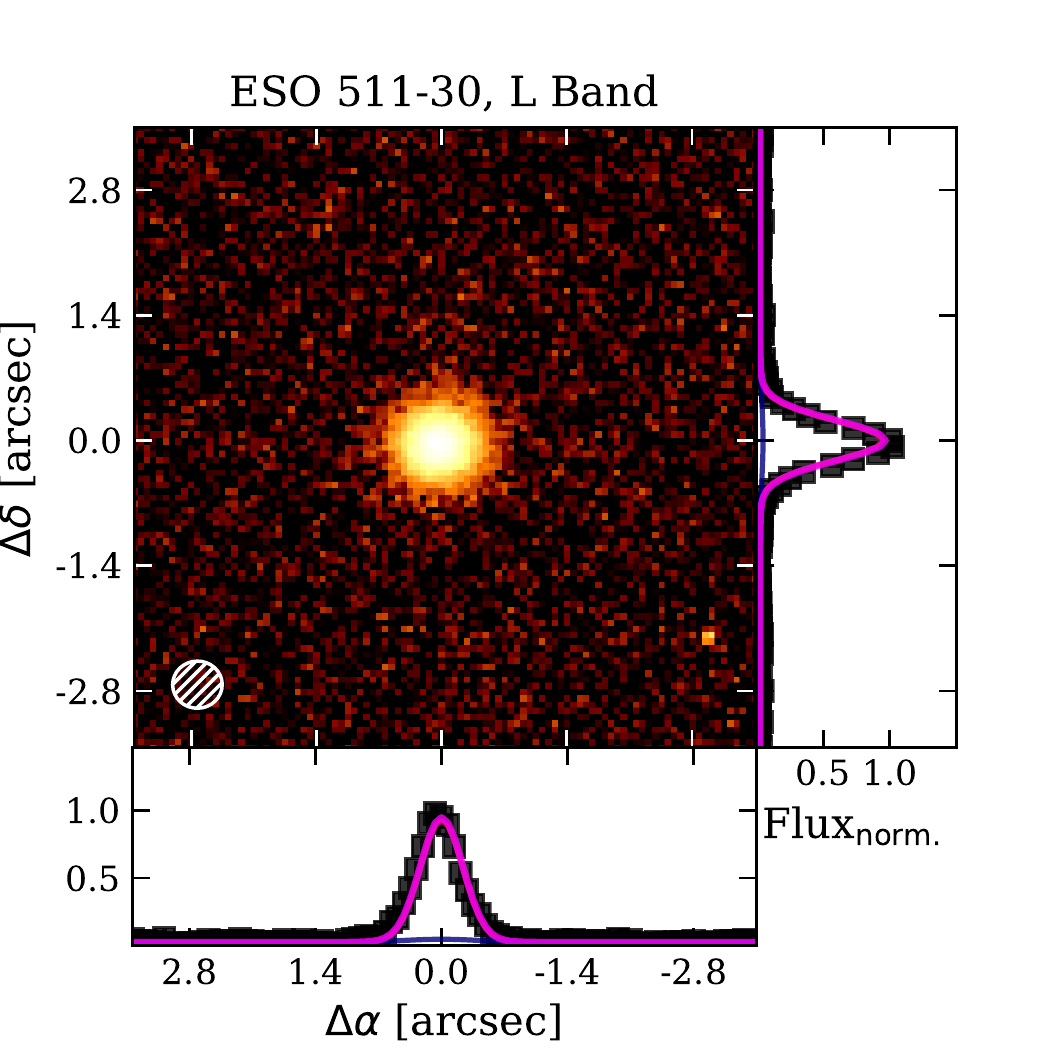}}
\subfloat{\includegraphics[width=0.25\hsize]{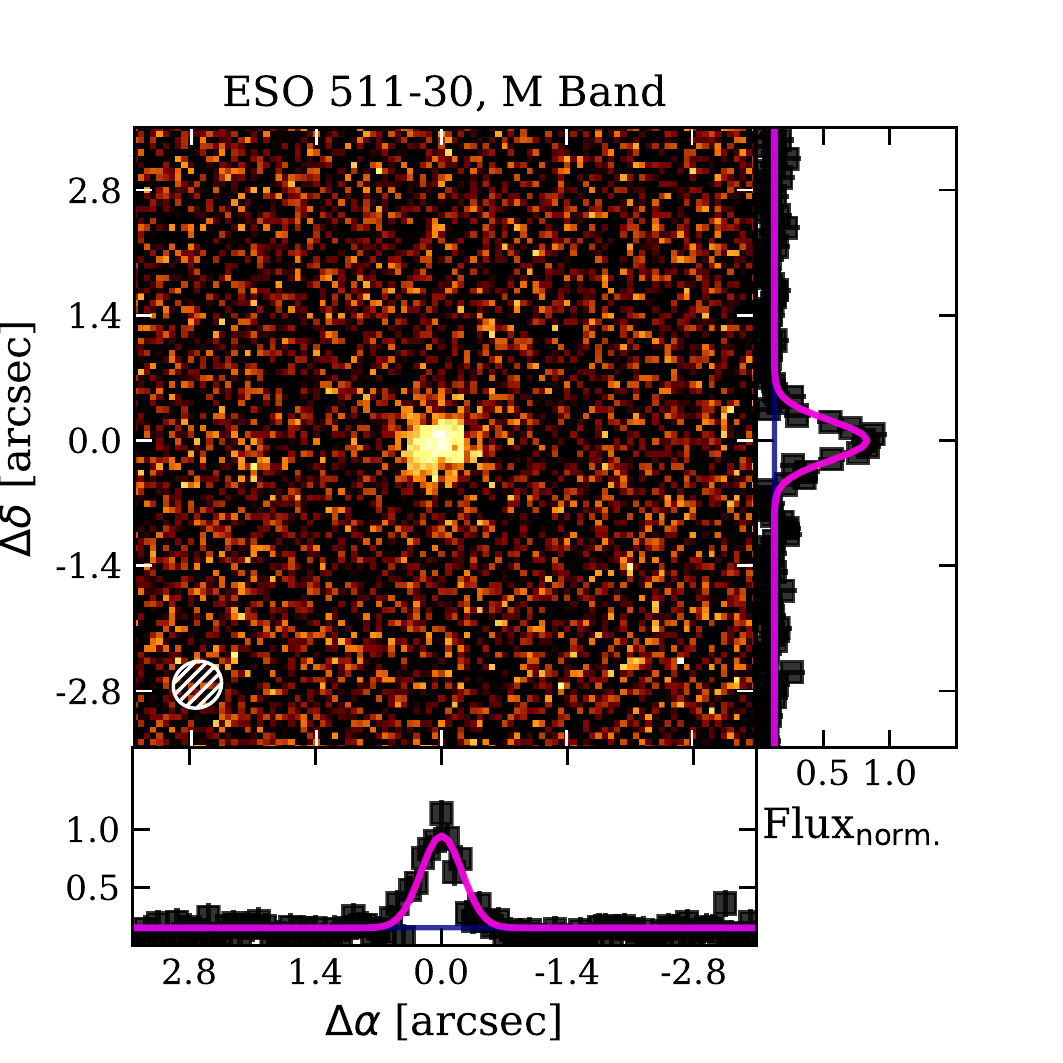}}
\subfloat{\includegraphics[width=0.25\hsize]{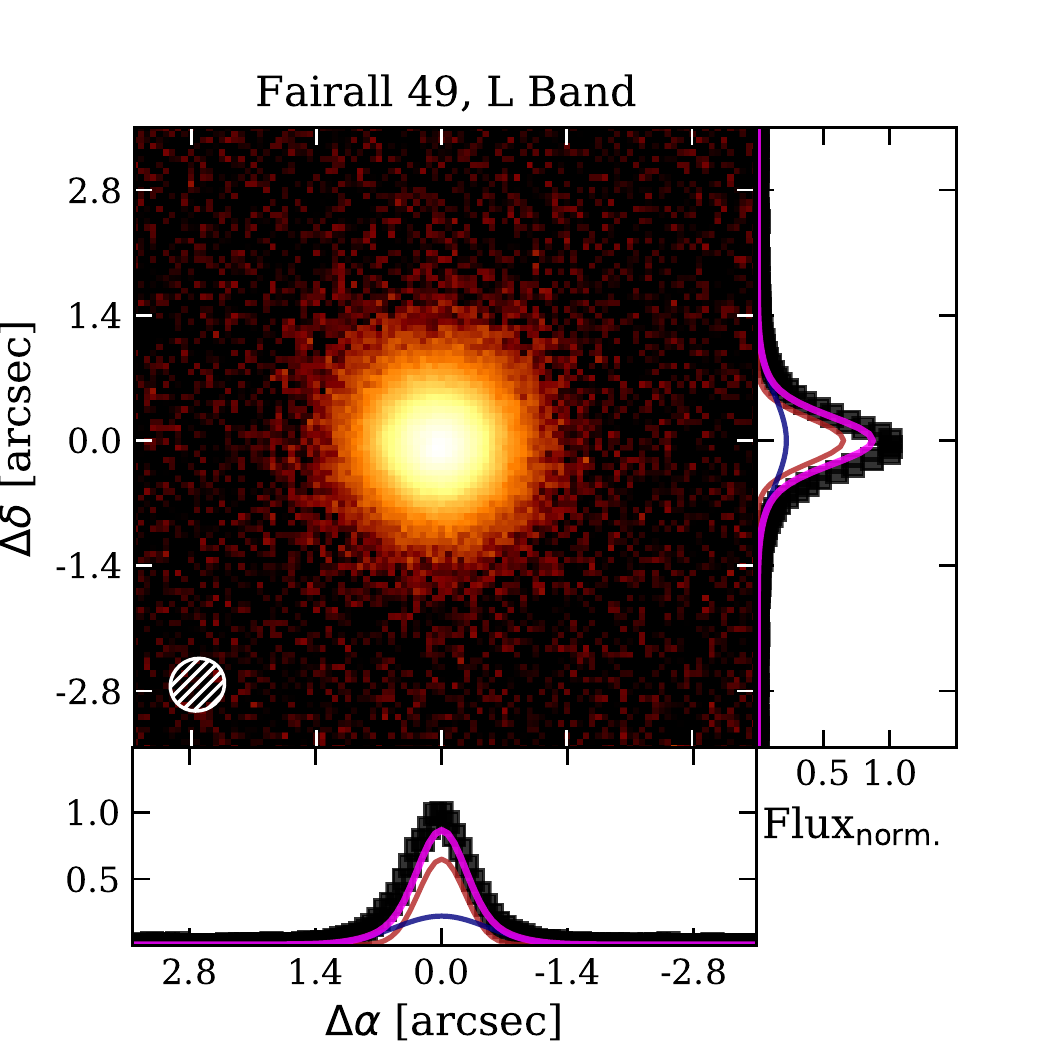}}
\subfloat{\includegraphics[width=0.25\hsize]{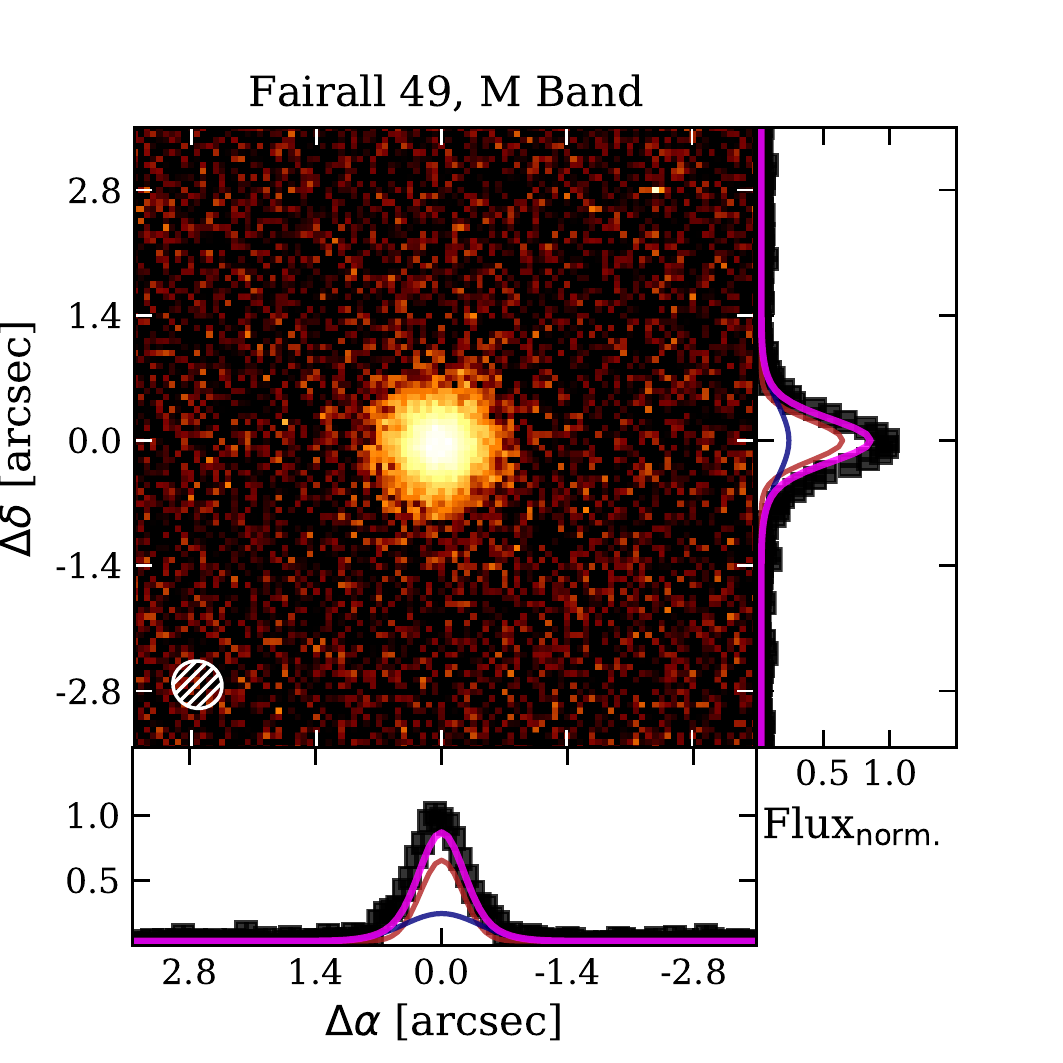}} \\
\caption{ As Fig \ref{fig:cutouts_one} but for all sources.}
\end{figure*}
\begin{figure*}
\subfloat{\includegraphics[width=0.25\hsize]{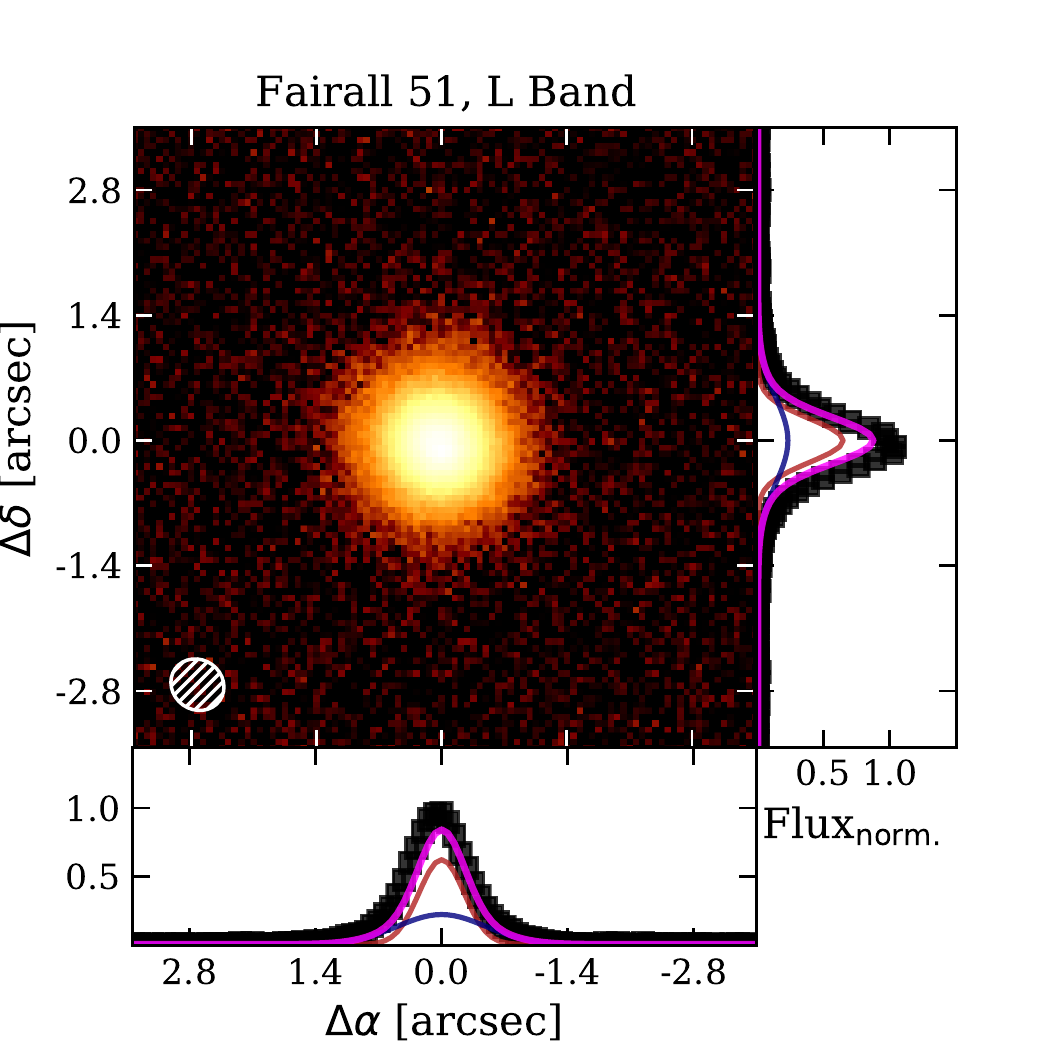}}
\subfloat{\includegraphics[width=0.25\hsize]{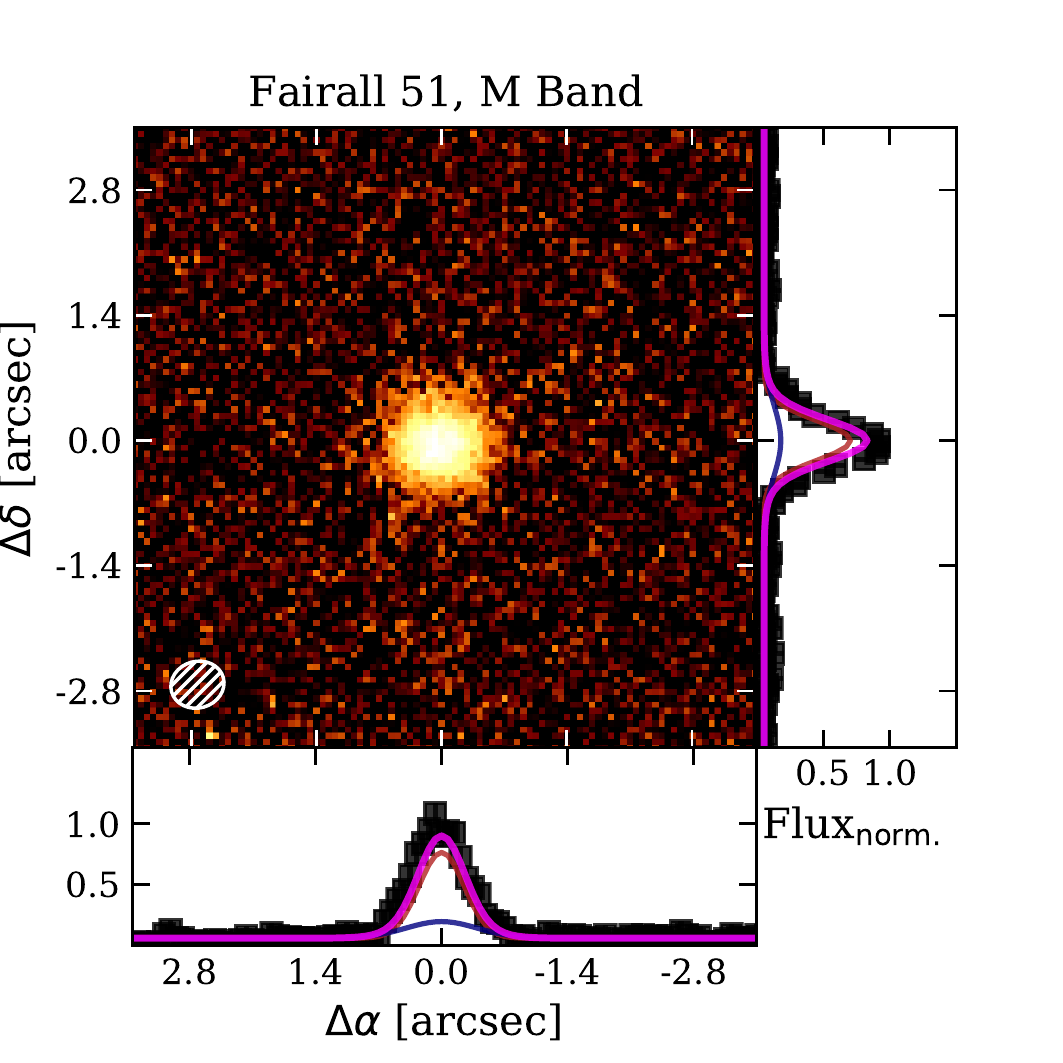}}
\subfloat{\includegraphics[width=0.25\hsize]{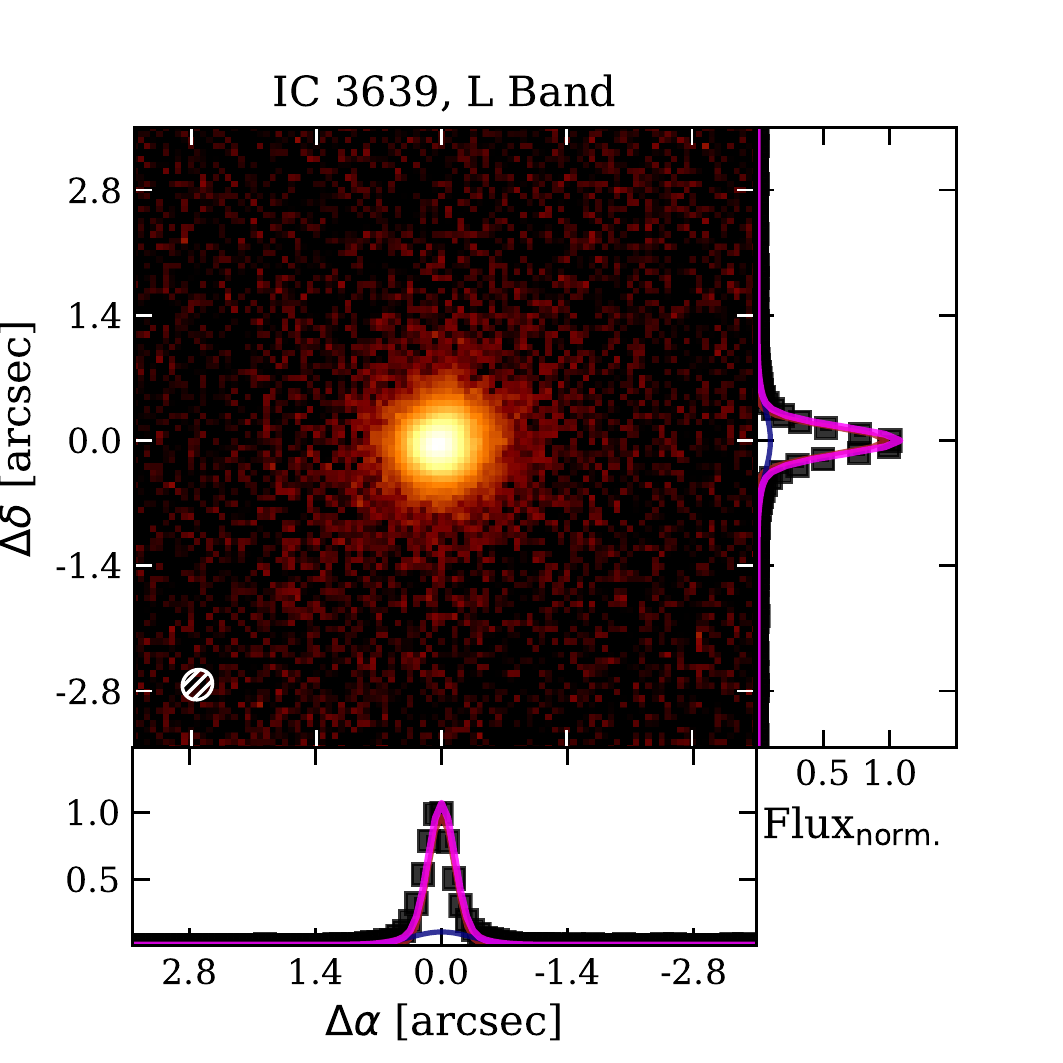}}
\subfloat{\includegraphics[width=0.25\hsize]{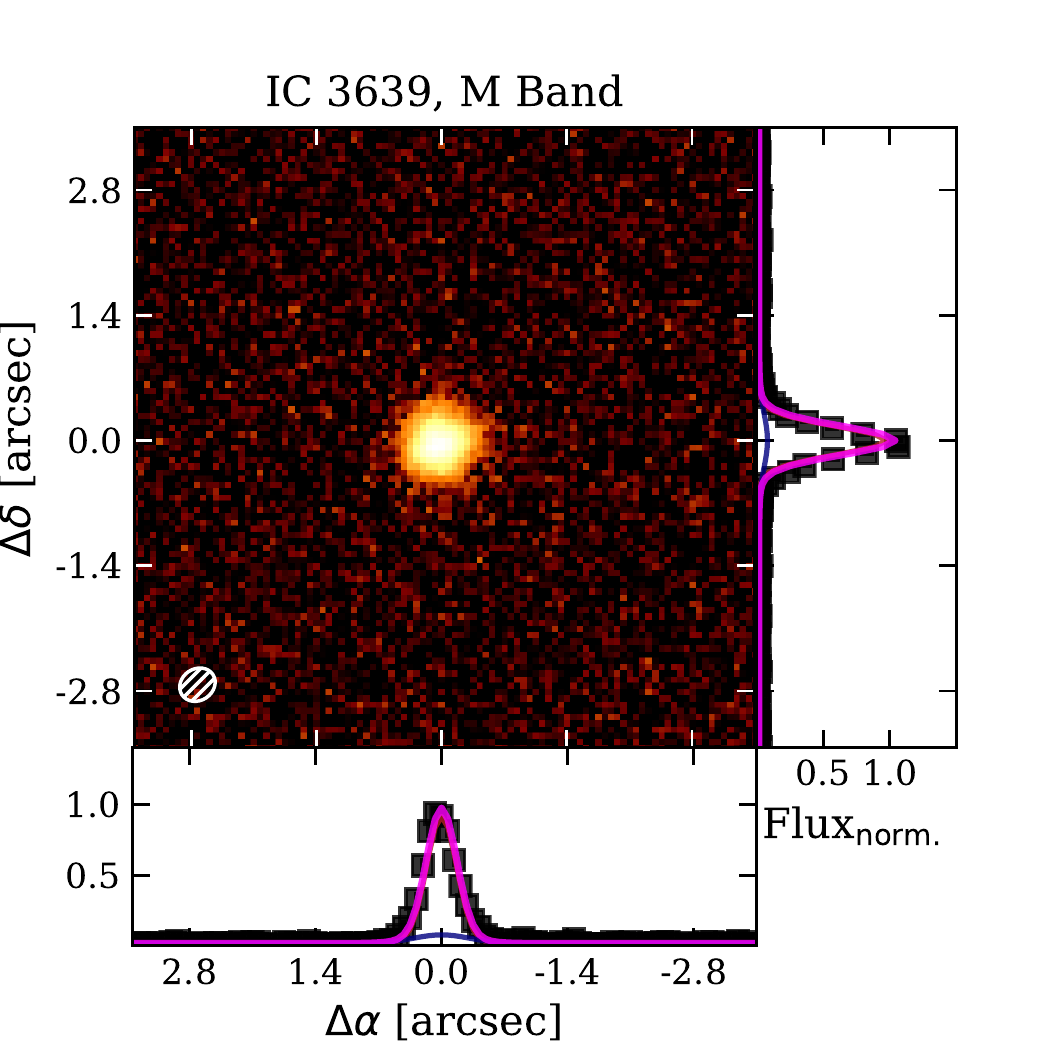}} \\
\subfloat{\includegraphics[width=0.25\hsize]{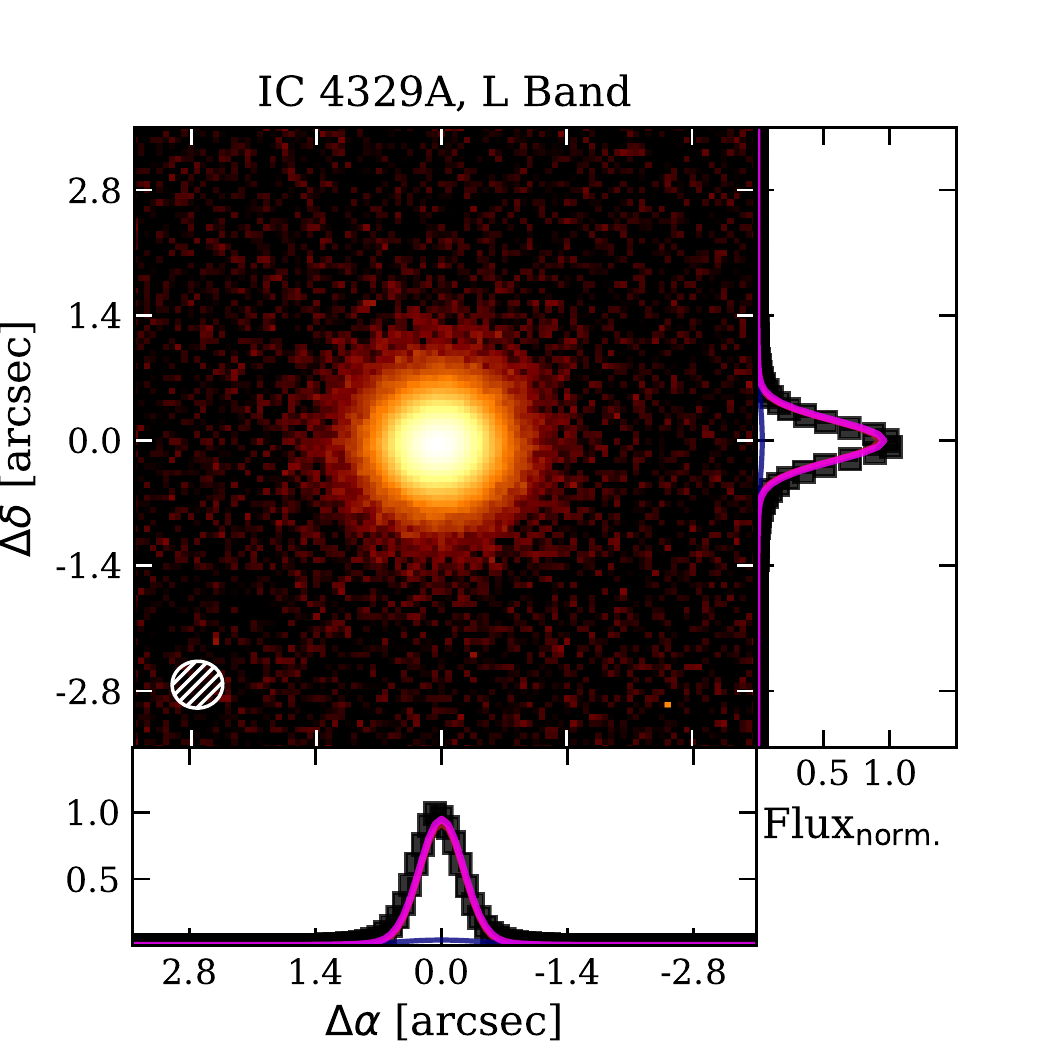}}
\subfloat{\includegraphics[width=0.25\hsize]{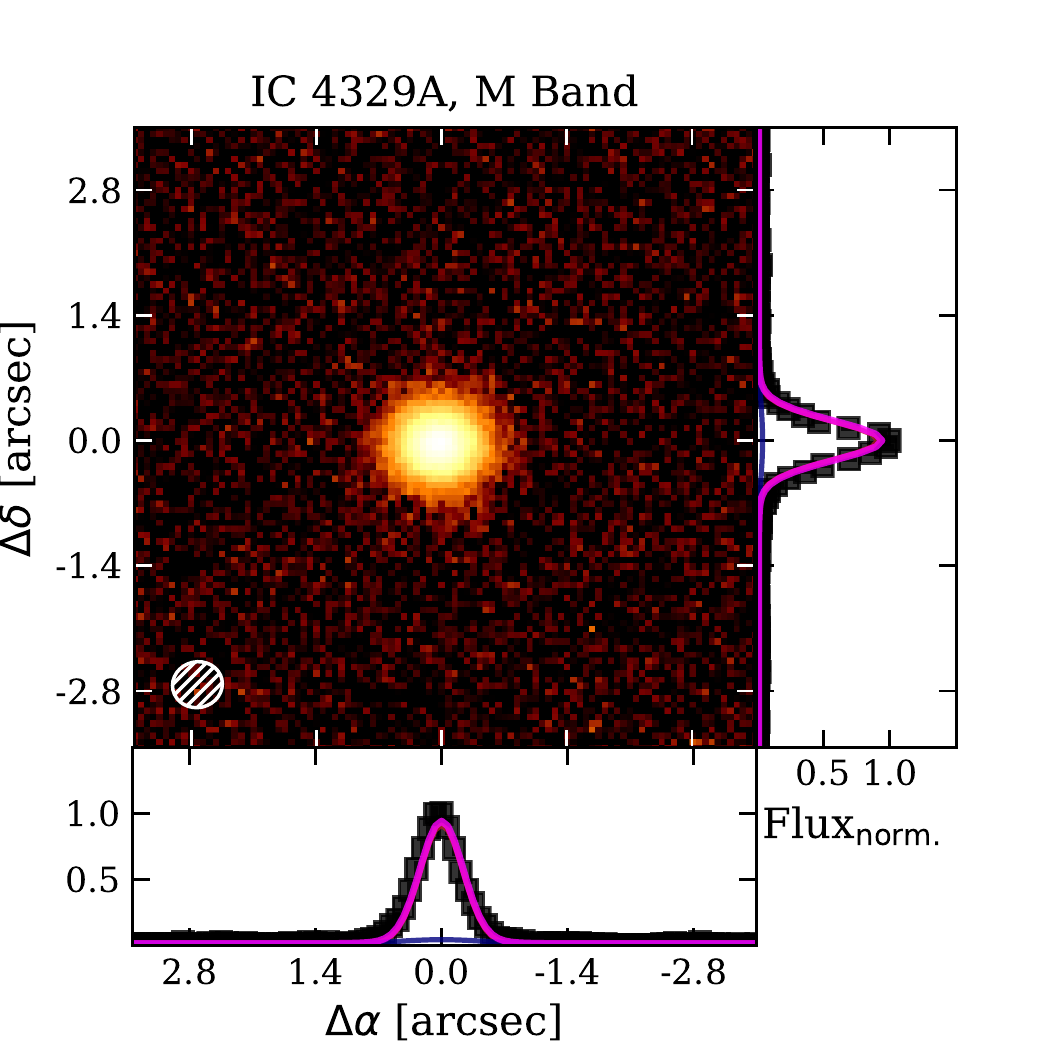}}
\subfloat{\includegraphics[width=0.25\hsize]{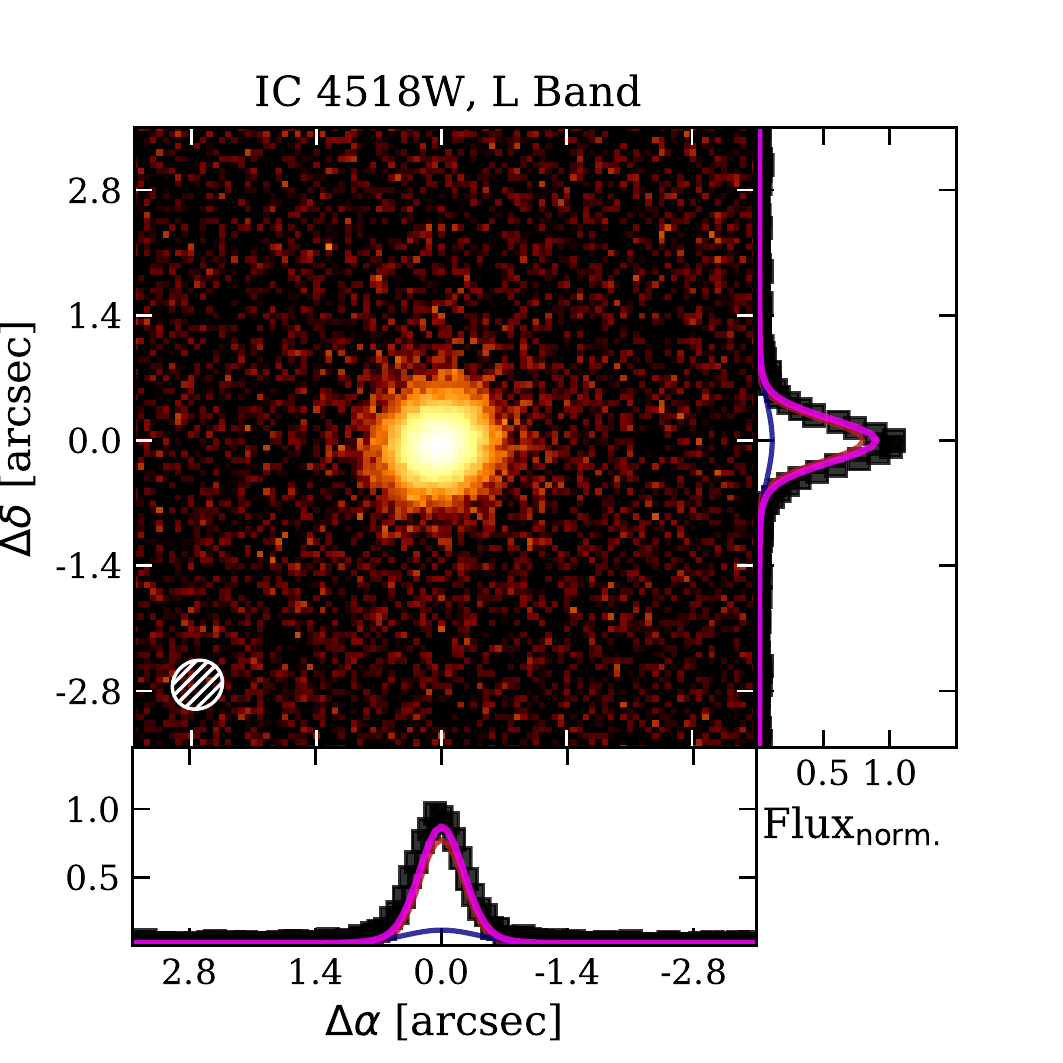}}
\subfloat{\includegraphics[width=0.25\hsize]{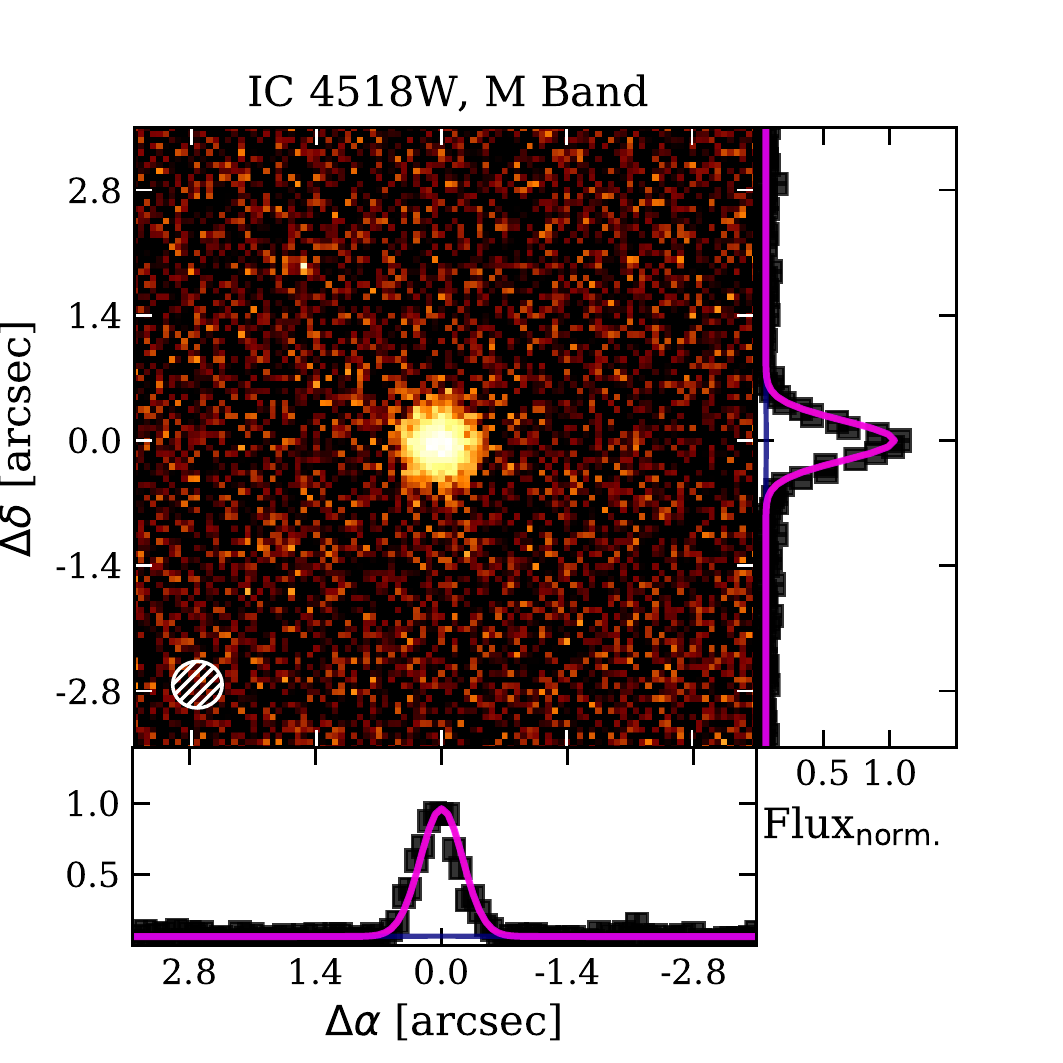}}\\
\subfloat{\includegraphics[width=0.25\hsize]{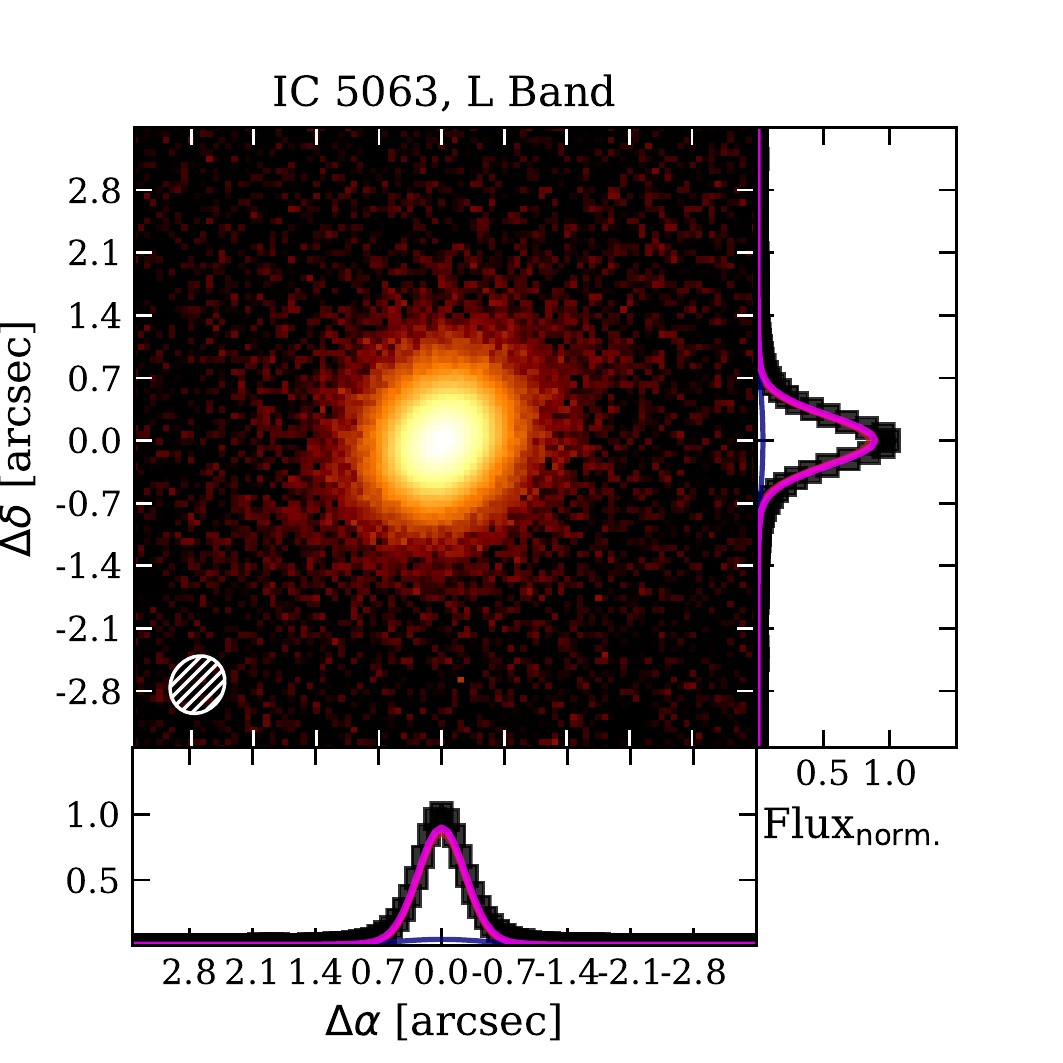}}
\subfloat{\includegraphics[width=0.25\hsize]{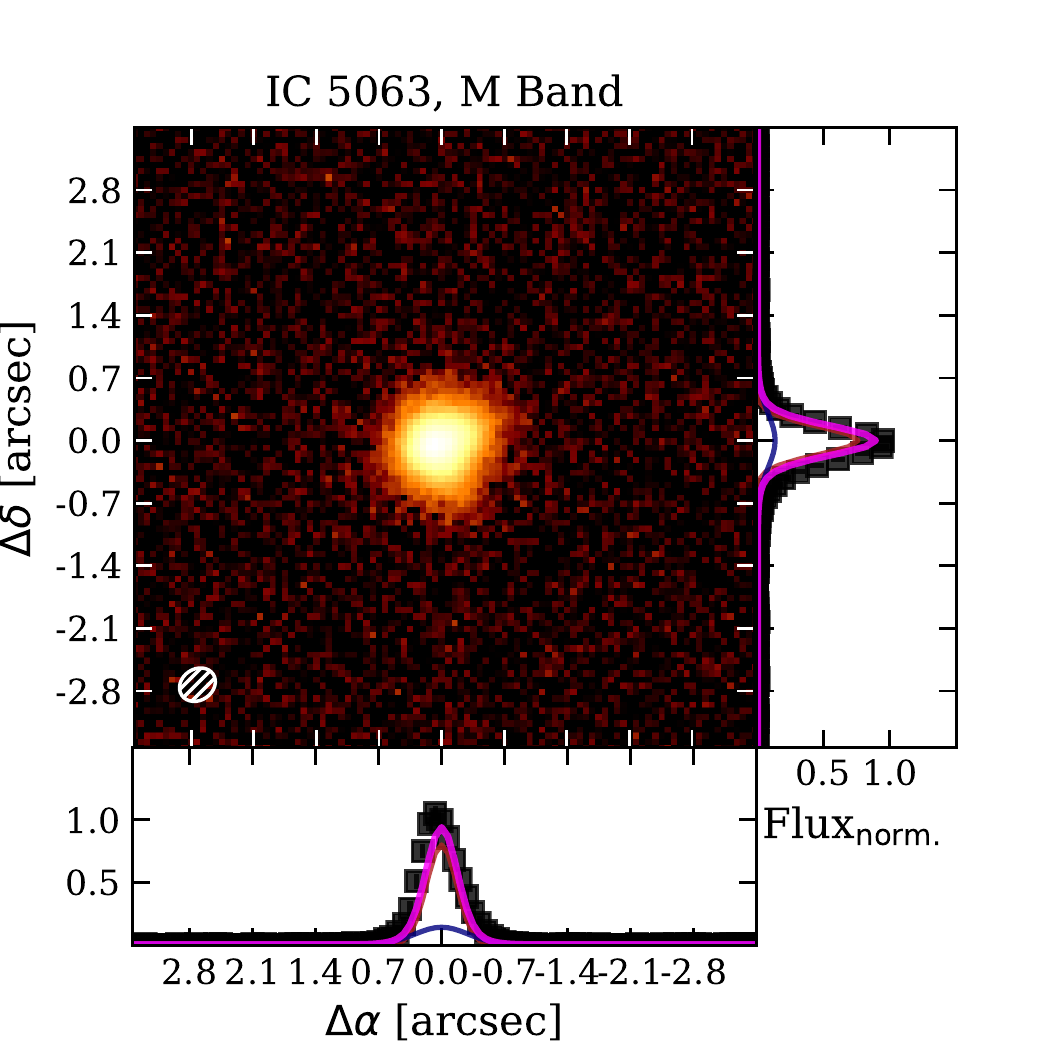}}
\subfloat{\includegraphics[width=0.25\hsize]{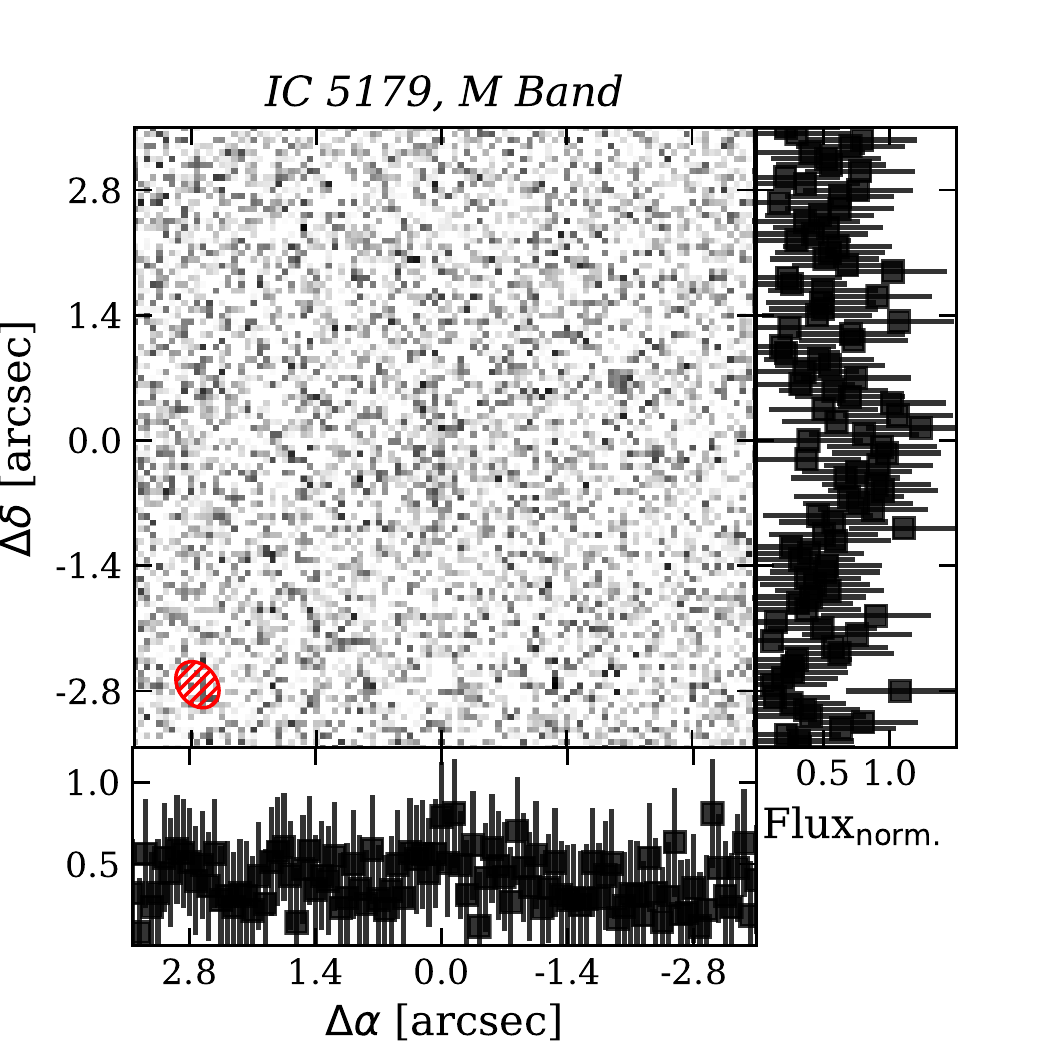}}
\subfloat{\includegraphics[width=0.25\hsize]{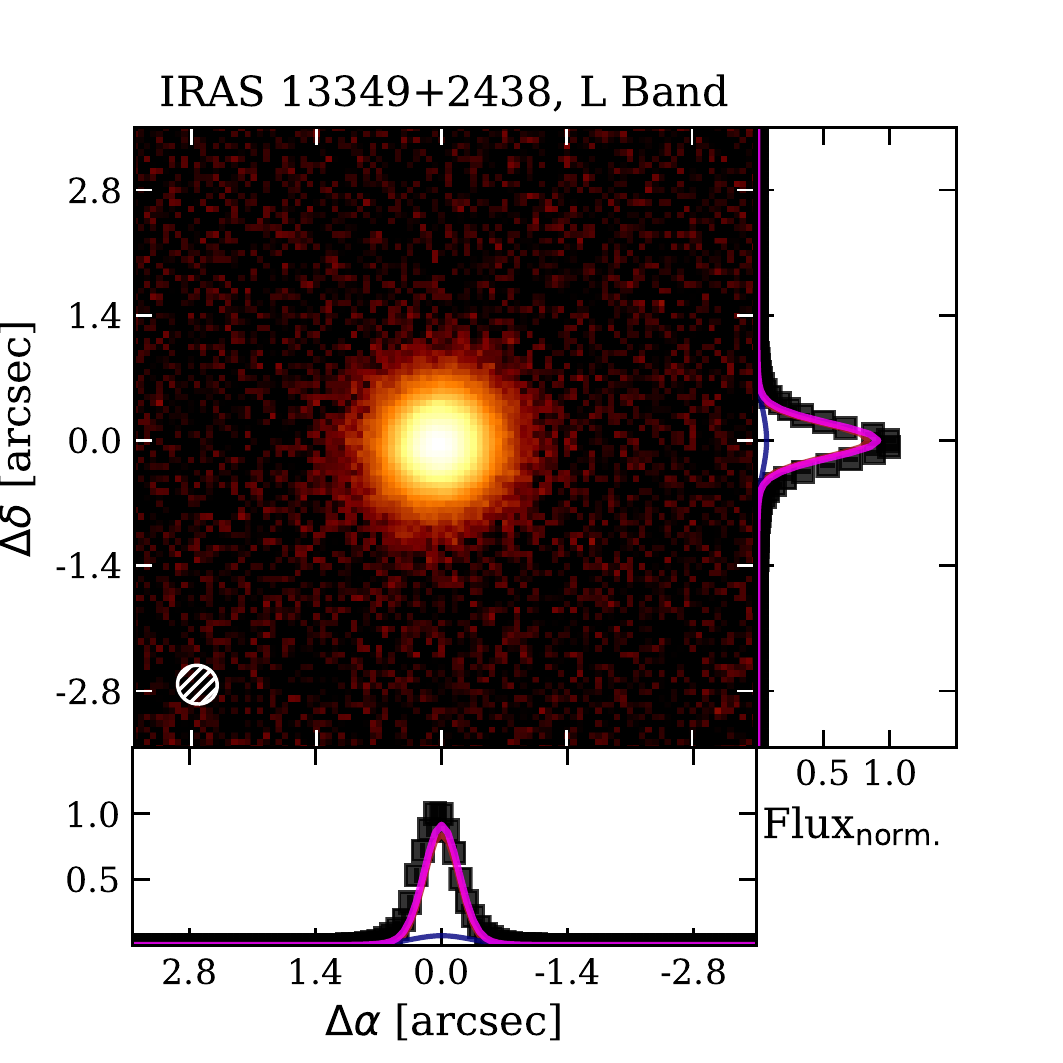}}\\
\subfloat{\includegraphics[width=0.25\hsize]{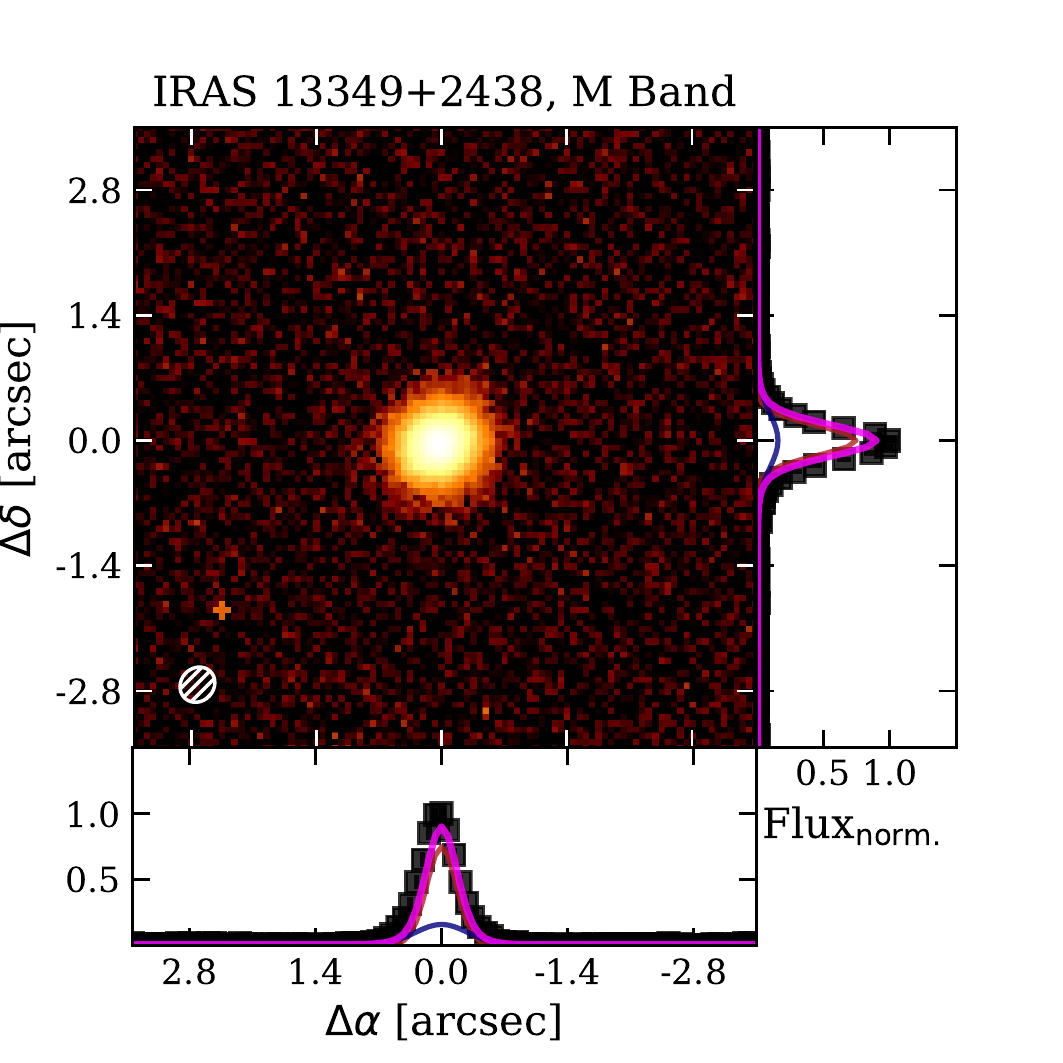}}
\subfloat{\includegraphics[width=0.25\hsize]{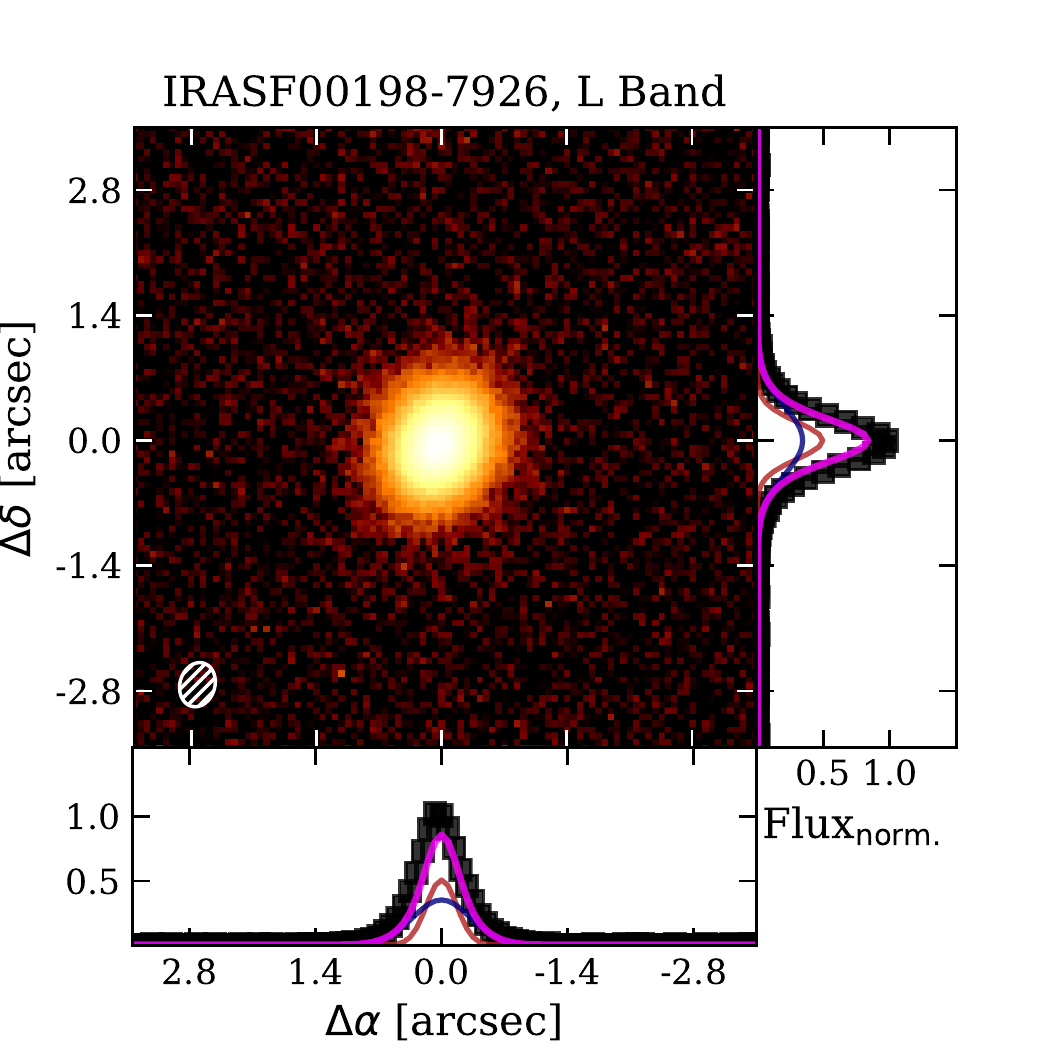}} 
\subfloat{\includegraphics[width=0.25\hsize]{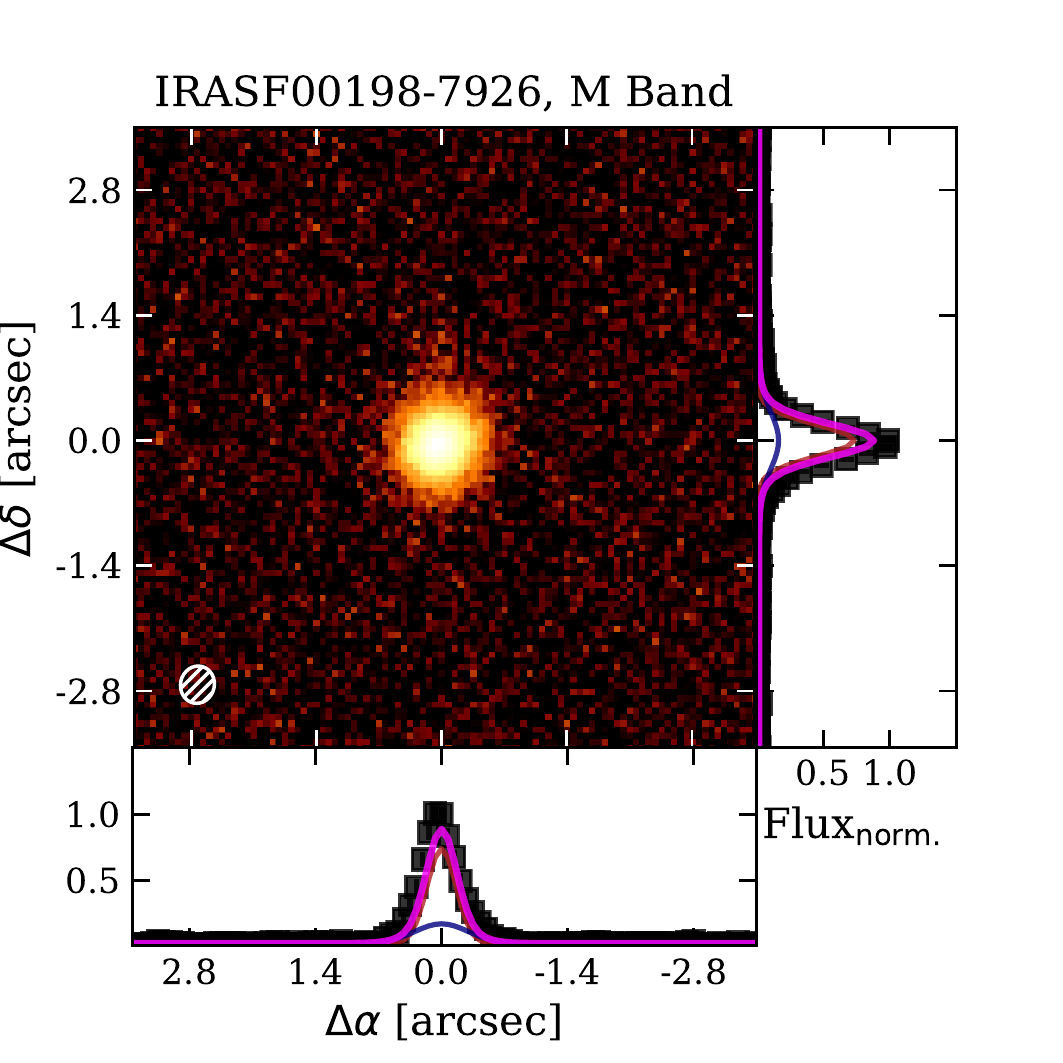}}
\subfloat{\includegraphics[width=0.25\hsize]{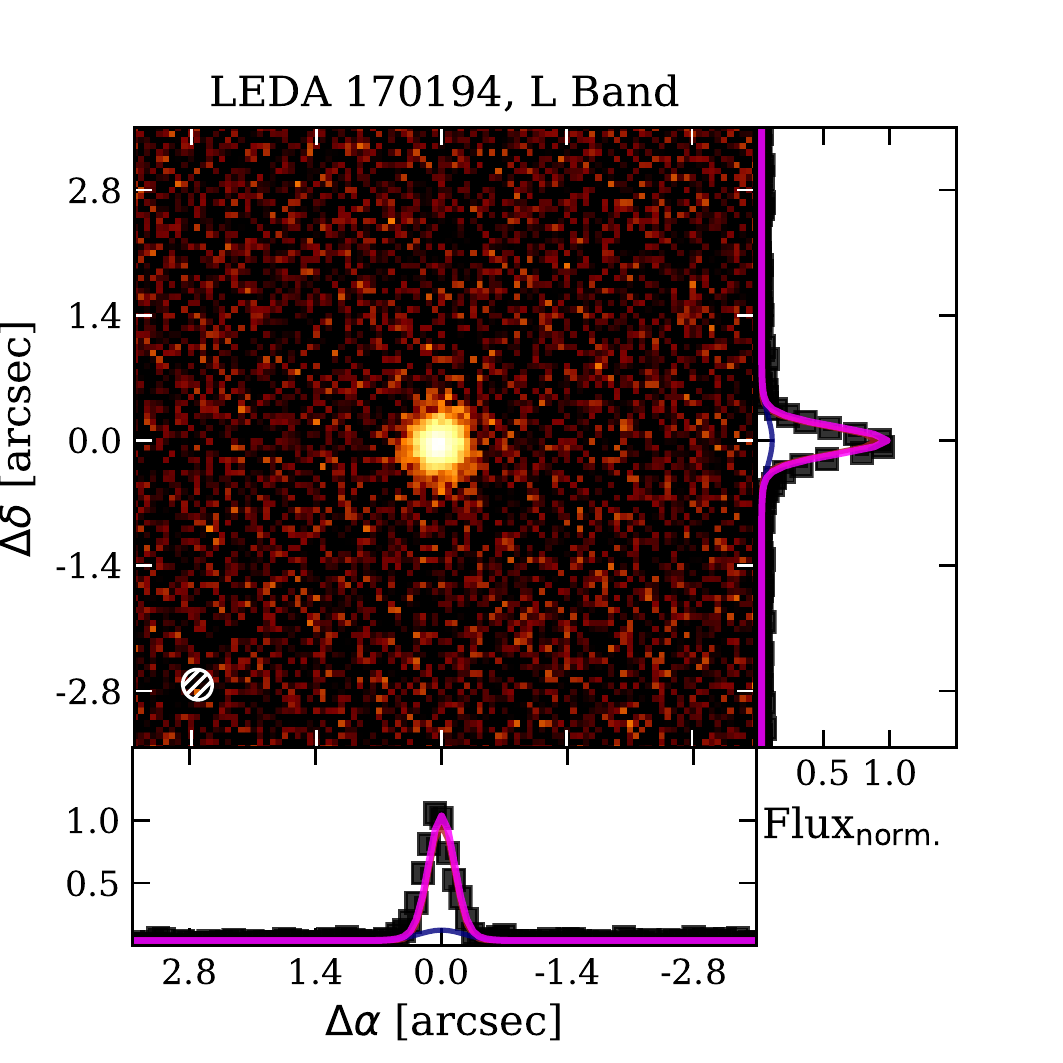}}\\
\subfloat{\includegraphics[width=0.25\hsize]{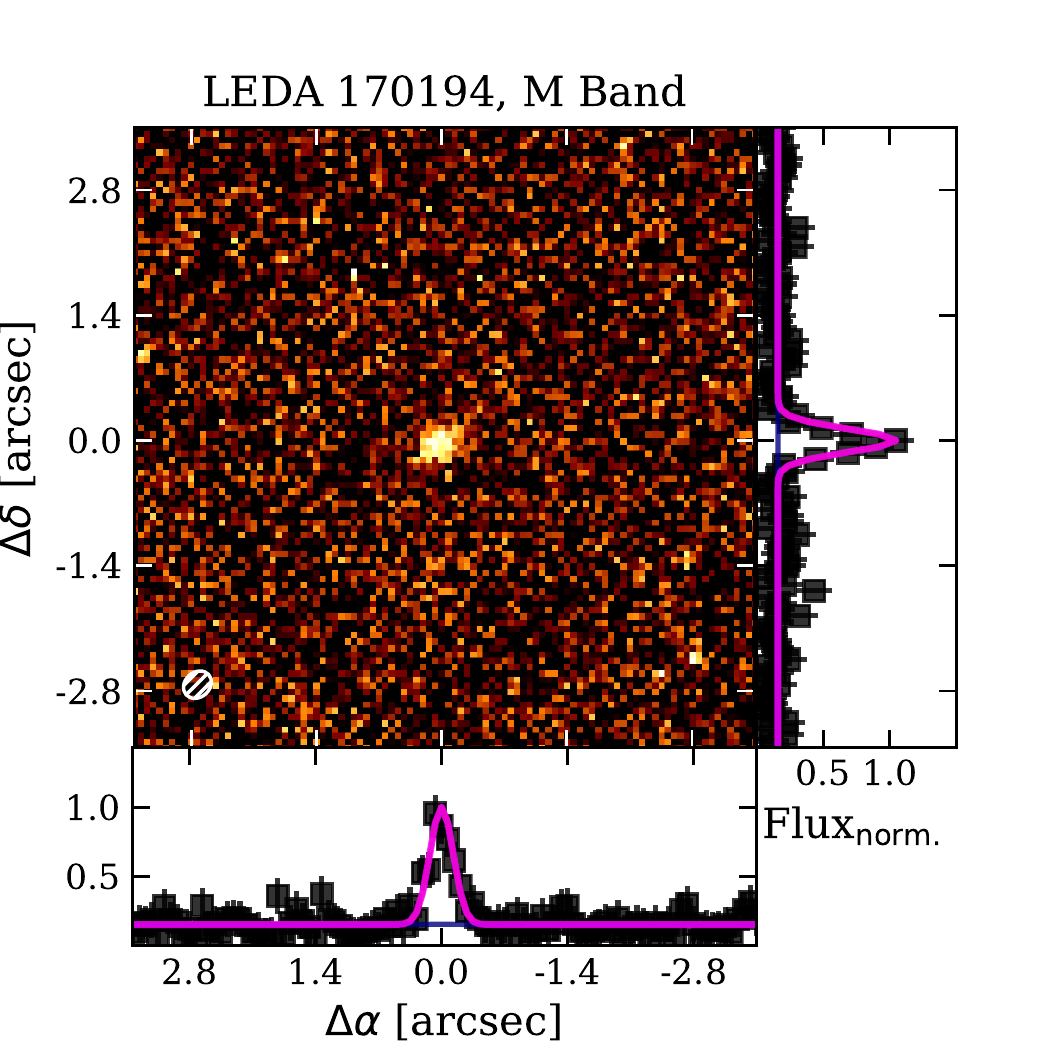}}
\subfloat{\includegraphics[width=0.25\hsize]{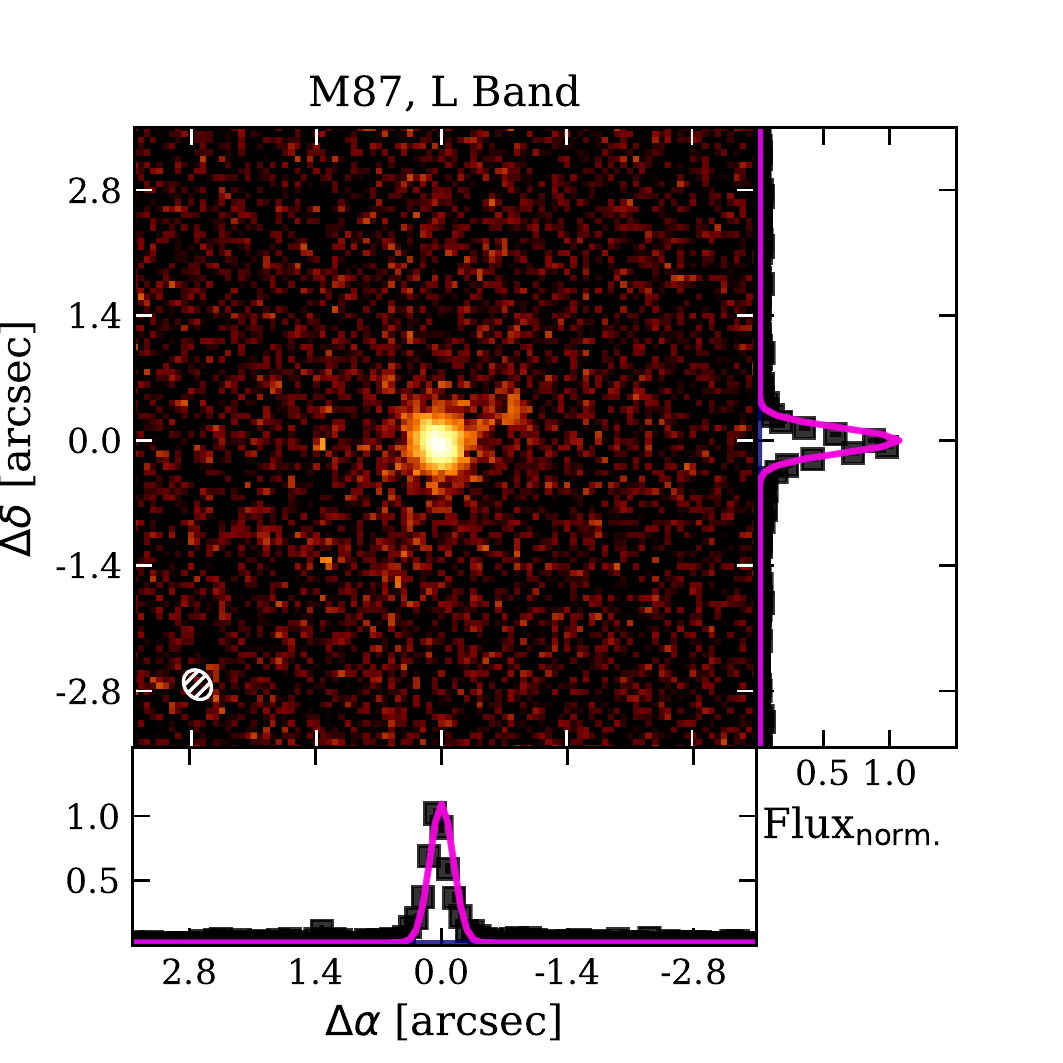}} 
\subfloat{\includegraphics[width=0.25\hsize]{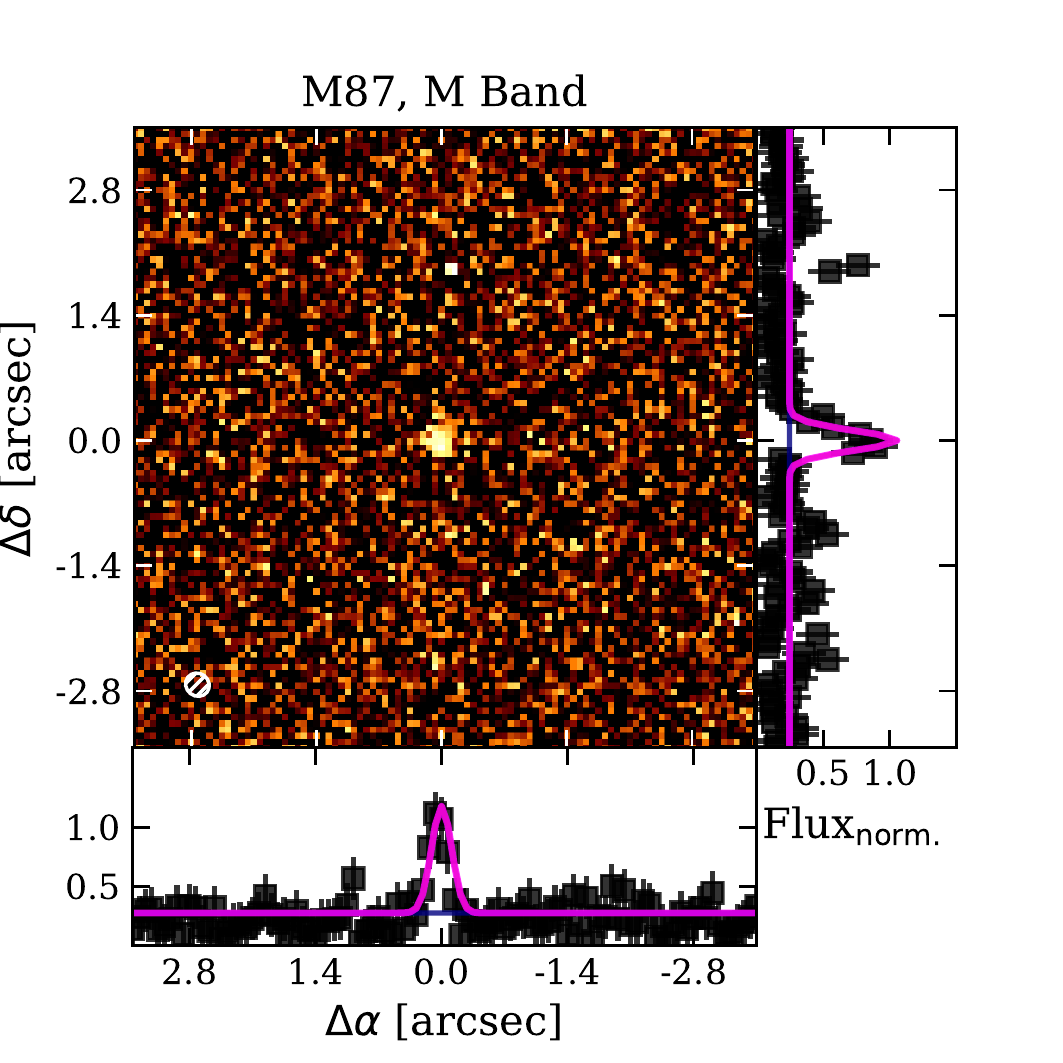}}
\subfloat{\includegraphics[width=0.25\hsize]{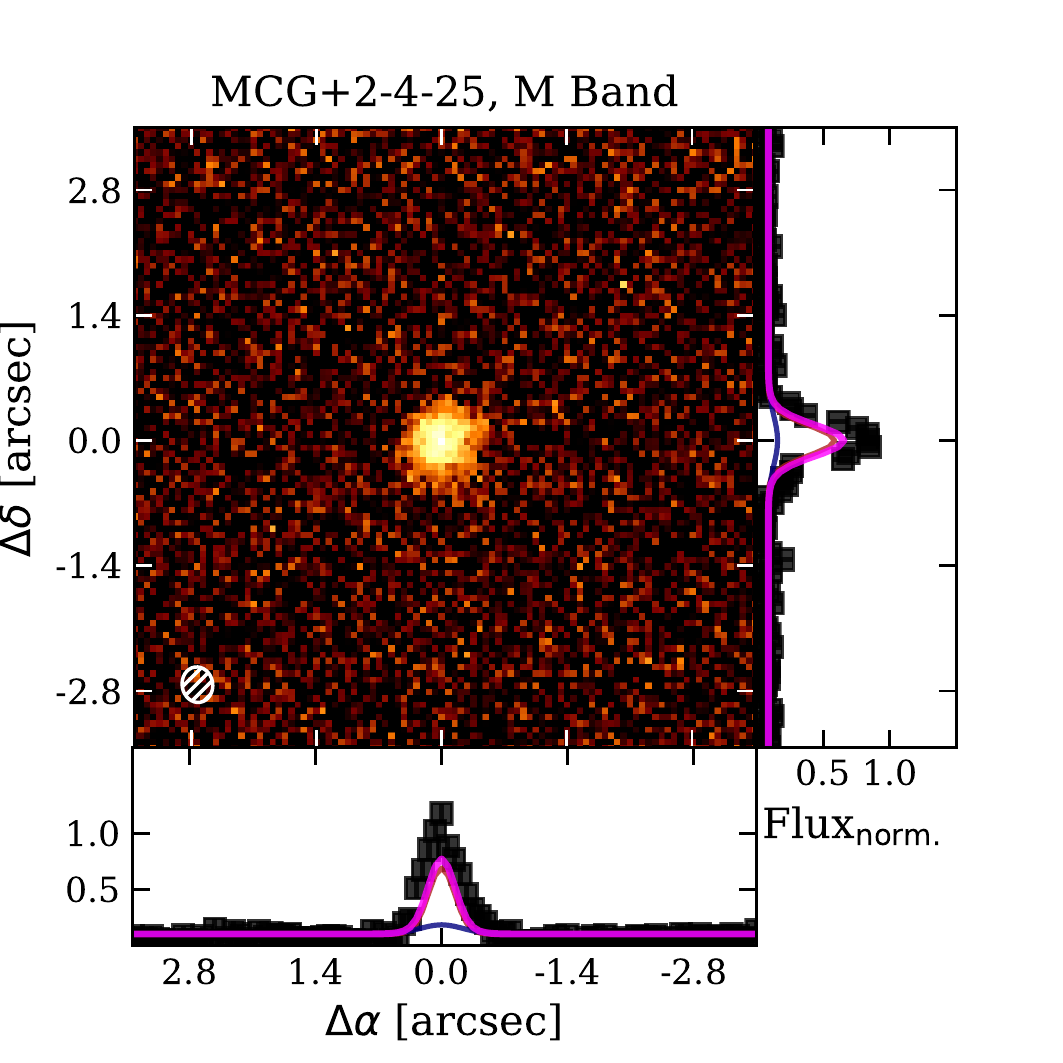}} \\
\caption{ As Fig \ref{fig:cutouts_one} but for all sources.}
\end{figure*}
\begin{figure*}
\subfloat{\includegraphics[width=0.25\hsize]{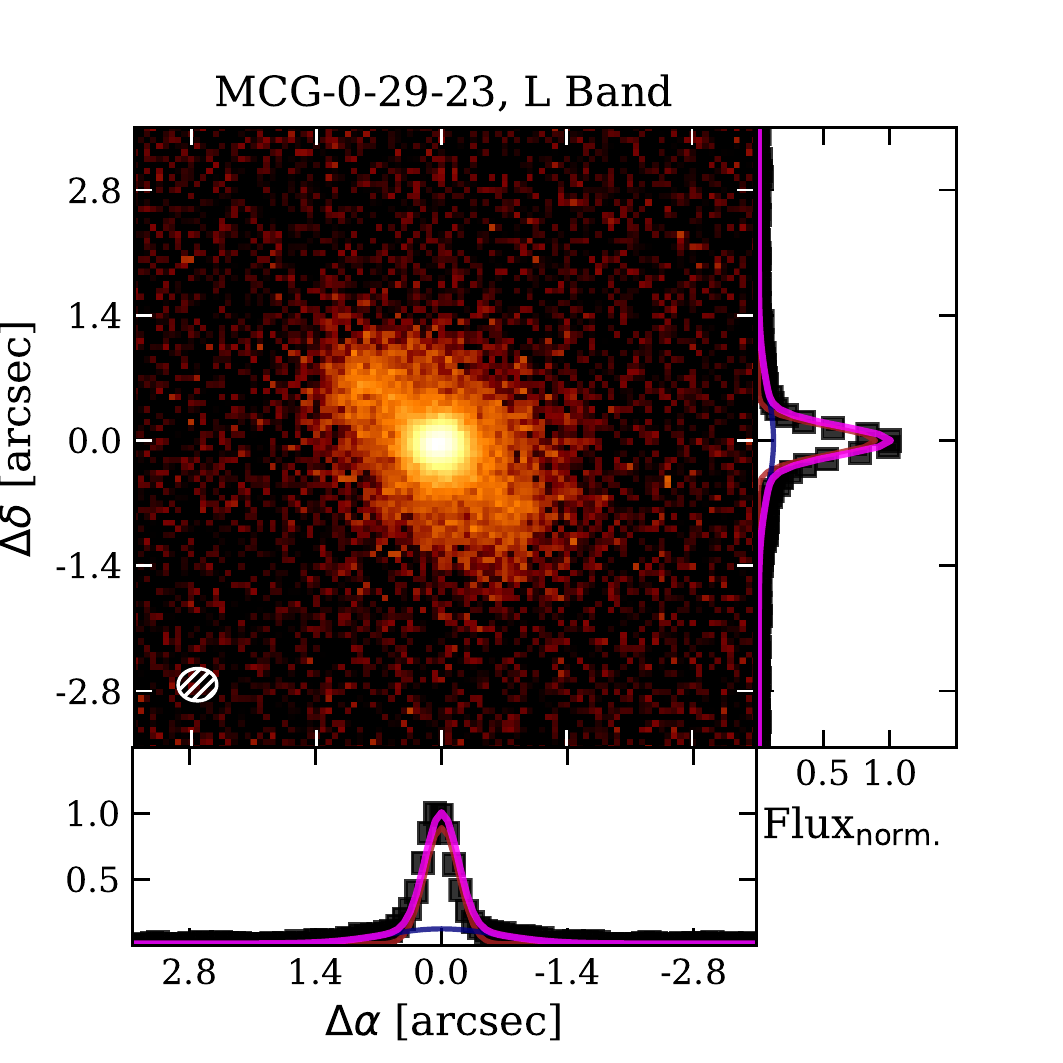}}
\subfloat{\includegraphics[width=0.25\hsize]{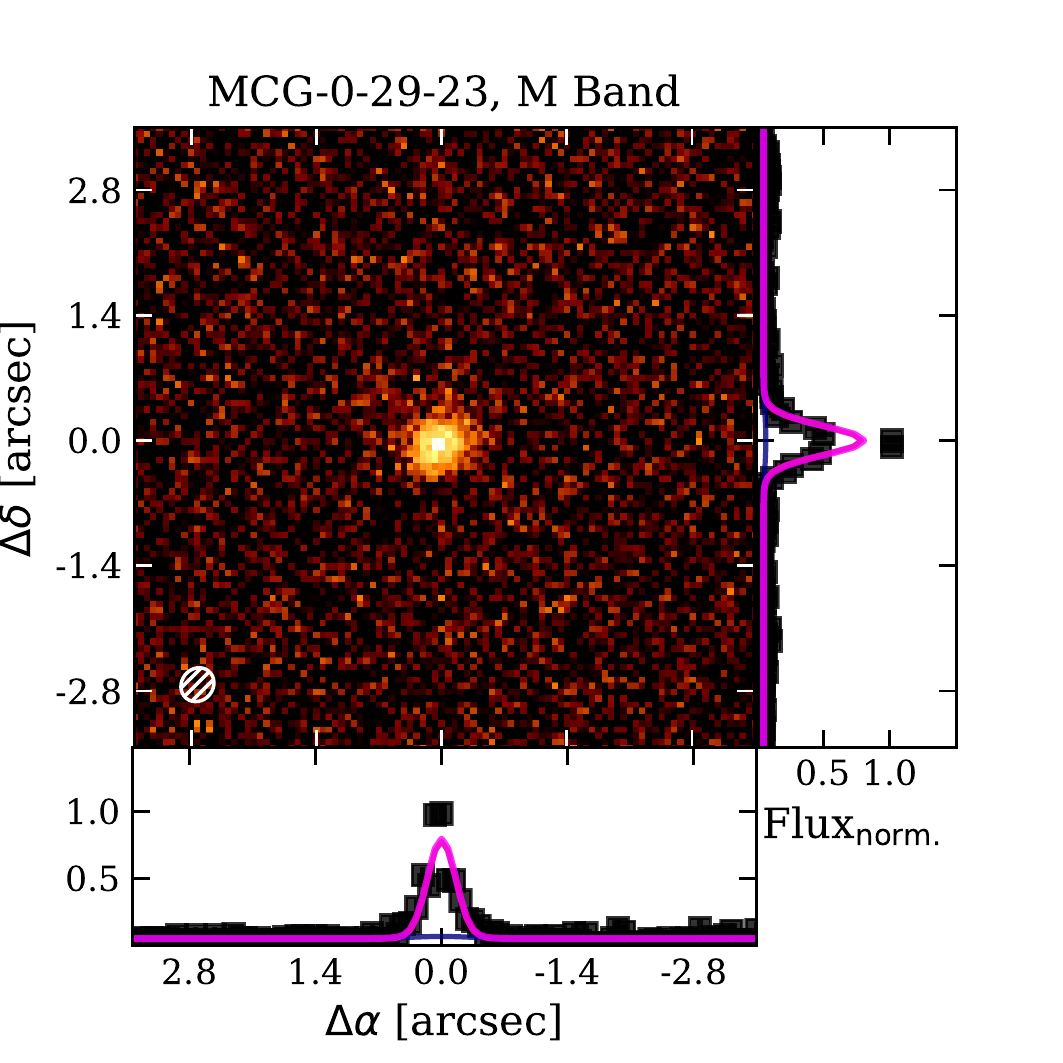}} 
\subfloat{\includegraphics[width=0.25\hsize]{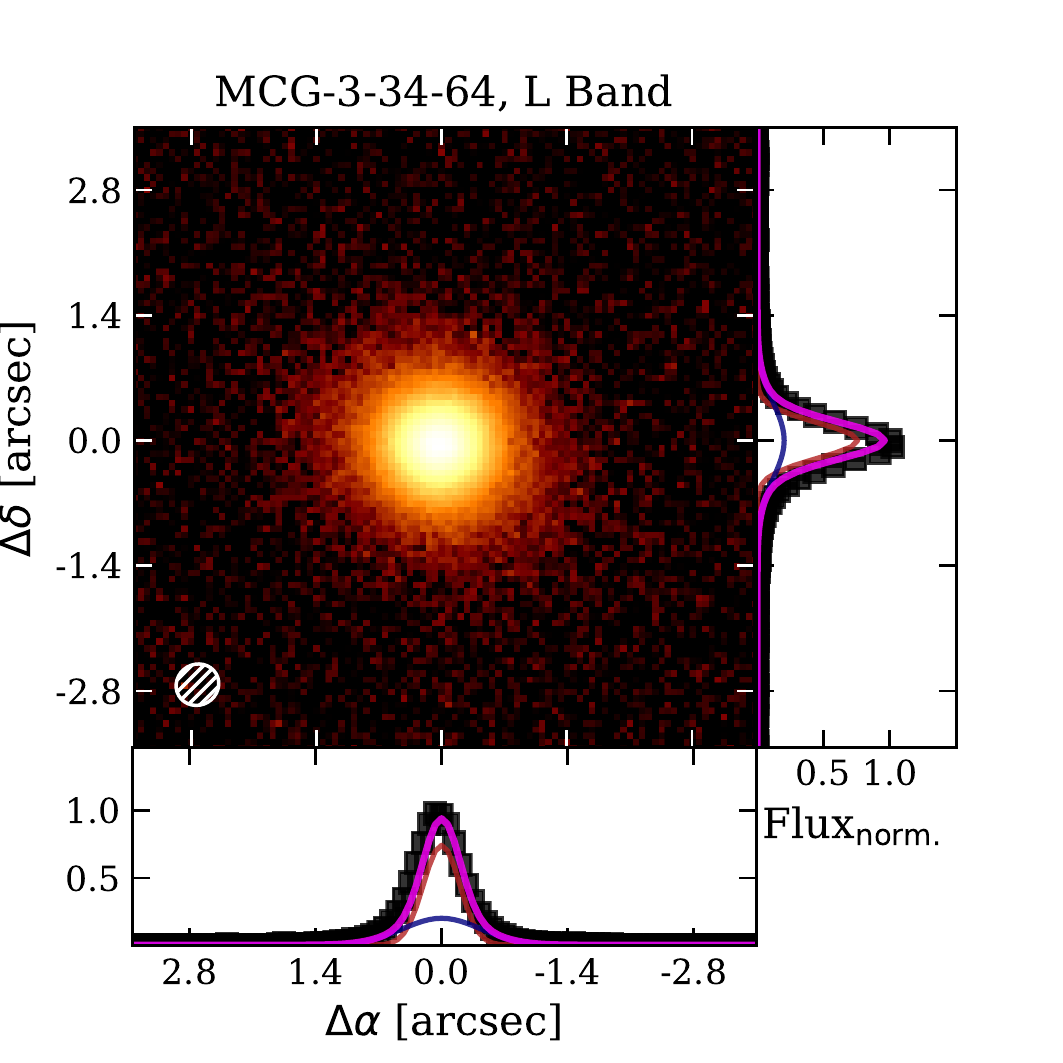}}
\subfloat{\includegraphics[width=0.25\hsize]{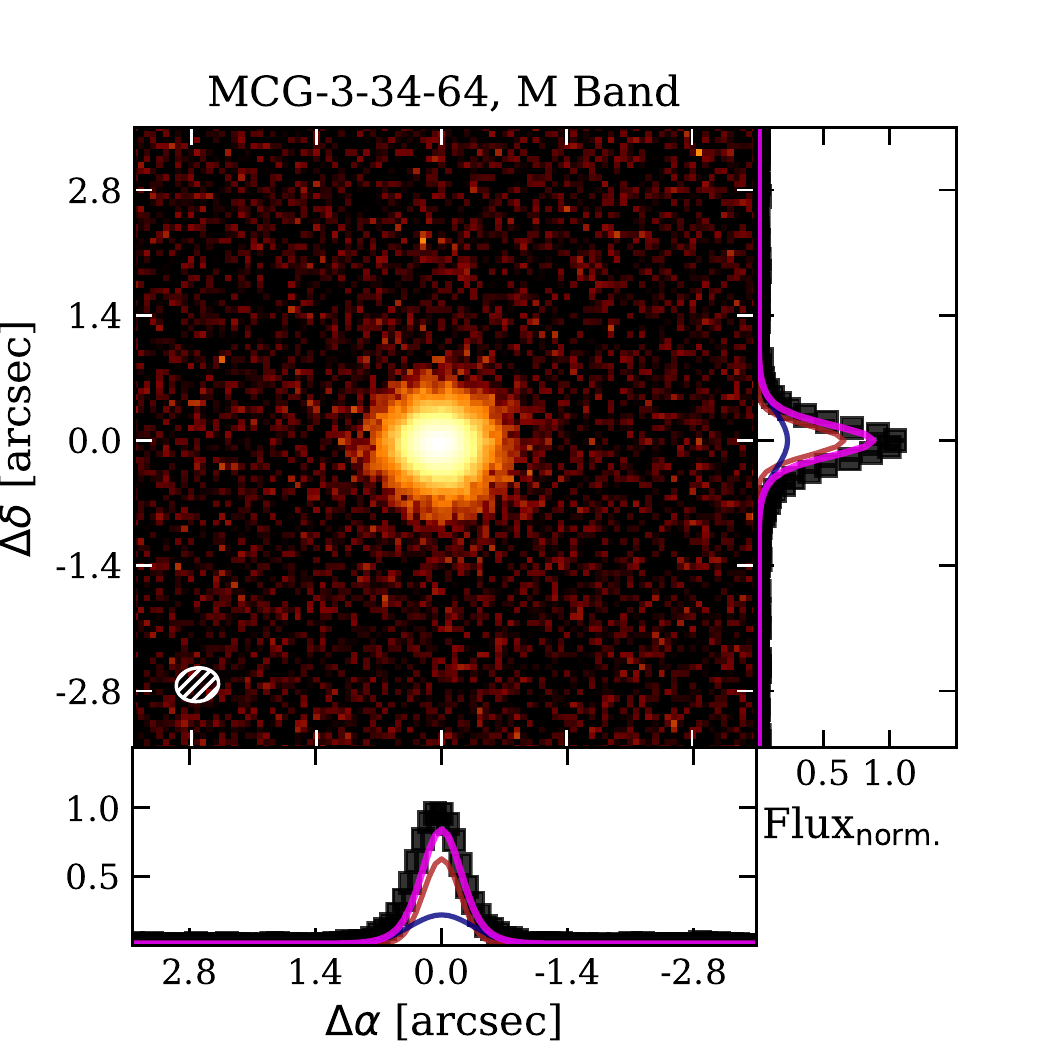}} \\
\subfloat{\includegraphics[width=0.25\hsize]{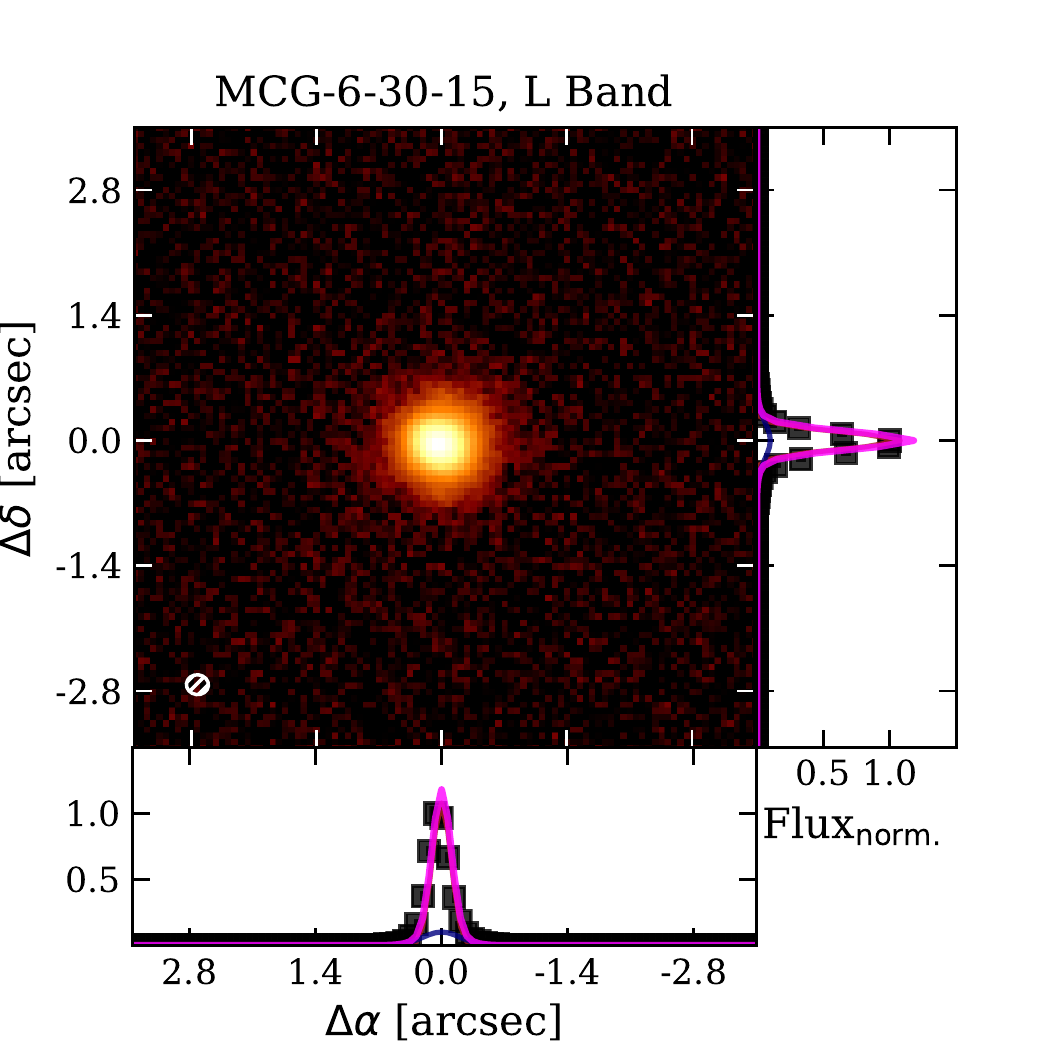}}
\subfloat{\includegraphics[width=0.25\hsize]{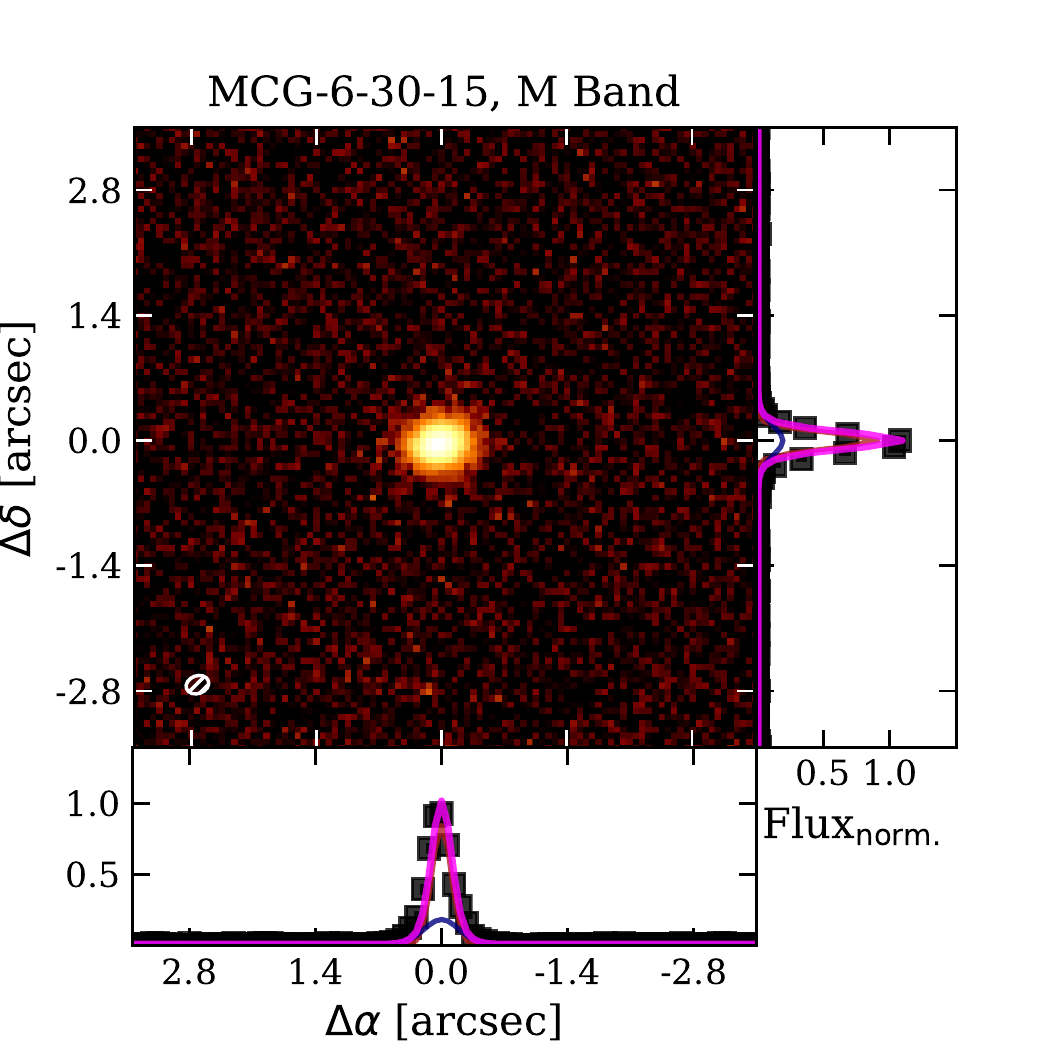}} 
\subfloat{\includegraphics[width=0.25\hsize]{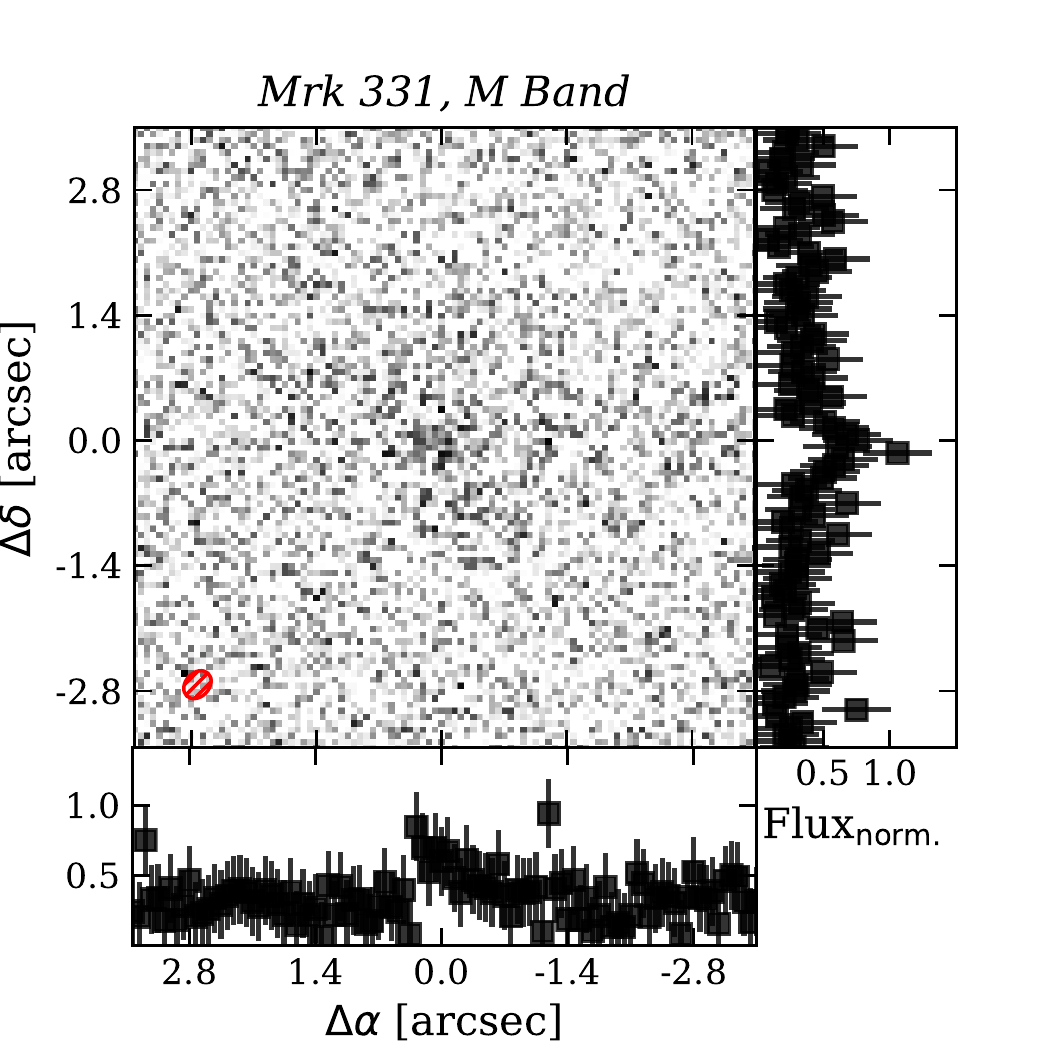}}
\subfloat{\includegraphics[width=0.25\hsize]{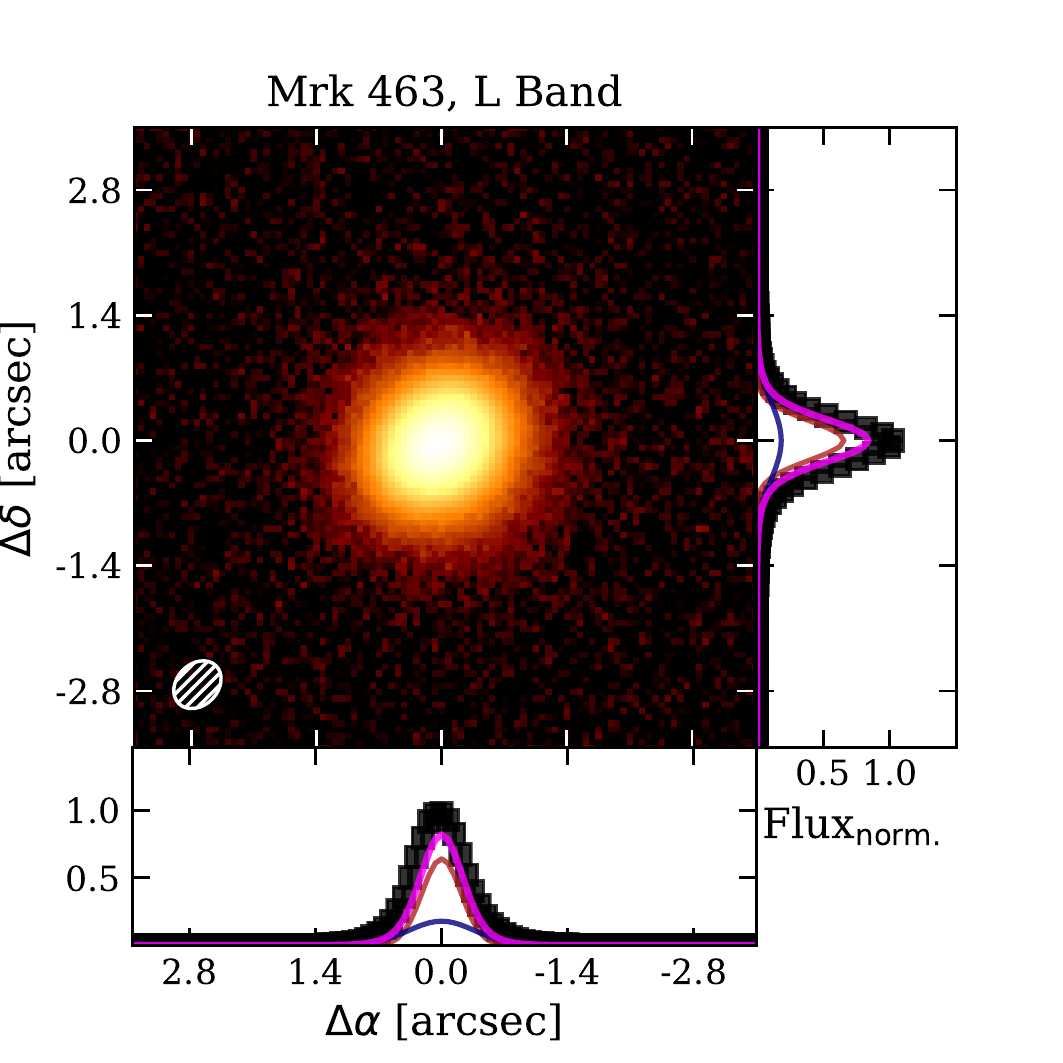}}\\
\subfloat{\includegraphics[width=0.25\hsize]{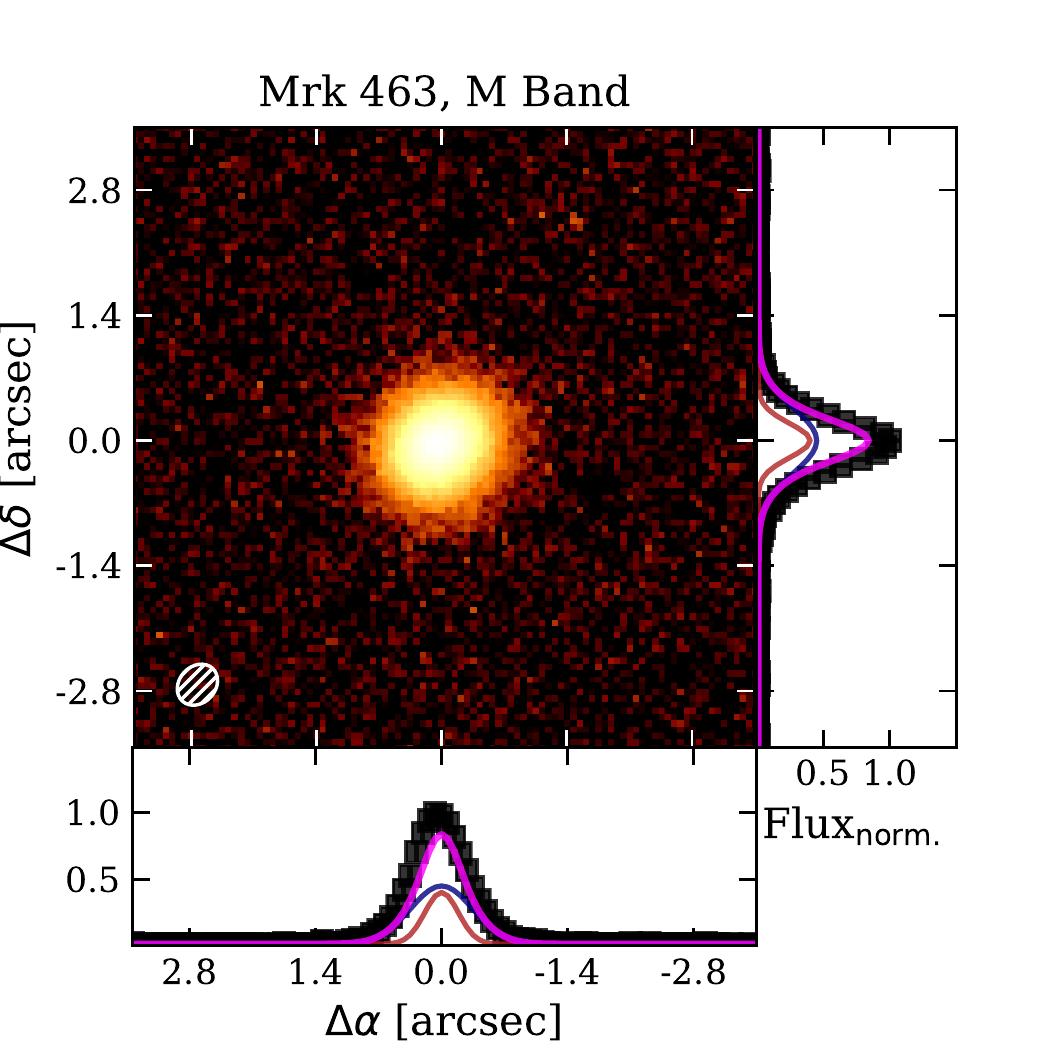}}
\subfloat{\includegraphics[width=0.25\hsize]{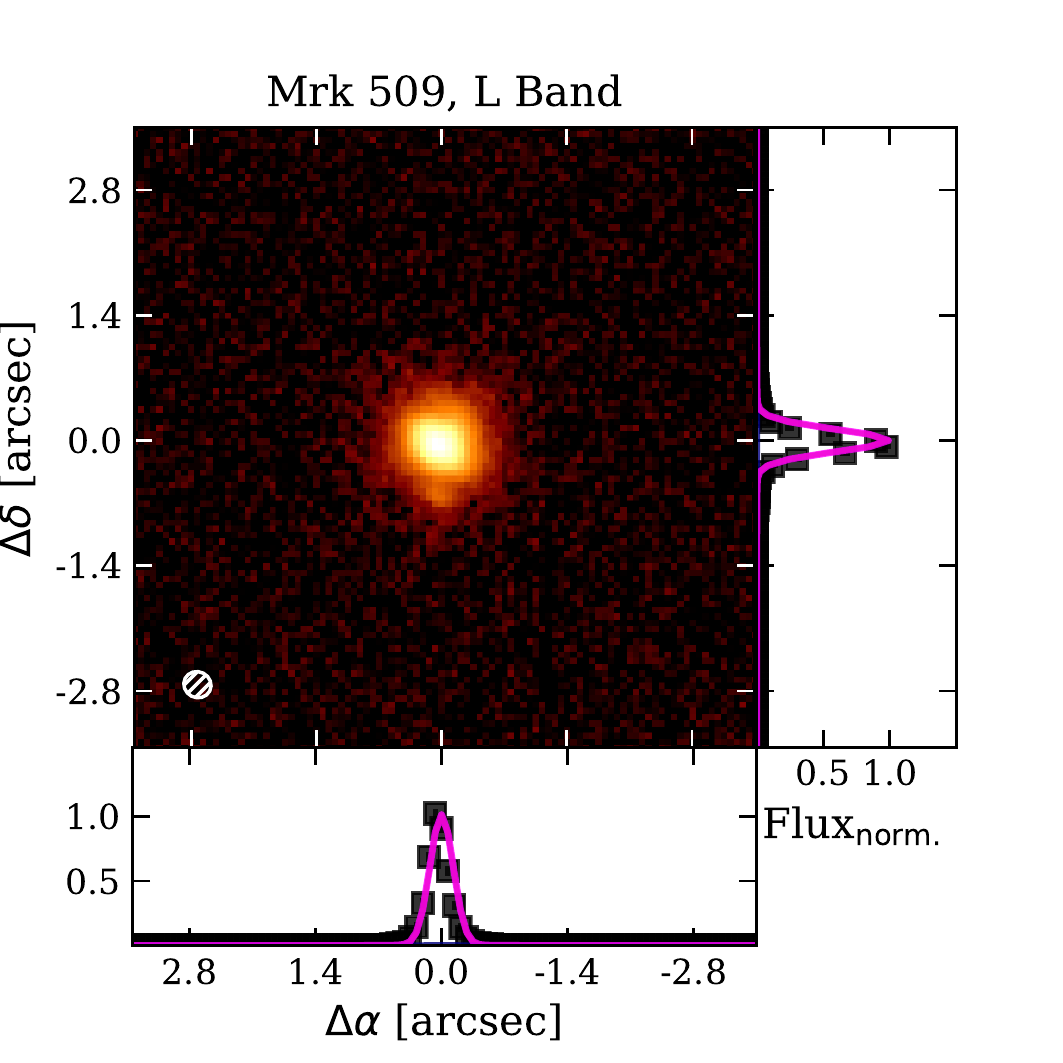}} 
\subfloat{\includegraphics[width=0.25\hsize]{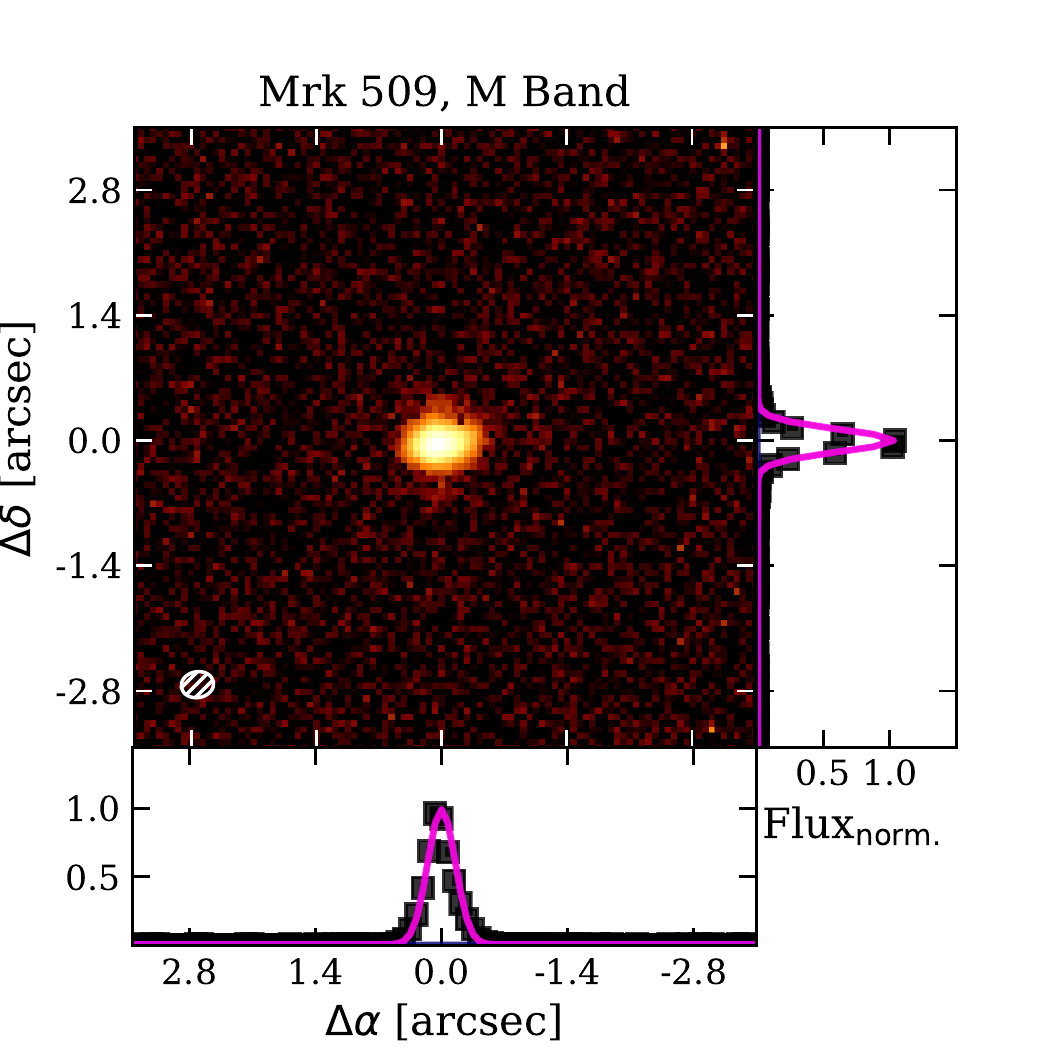}}
\subfloat{\includegraphics[width=0.25\hsize]{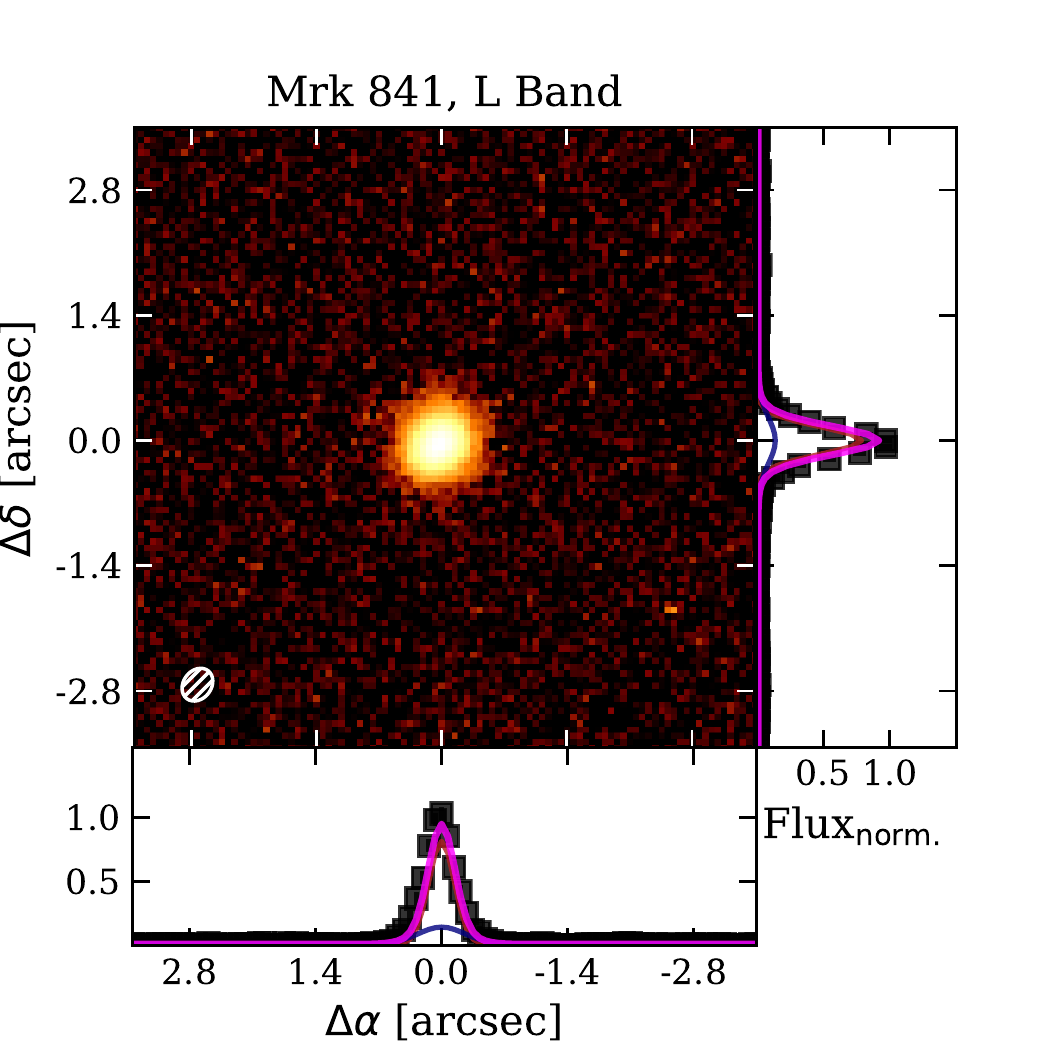}} \\
\subfloat{\includegraphics[width=0.25\hsize]{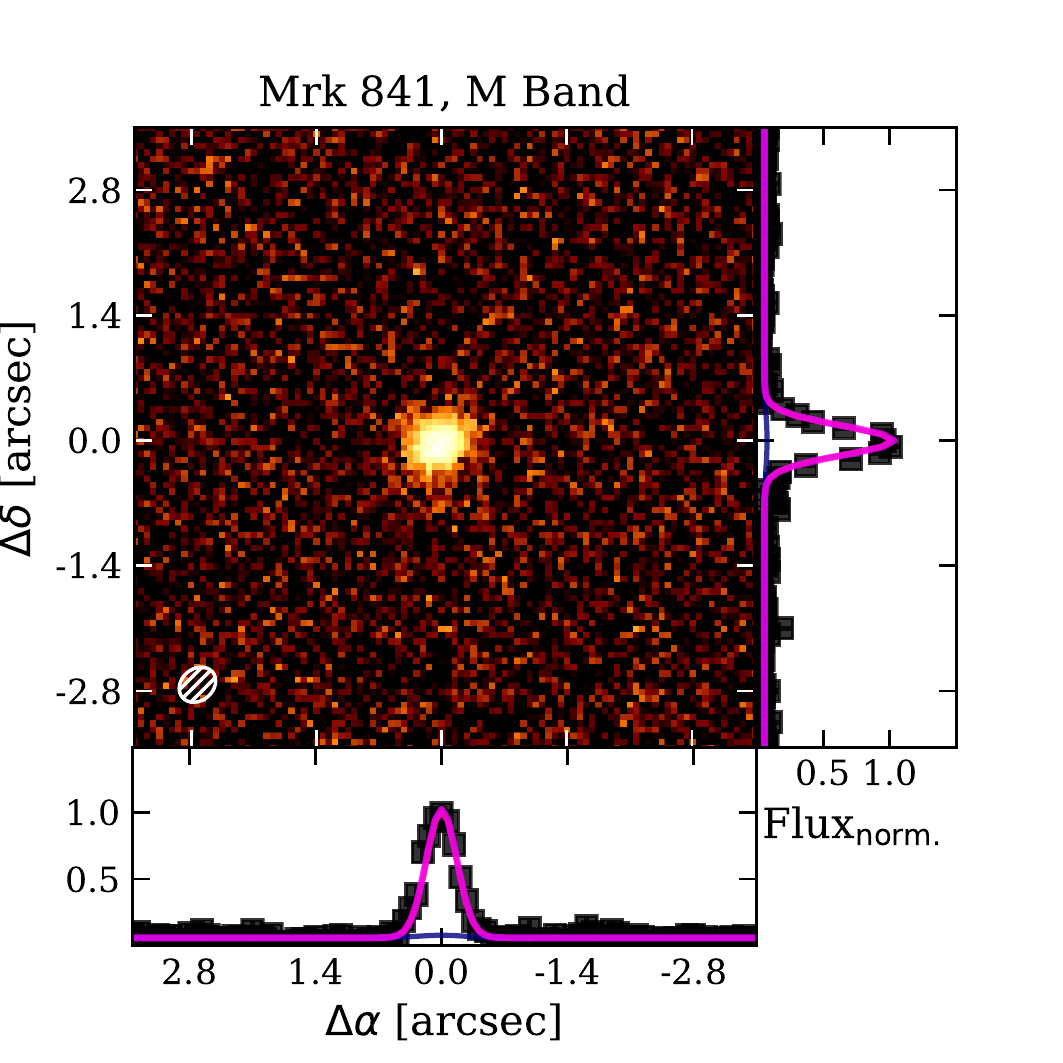}}
\subfloat{\includegraphics[width=0.25\hsize]{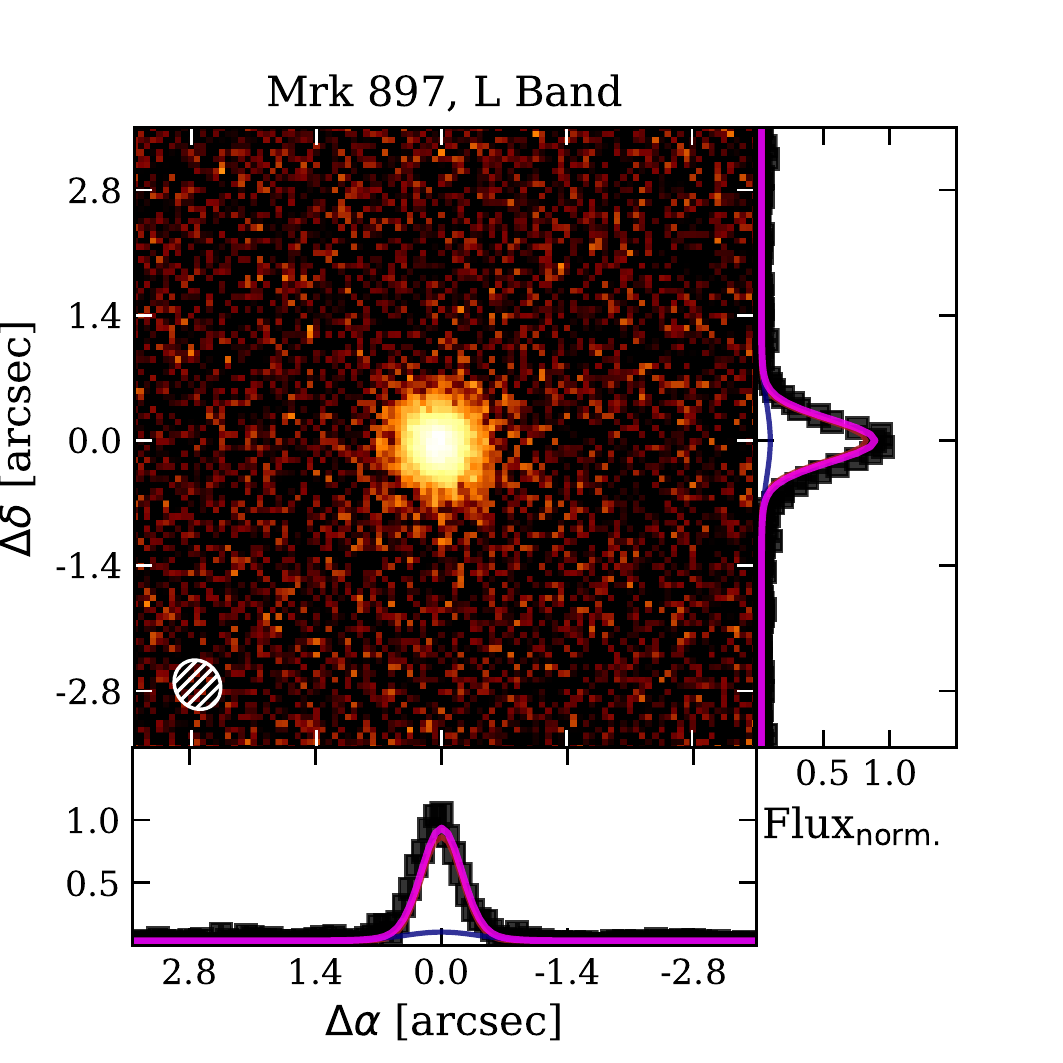}} 
\subfloat{\includegraphics[width=0.25\hsize]{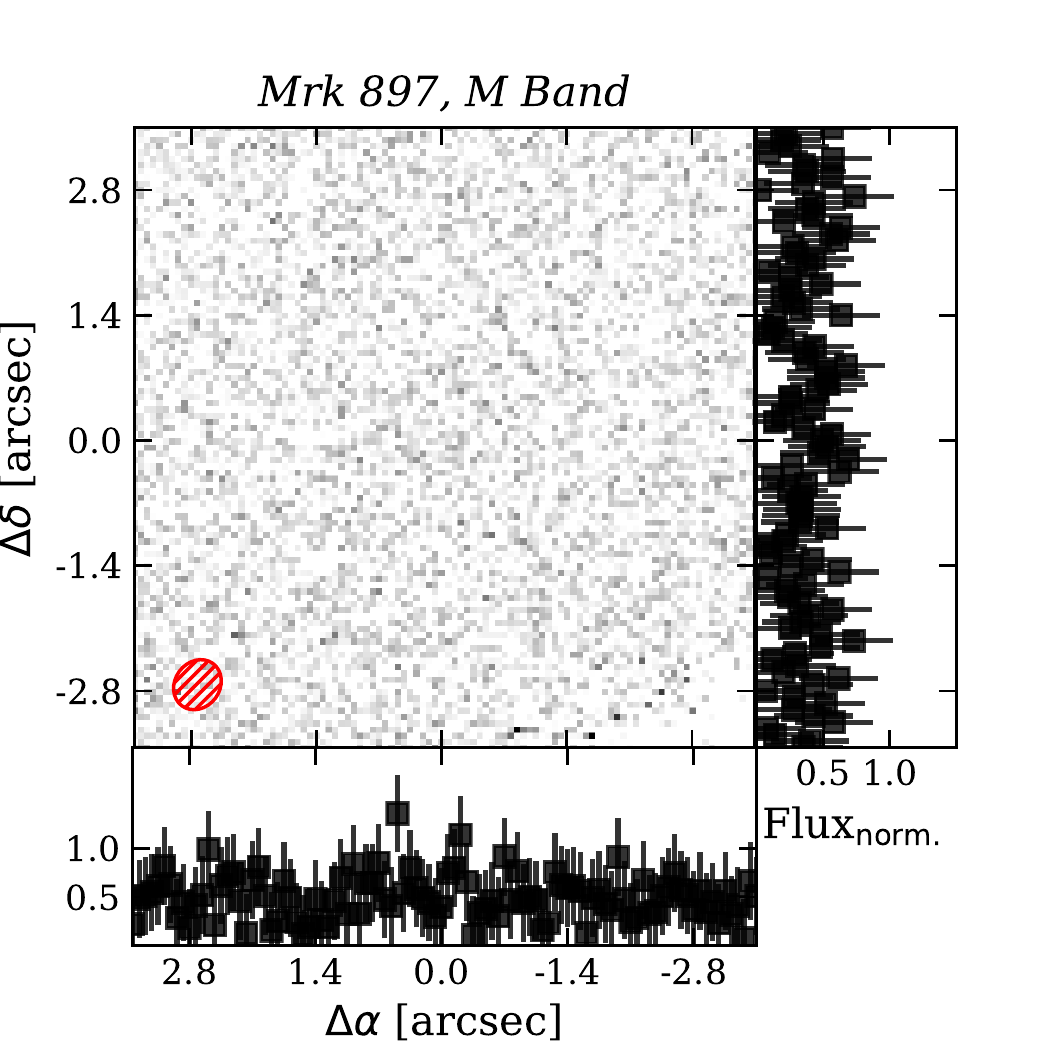}}
\subfloat{\includegraphics[width=0.25\hsize]{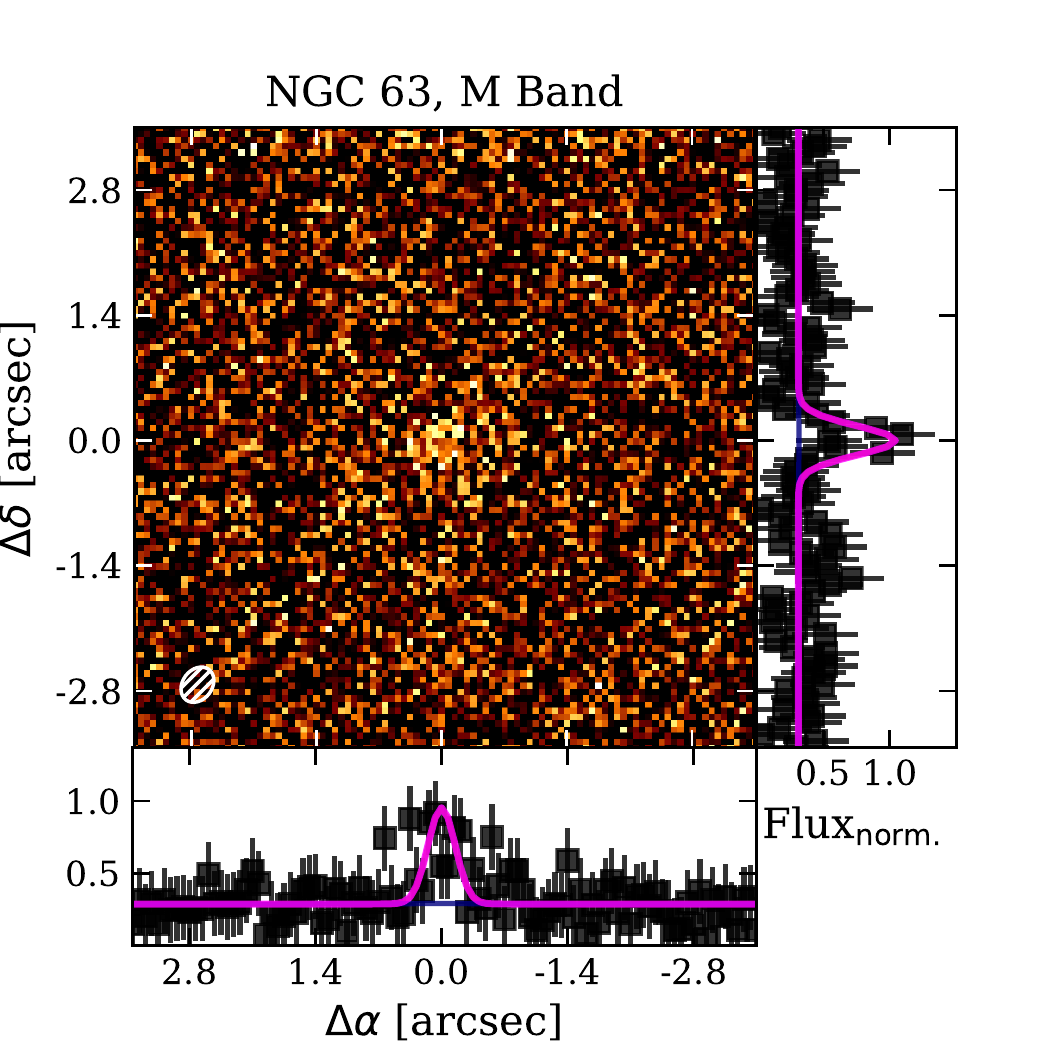}} \\
\subfloat{\includegraphics[width=0.25\hsize]{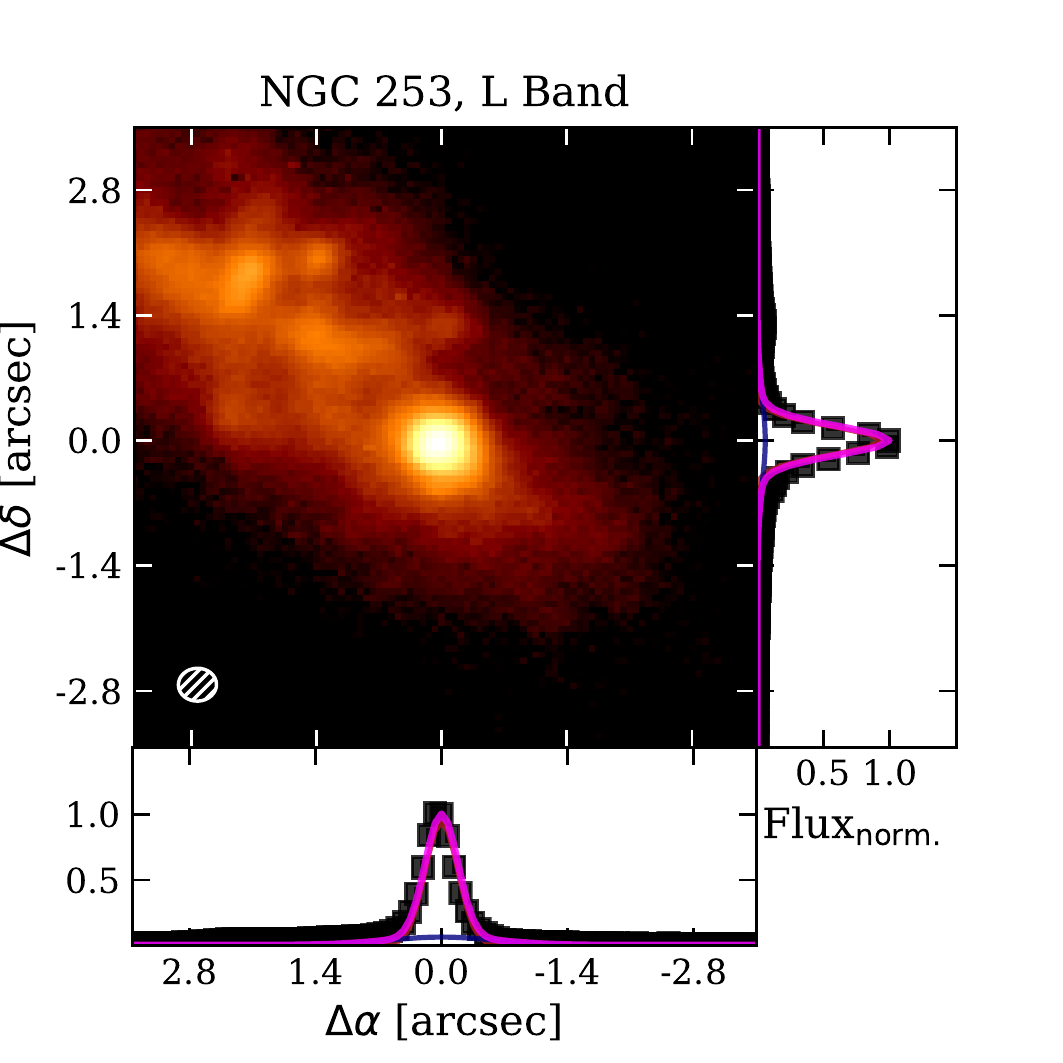}}
\subfloat{\includegraphics[width=0.25\hsize]{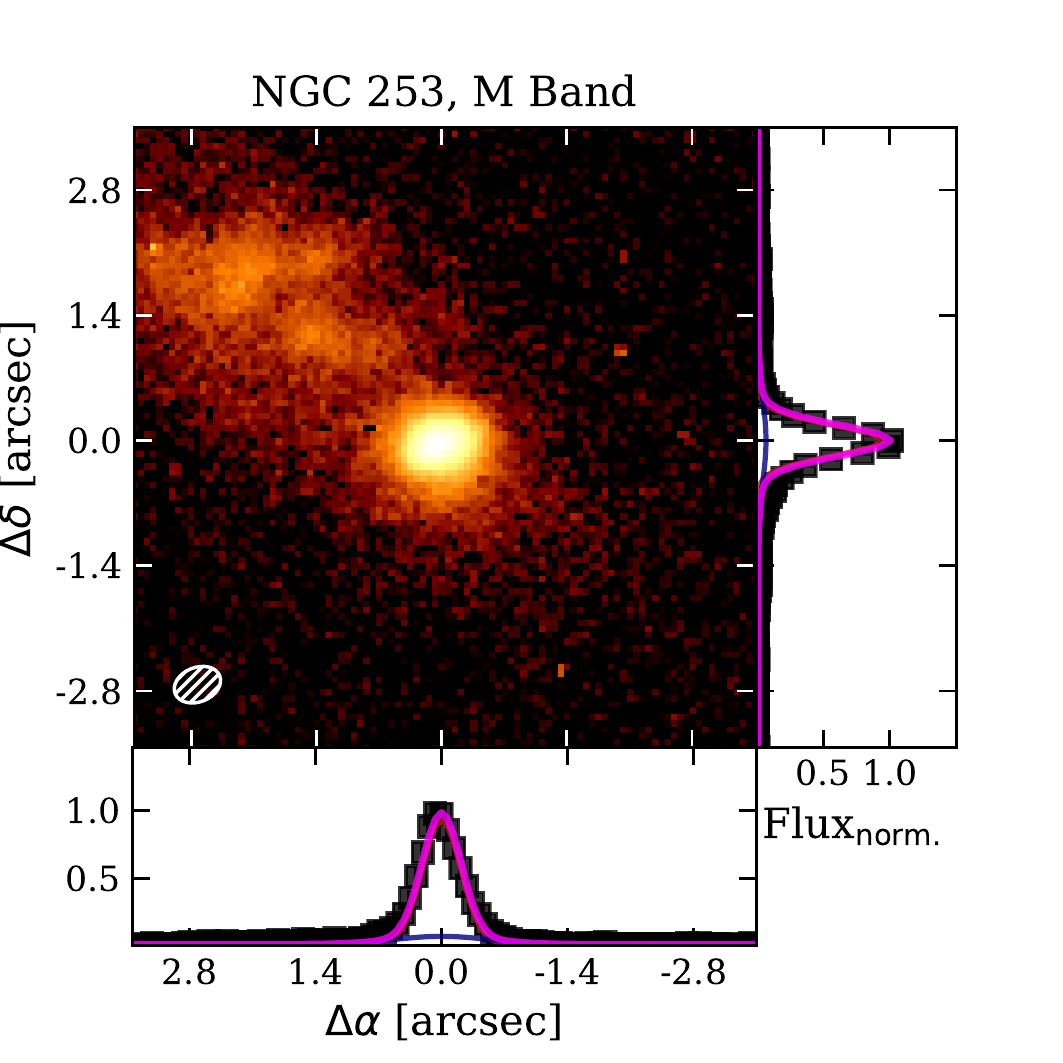}} 
\subfloat{\includegraphics[width=0.25\hsize]{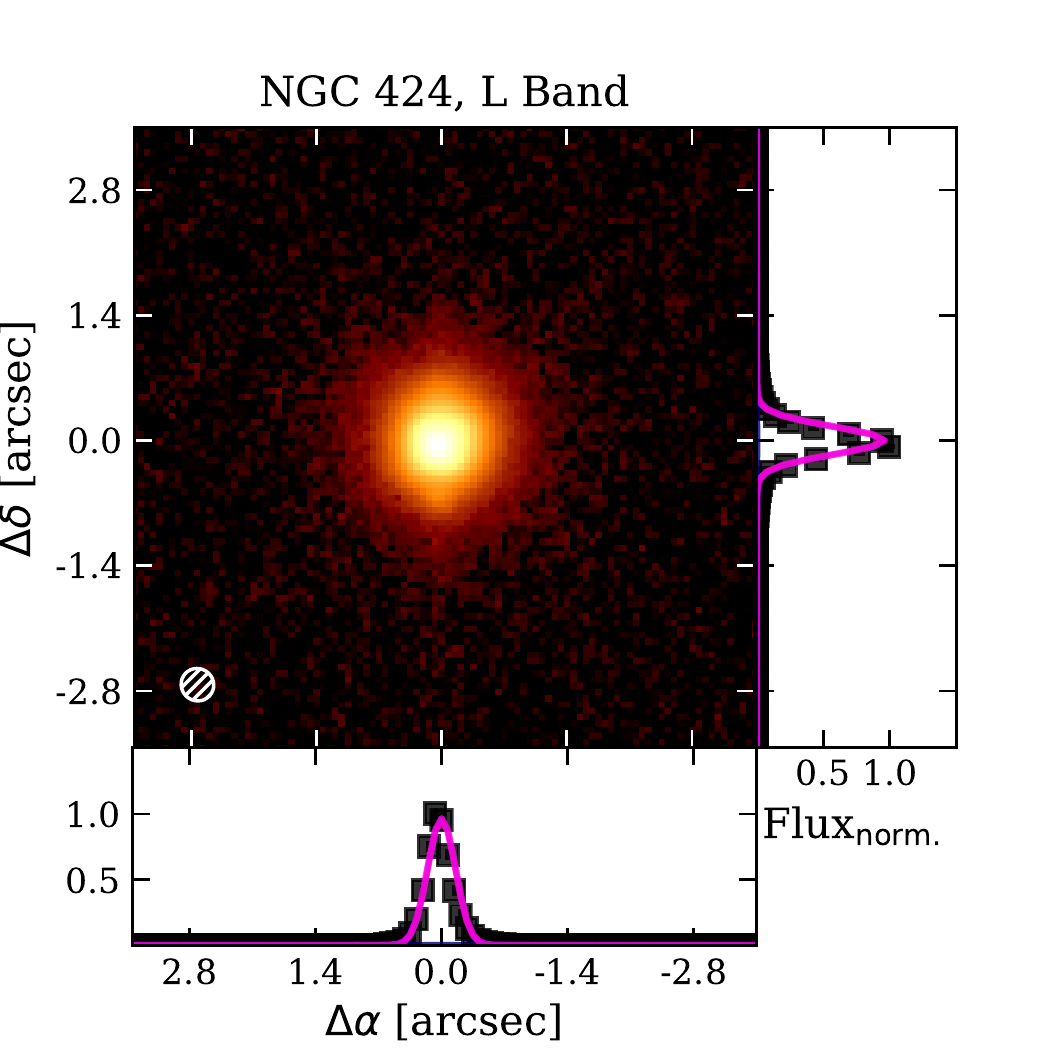}}
\subfloat{\includegraphics[width=0.25\hsize]{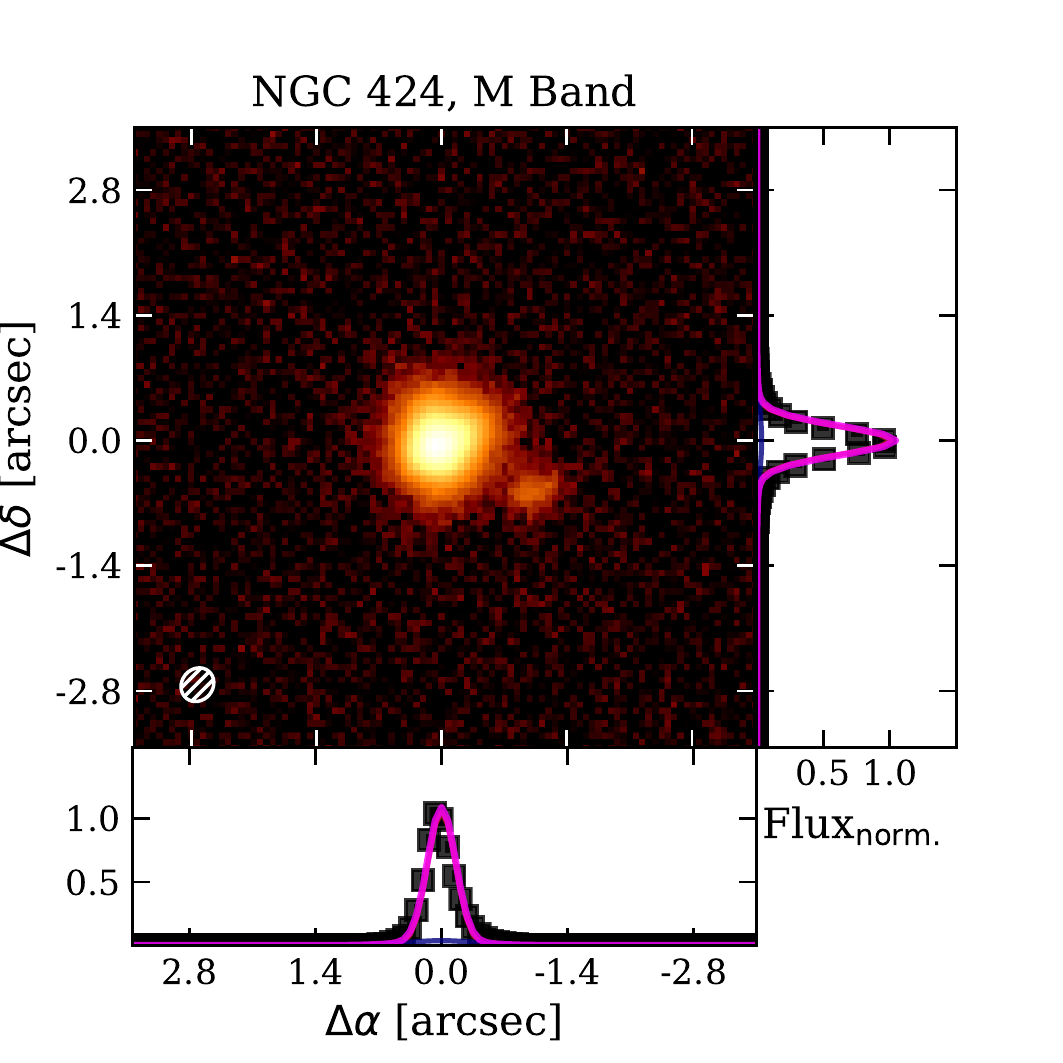}}\\
\caption{ As Fig \ref{fig:cutouts_one} but for all sources.}
\end{figure*}
\begin{figure*}
\subfloat{\includegraphics[width=0.25\hsize]{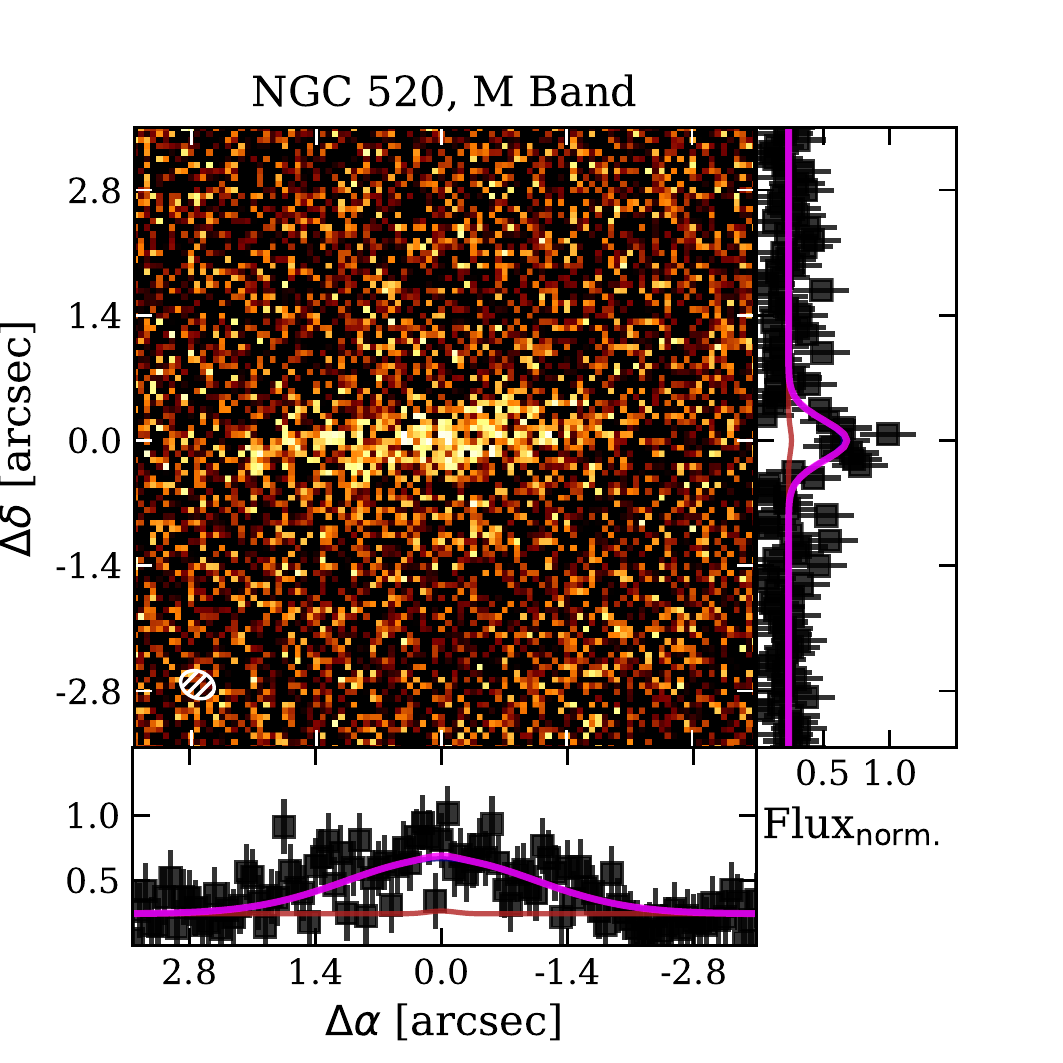}}
\subfloat{\includegraphics[width=0.25\hsize]{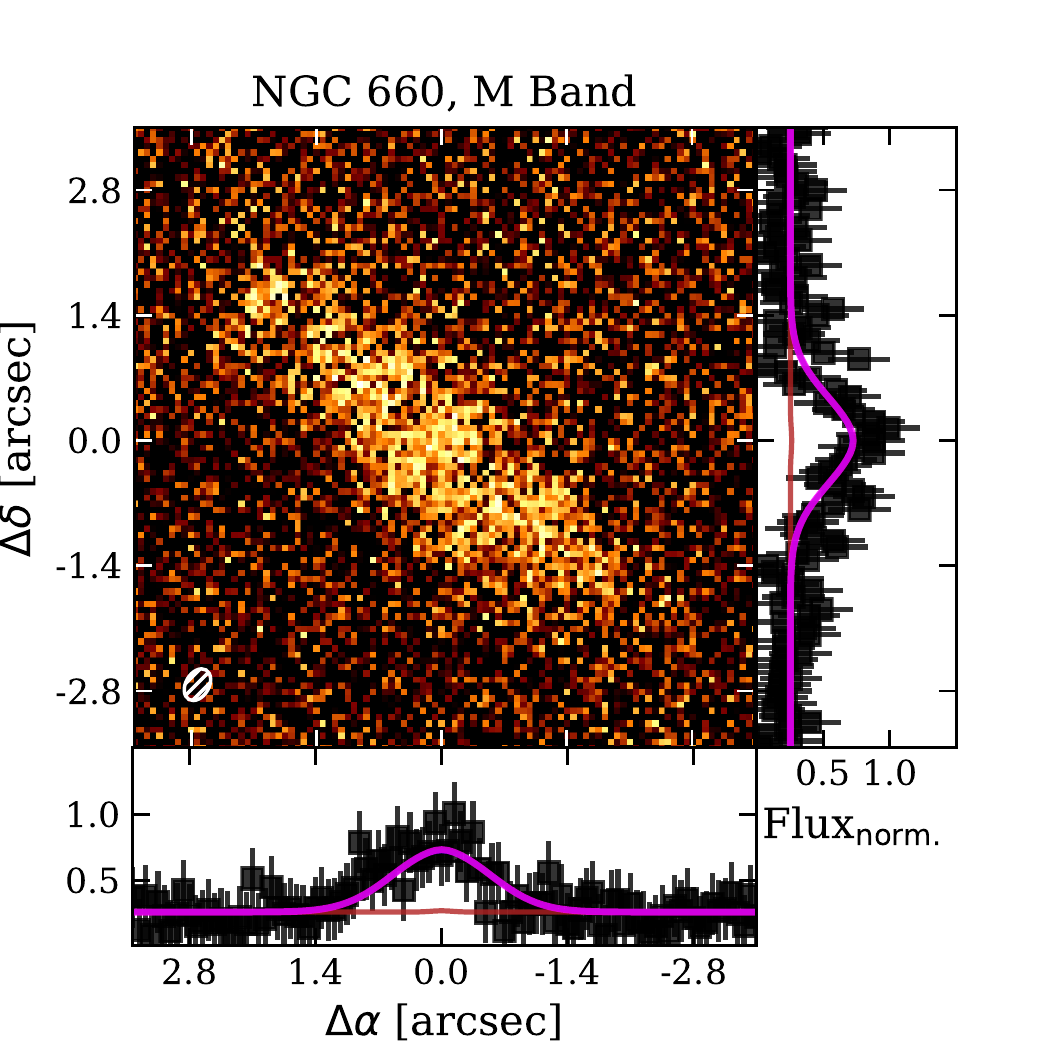}} 
\subfloat{\includegraphics[width=0.25\hsize]{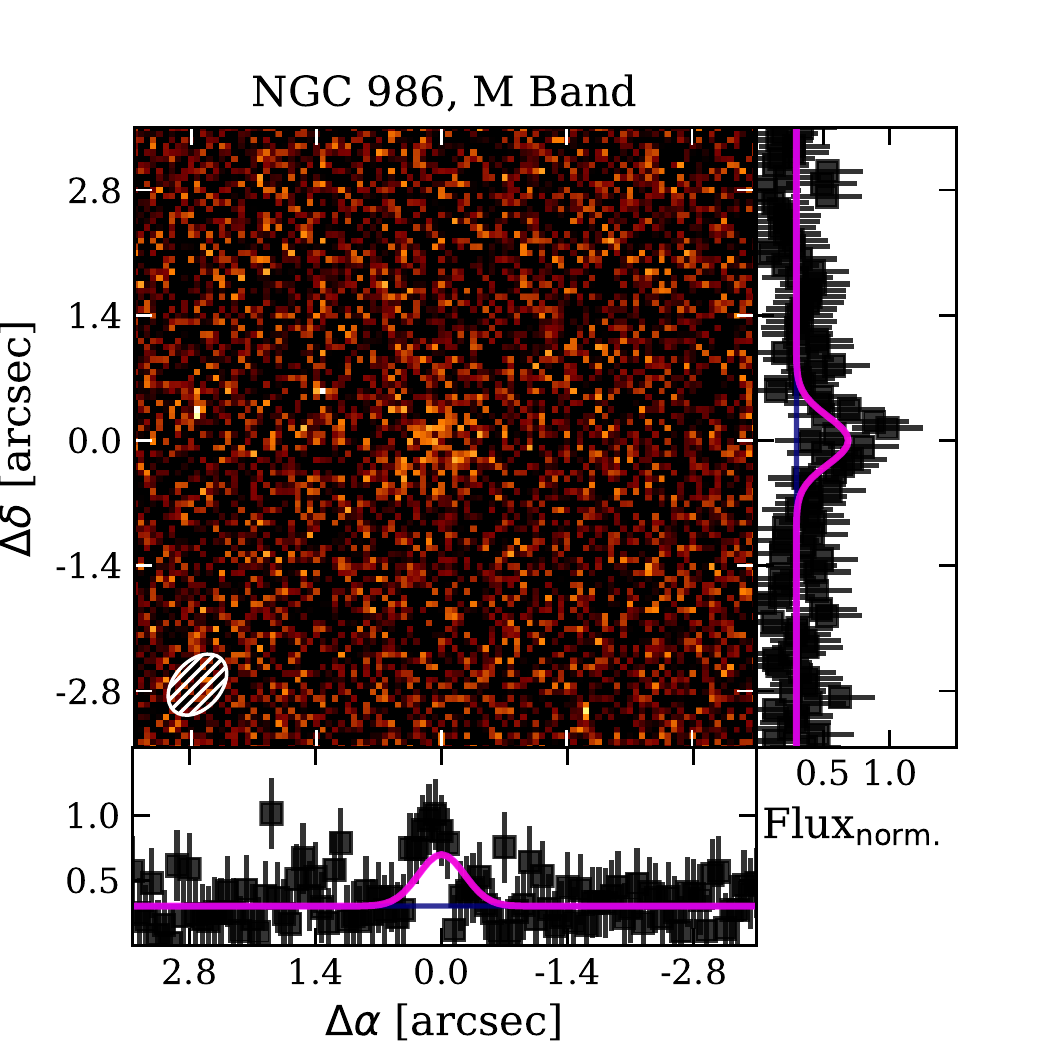}}
\subfloat{\includegraphics[width=0.25\hsize]{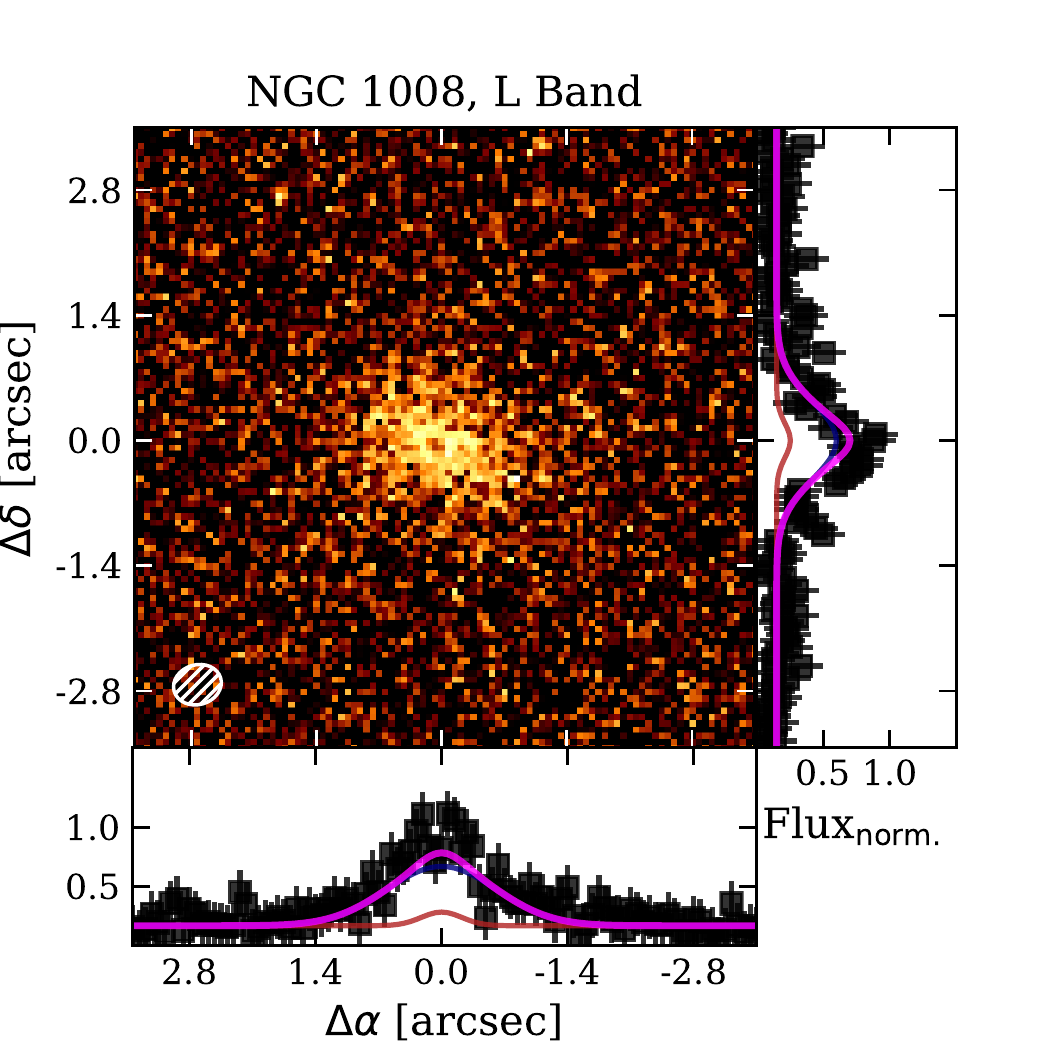}}\\
\subfloat{\includegraphics[width=0.25\hsize]{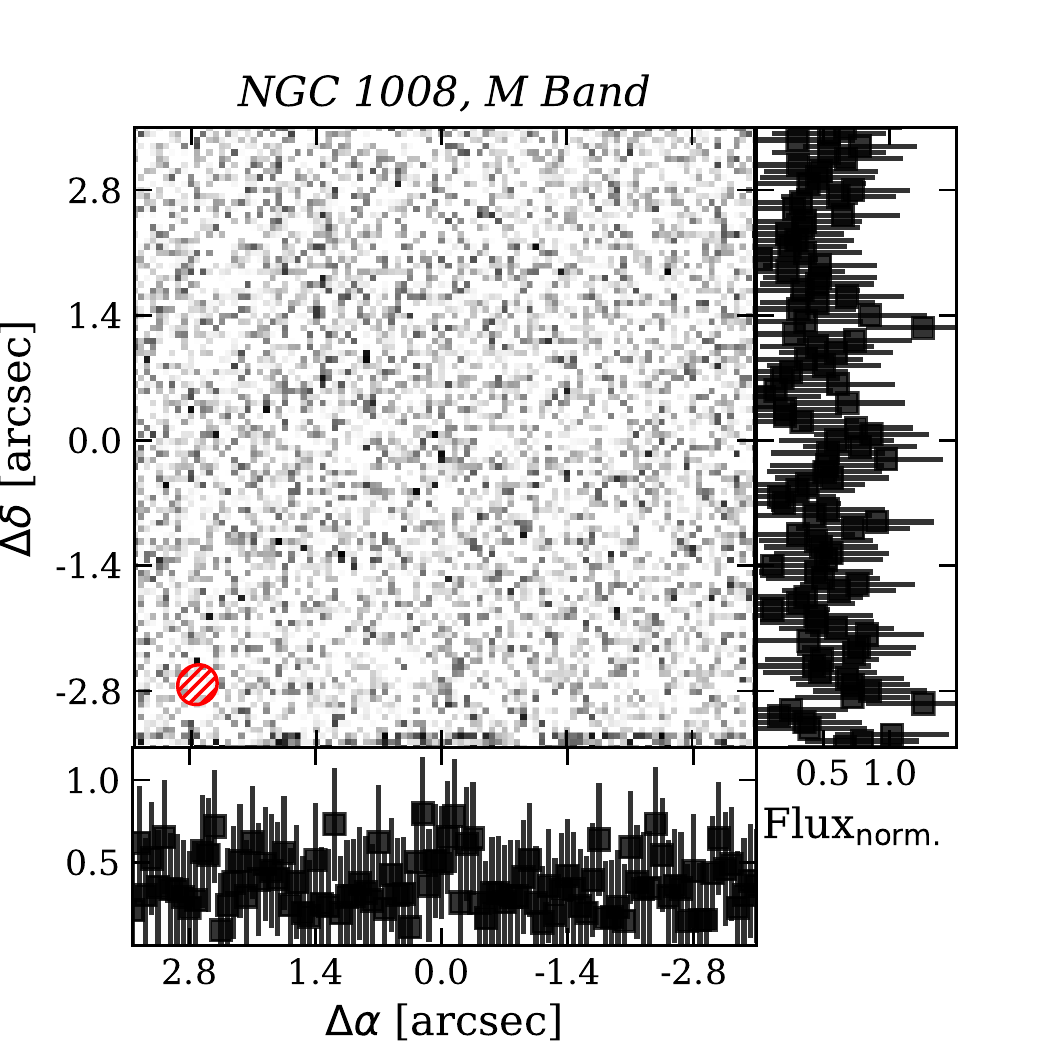}}
\subfloat{\includegraphics[width=0.25\hsize]{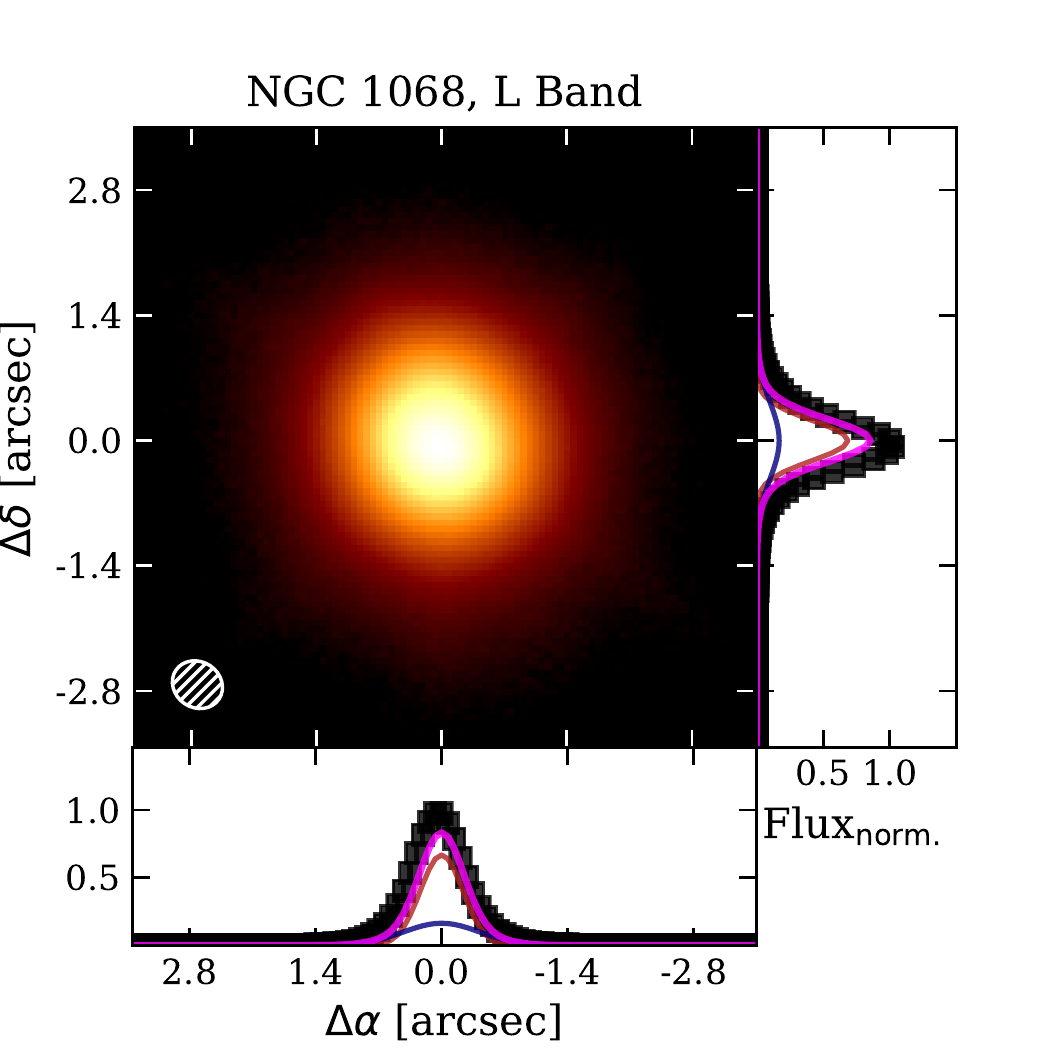}} 
\subfloat{\includegraphics[width=0.25\hsize]{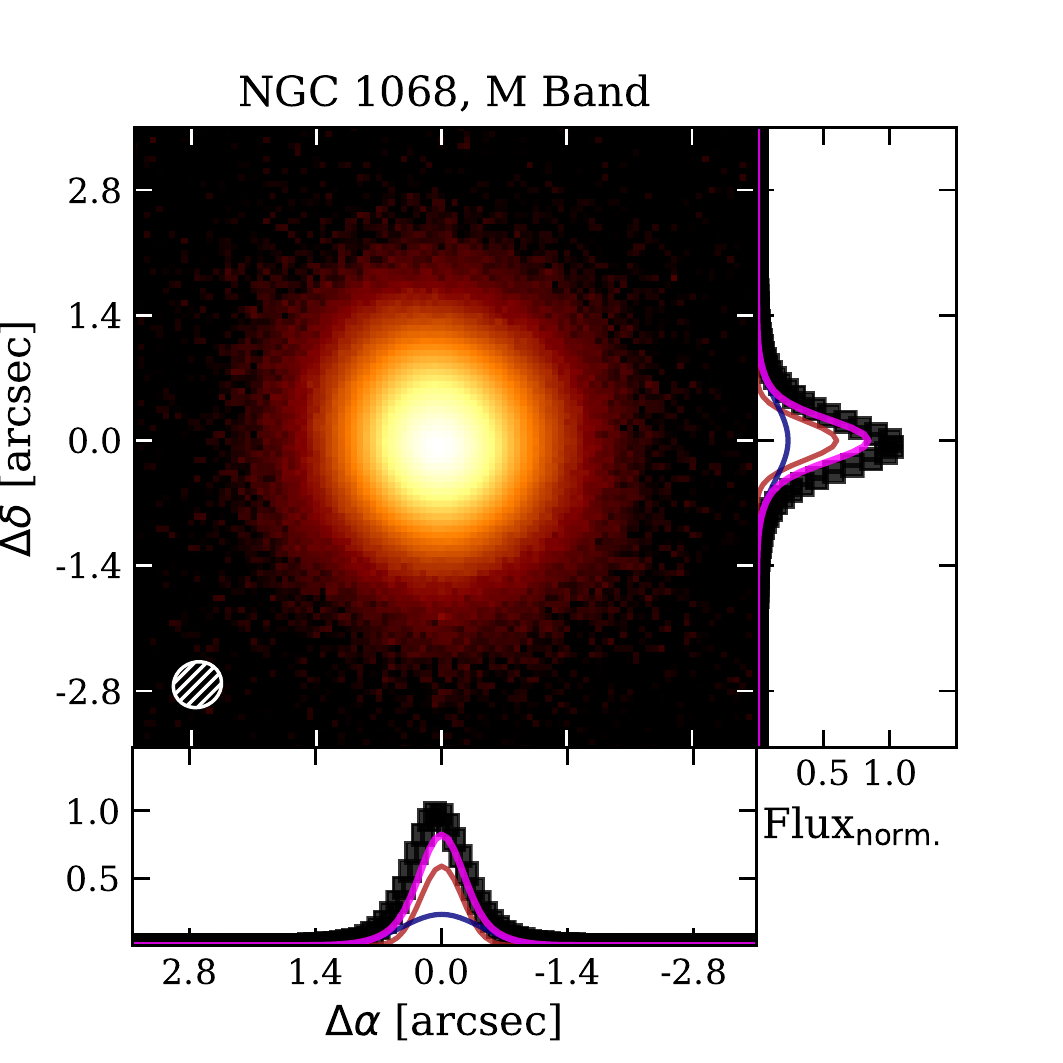}}
\subfloat{\includegraphics[width=0.25\hsize]{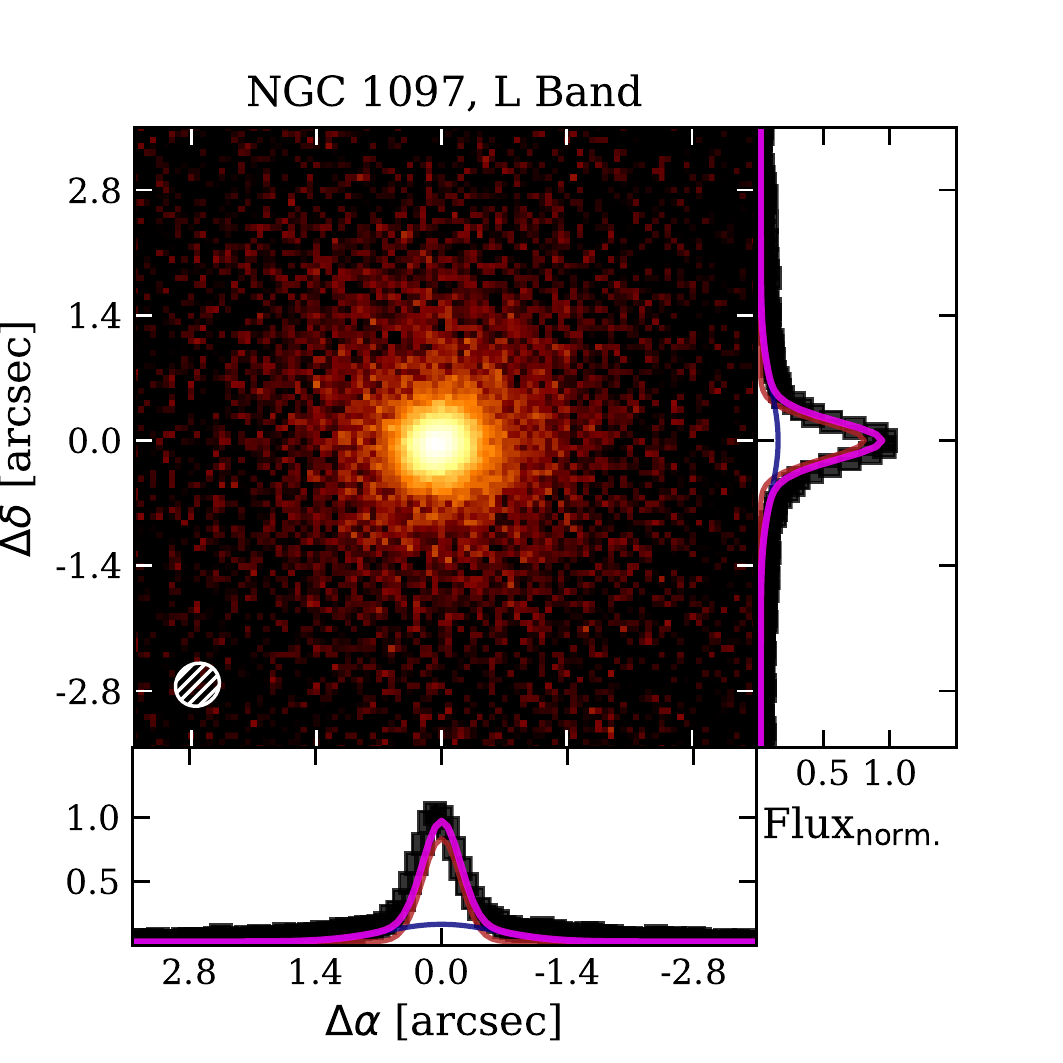}}\\
\subfloat{\includegraphics[width=0.25\hsize]{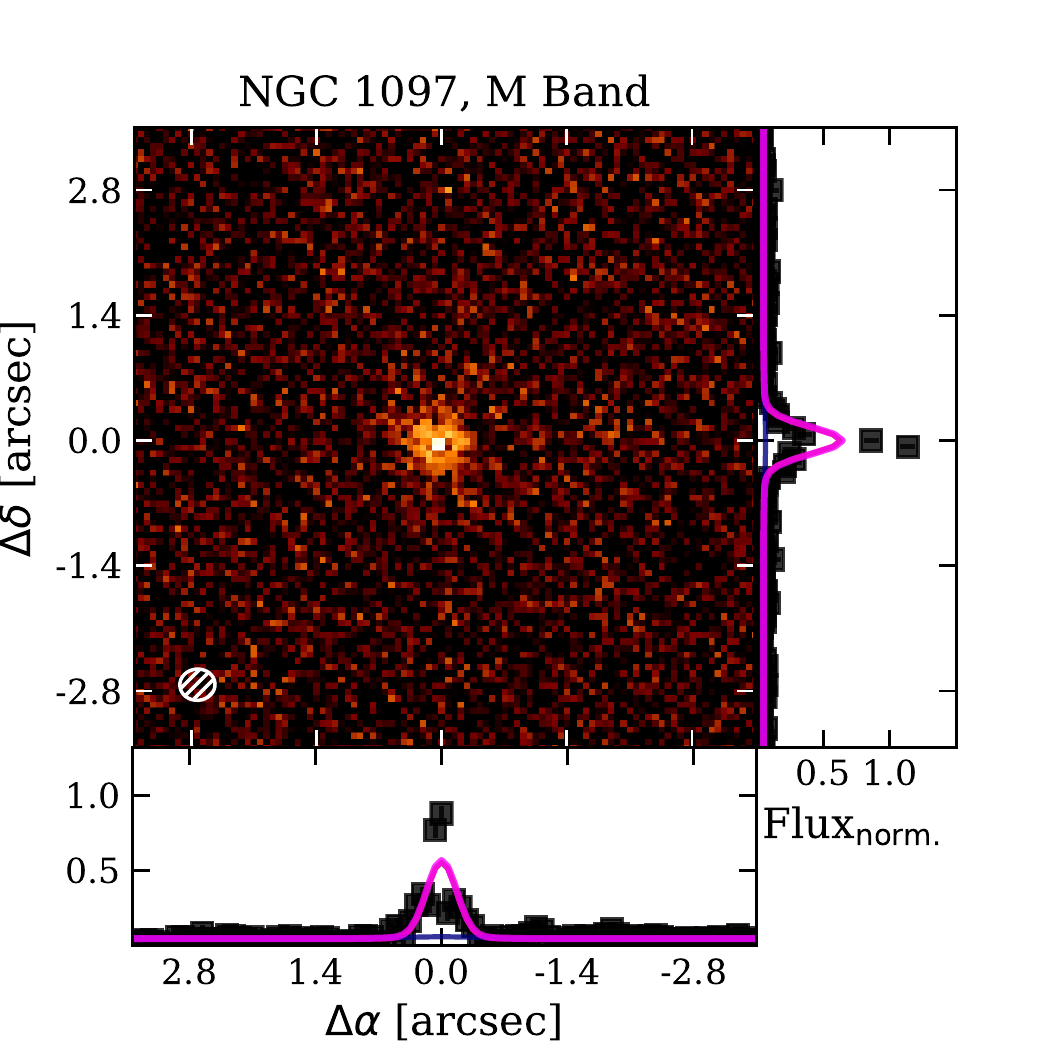}}
\subfloat{\includegraphics[width=0.25\hsize]{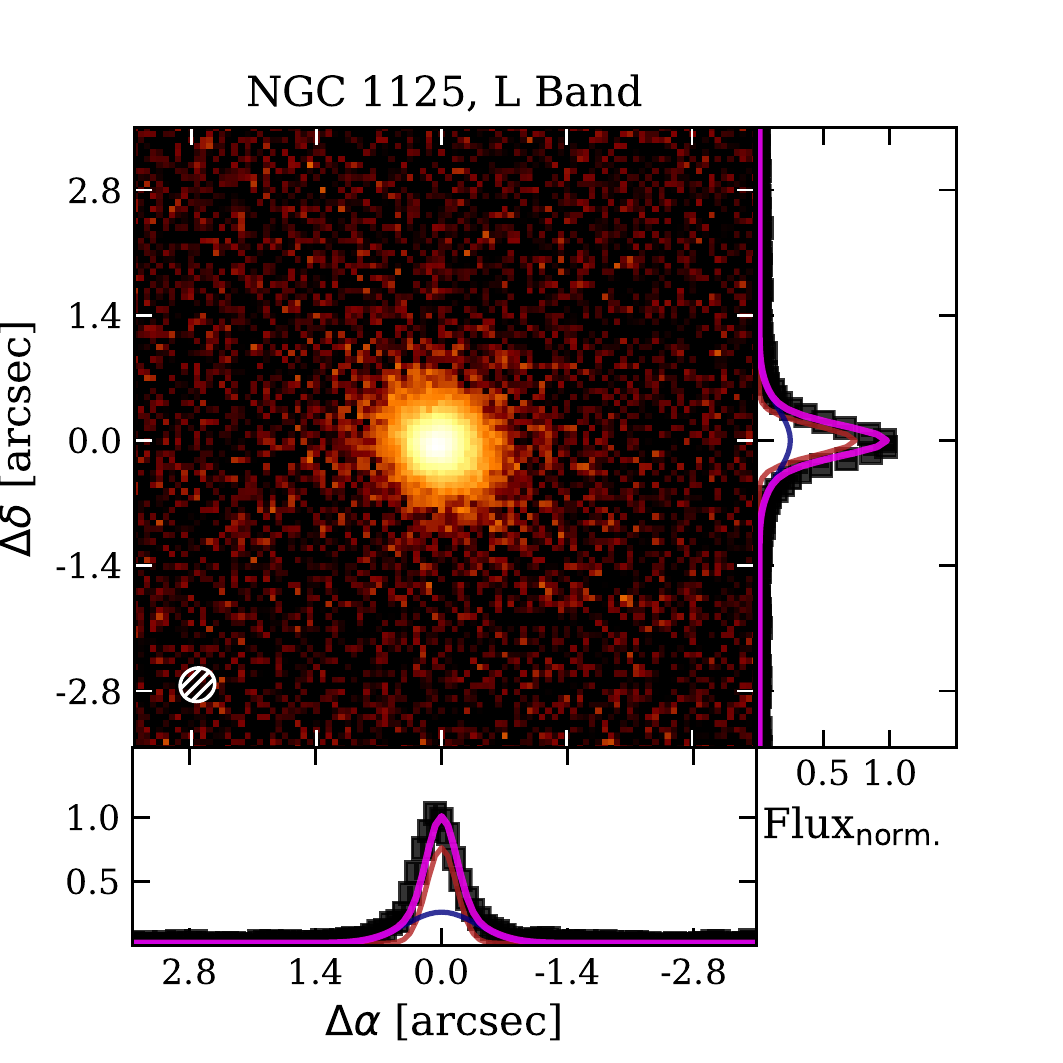}} 
\subfloat{\includegraphics[width=0.25\hsize]{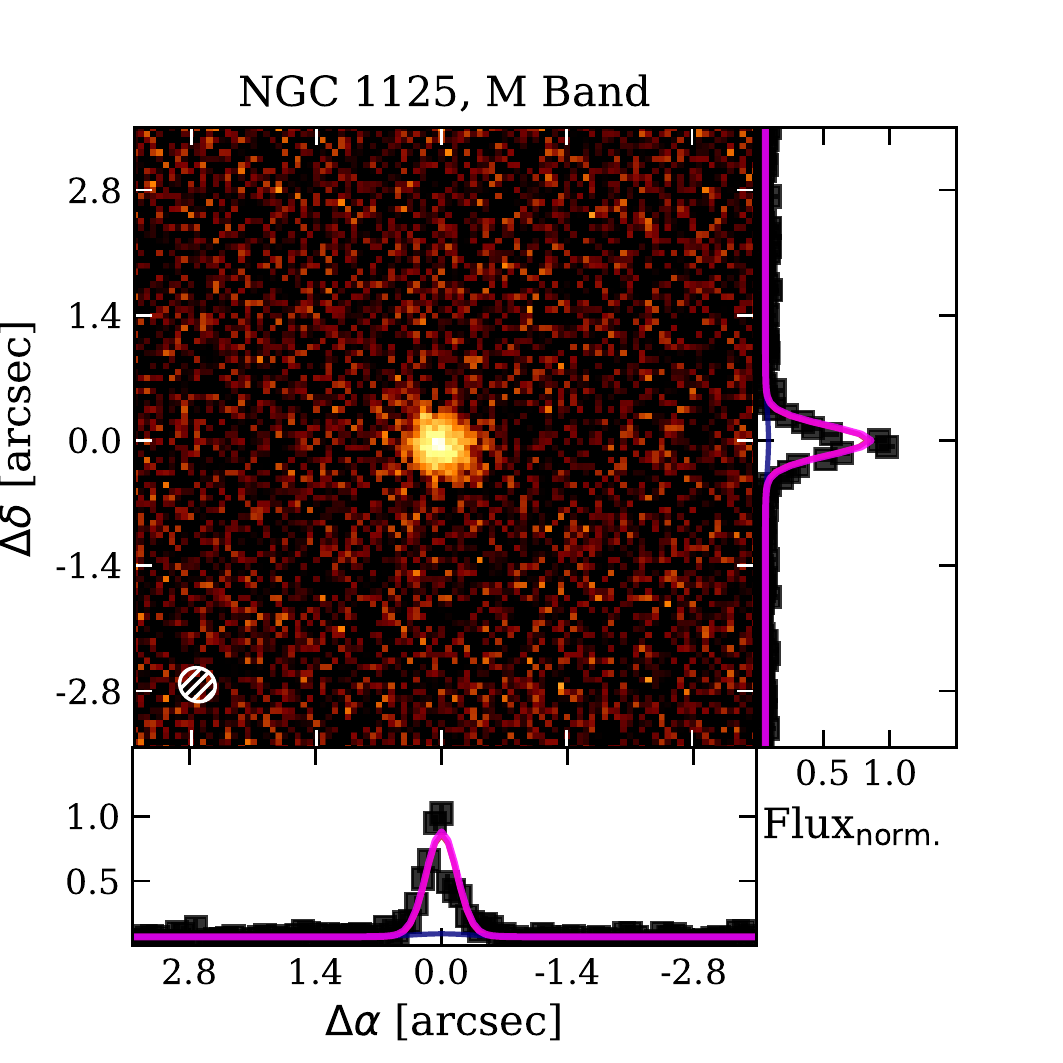}}
\subfloat{\includegraphics[width=0.25\hsize]{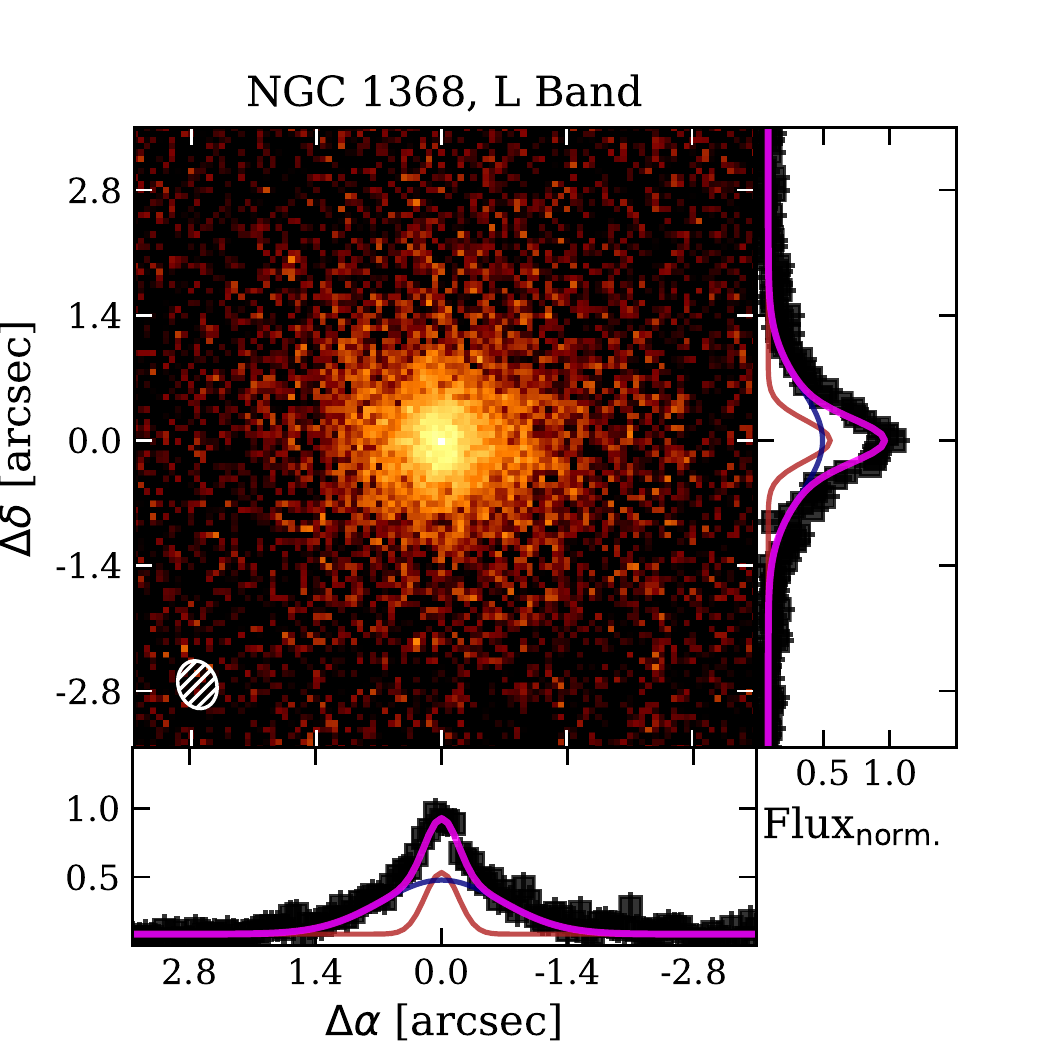}}\\
\subfloat{\includegraphics[width=0.25\hsize]{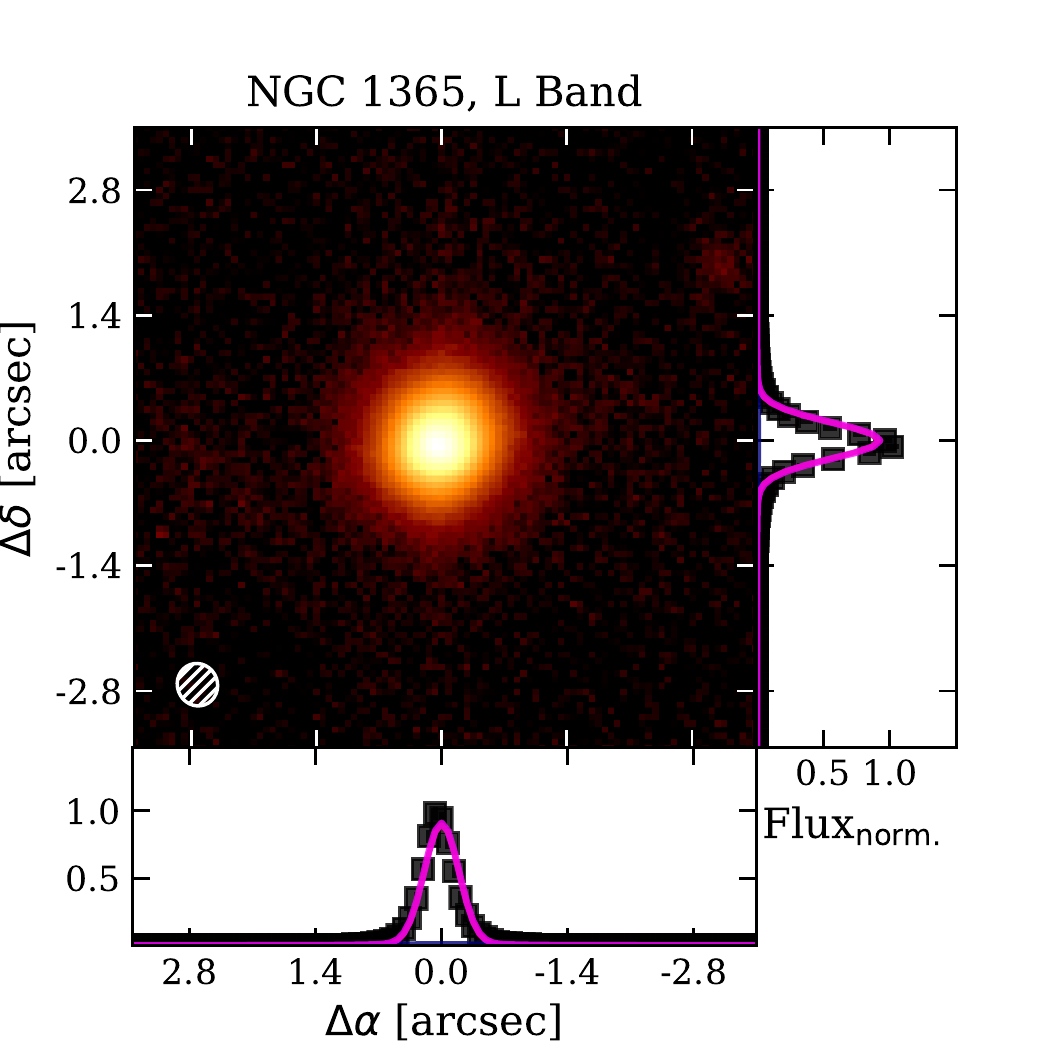}}
\subfloat{\includegraphics[width=0.25\hsize]{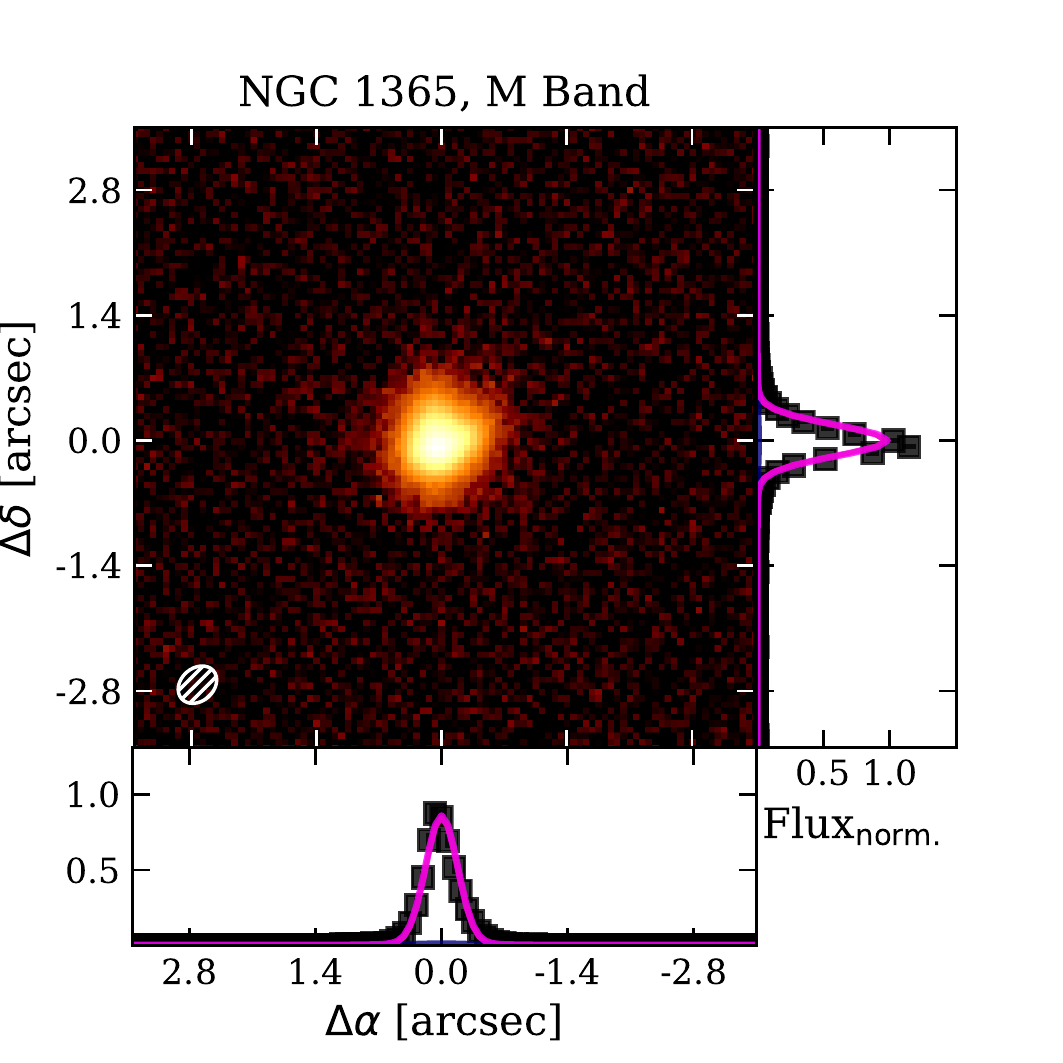}} 
\subfloat{\includegraphics[width=0.25\hsize]{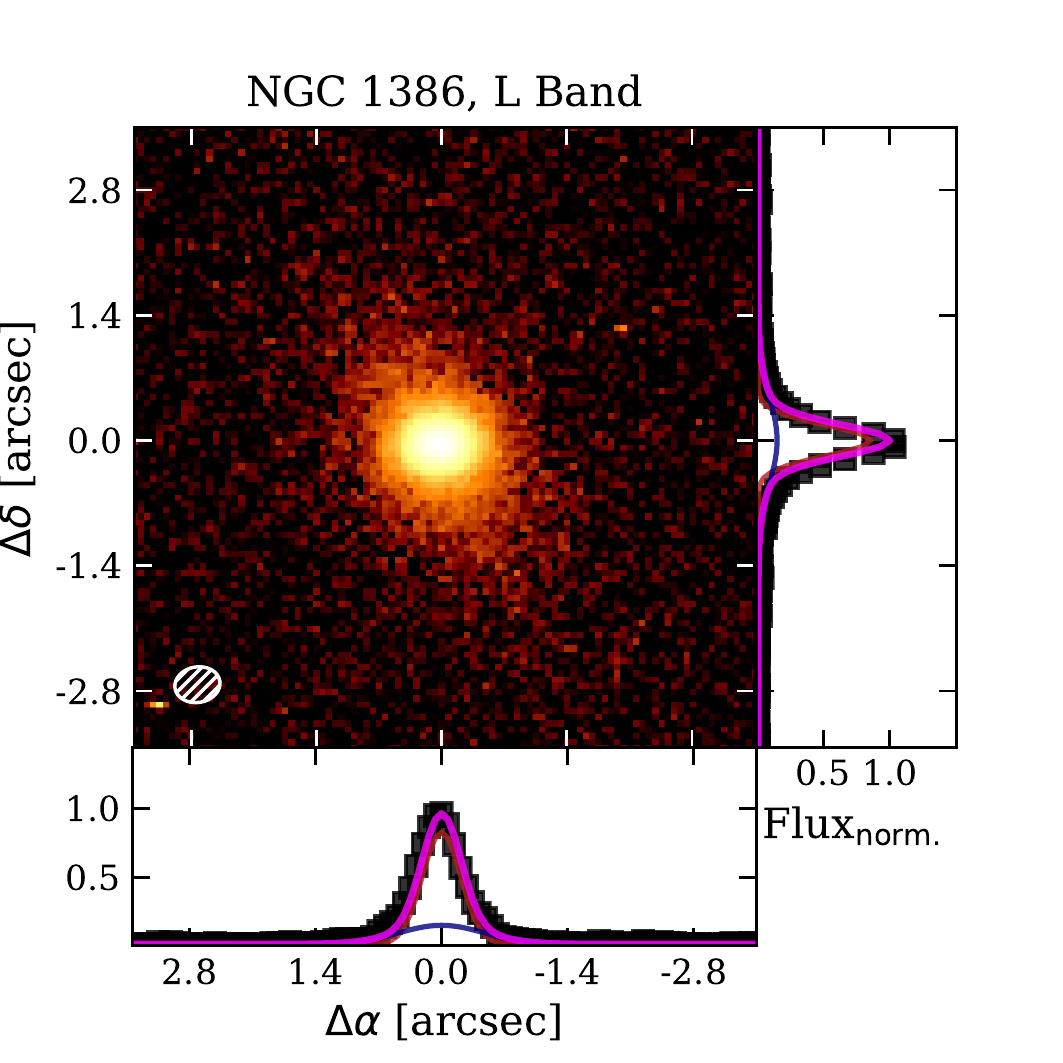}}
\subfloat{\includegraphics[width=0.25\hsize]{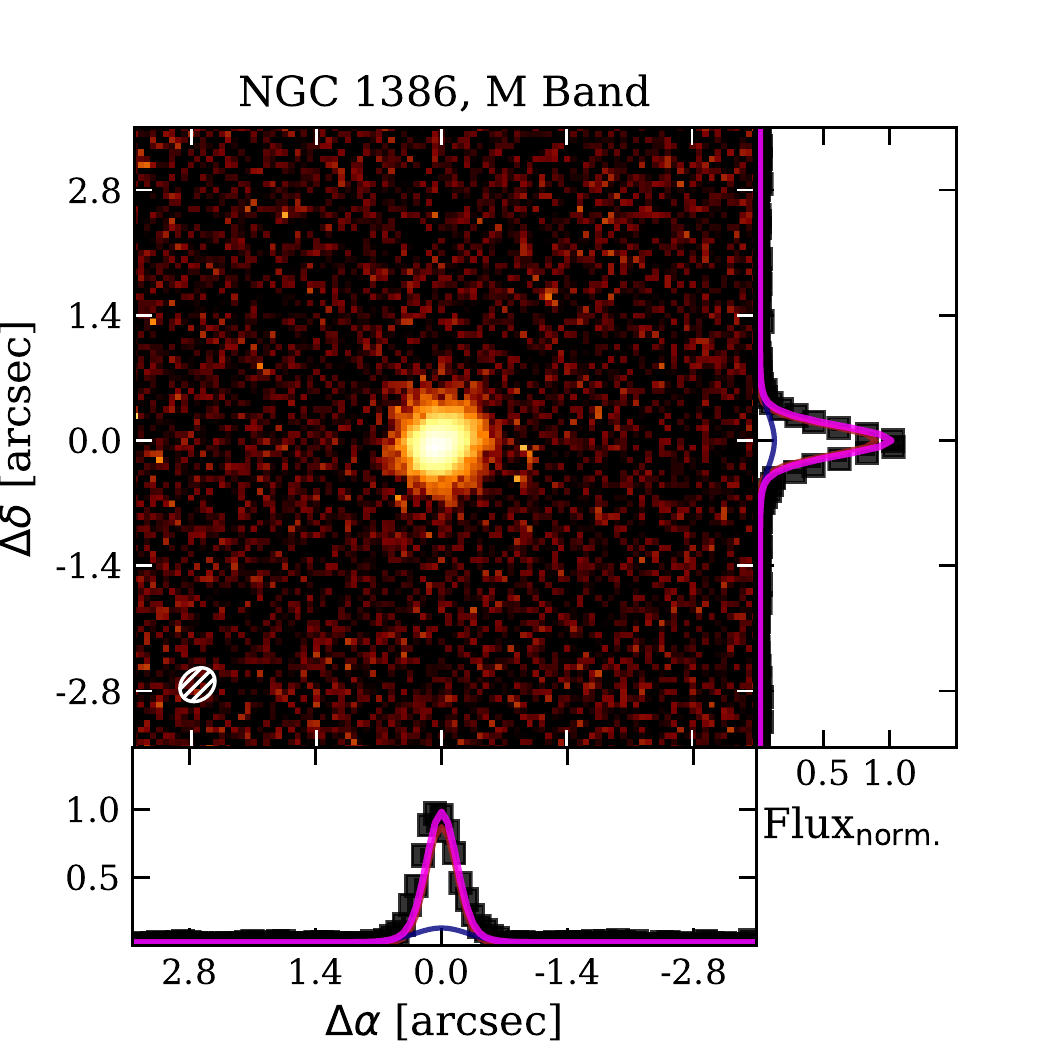}} \\
\subfloat{\includegraphics[width=0.25\hsize]{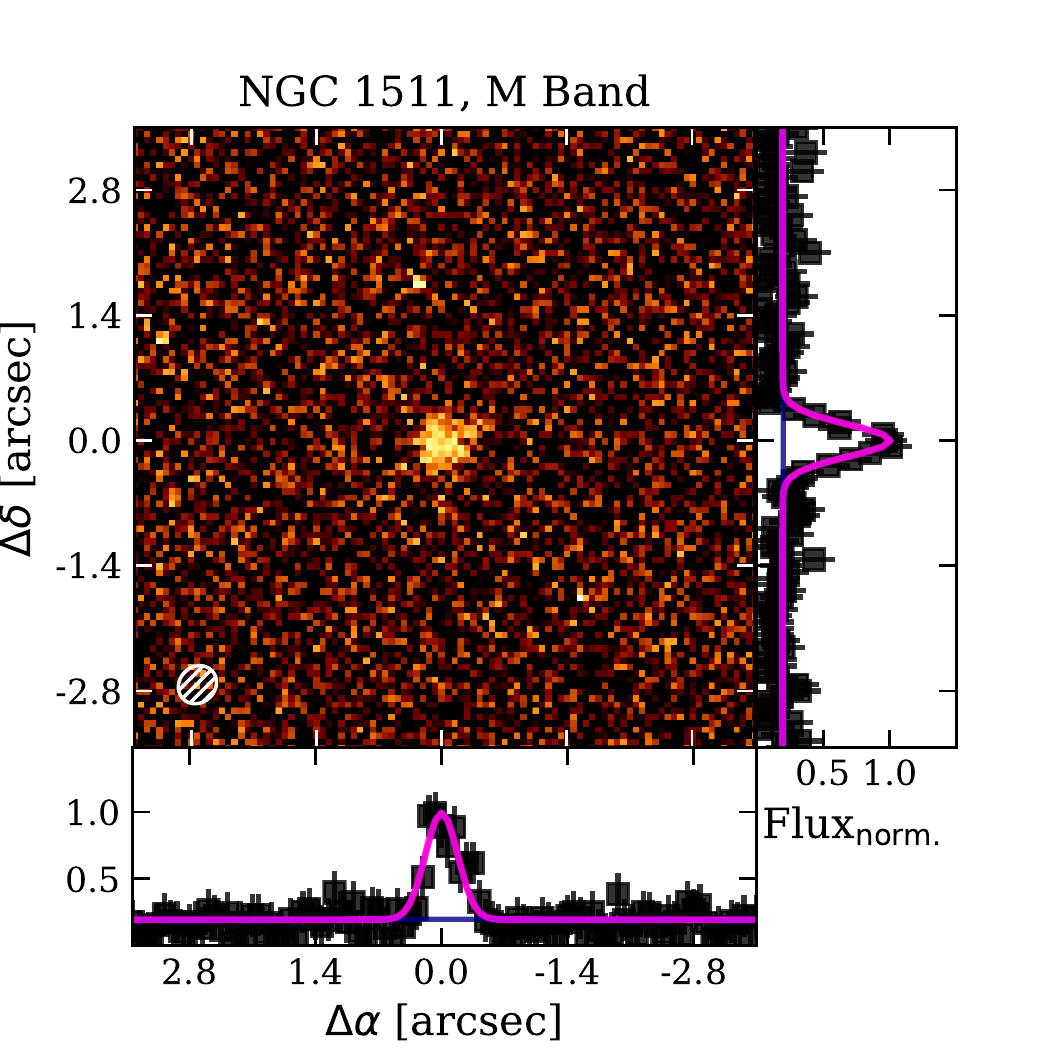}}
\subfloat{\includegraphics[width=0.25\hsize]{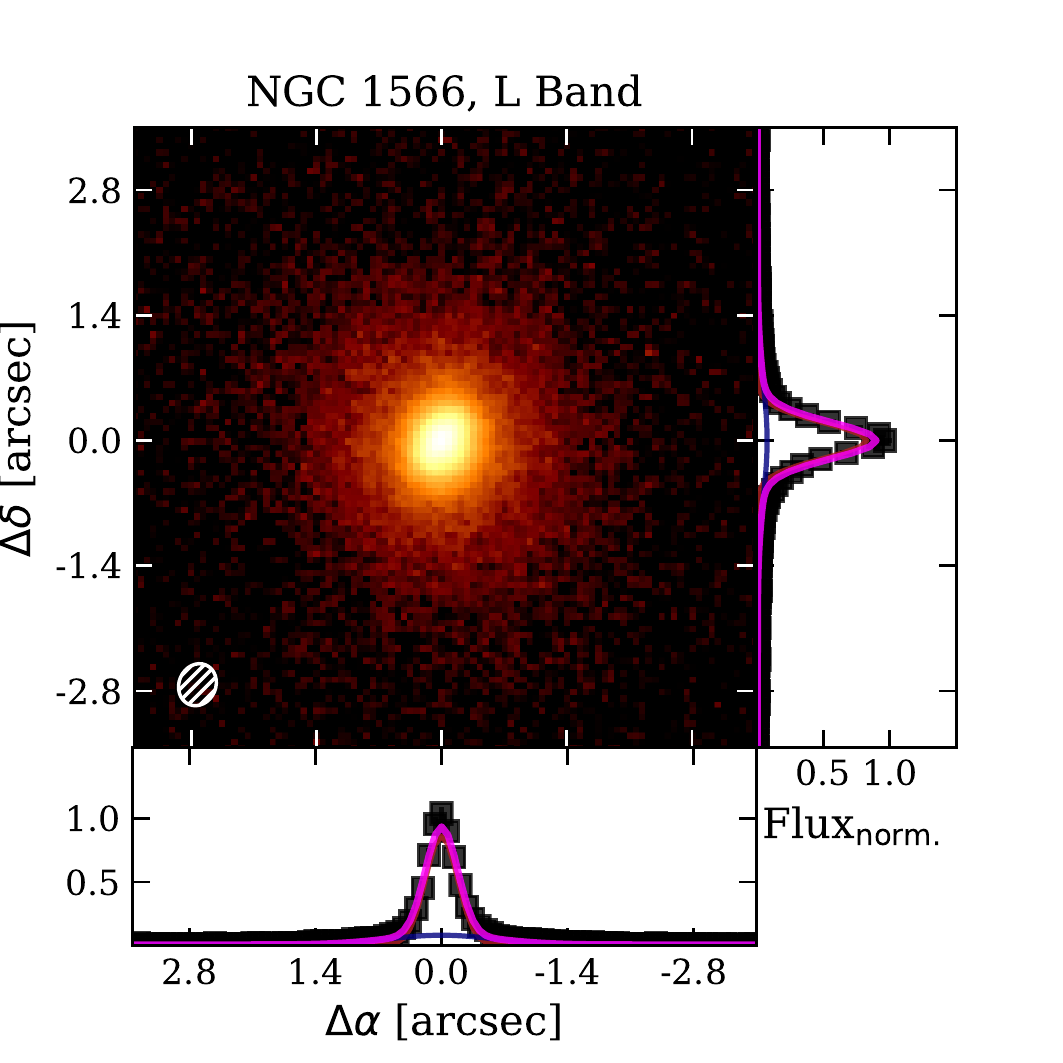}} 
\subfloat{\includegraphics[width=0.25\hsize]{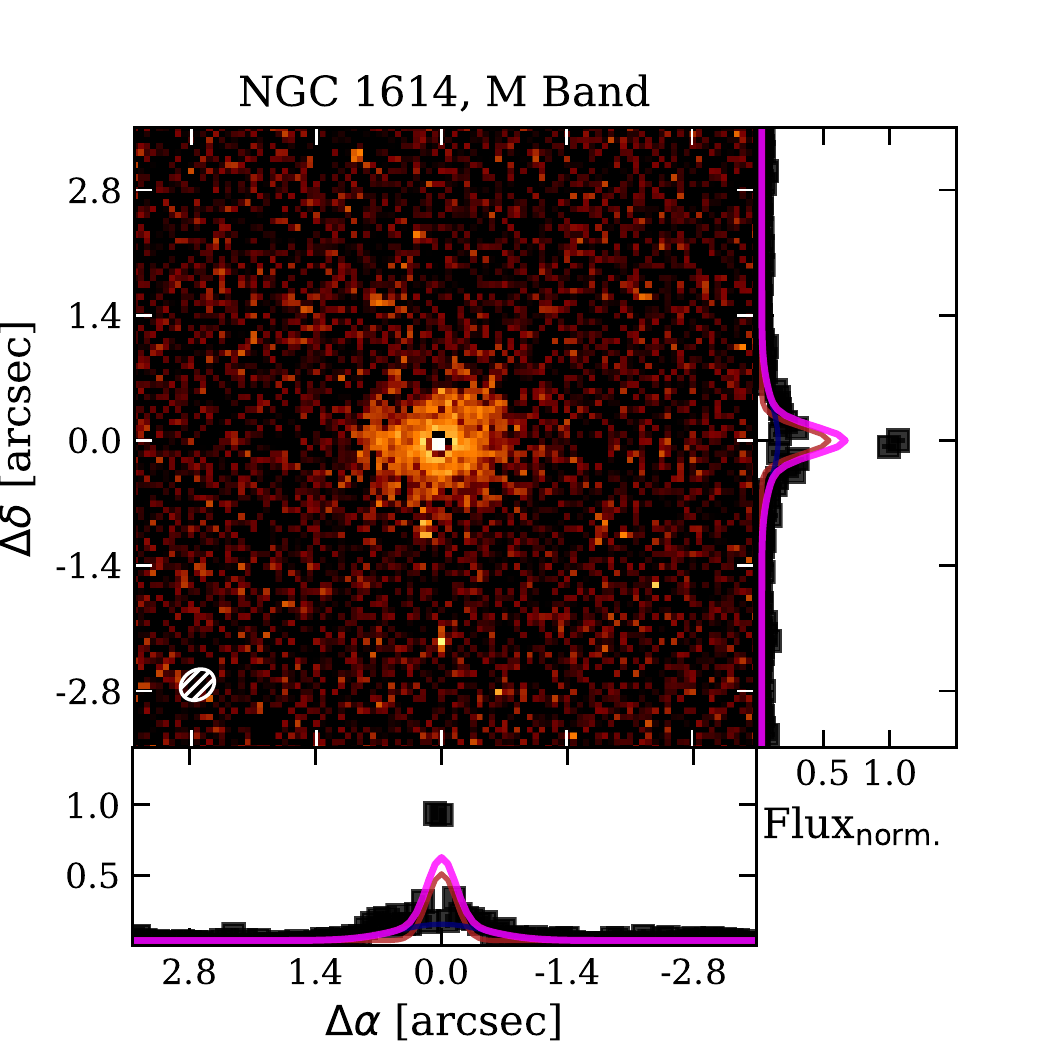}}
\subfloat{\includegraphics[width=0.25\hsize]{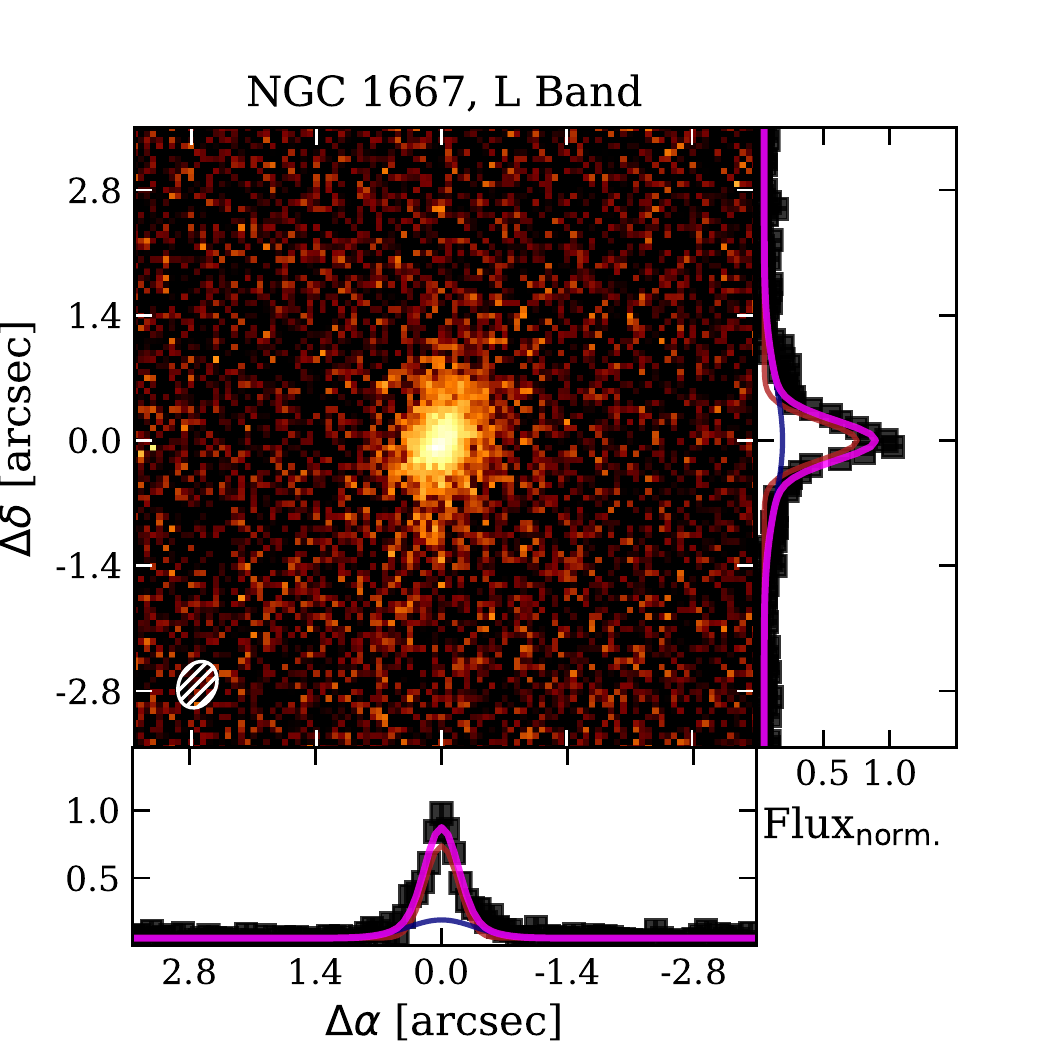}}\\
\caption{ As Fig \ref{fig:cutouts_one} but for all sources.}
\end{figure*}
\begin{figure*}
\subfloat{\includegraphics[width=0.25\hsize]{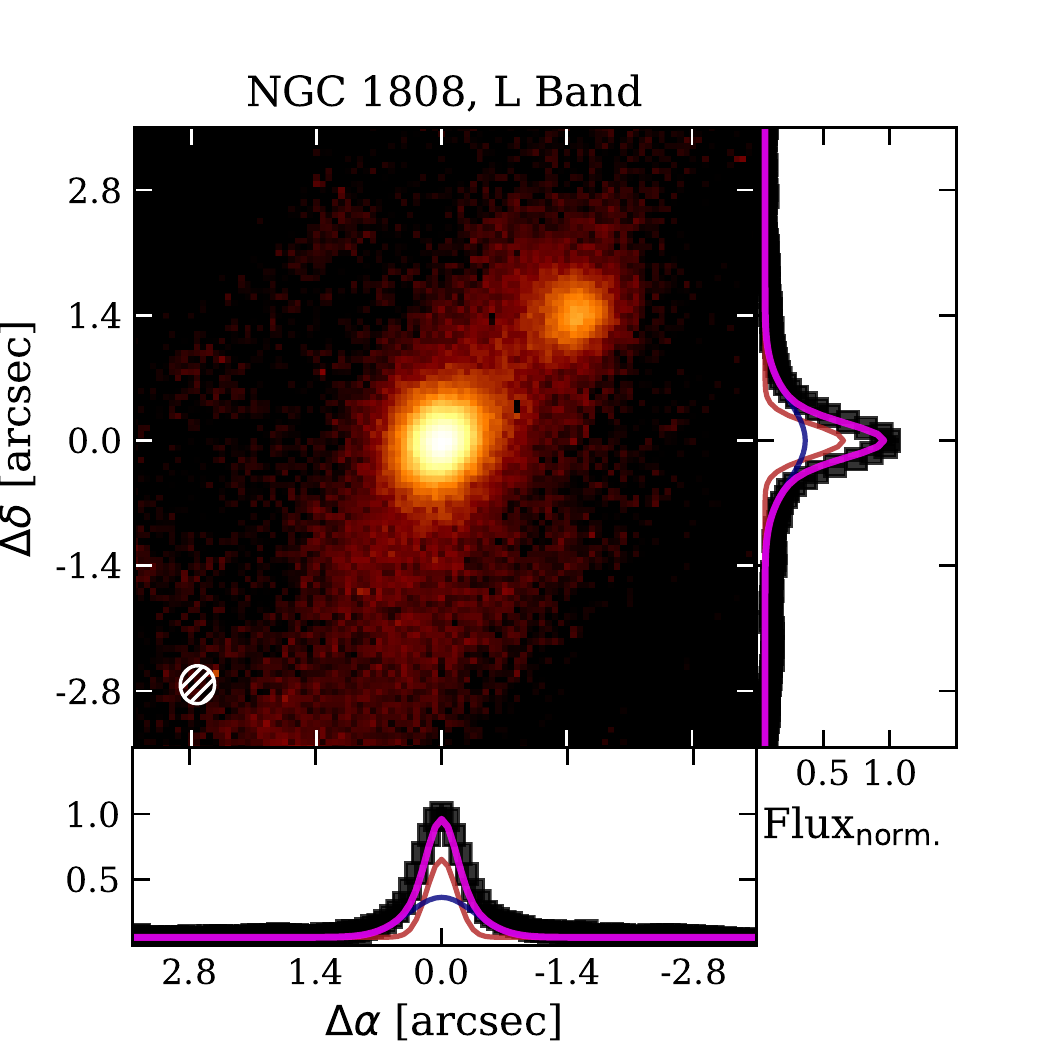}}
\subfloat{\includegraphics[width=0.25\hsize]{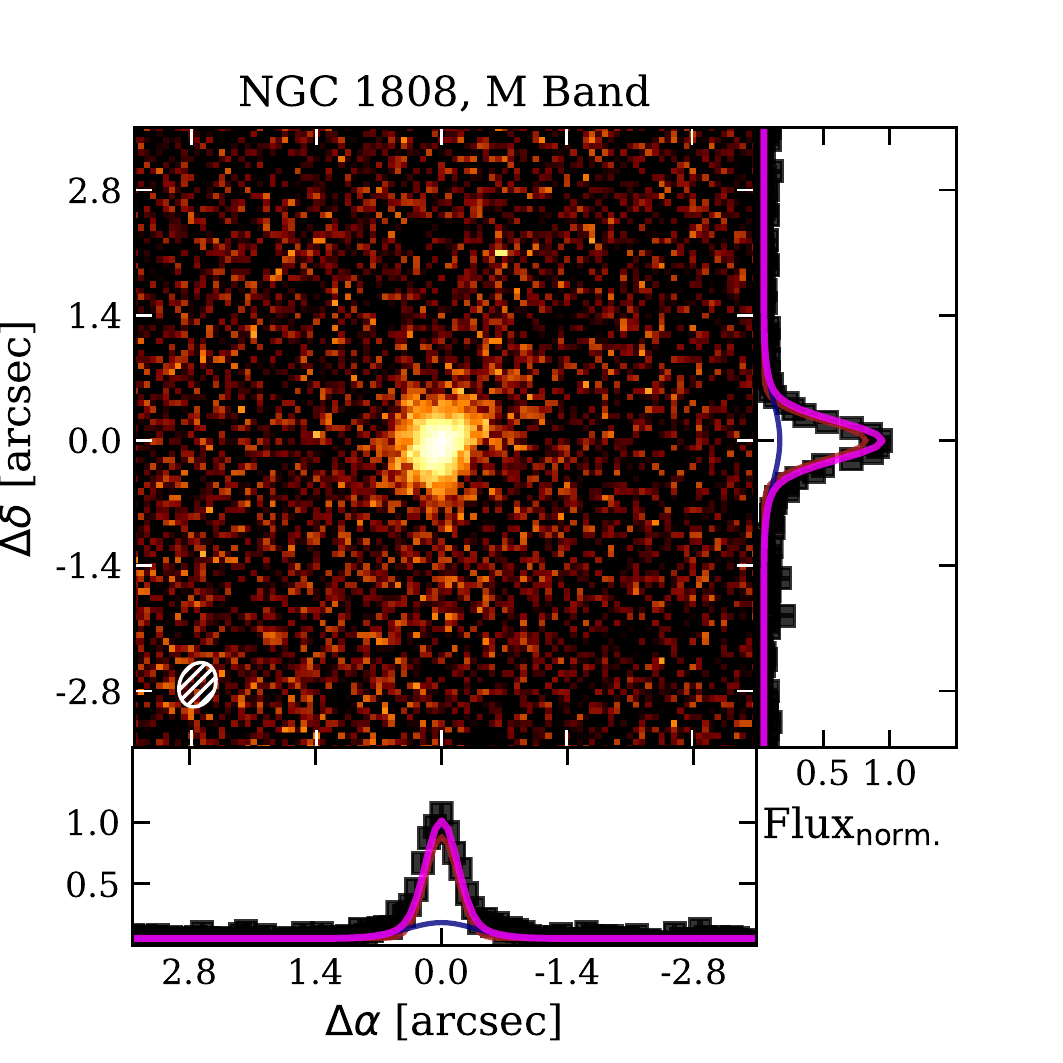}} 
\subfloat{\includegraphics[width=0.25\hsize]{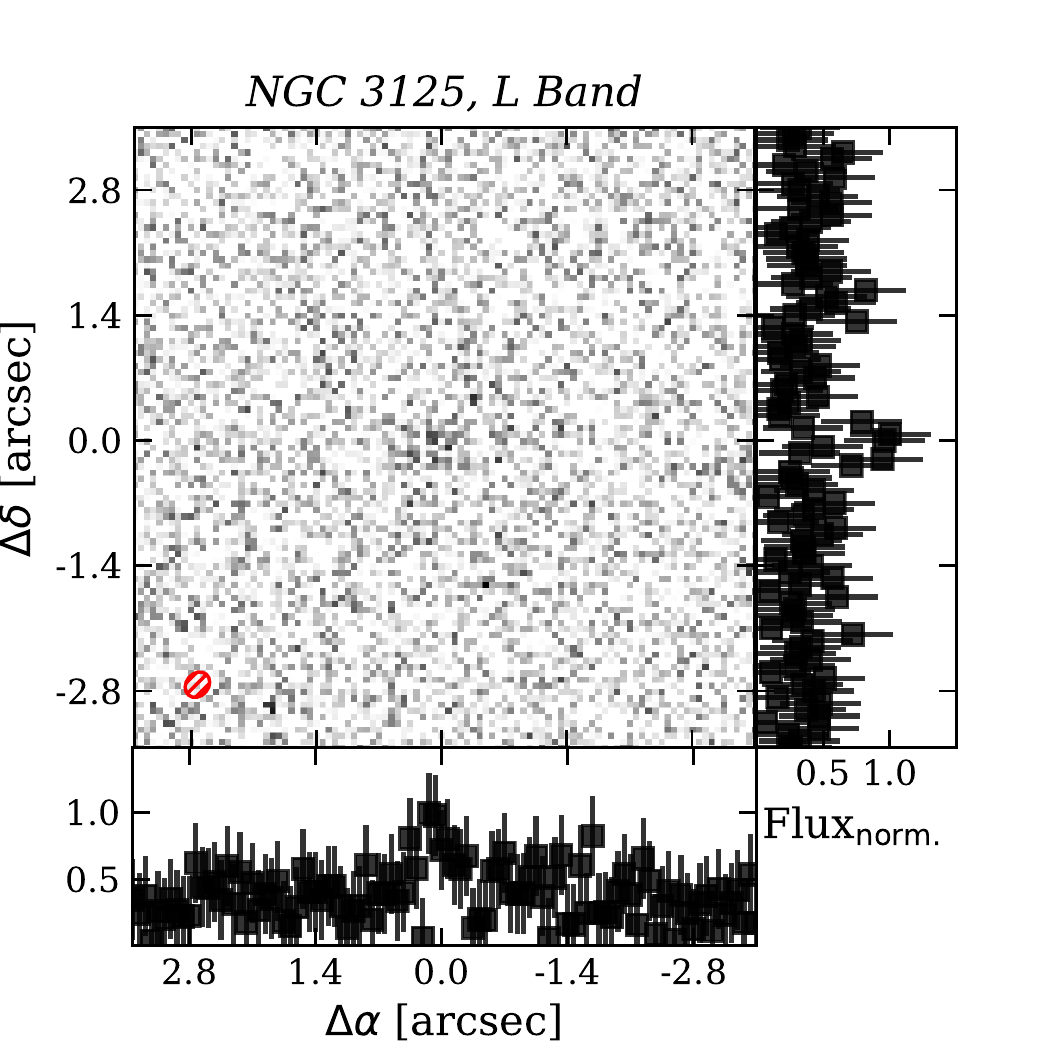}}
\subfloat{\includegraphics[width=0.25\hsize]{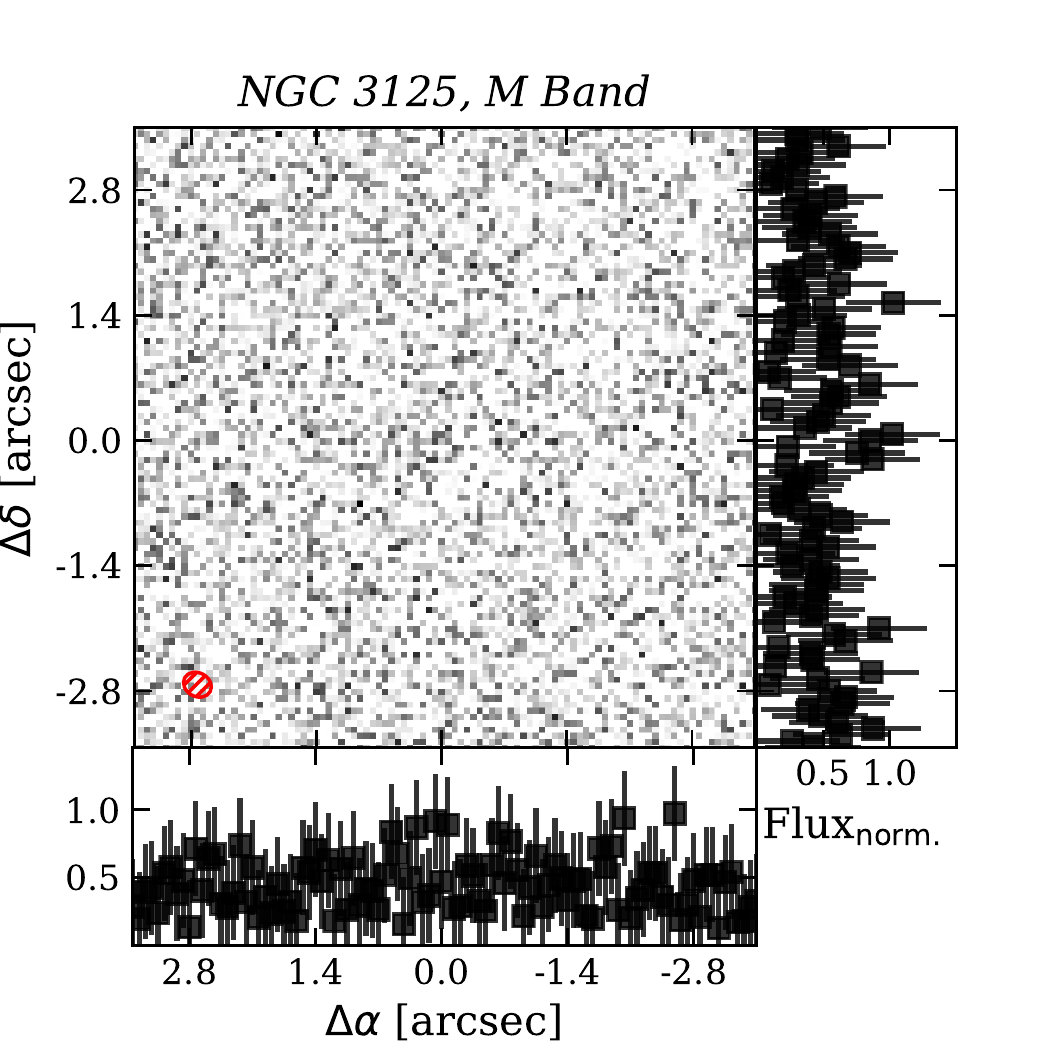}}\\
\subfloat{\includegraphics[width=0.25\hsize]{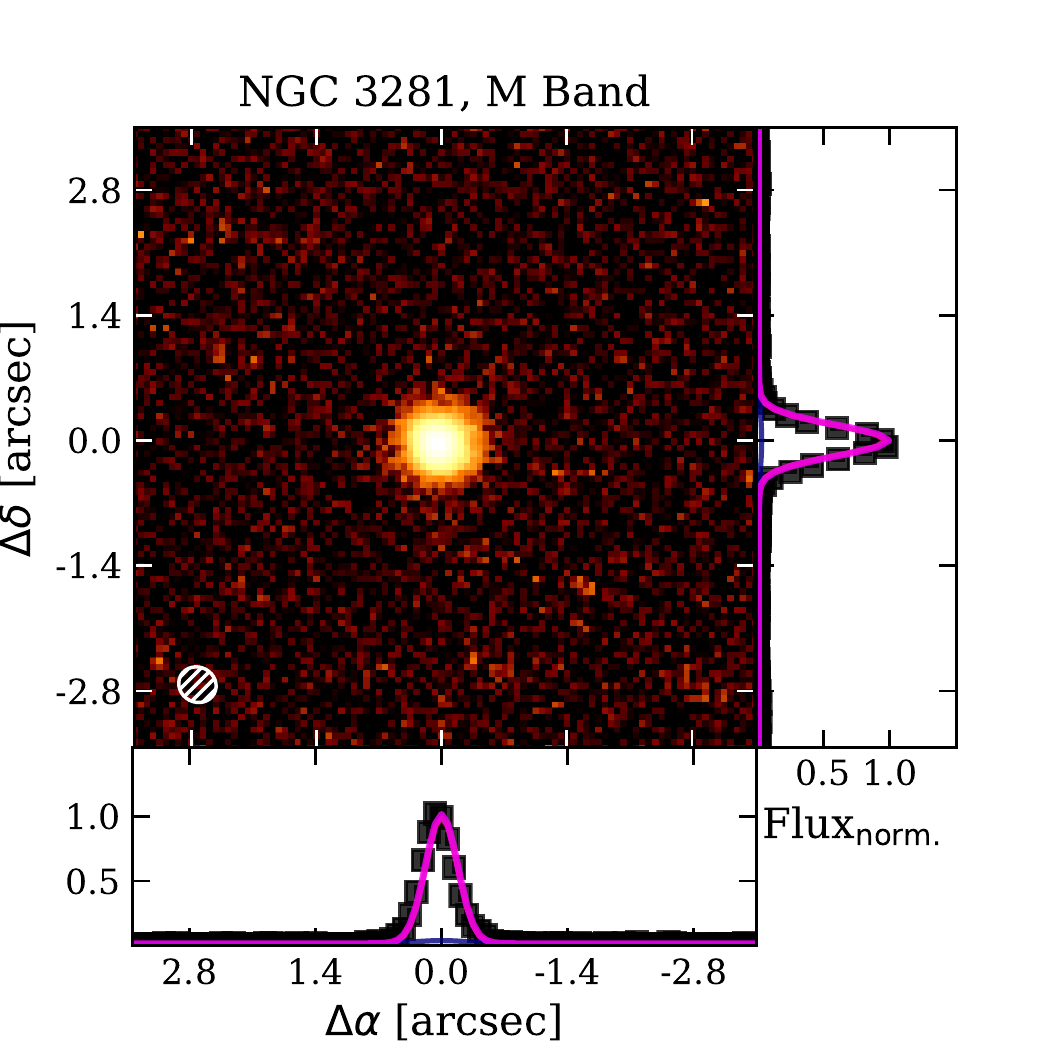}}
\subfloat{\includegraphics[width=0.25\hsize]{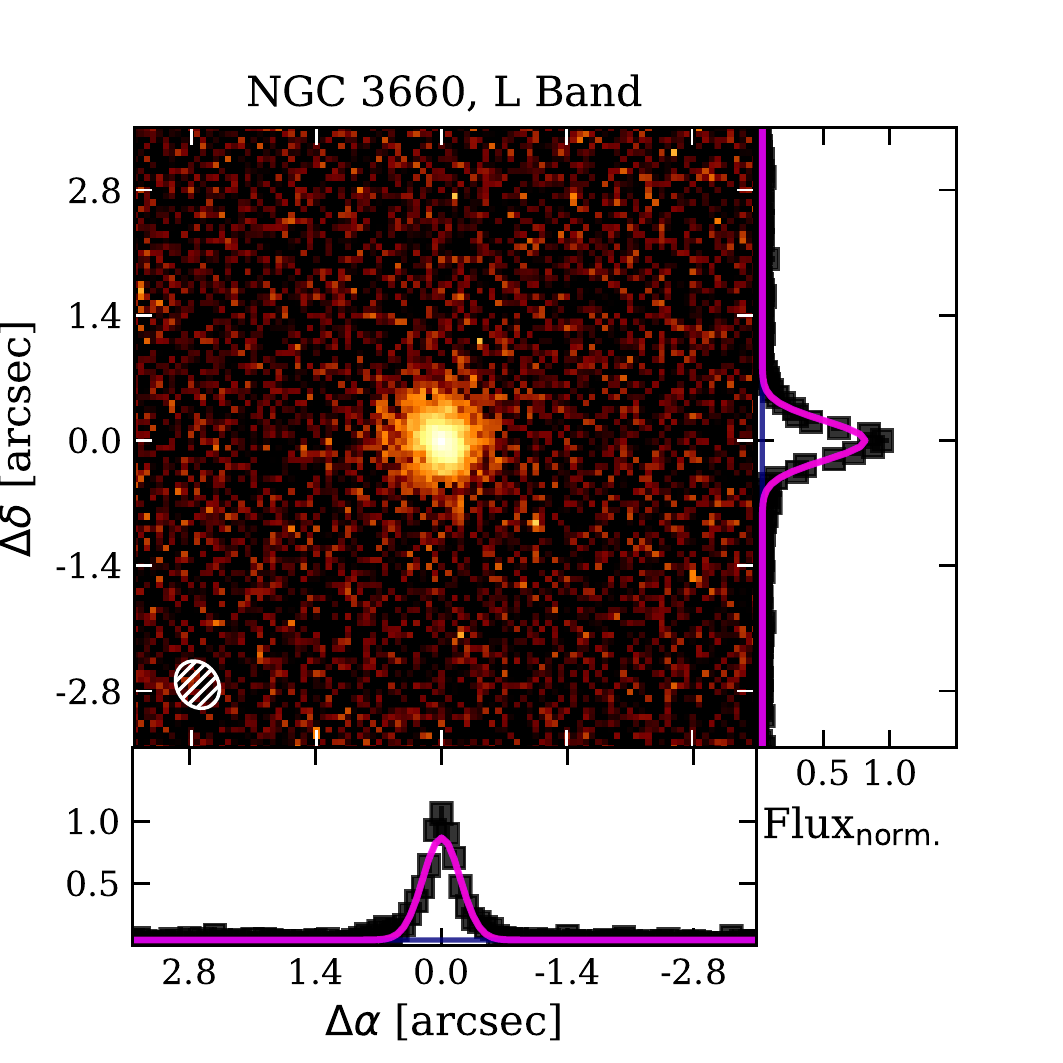}} 
\subfloat{\includegraphics[width=0.25\hsize]{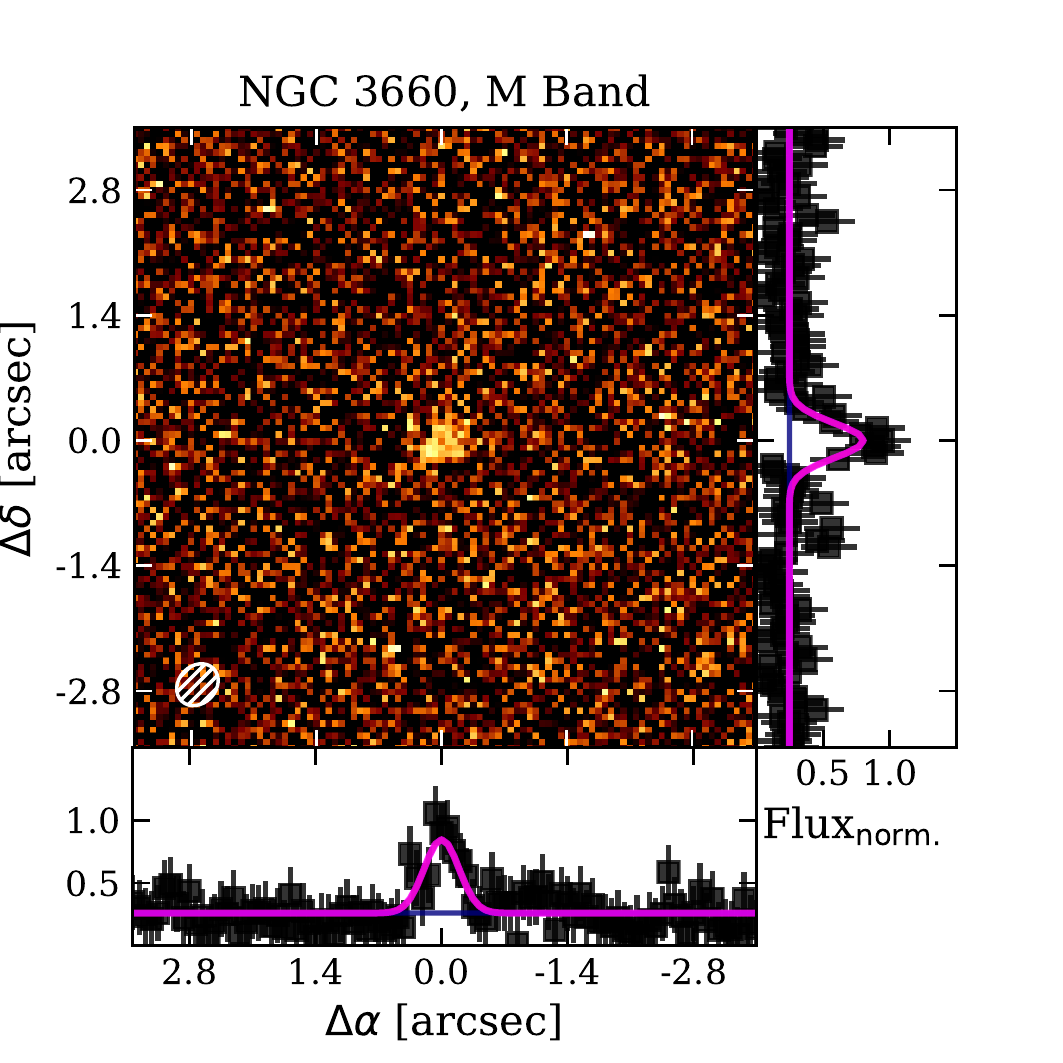}}
\subfloat{\includegraphics[width=0.25\hsize]{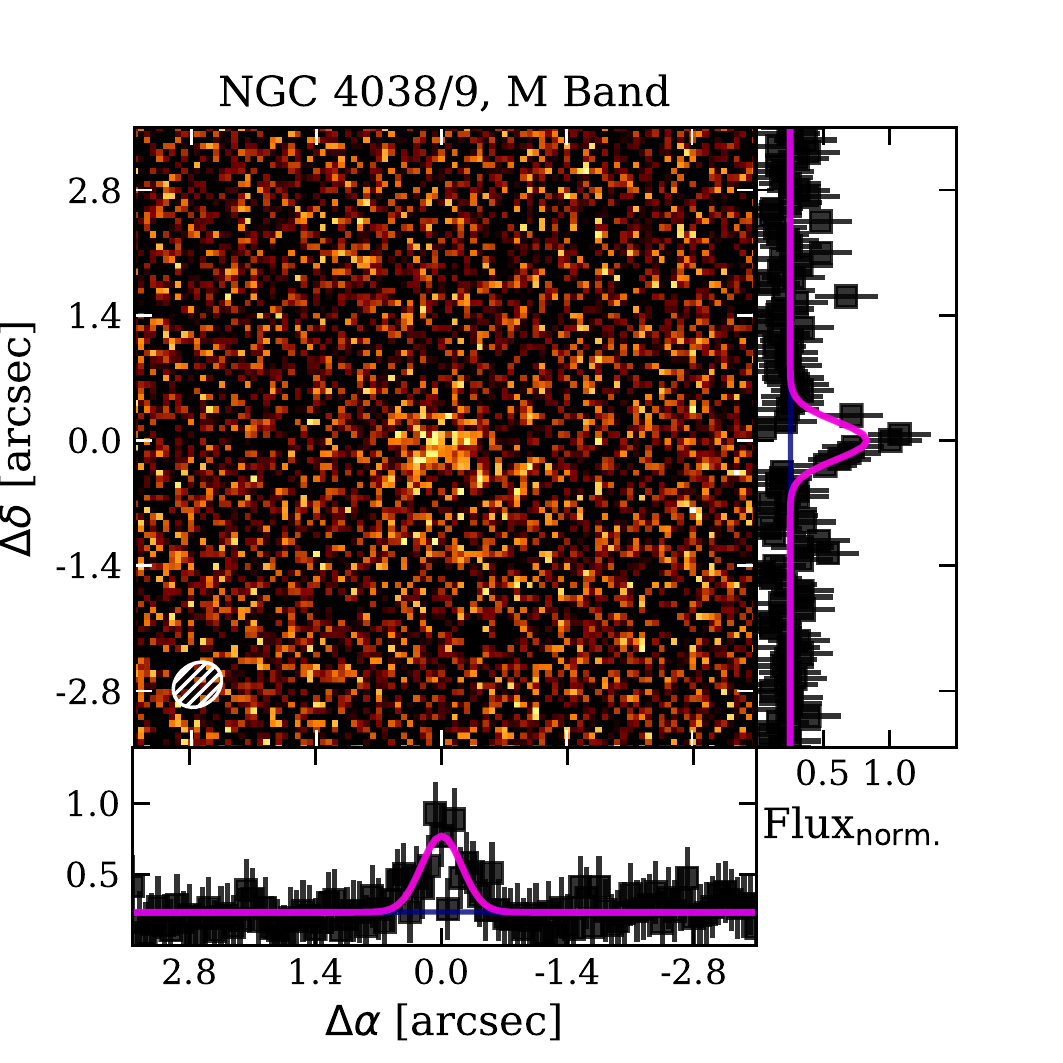}}\\
\subfloat{\includegraphics[width=0.25\hsize]{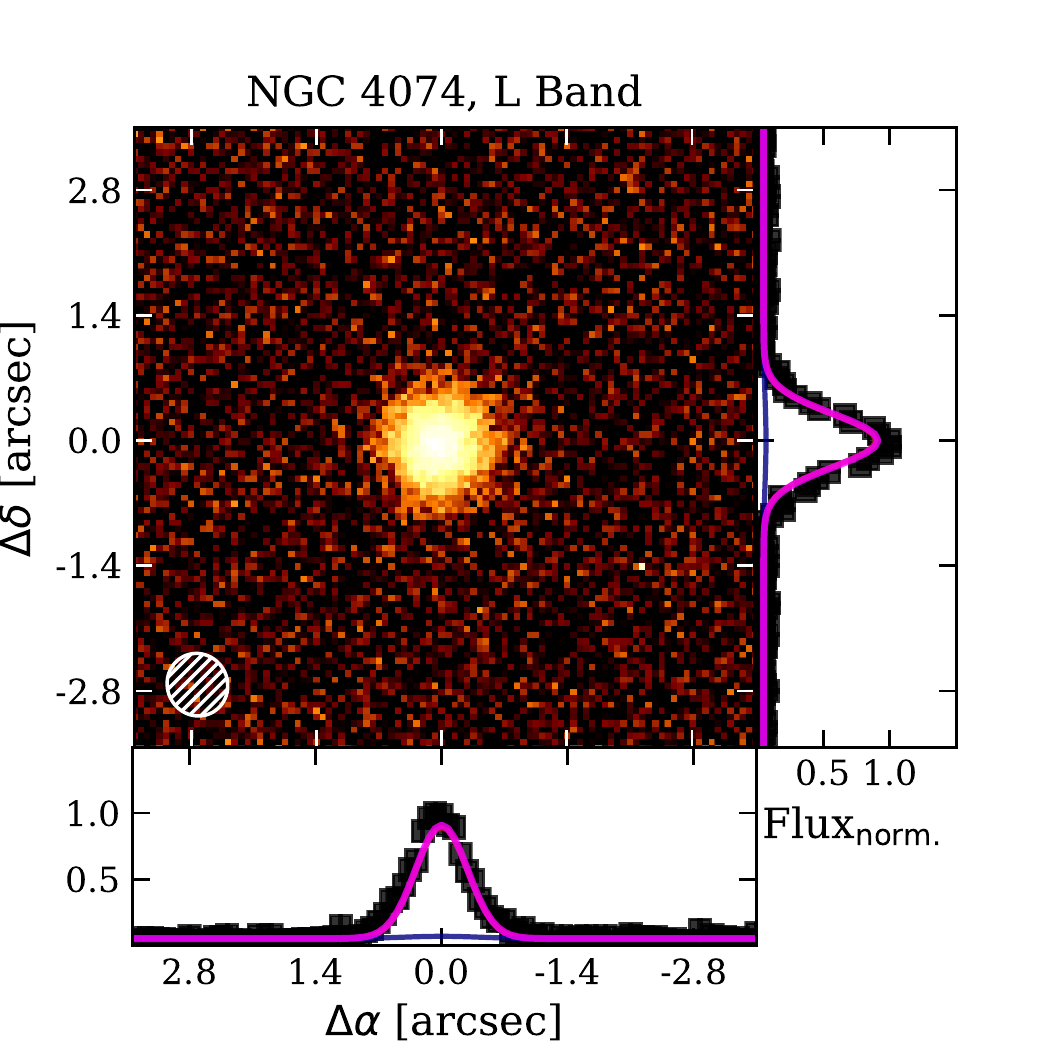}}
\subfloat{\includegraphics[width=0.25\hsize]{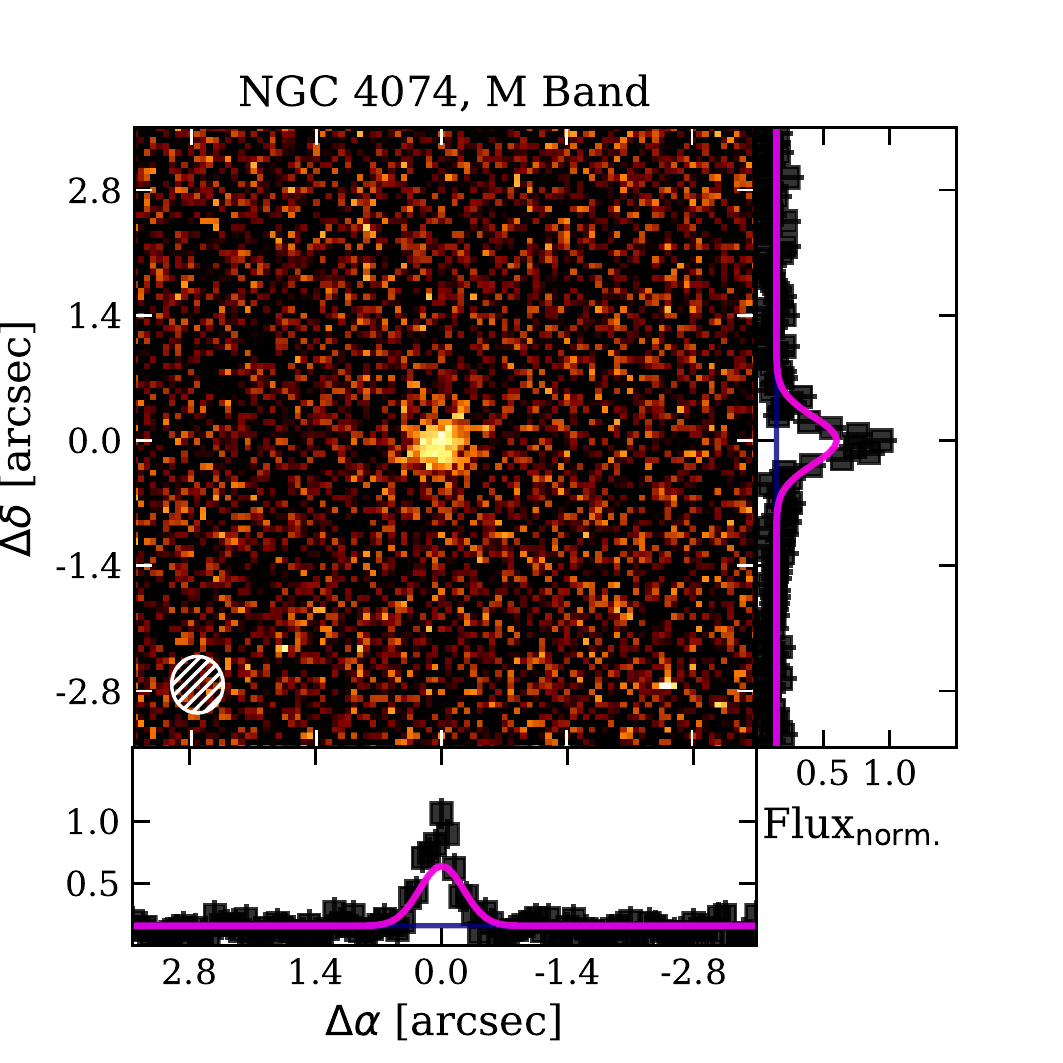}} 
\subfloat{\includegraphics[width=0.25\hsize]{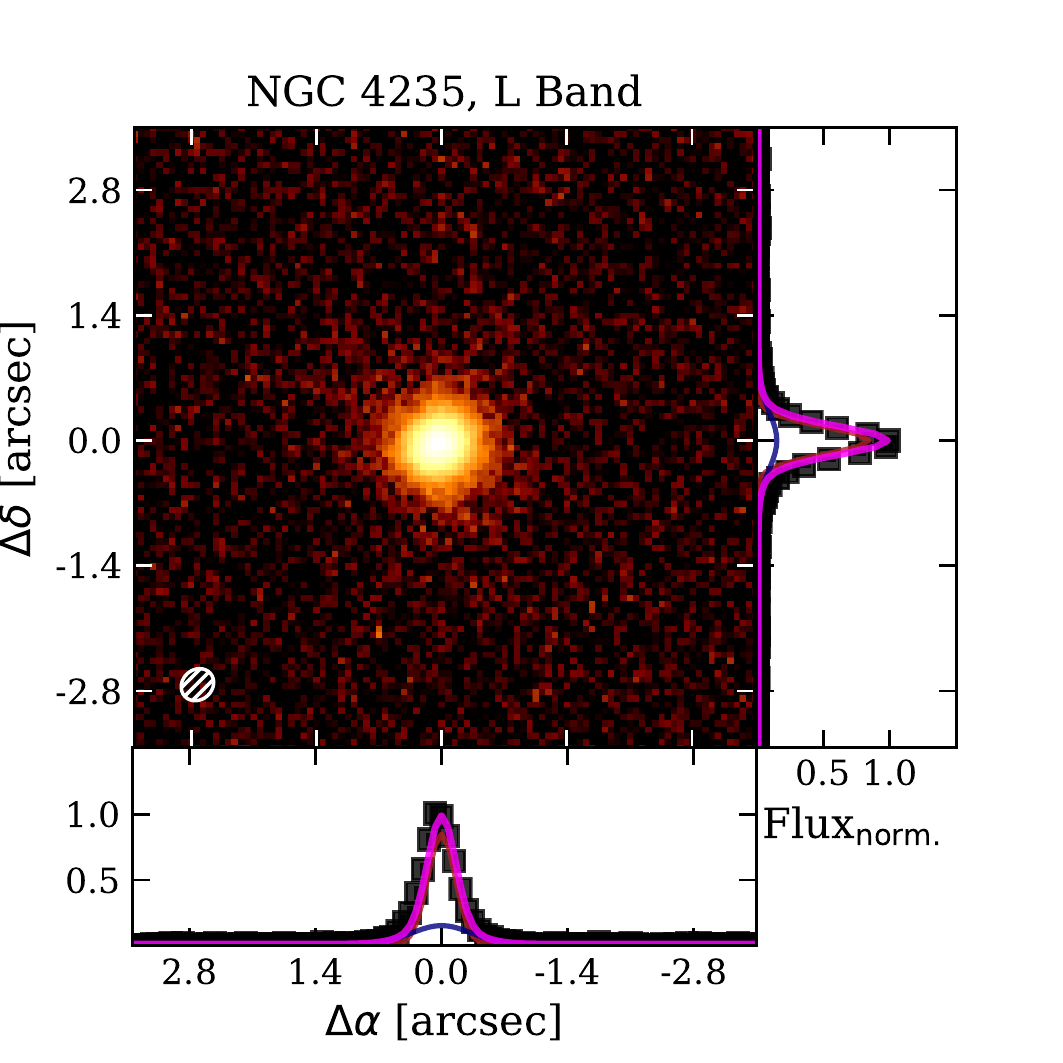}}
\subfloat{\includegraphics[width=0.25\hsize]{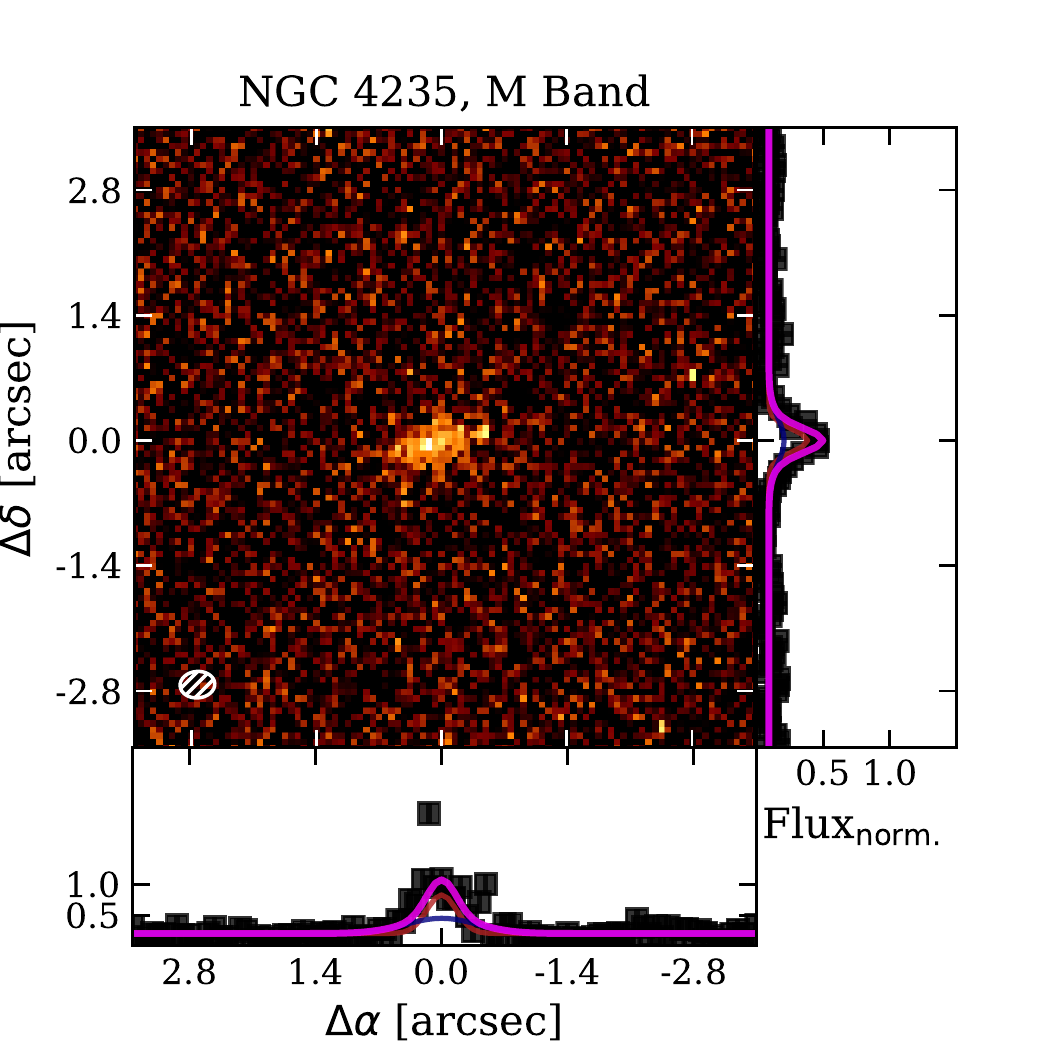}}\\
\subfloat{\includegraphics[width=0.25\hsize]{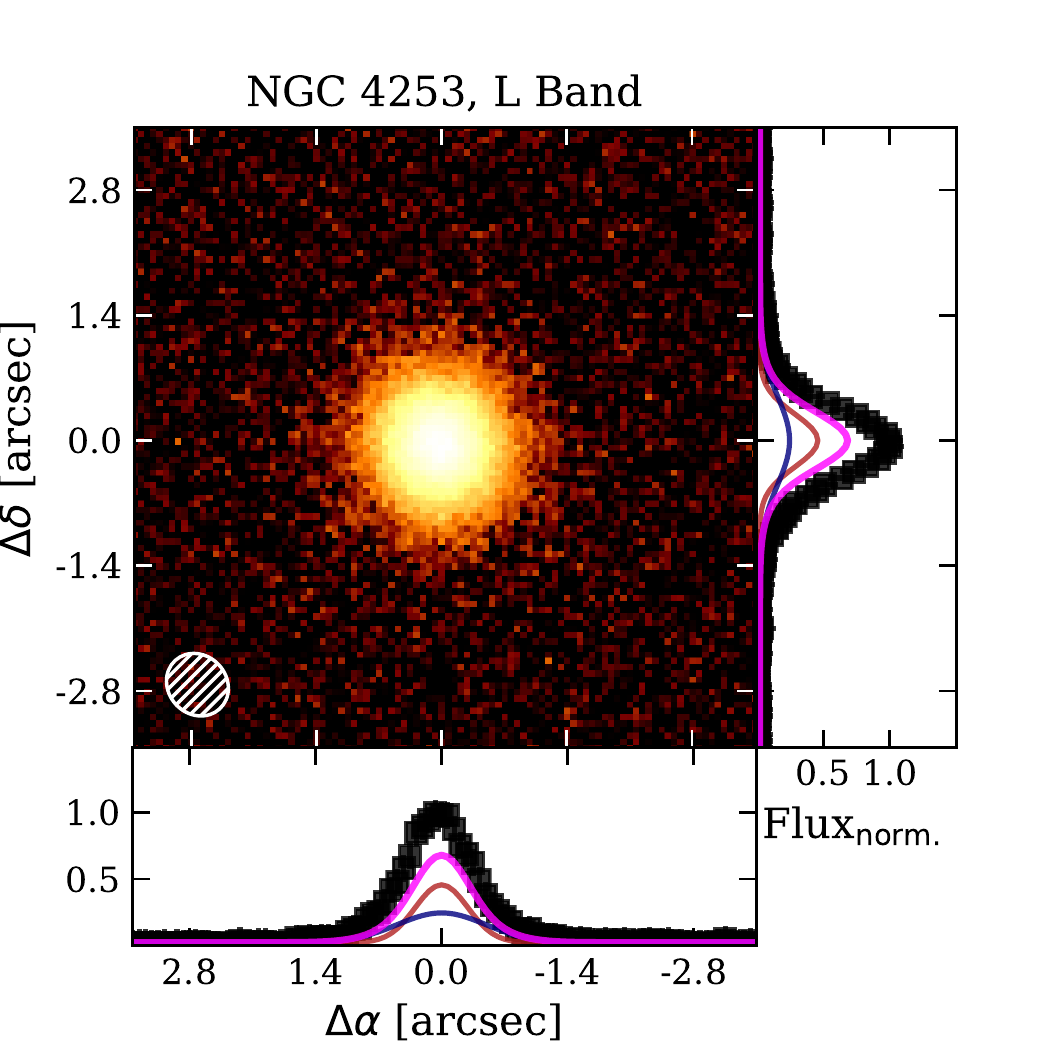}}
\subfloat{\includegraphics[width=0.25\hsize]{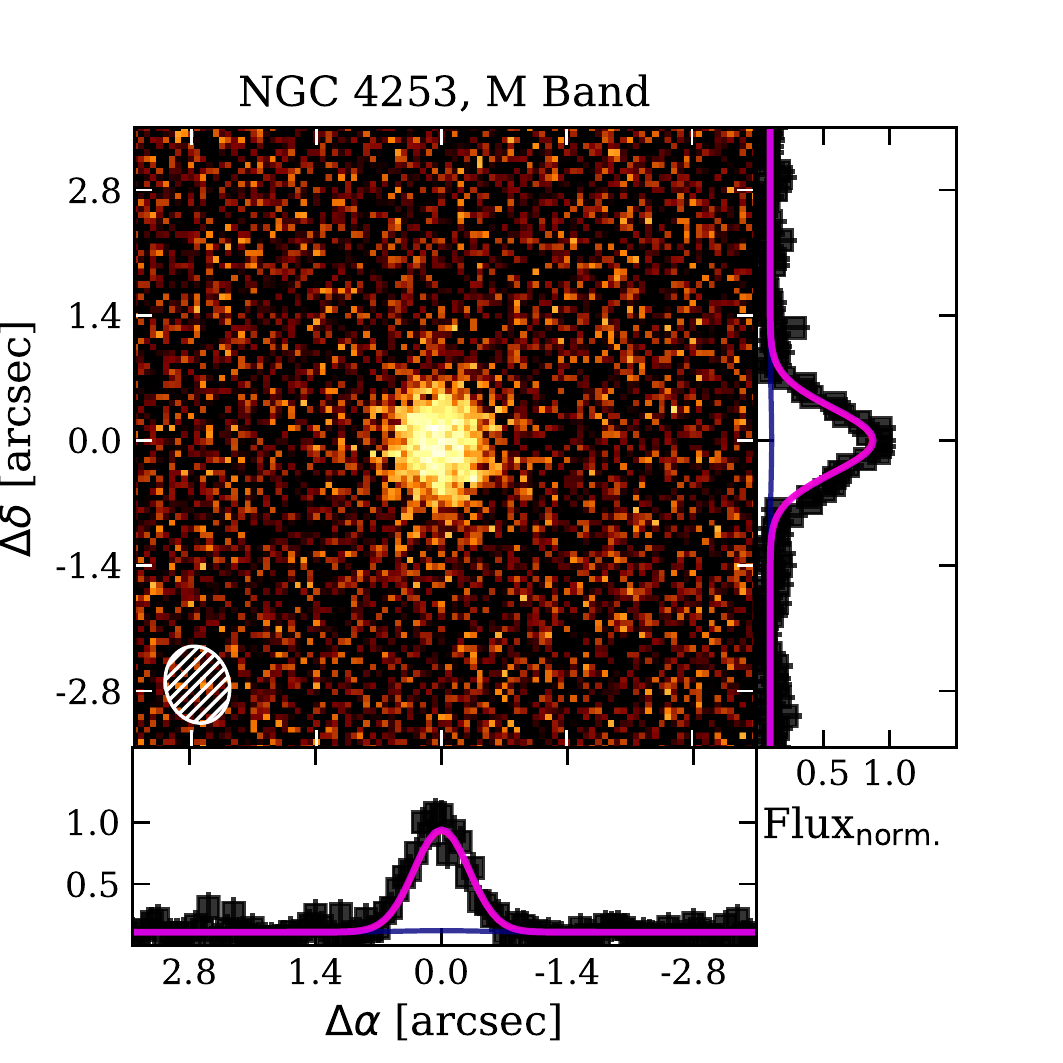}} 
\subfloat{\includegraphics[width=0.25\hsize]{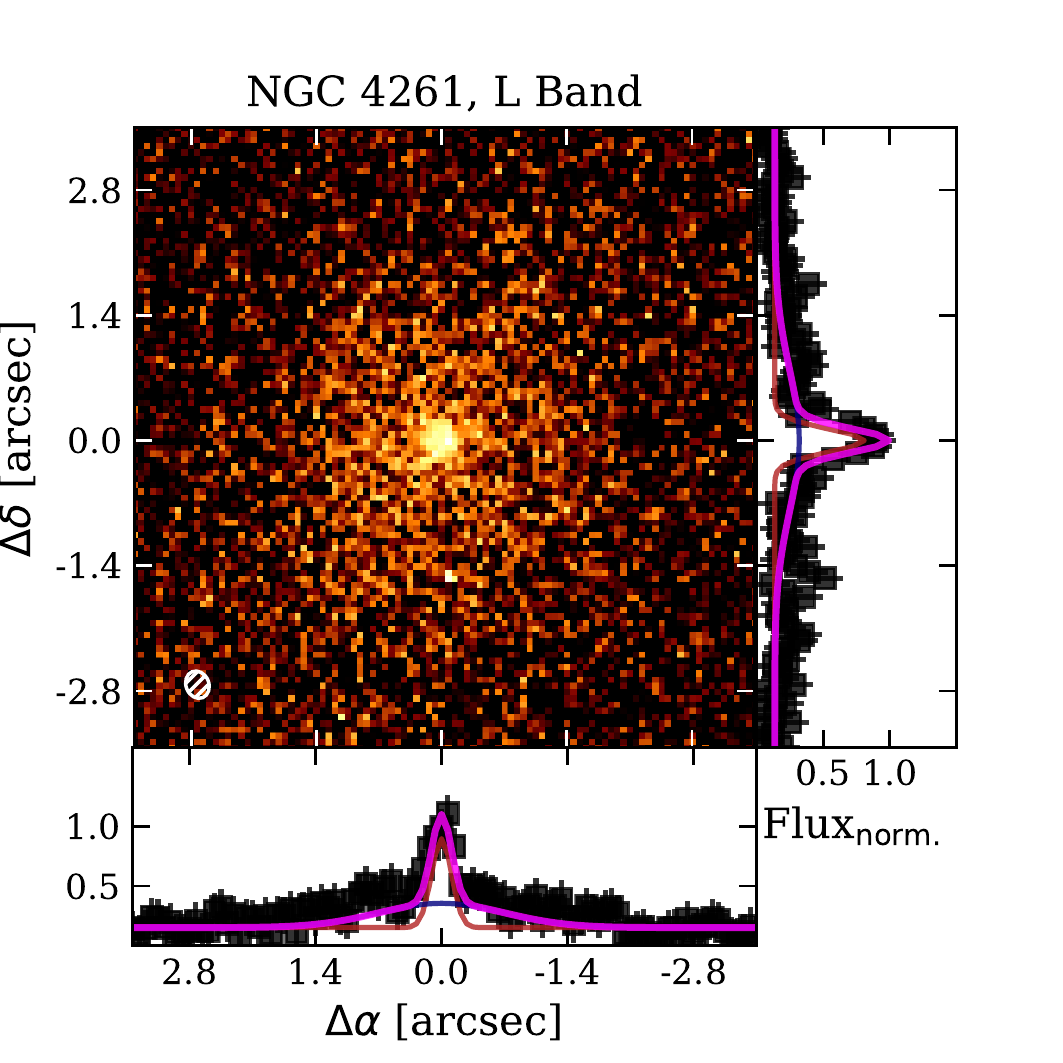}}
\subfloat{\includegraphics[width=0.25\hsize]{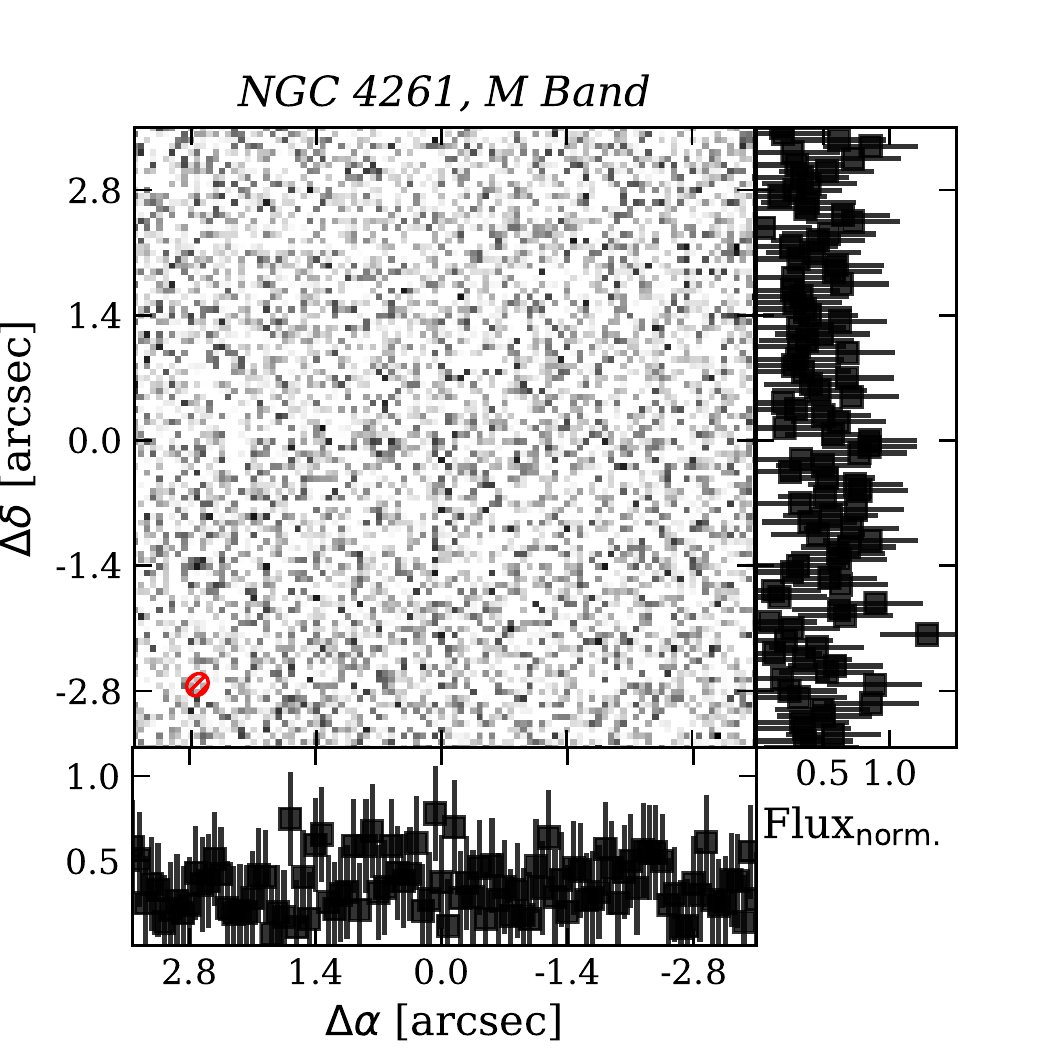}}\\
\subfloat{\includegraphics[width=0.25\hsize]{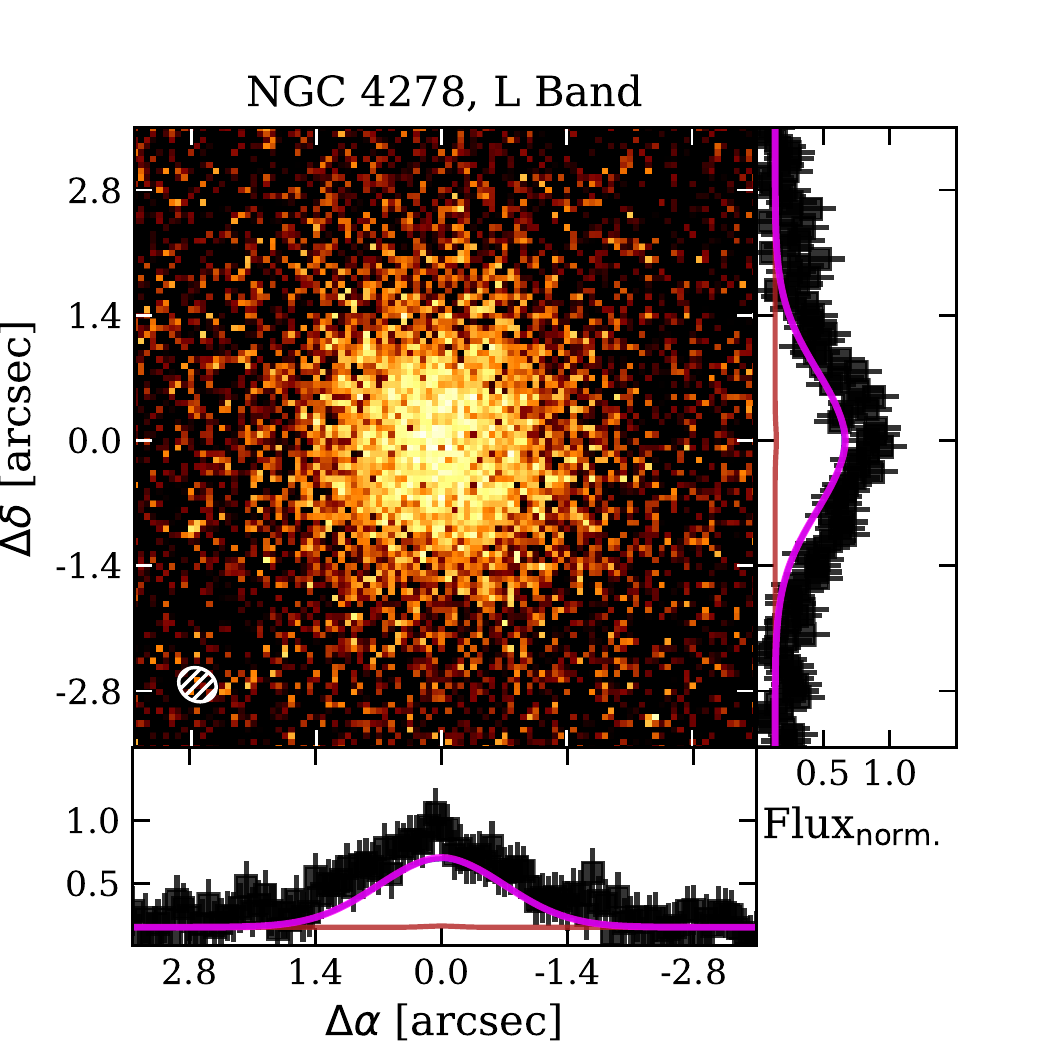}}
\subfloat{\includegraphics[width=0.25\hsize]{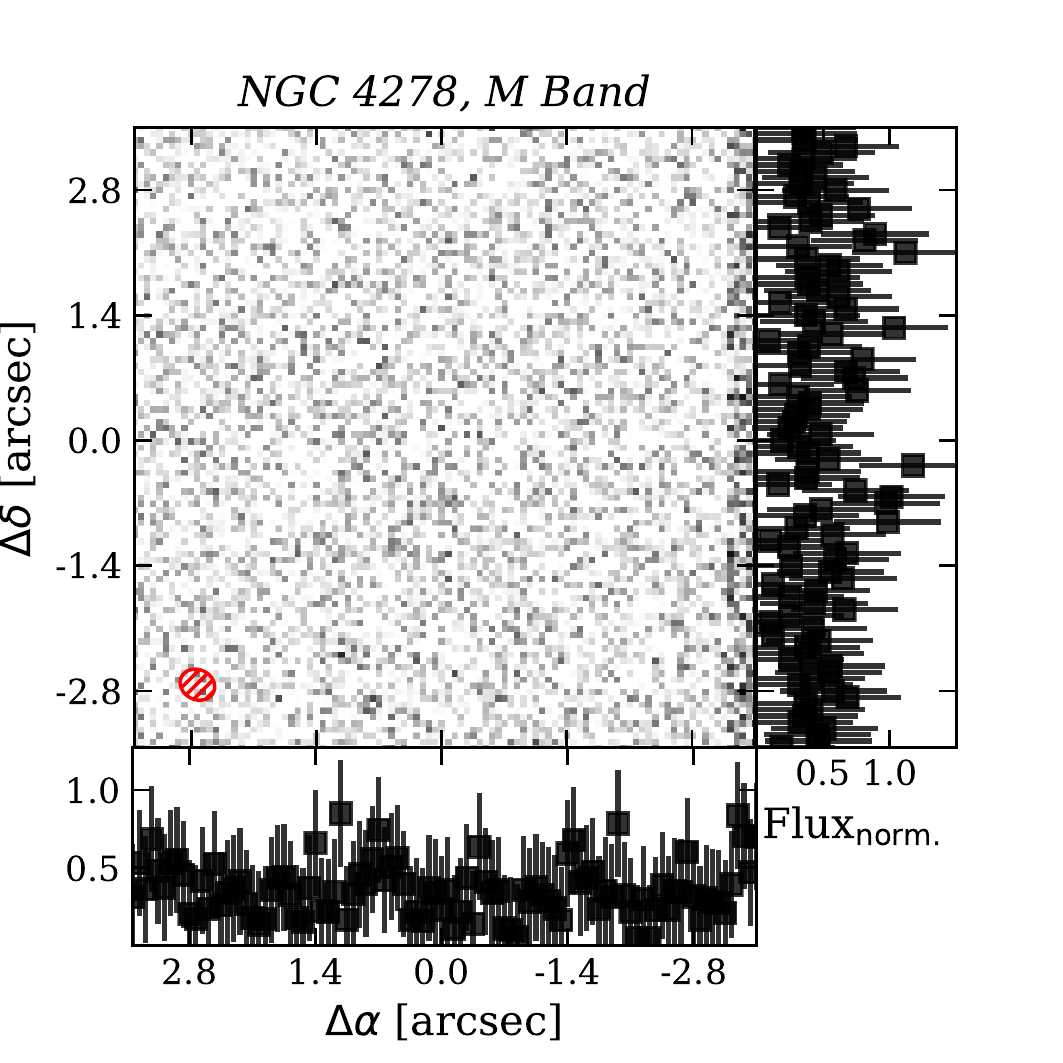}} 
\subfloat{\includegraphics[width=0.25\hsize]{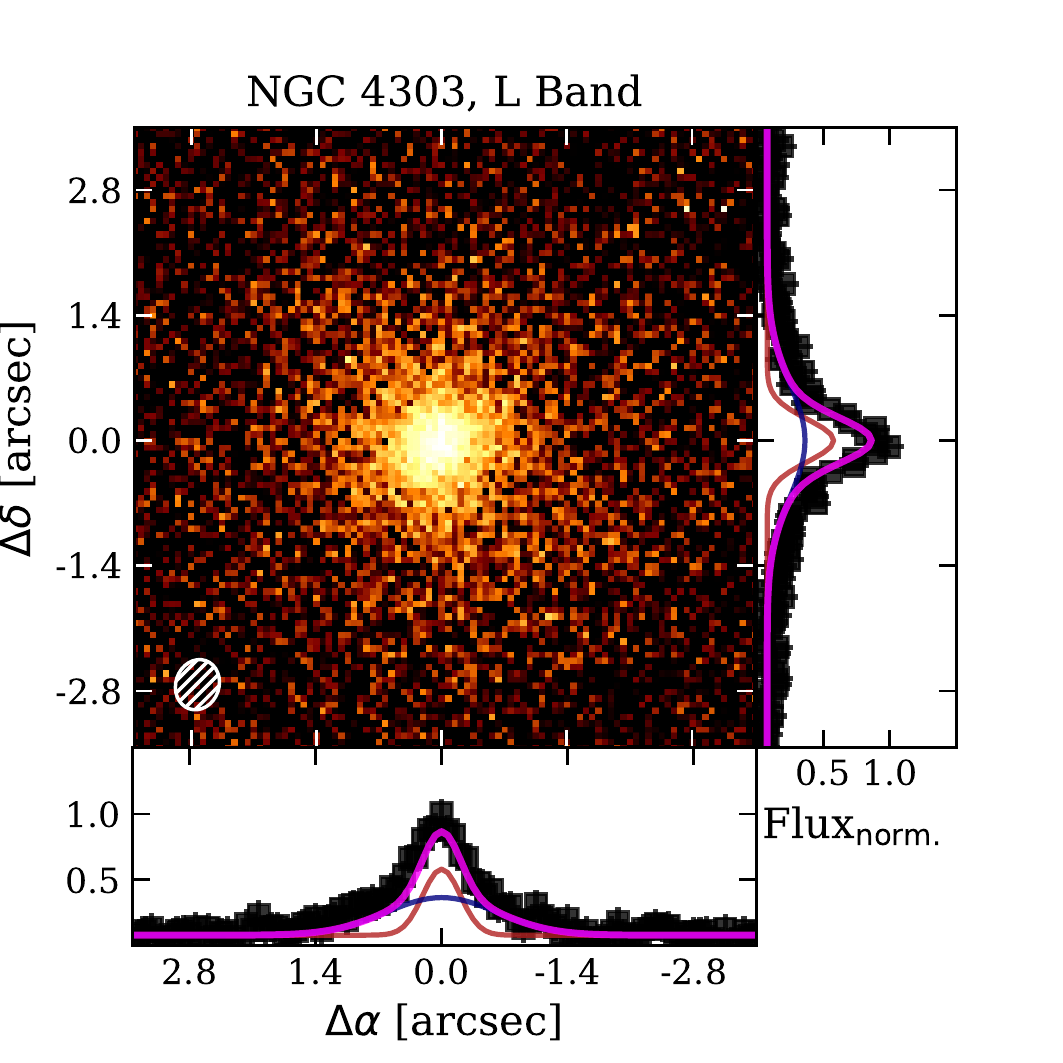}}
\subfloat{\includegraphics[width=0.25\hsize]{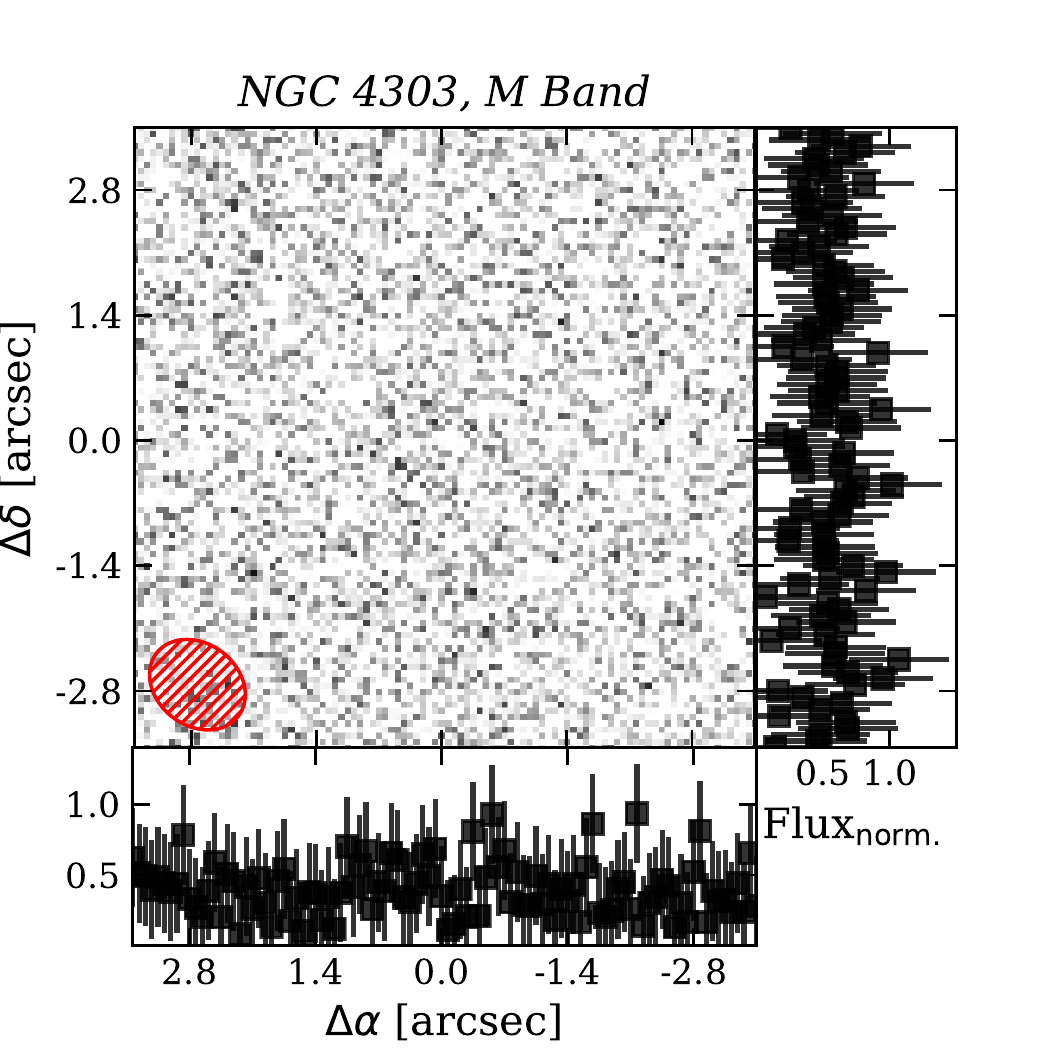}}\\
\caption{ As Fig \ref{fig:cutouts_one} but for all sources.}
\end{figure*}
\begin{figure*}
\subfloat{\includegraphics[width=0.25\hsize]{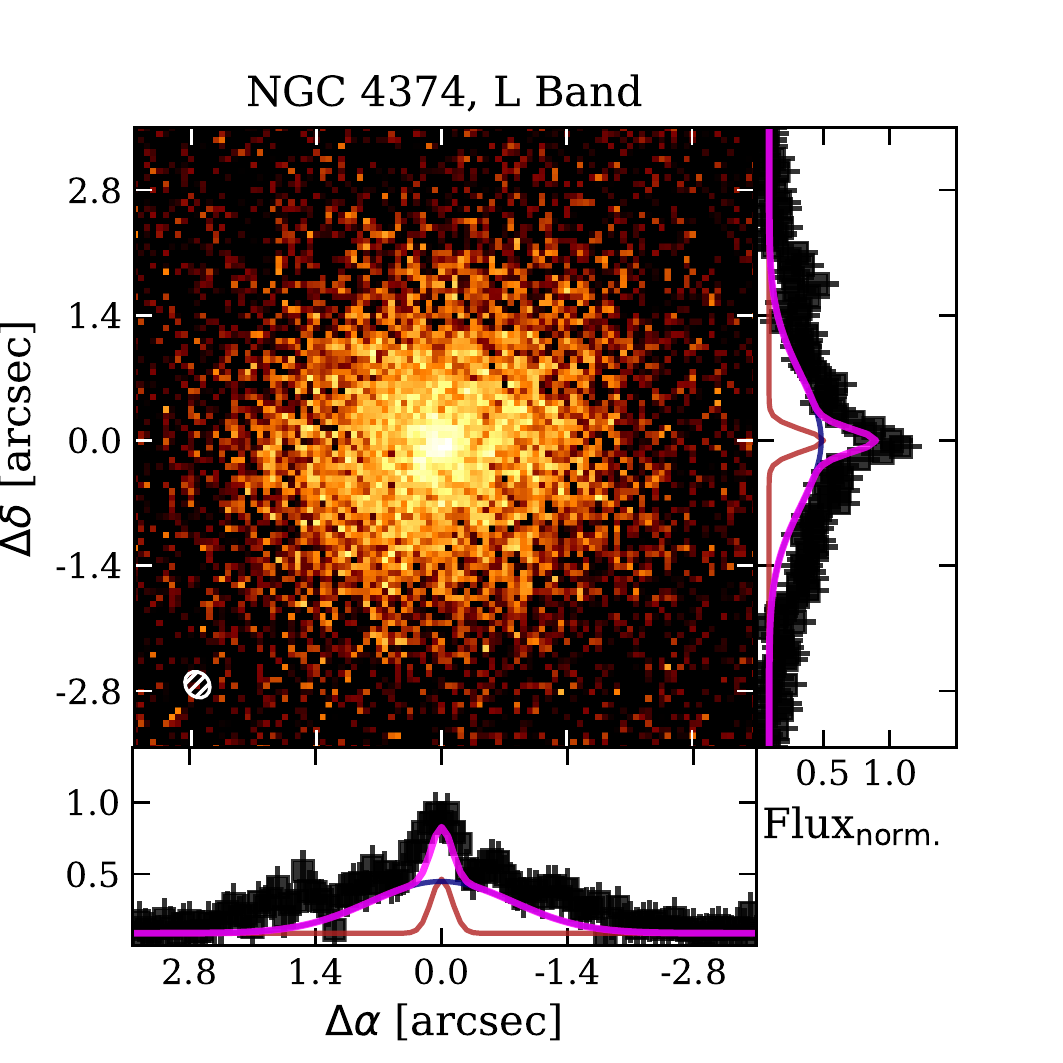}}
\subfloat{\includegraphics[width=0.25\hsize]{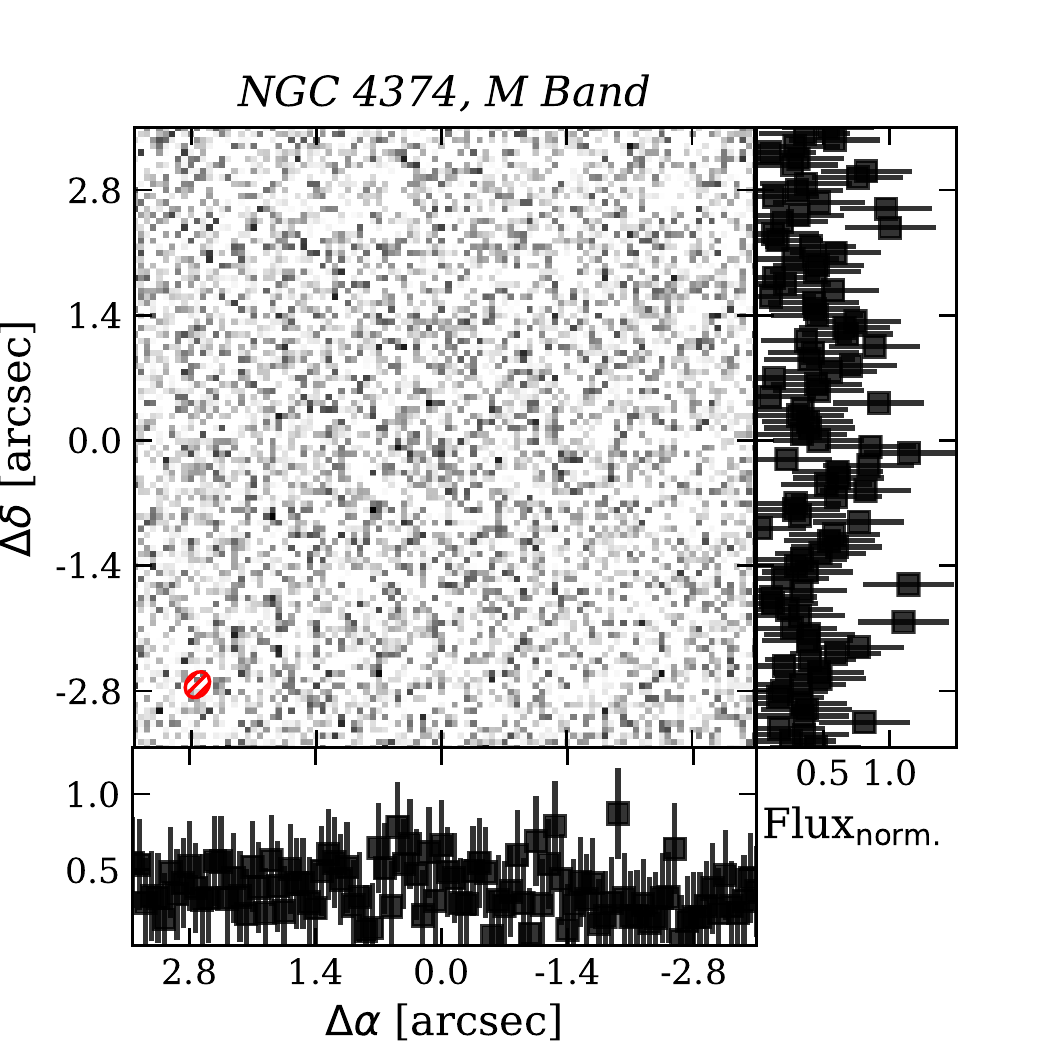}} 
\subfloat{\includegraphics[width=0.25\hsize]{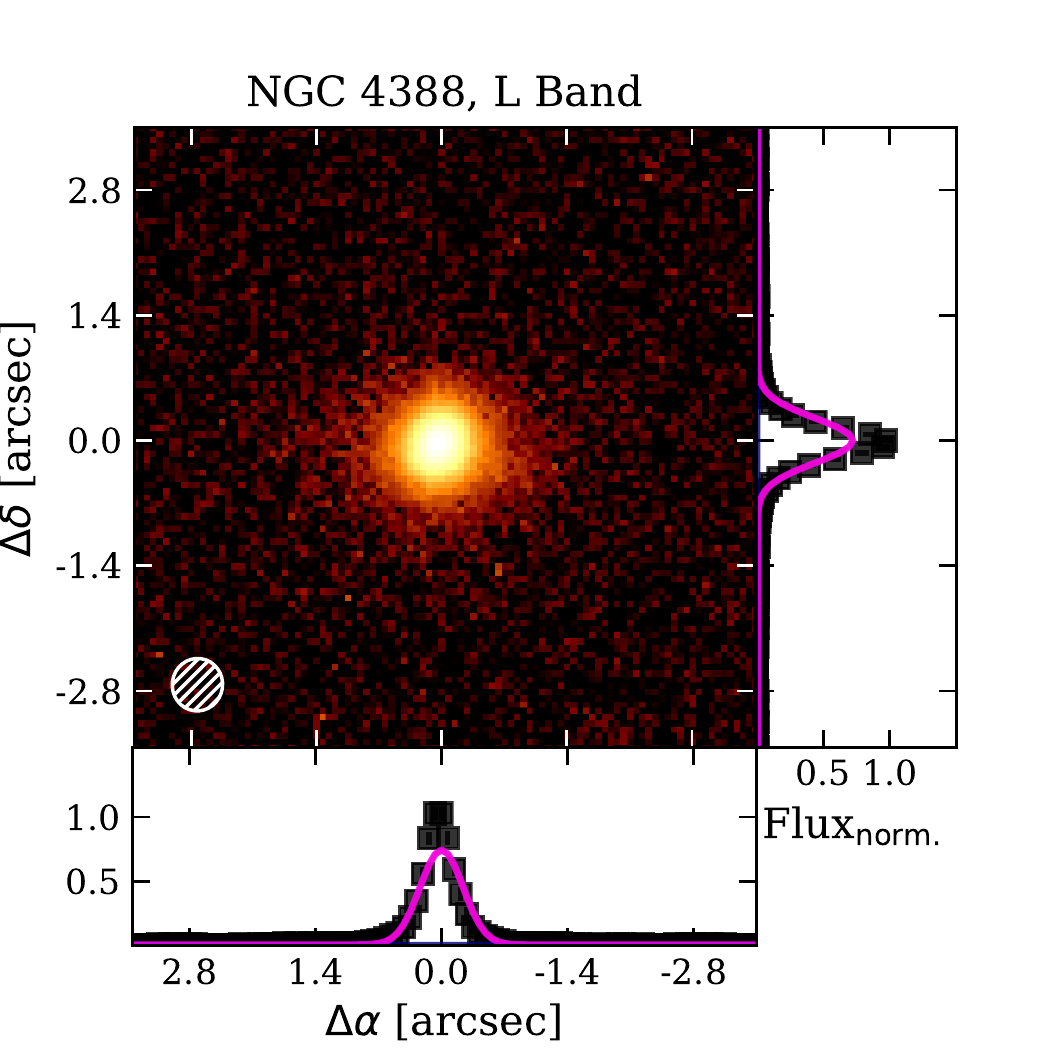}}
\subfloat{\includegraphics[width=0.25\hsize]{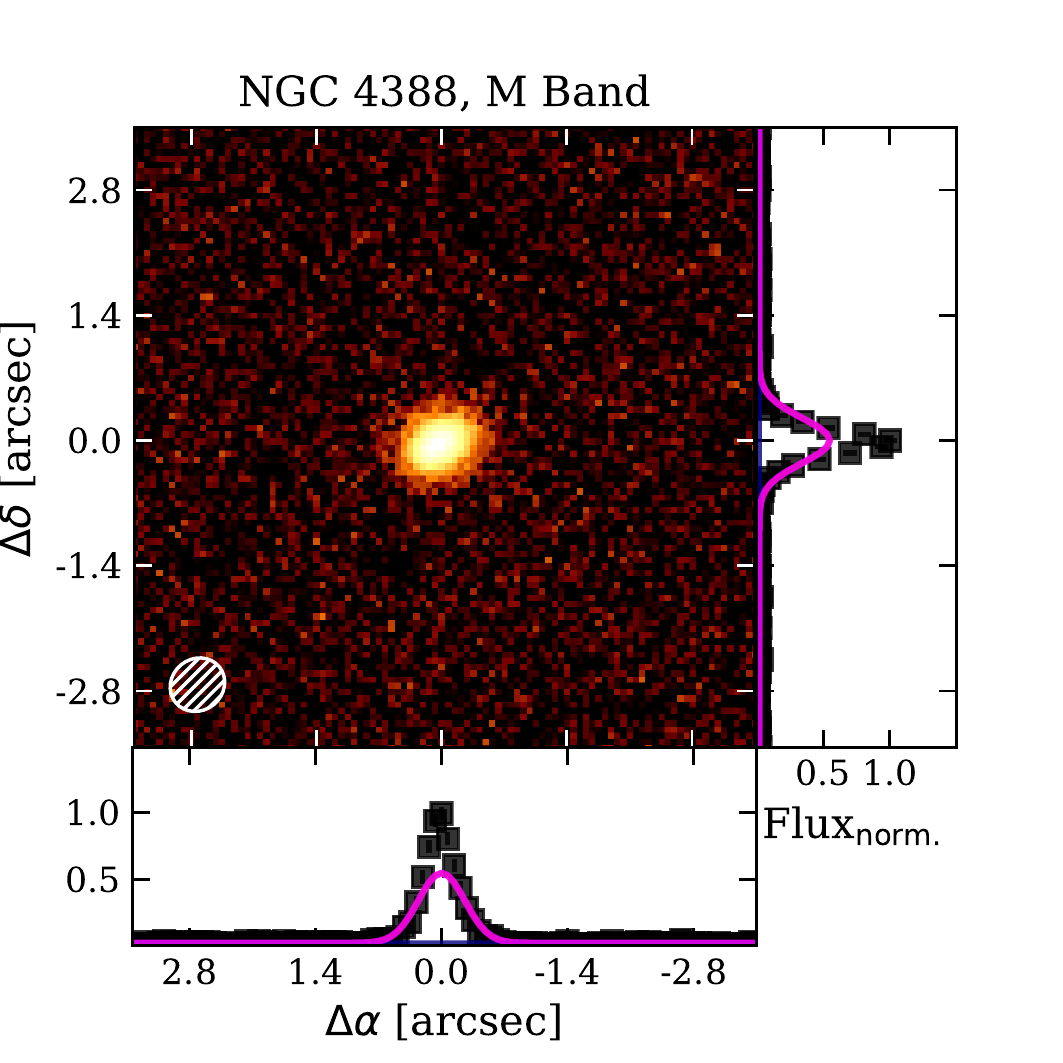}}\\
\subfloat{\includegraphics[width=0.25\hsize]{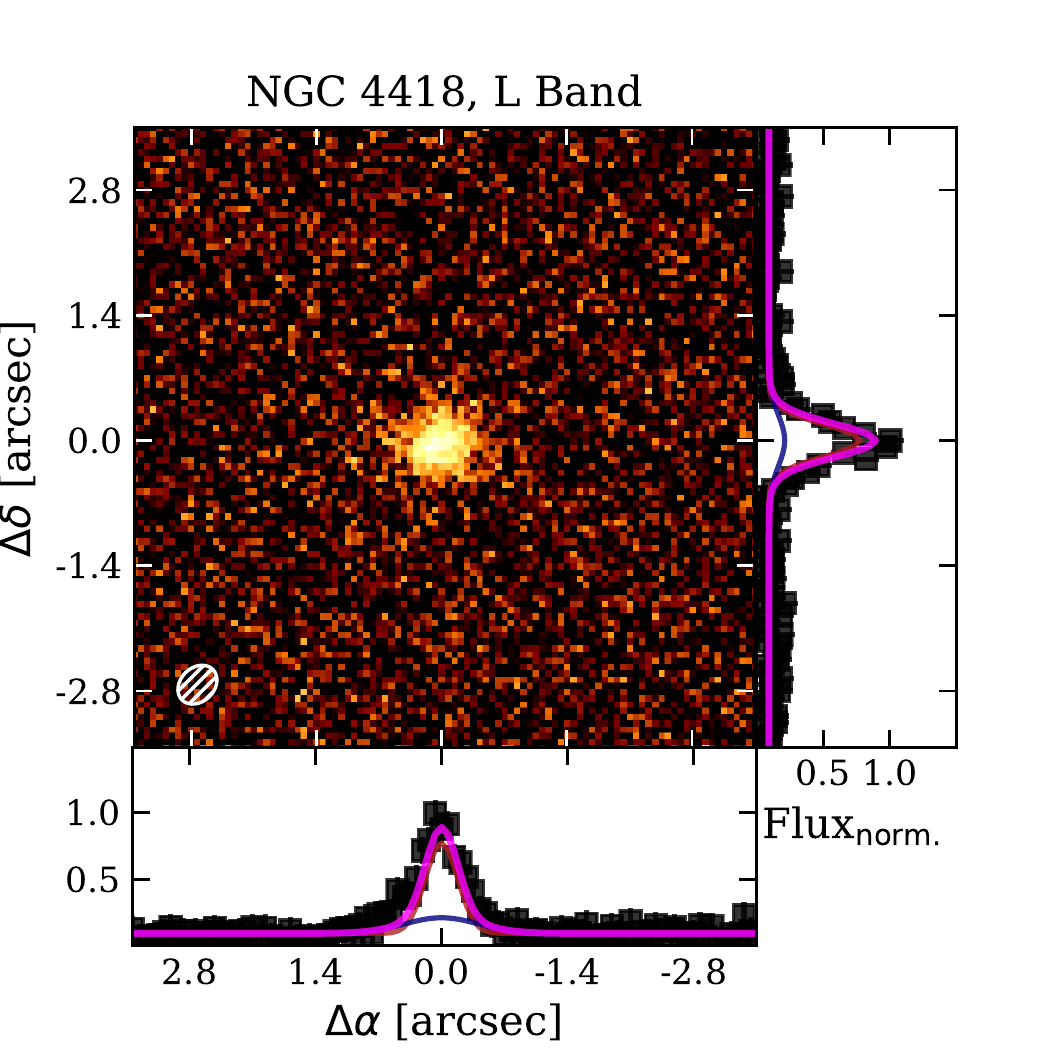}}
\subfloat{\includegraphics[width=0.25\hsize]{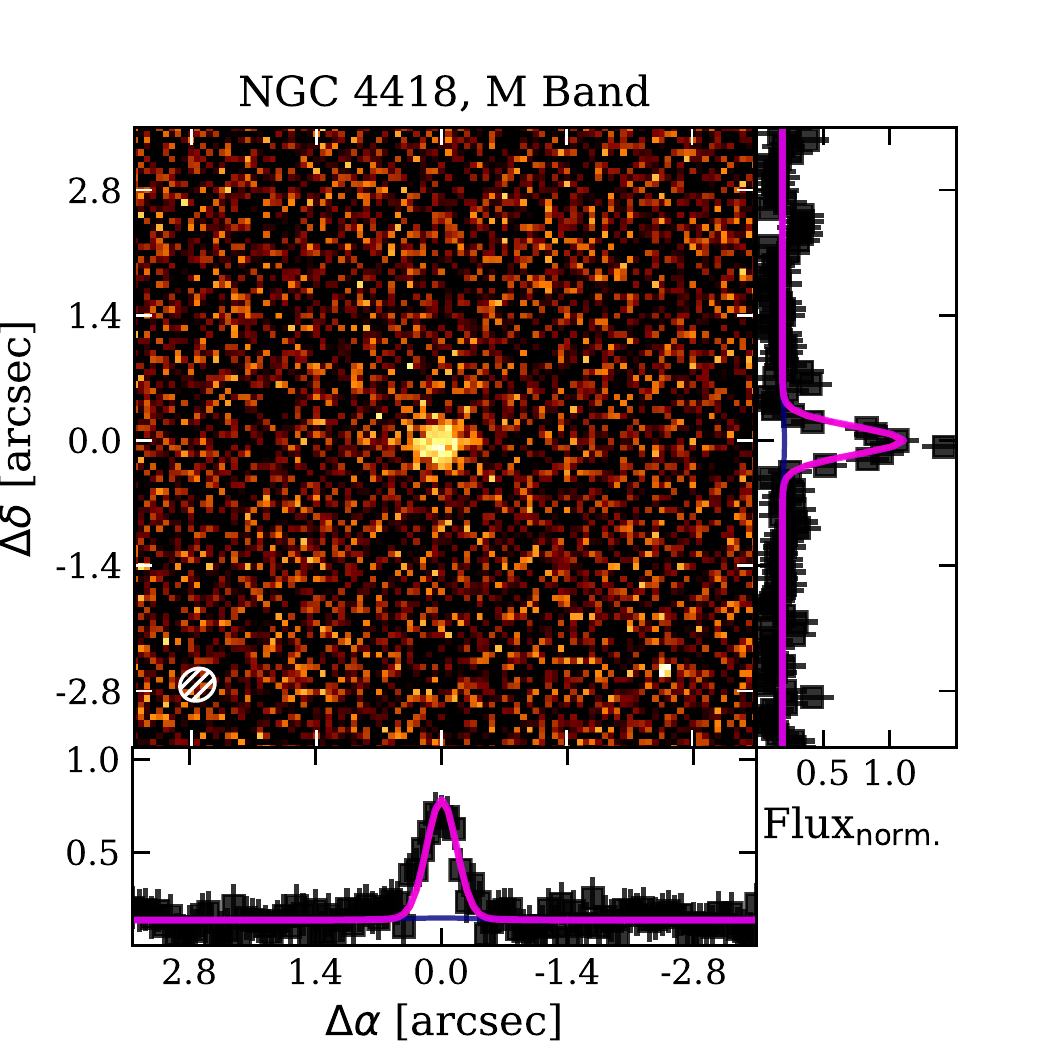}} 
\subfloat{\includegraphics[width=0.25\hsize]{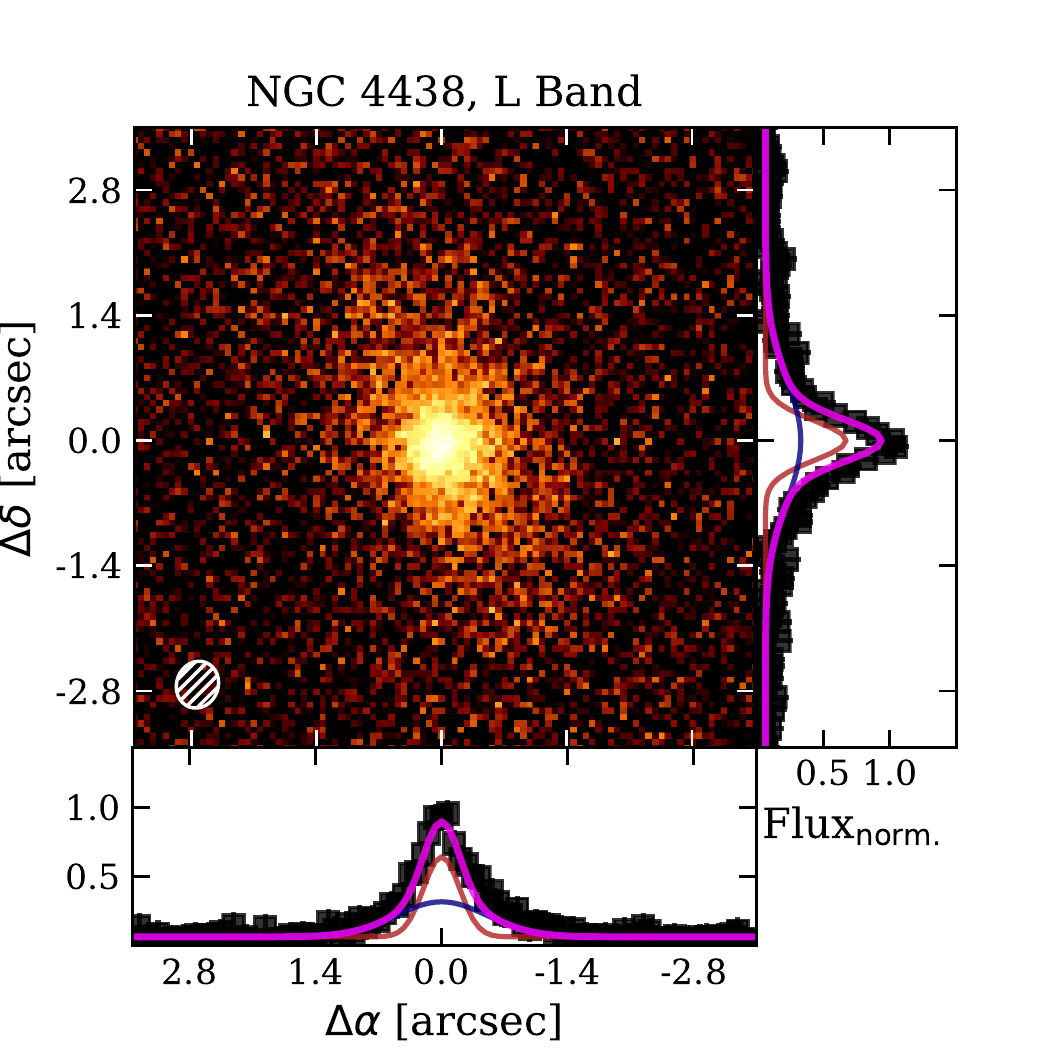}}
\subfloat{\includegraphics[width=0.25\hsize]{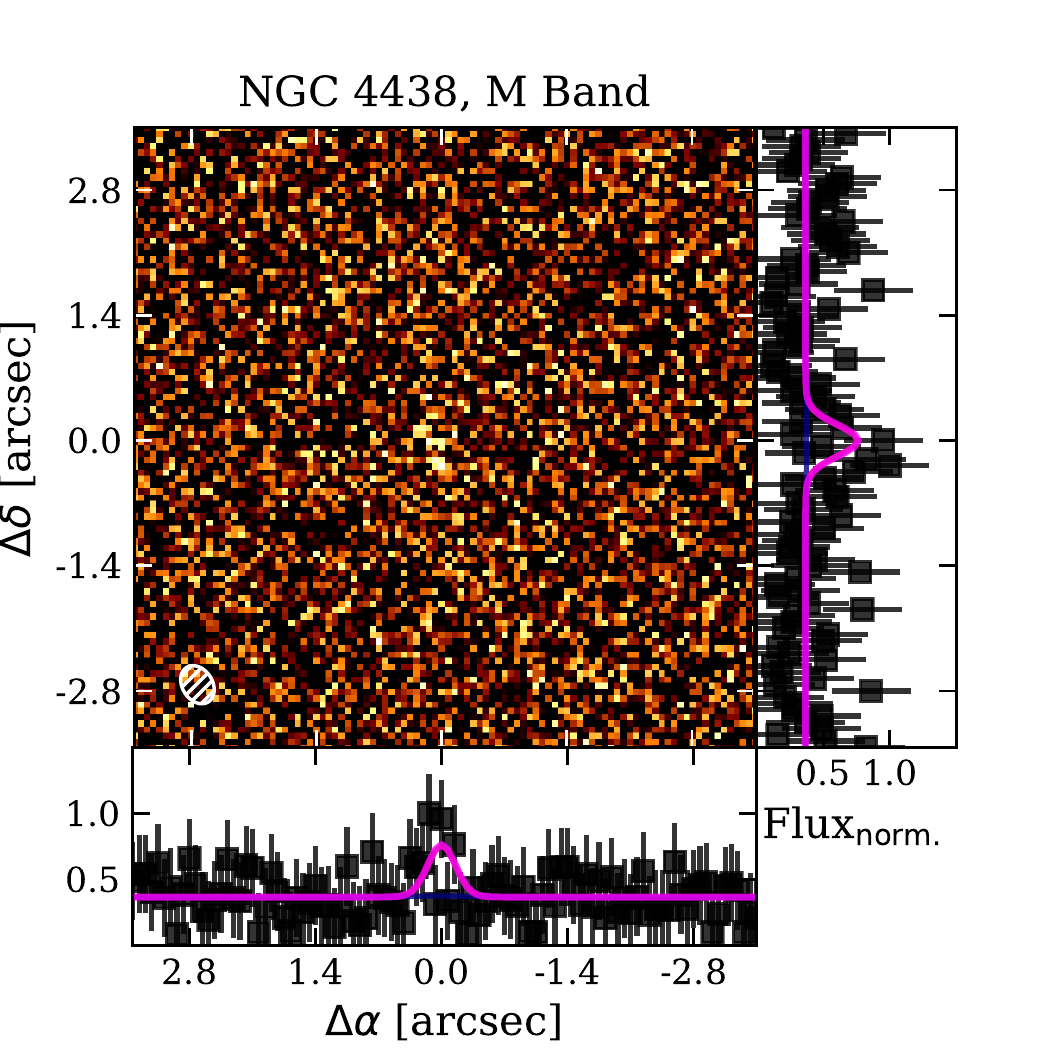}} \\
\subfloat{\includegraphics[width=0.25\hsize]{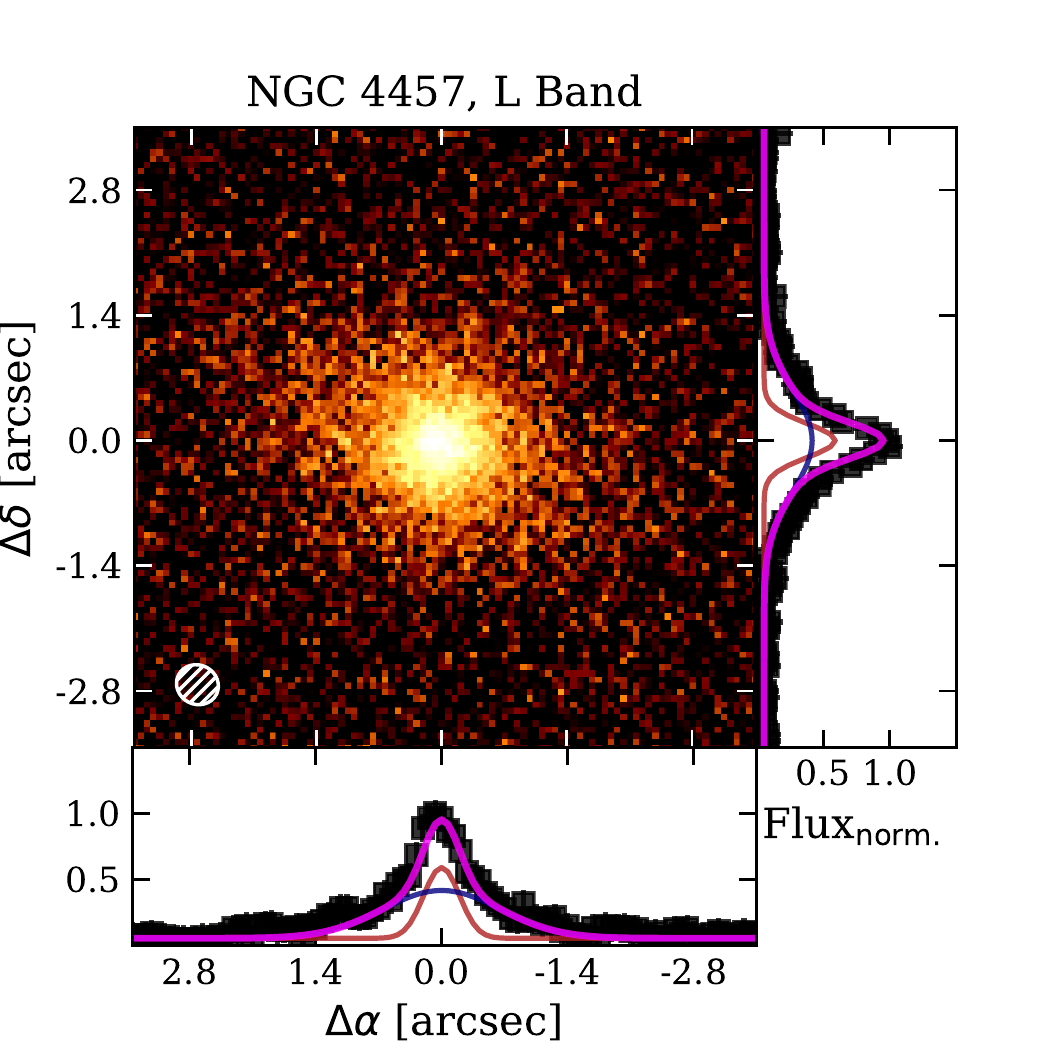}}
\subfloat{\includegraphics[width=0.25\hsize]{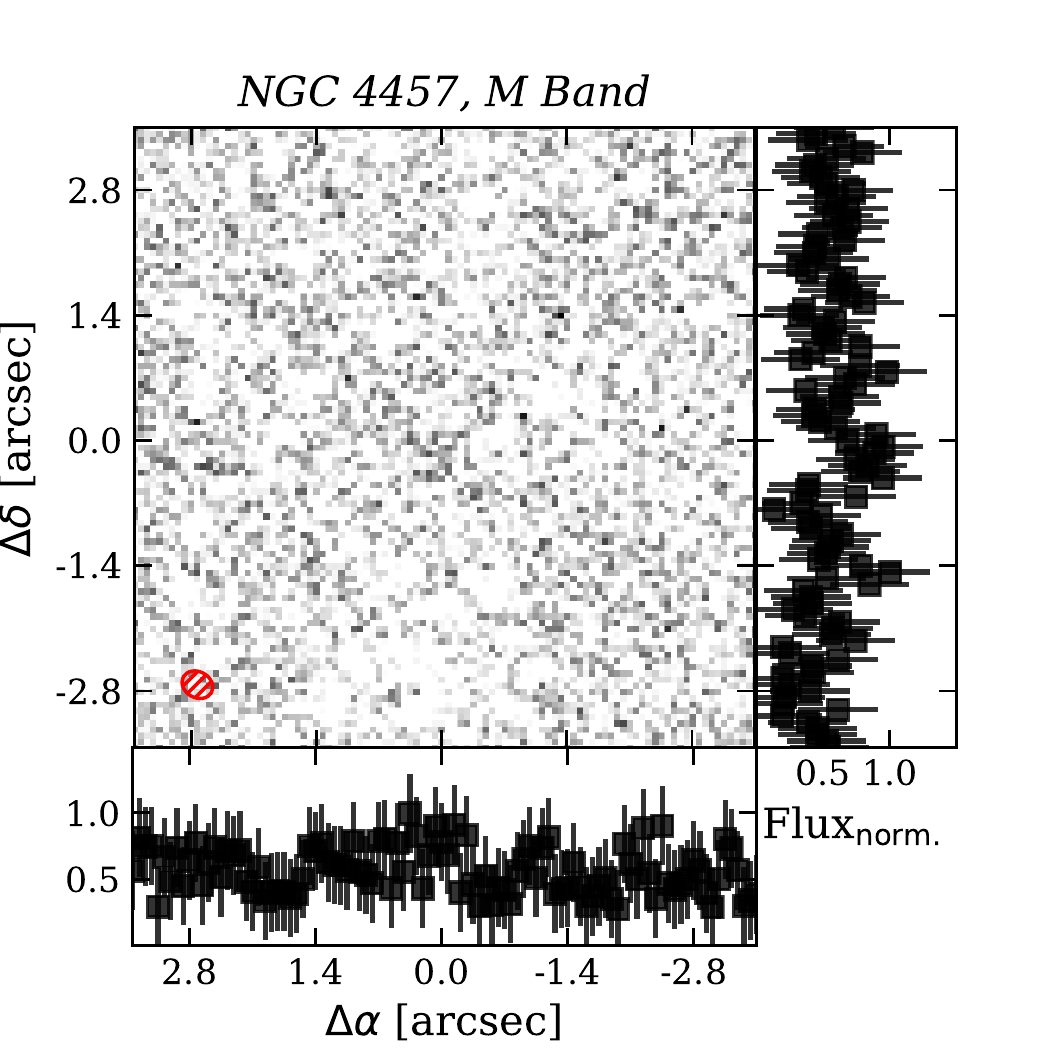}} 
\subfloat{\includegraphics[width=0.25\hsize]{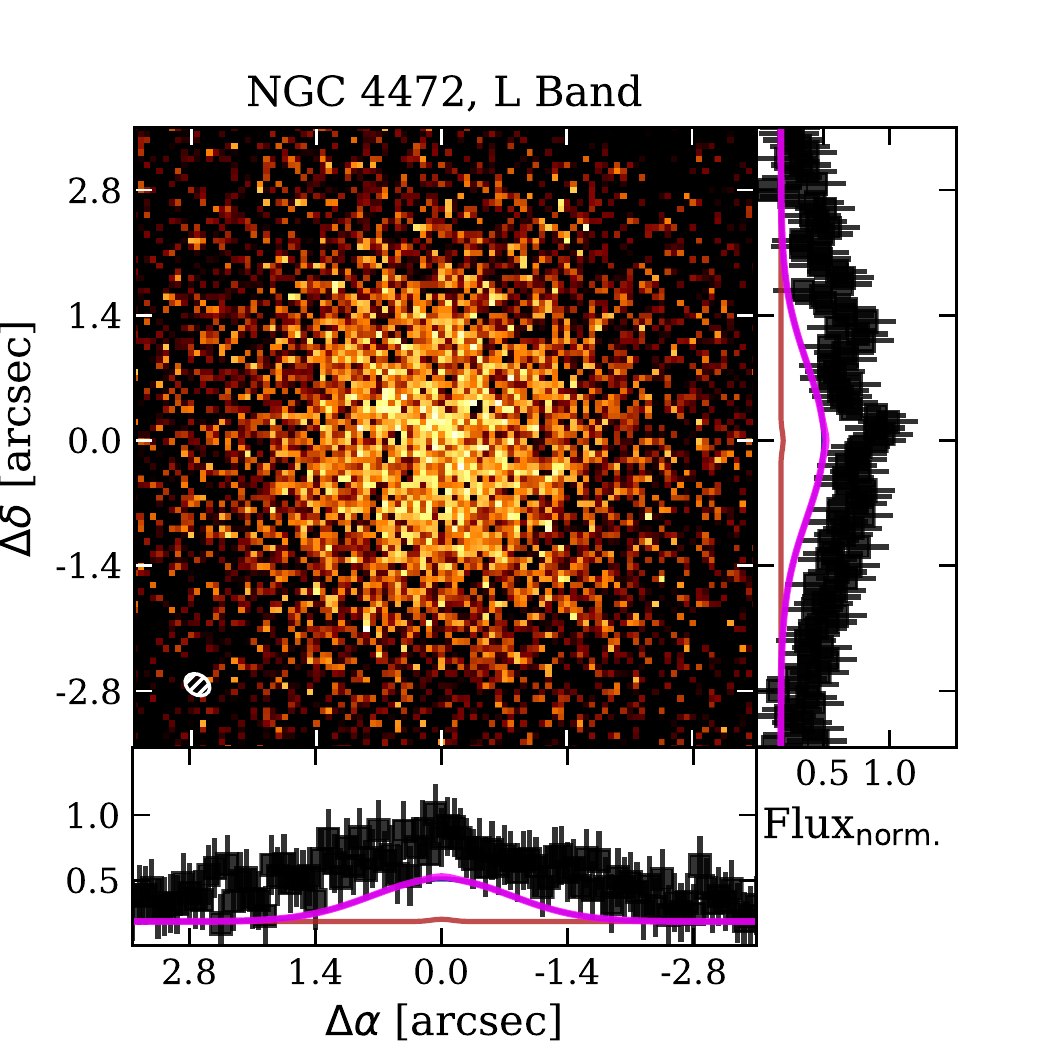}}
\subfloat{\includegraphics[width=0.25\hsize]{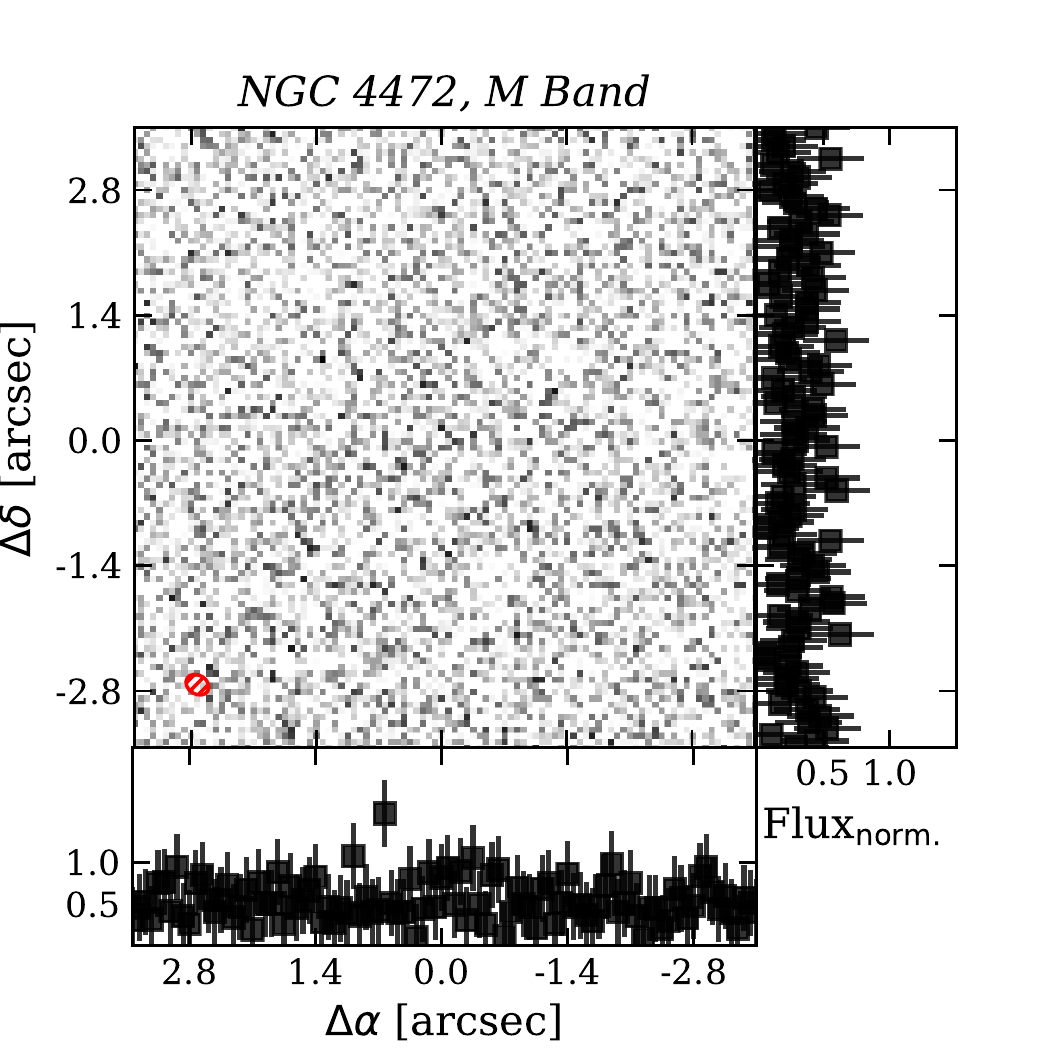}} \\
\subfloat{\includegraphics[width=0.25\hsize]{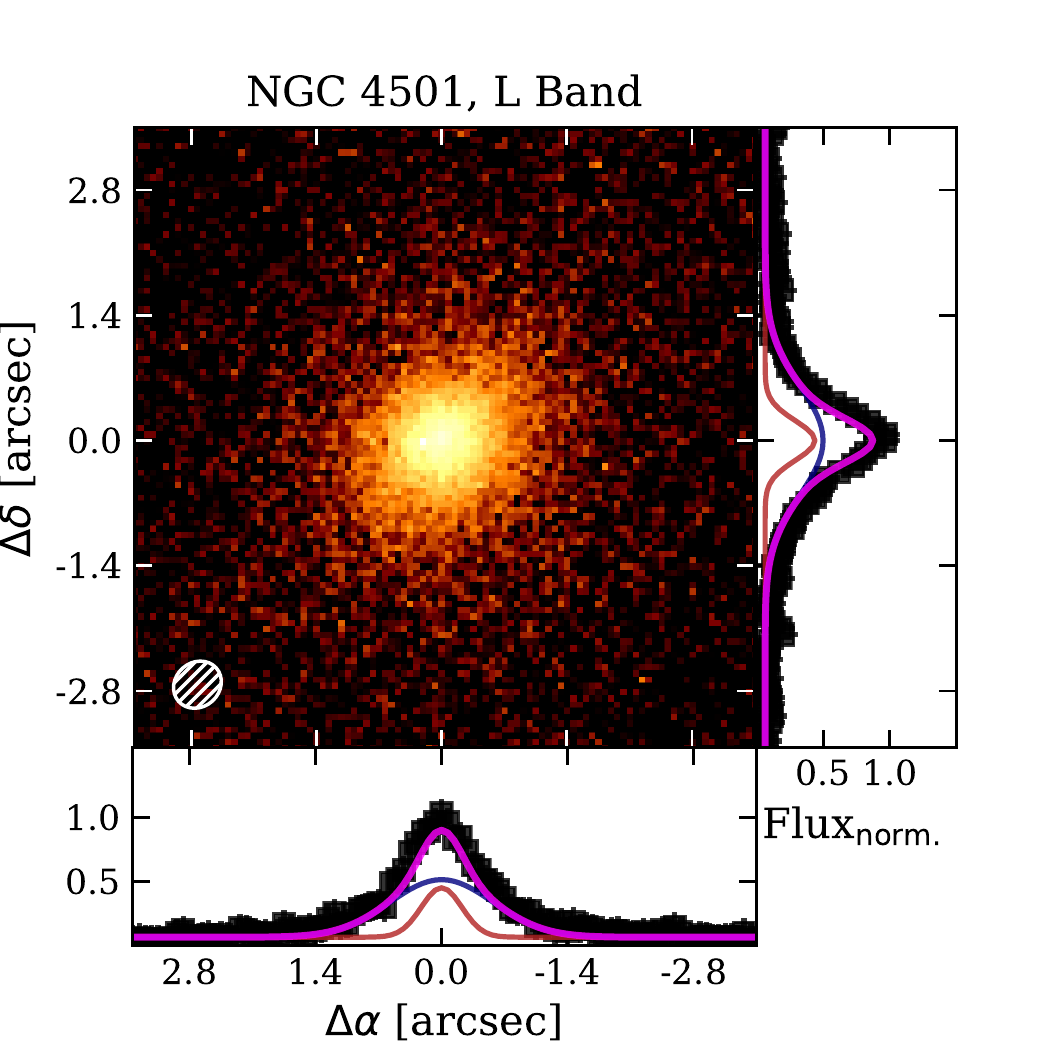}}
\subfloat{\includegraphics[width=0.25\hsize]{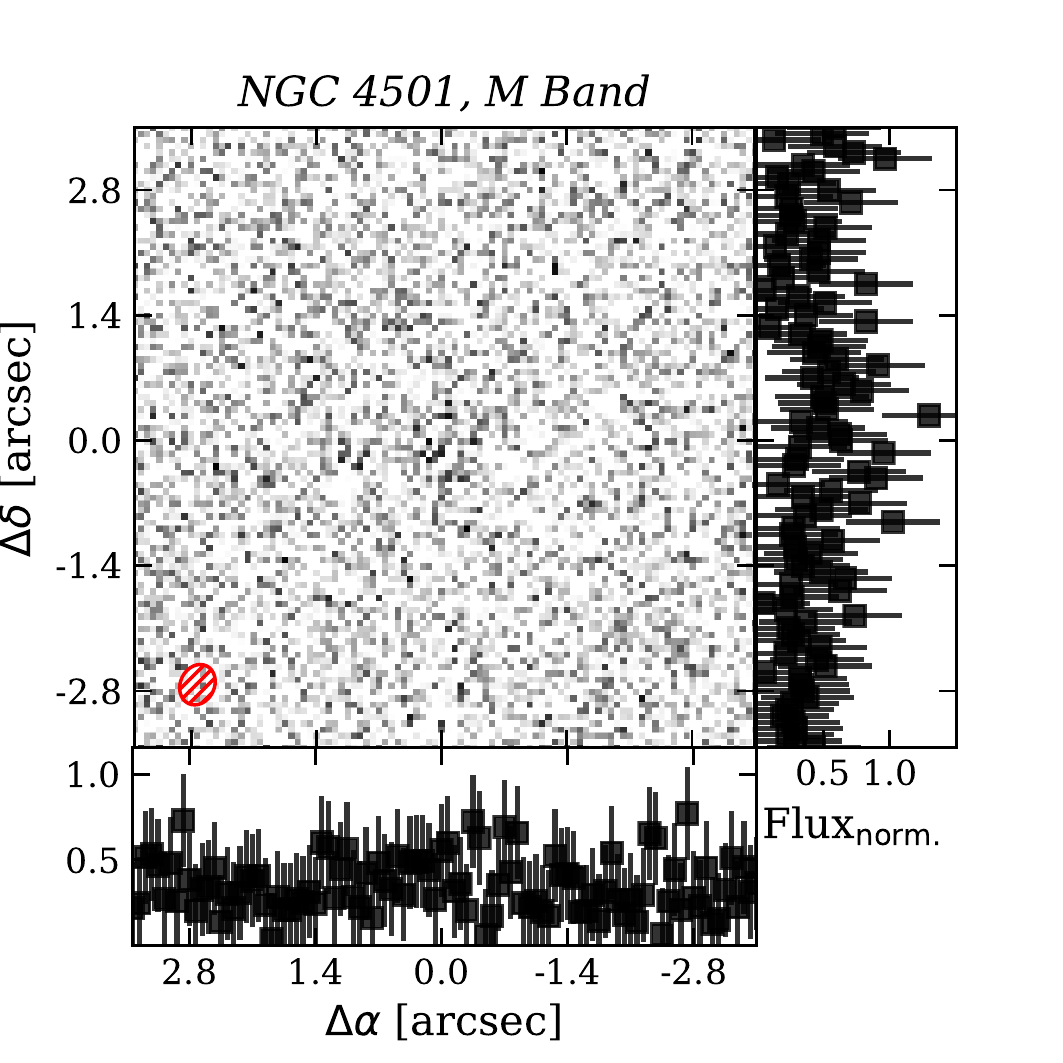}} 
\subfloat{\includegraphics[width=0.25\hsize]{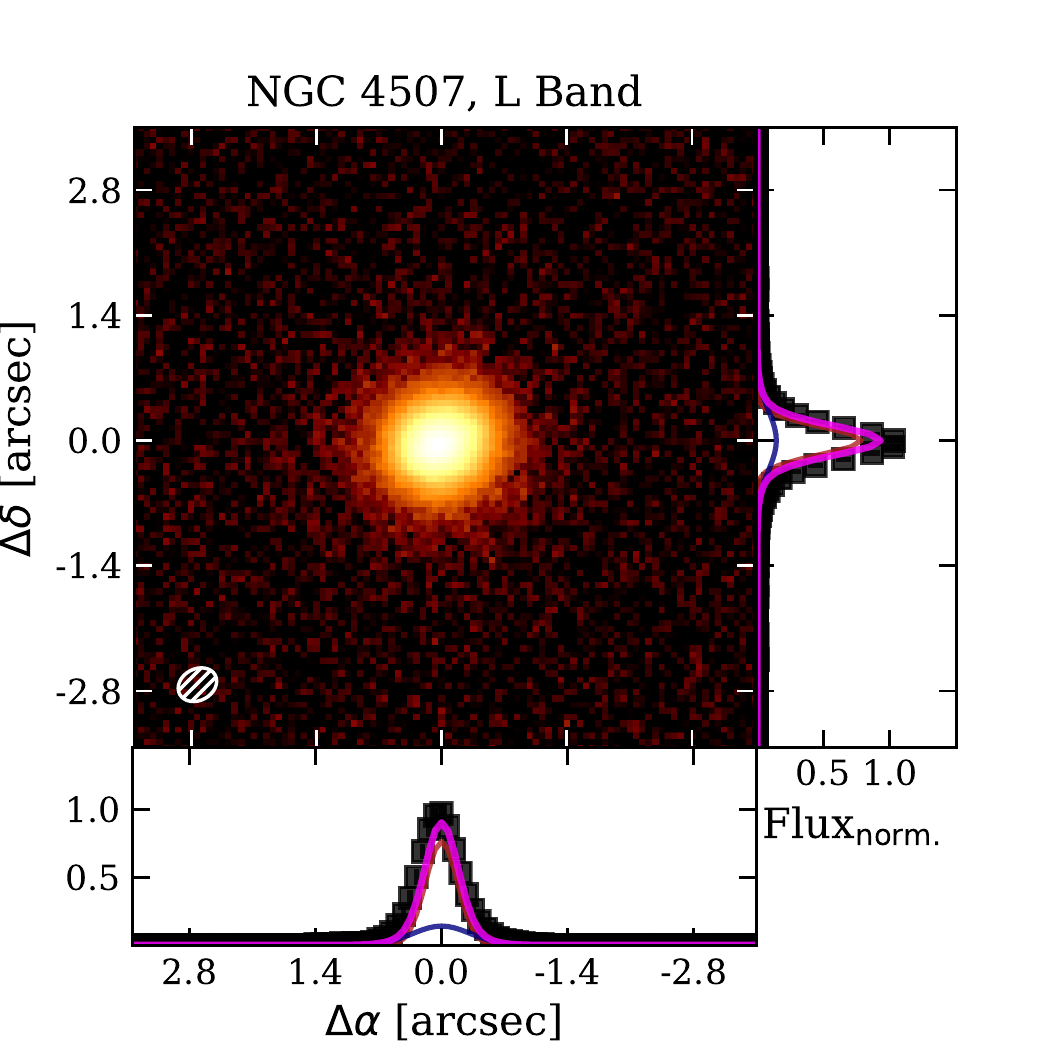}}
\subfloat{\includegraphics[width=0.25\hsize]{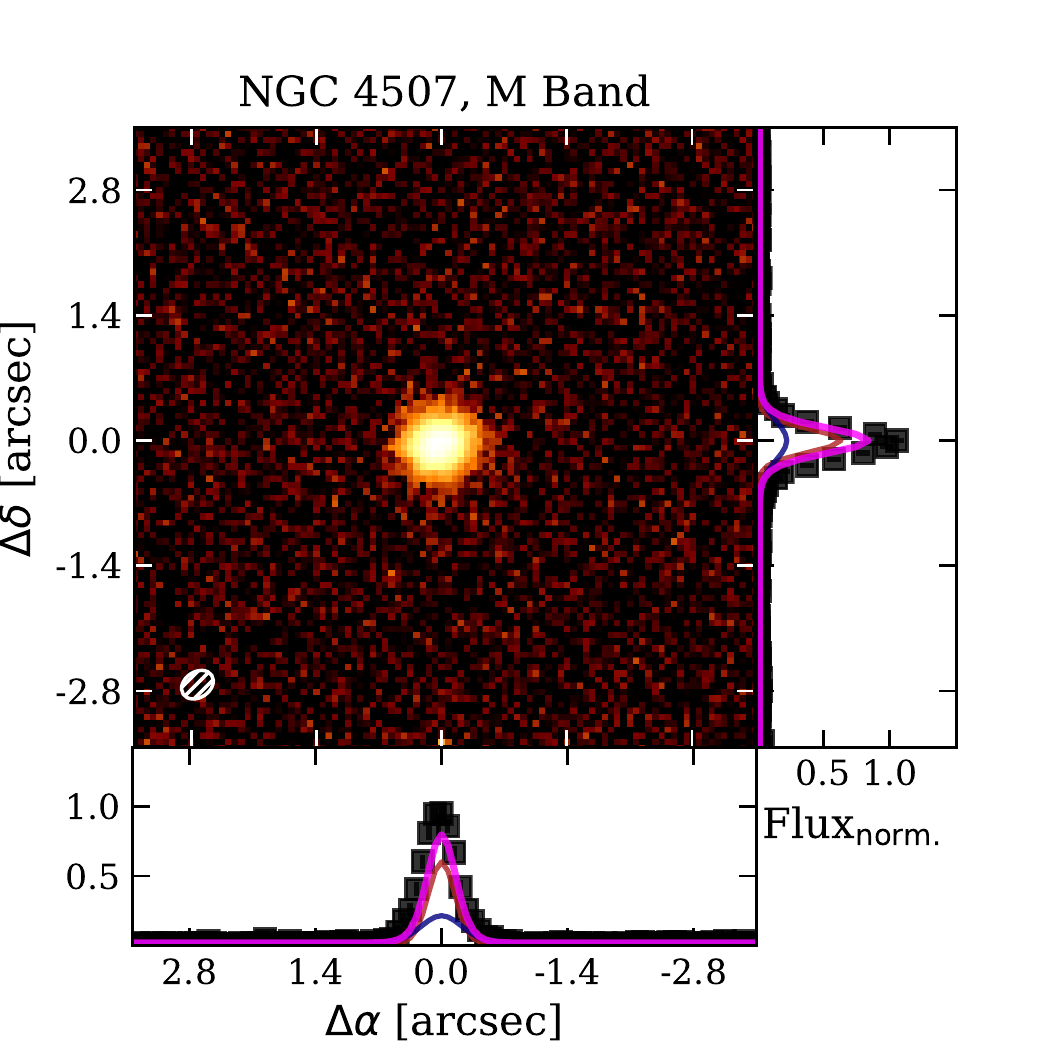}}\\
\subfloat{\includegraphics[width=0.25\hsize]{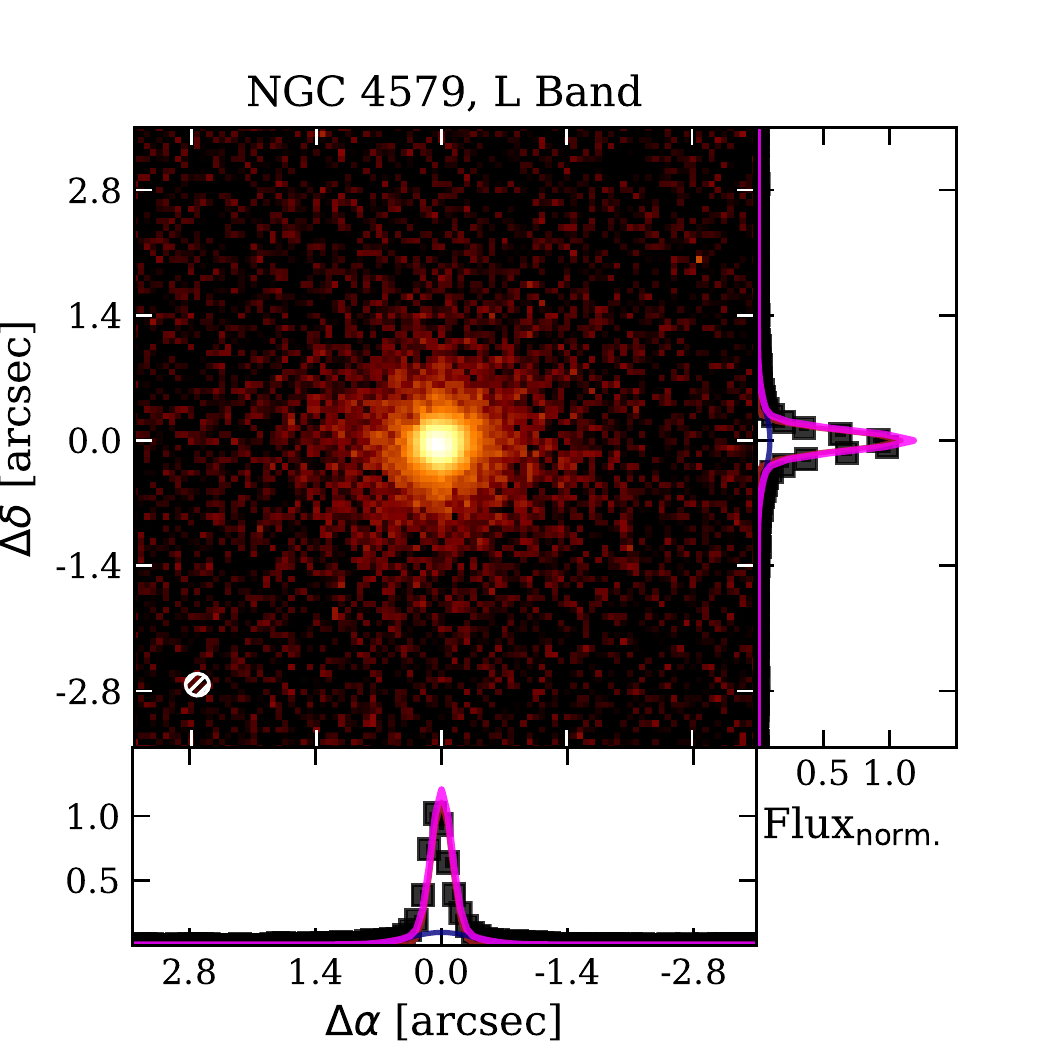}}
\subfloat{\includegraphics[width=0.25\hsize]{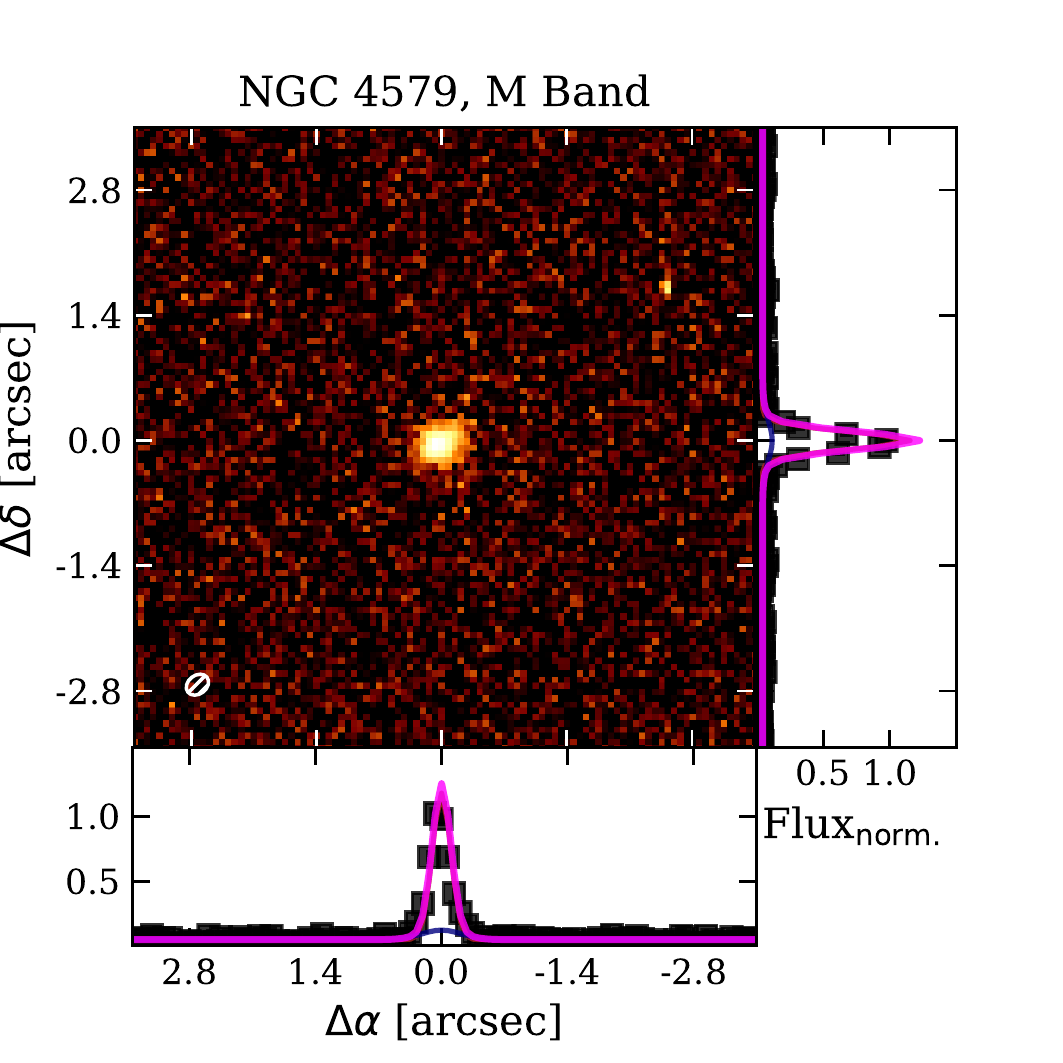}} 
\subfloat{\includegraphics[width=0.25\hsize]{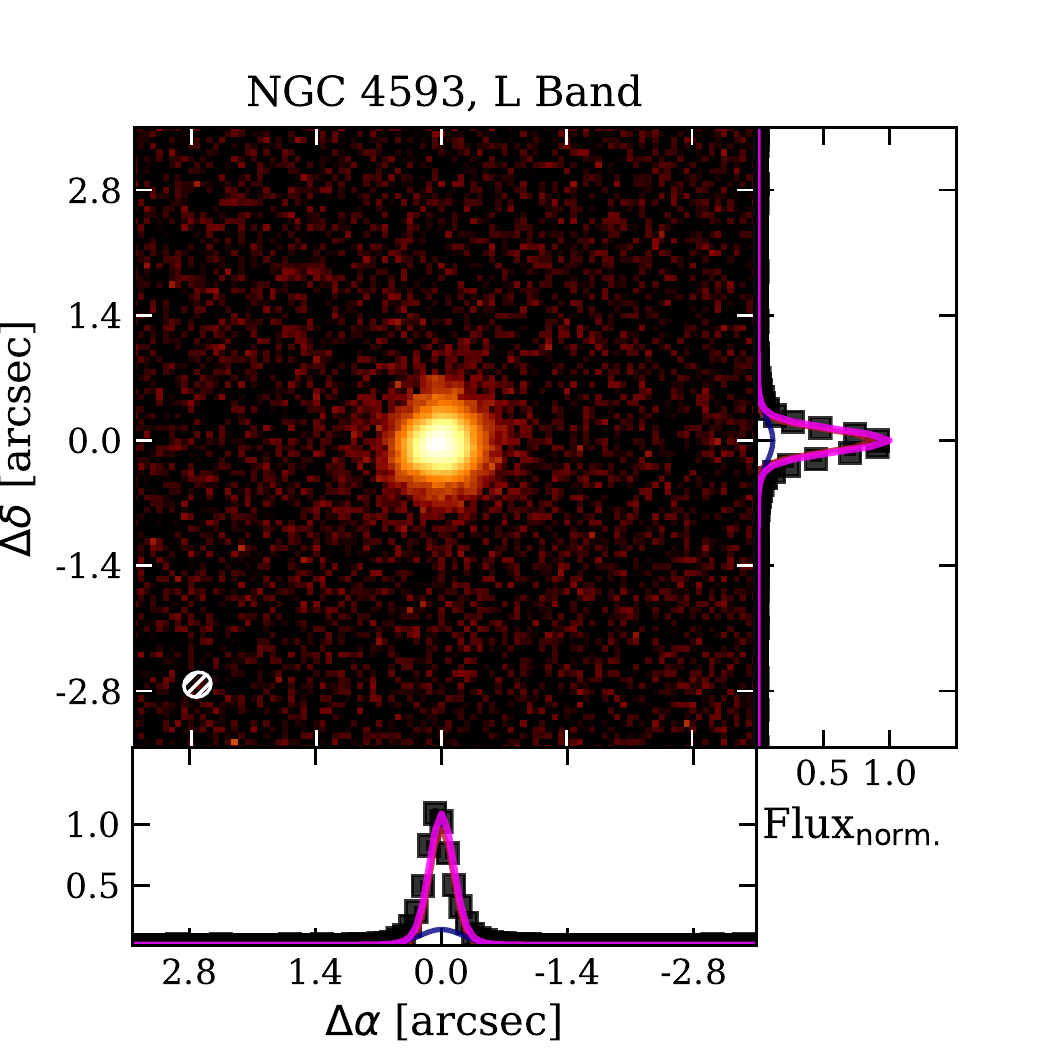}}
\subfloat{\includegraphics[width=0.25\hsize]{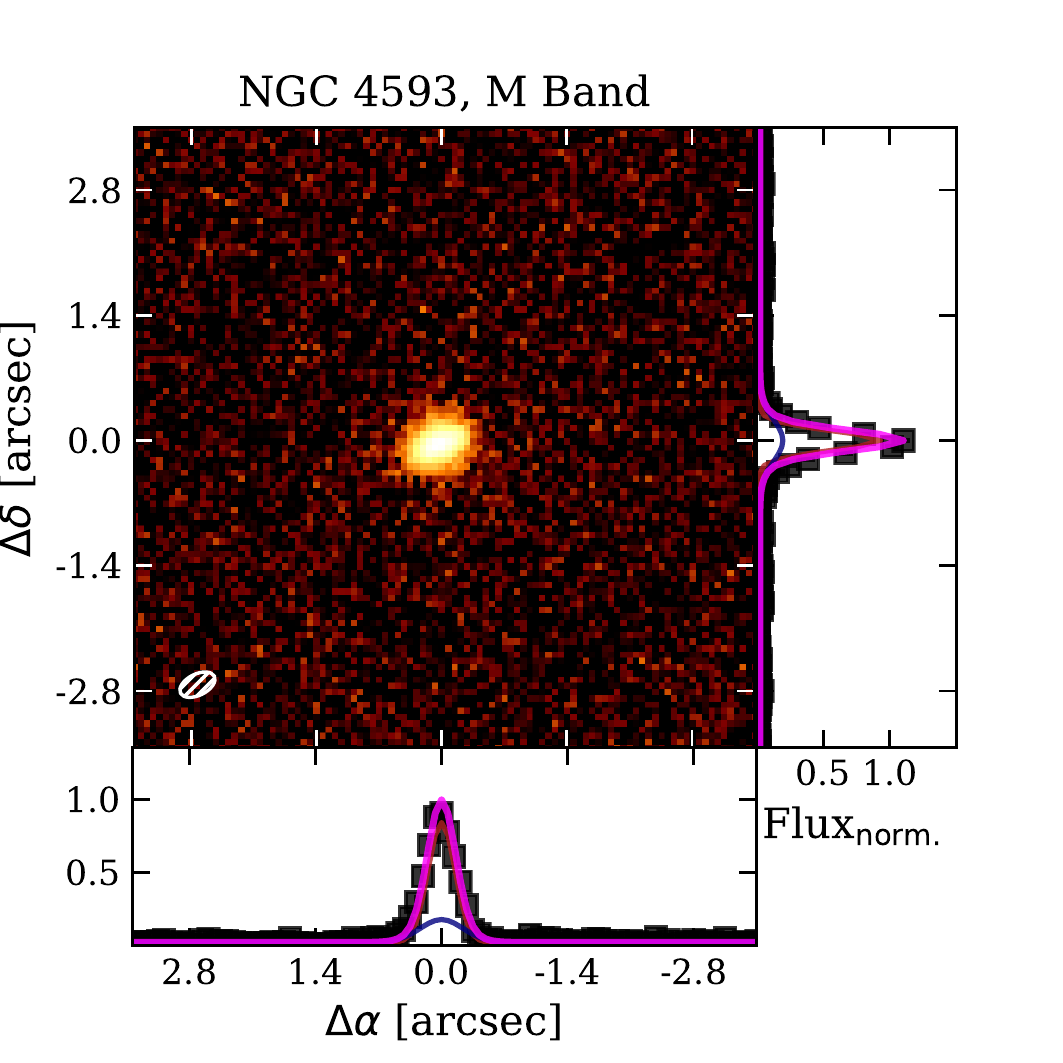}}\\
\caption{ As Fig \ref{fig:cutouts_one} but for all sources.}
\end{figure*}
\begin{figure*}
\subfloat{\includegraphics[width=0.25\hsize]{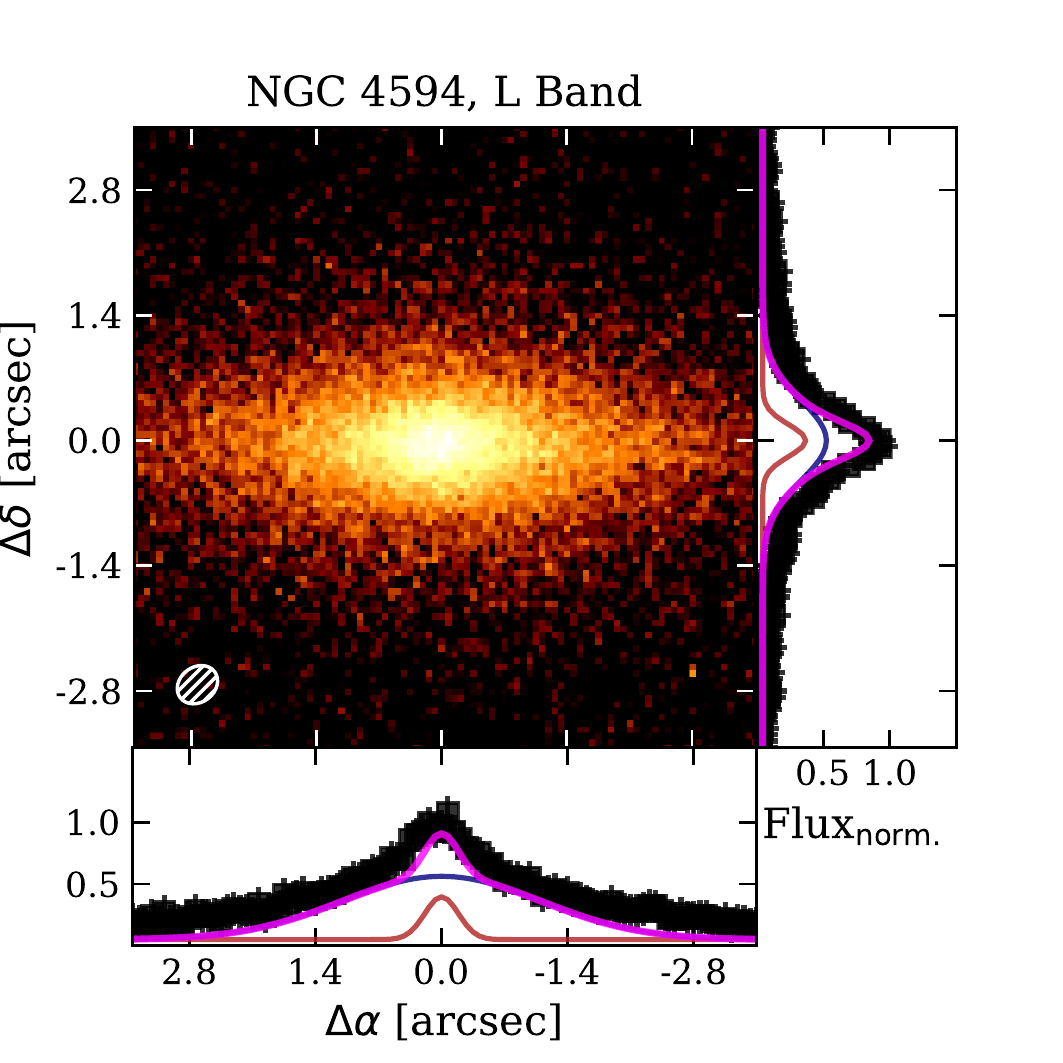}}
\subfloat{\includegraphics[width=0.25\hsize]{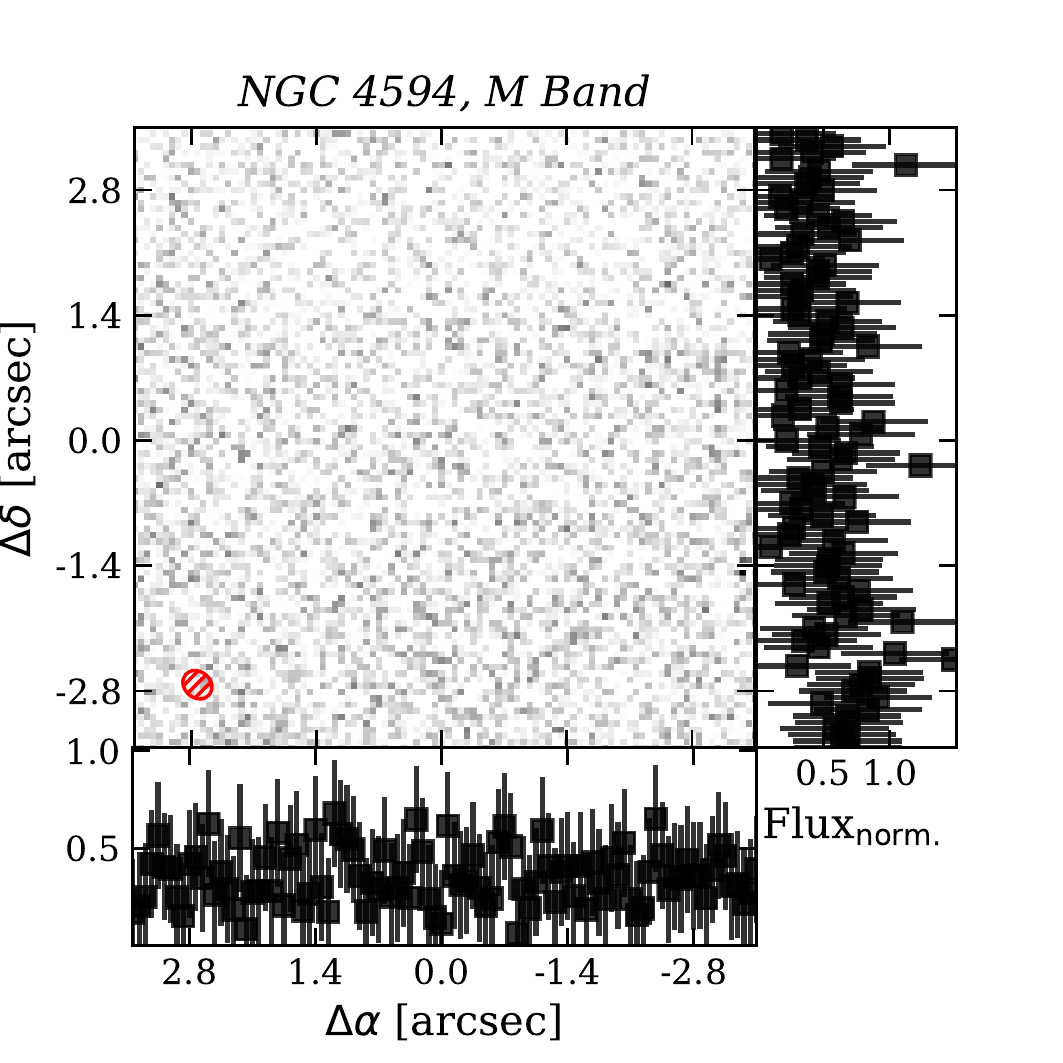}} 
\subfloat{\includegraphics[width=0.25\hsize]{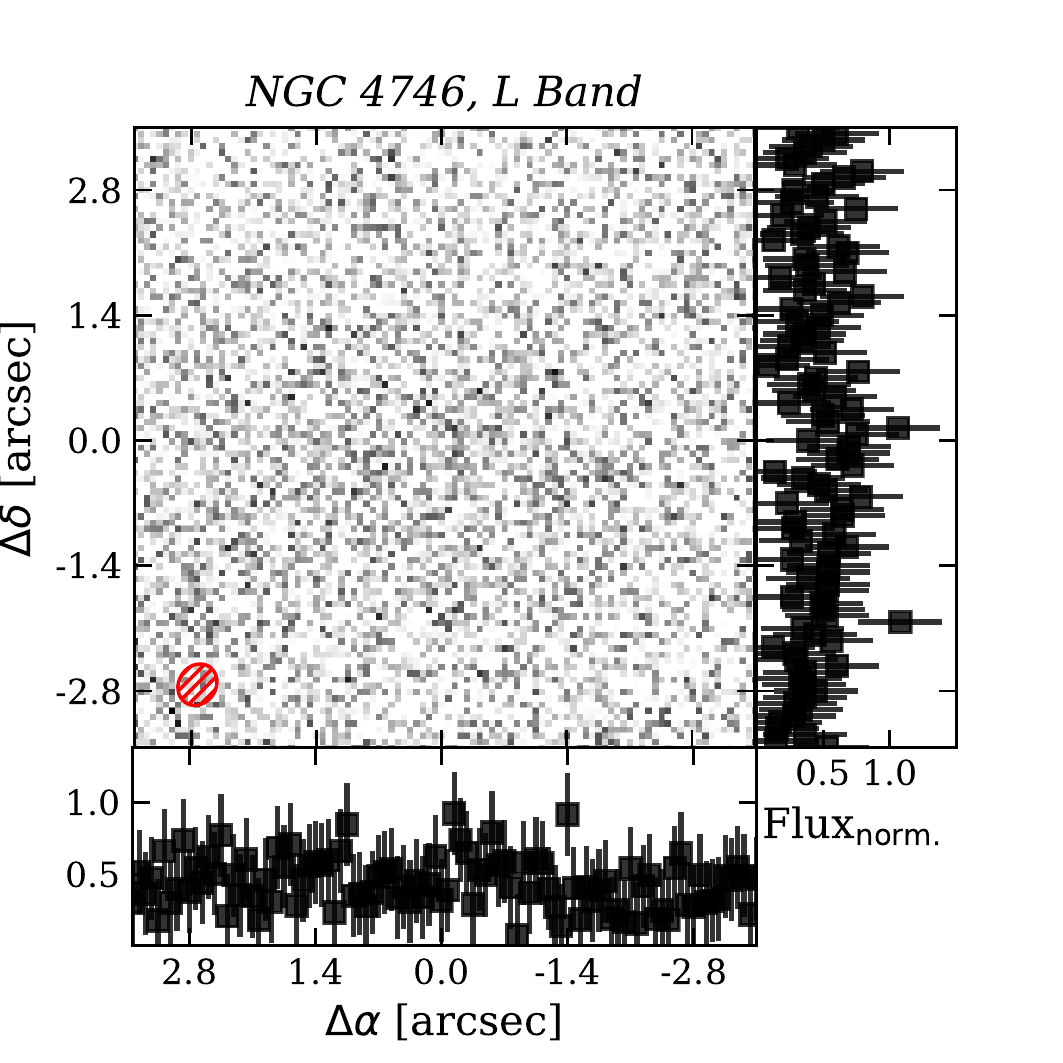}}
\subfloat{\includegraphics[width=0.25\hsize]{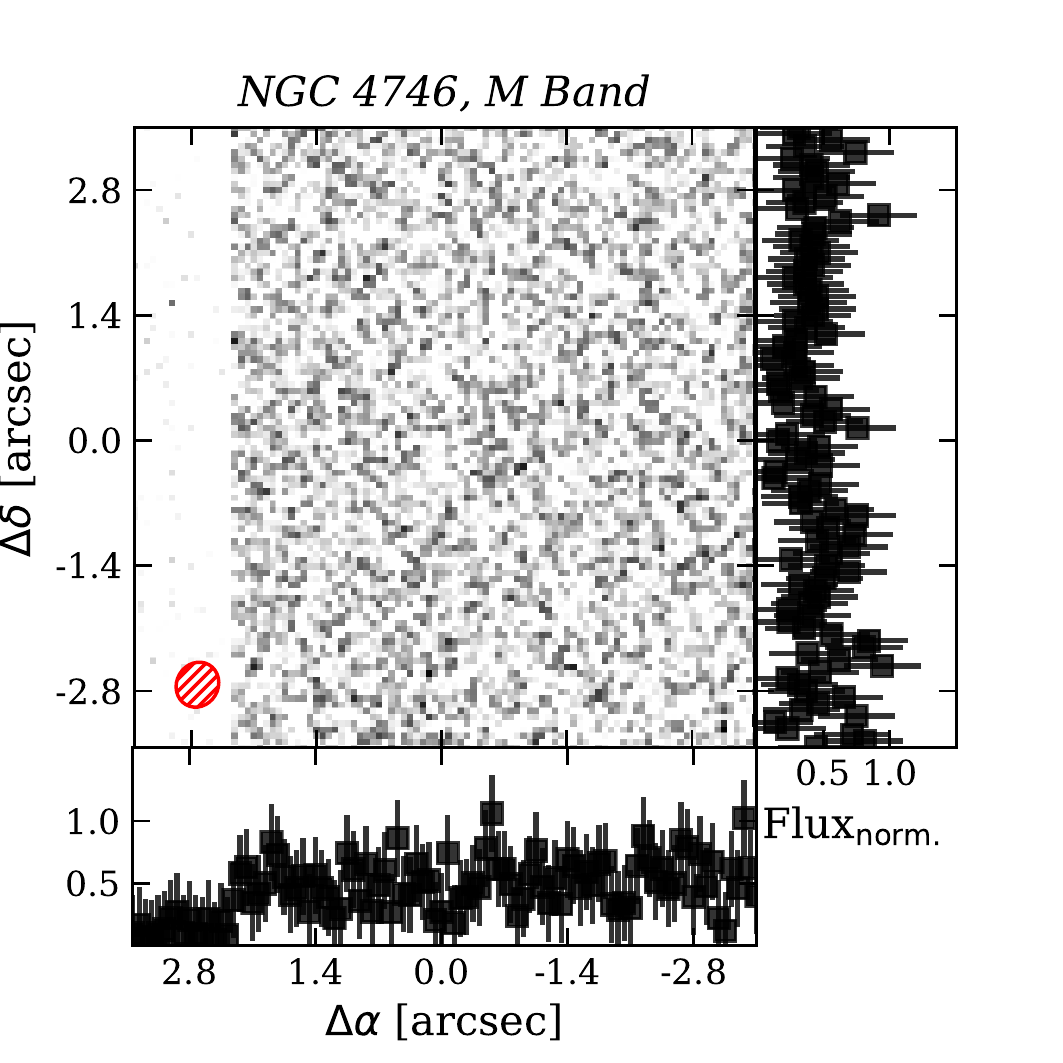}} \\
\subfloat{\includegraphics[width=0.25\hsize]{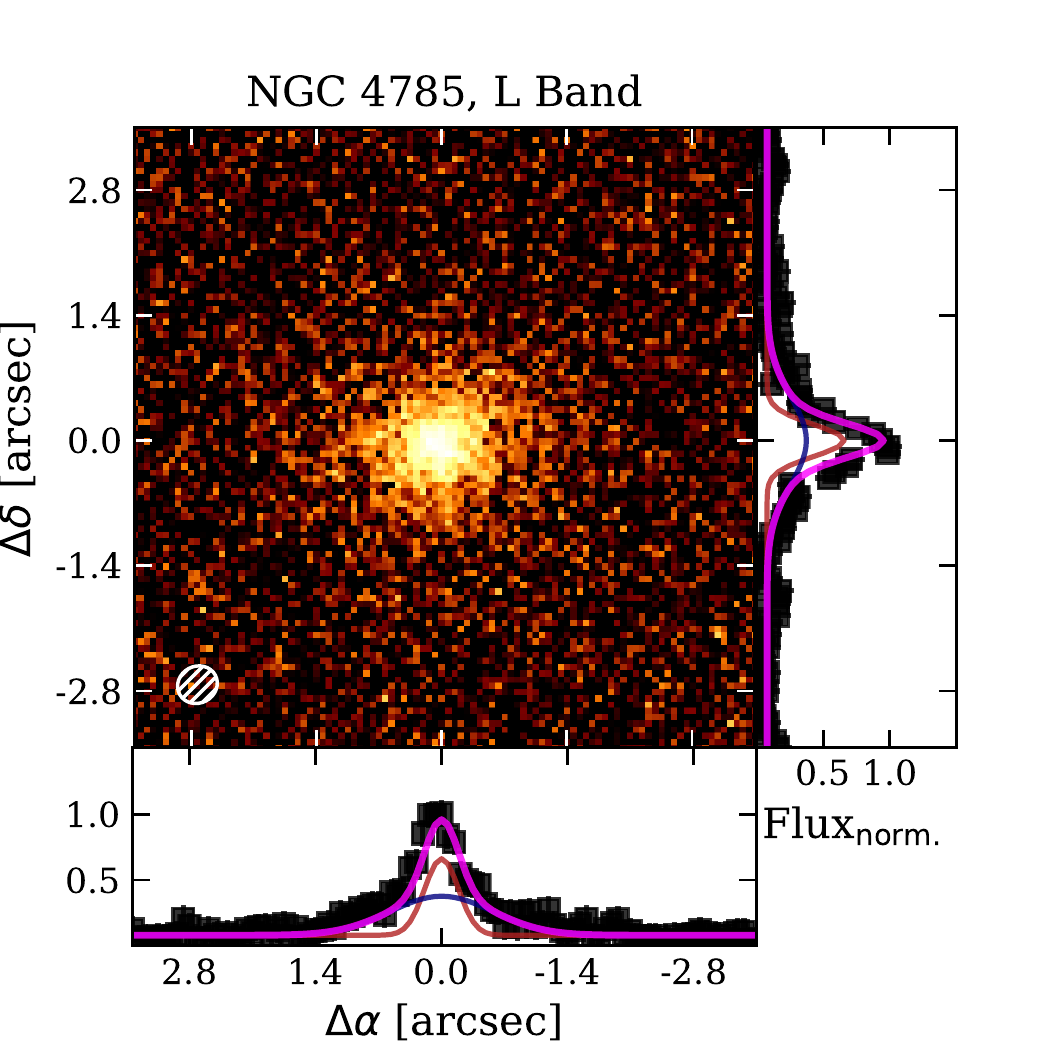}}
\subfloat{\includegraphics[width=0.25\hsize]{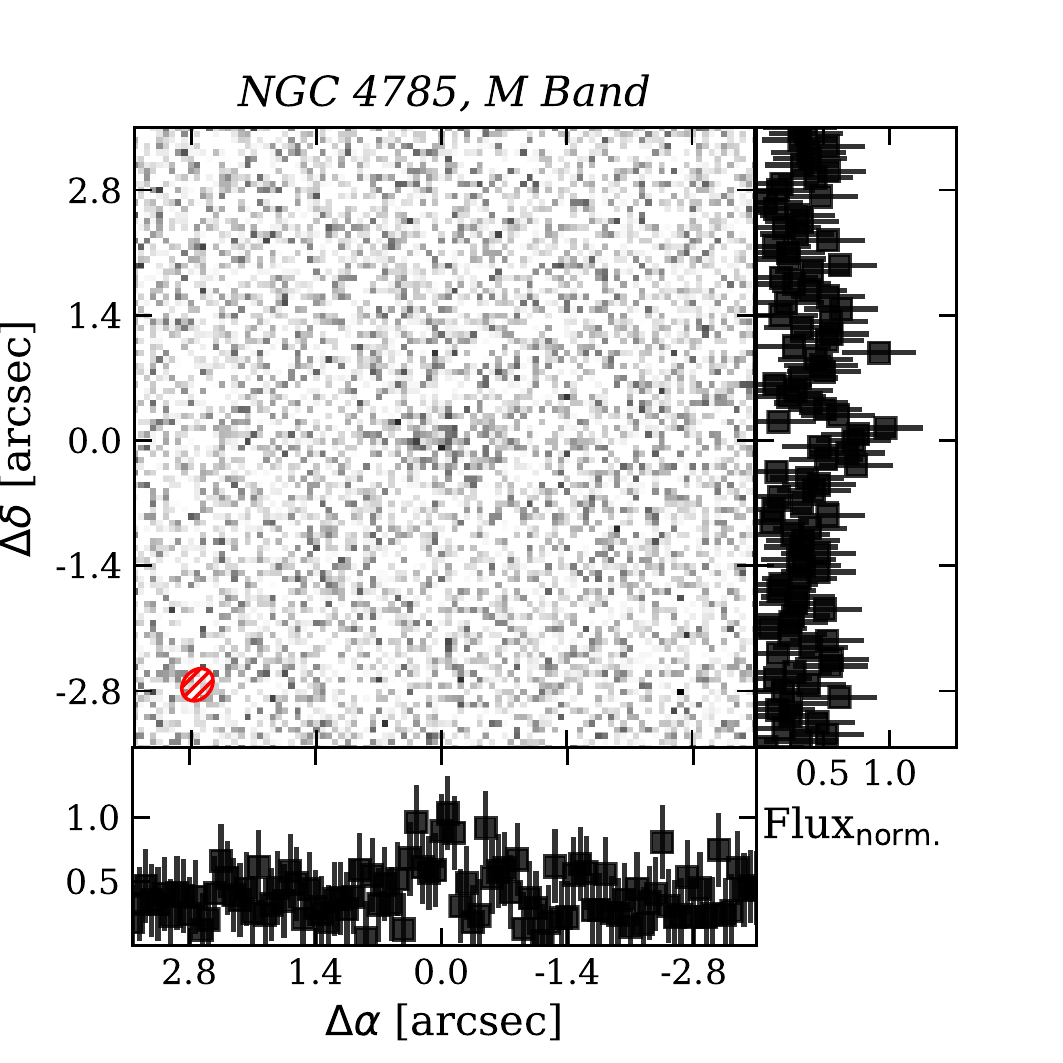}} 
\subfloat{\includegraphics[width=0.25\hsize]{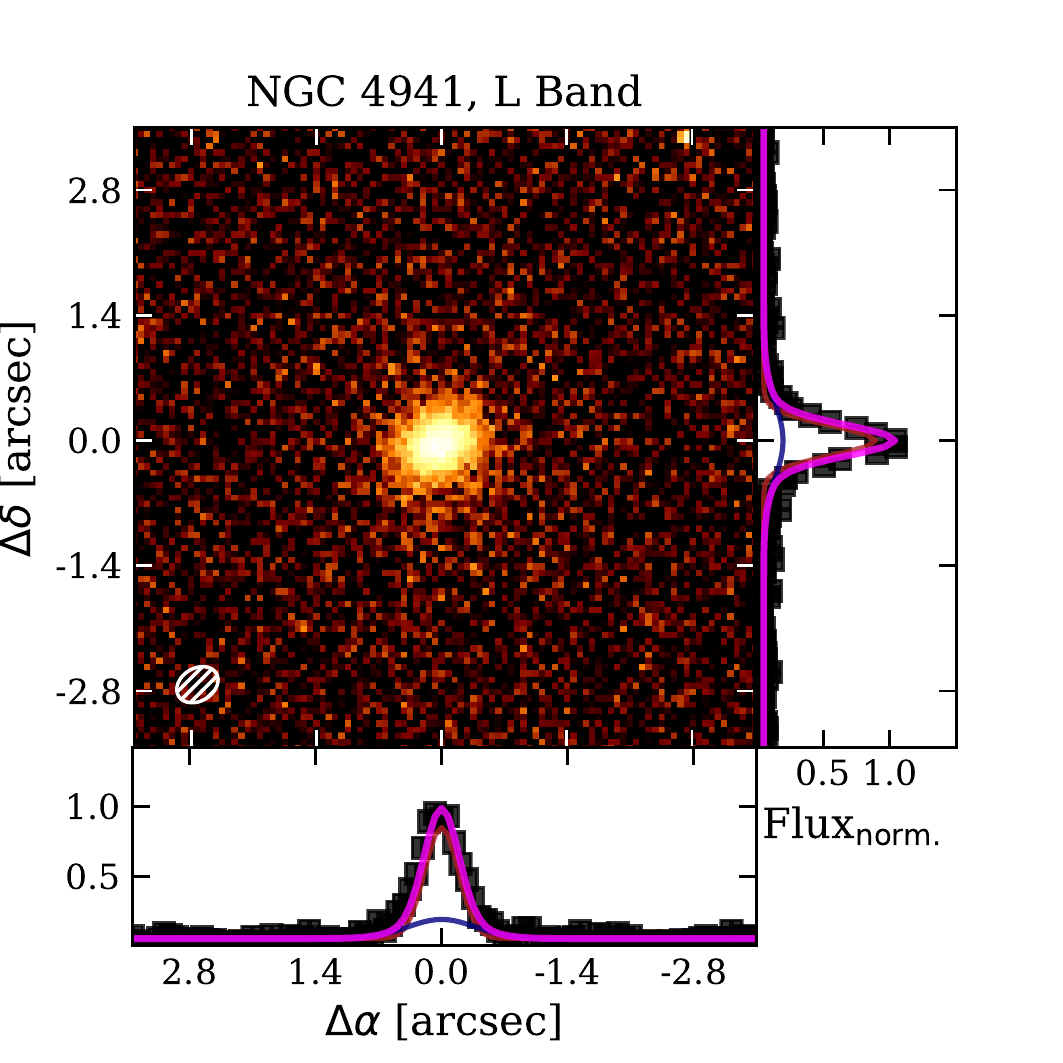}}
\subfloat{\includegraphics[width=0.25\hsize]{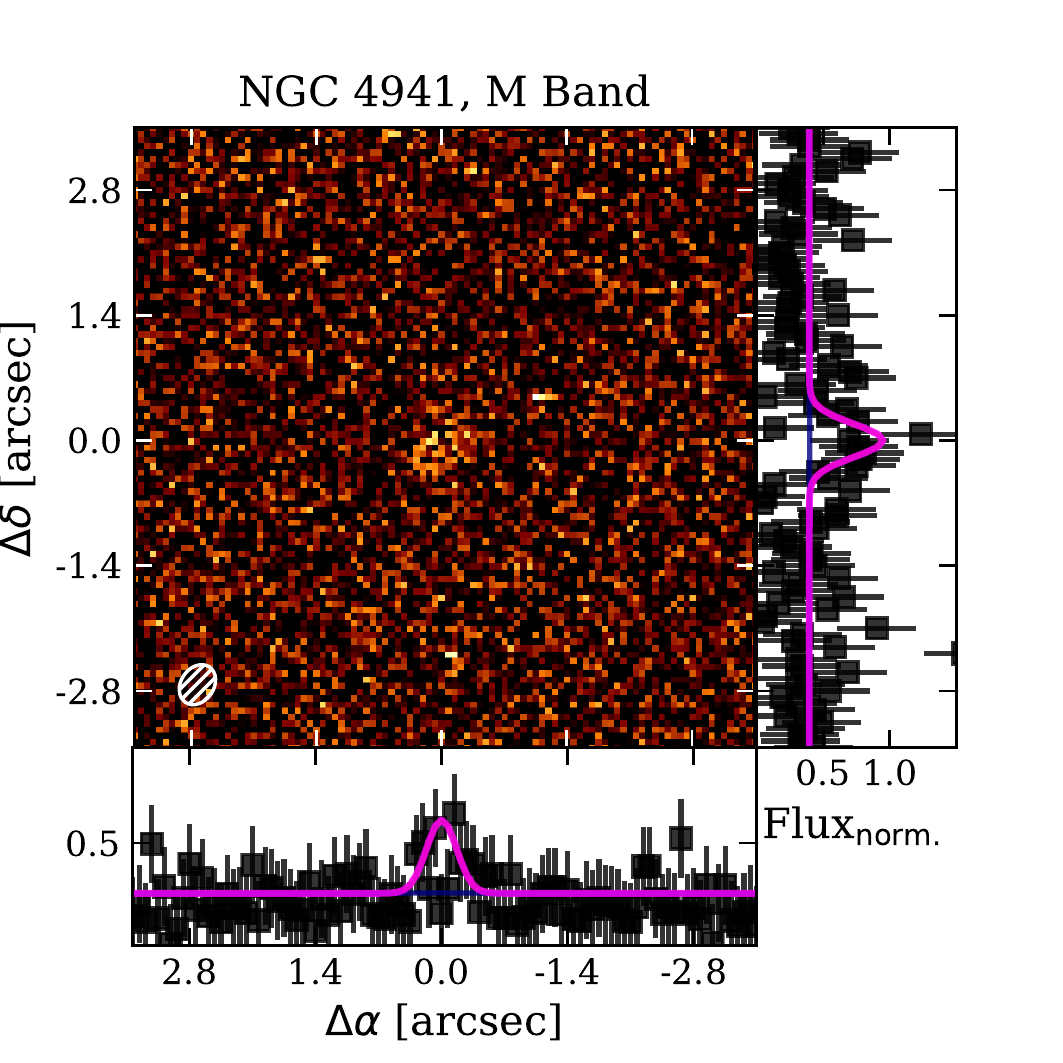}} \\
\subfloat{\includegraphics[width=0.25\hsize]{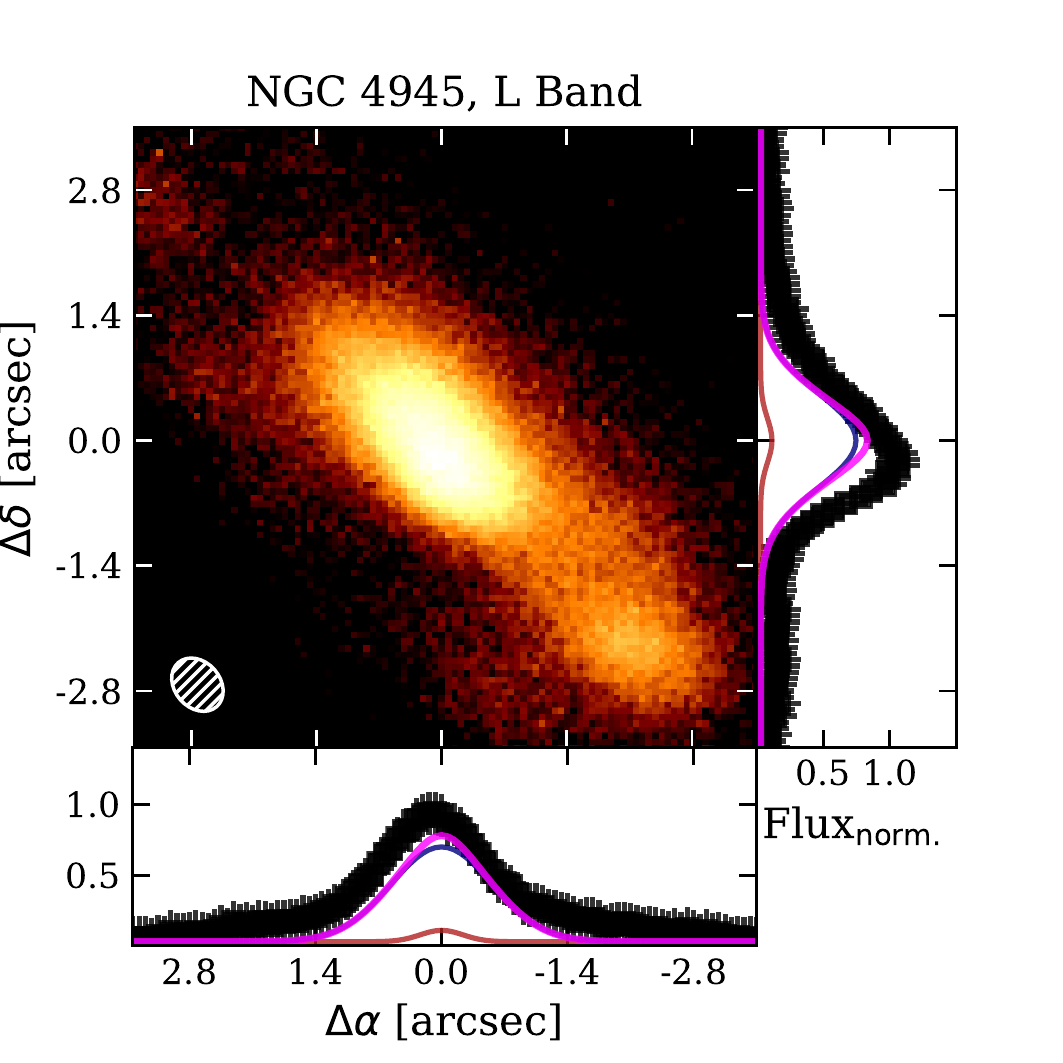}}
\subfloat{\includegraphics[width=0.25\hsize]{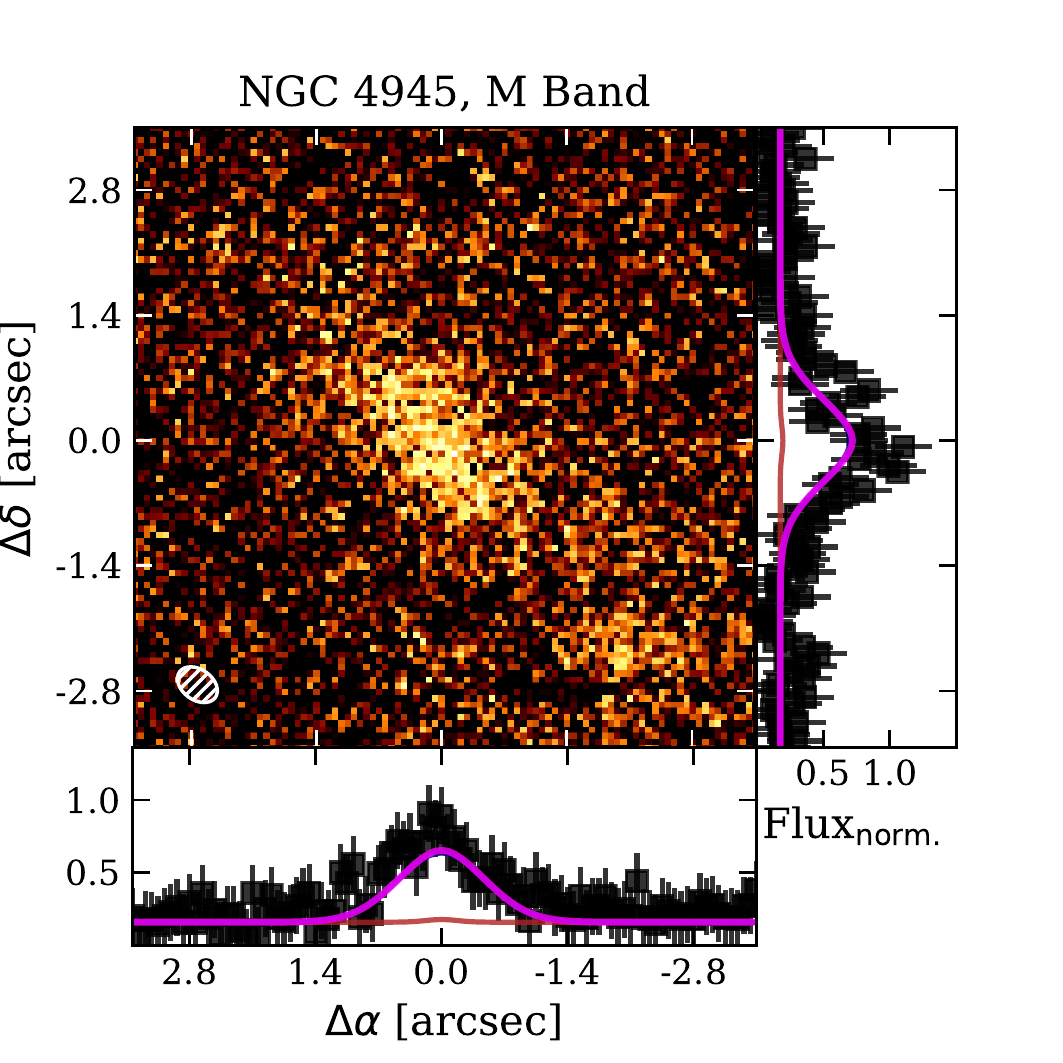}} 
\subfloat{\includegraphics[width=0.25\hsize]{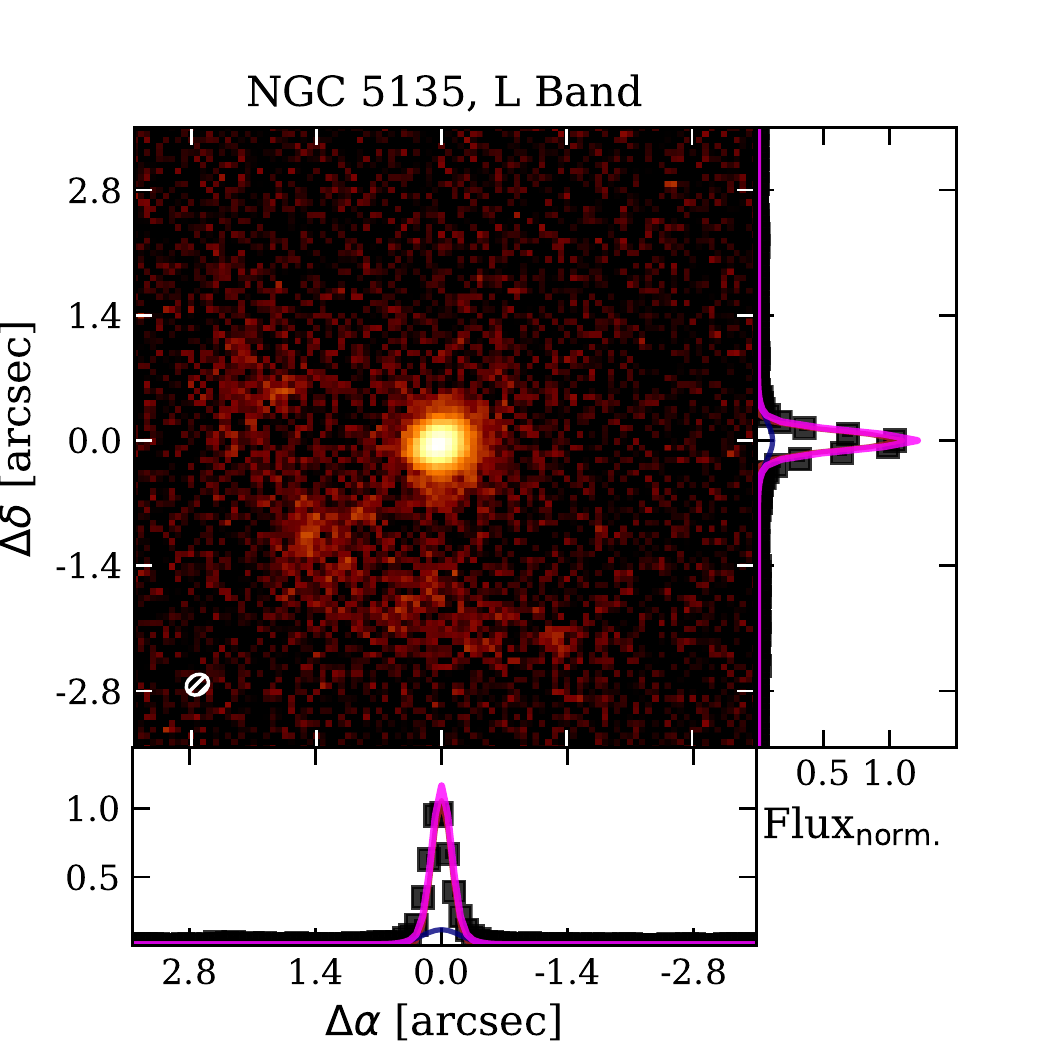}}
\subfloat{\includegraphics[width=0.25\hsize]{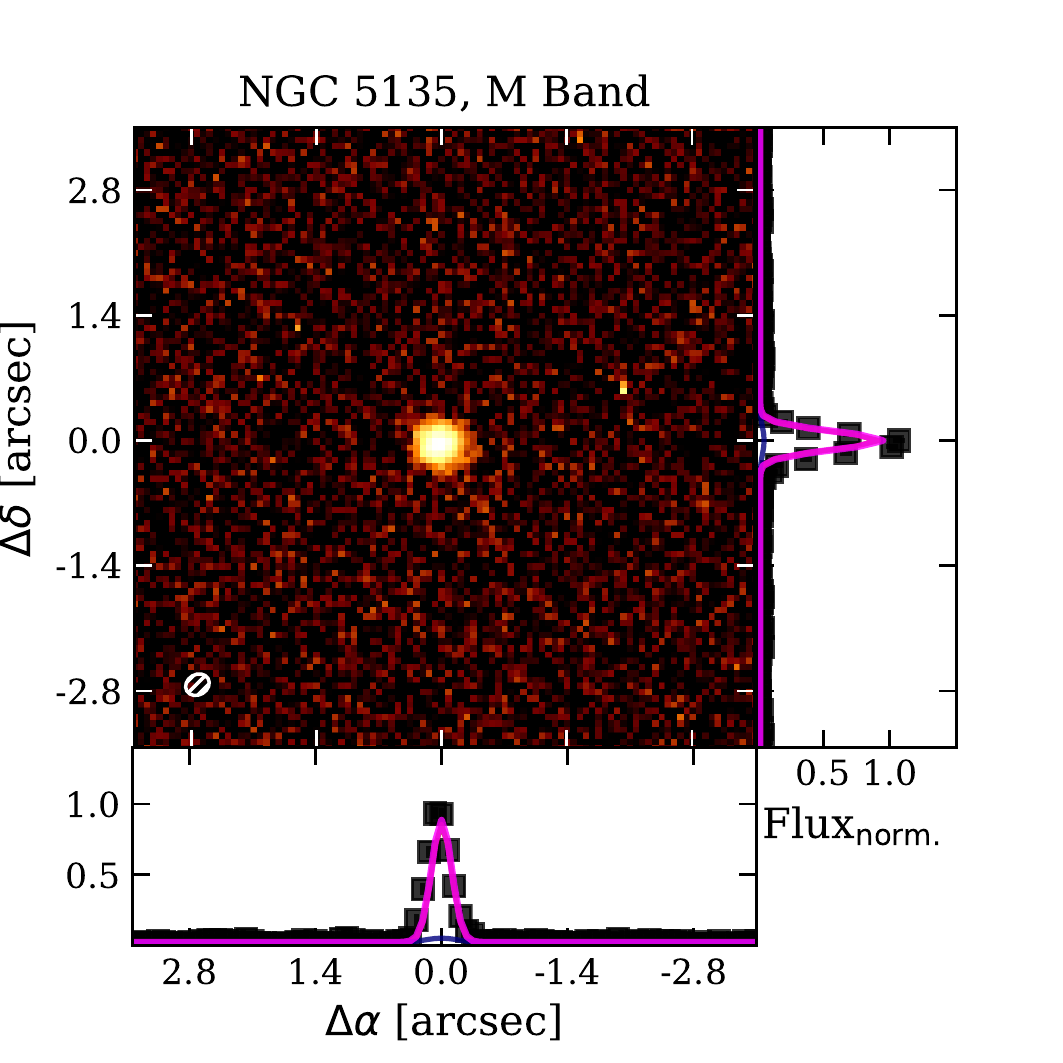}} \\
\subfloat{\includegraphics[width=0.25\hsize]{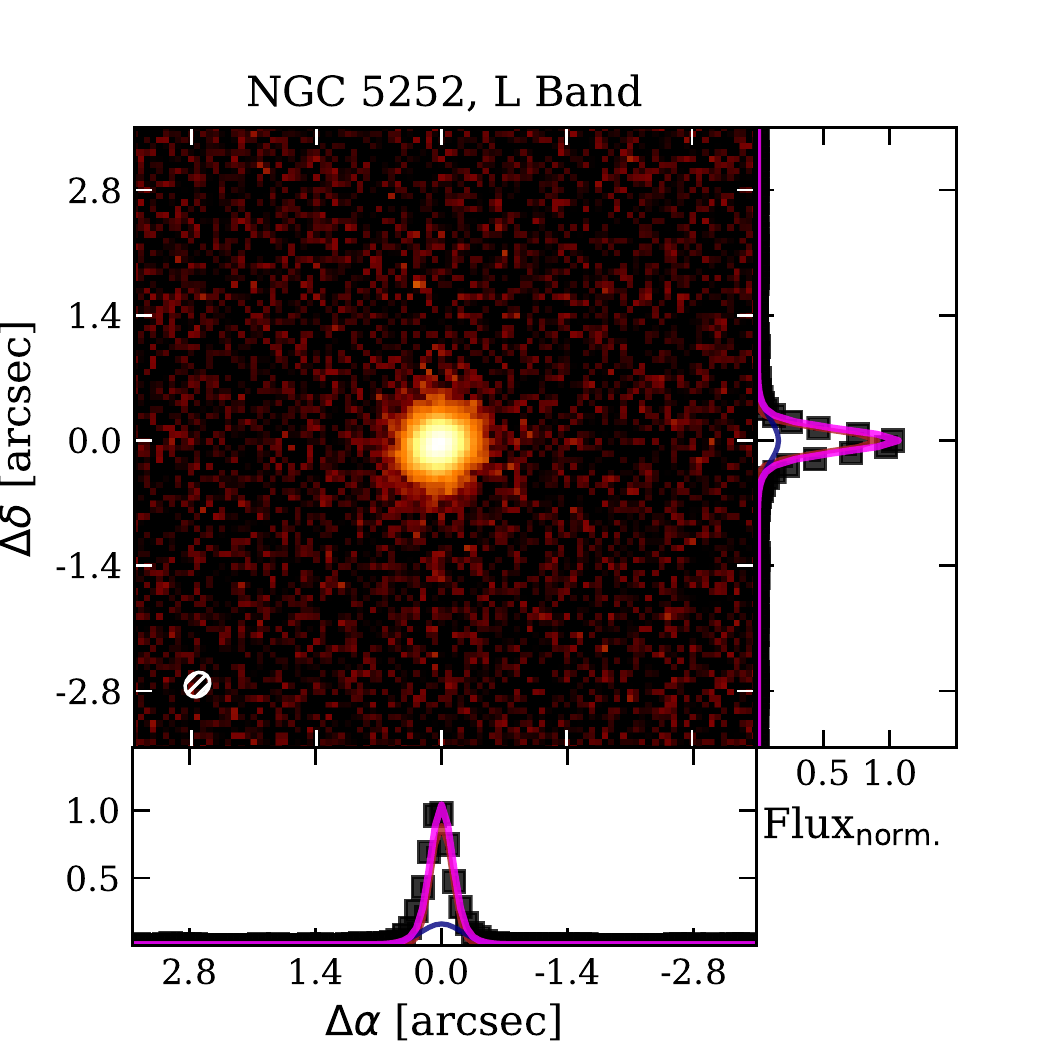}}
\subfloat{\includegraphics[width=0.25\hsize]{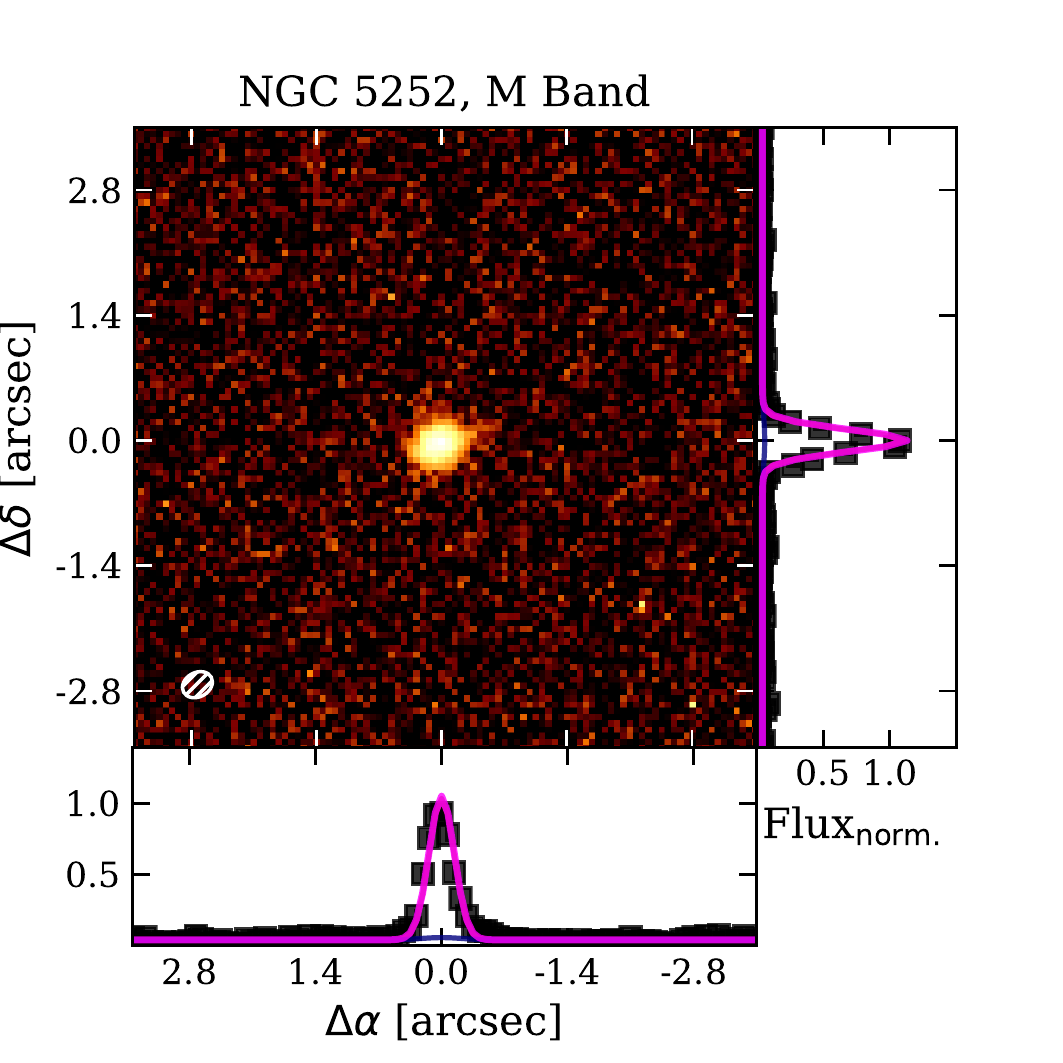}} 
\subfloat{\includegraphics[width=0.25\hsize]{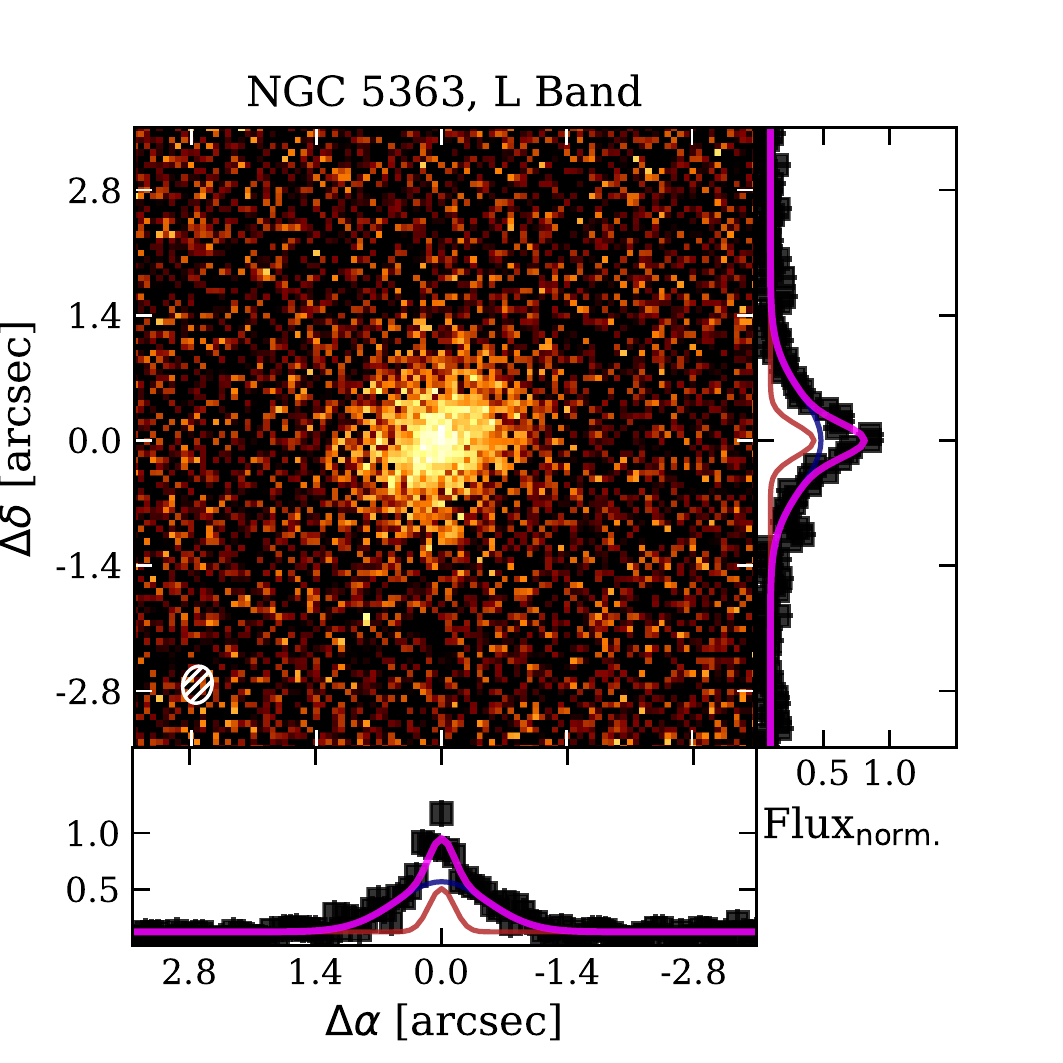}}
\subfloat{\includegraphics[width=0.25\hsize]{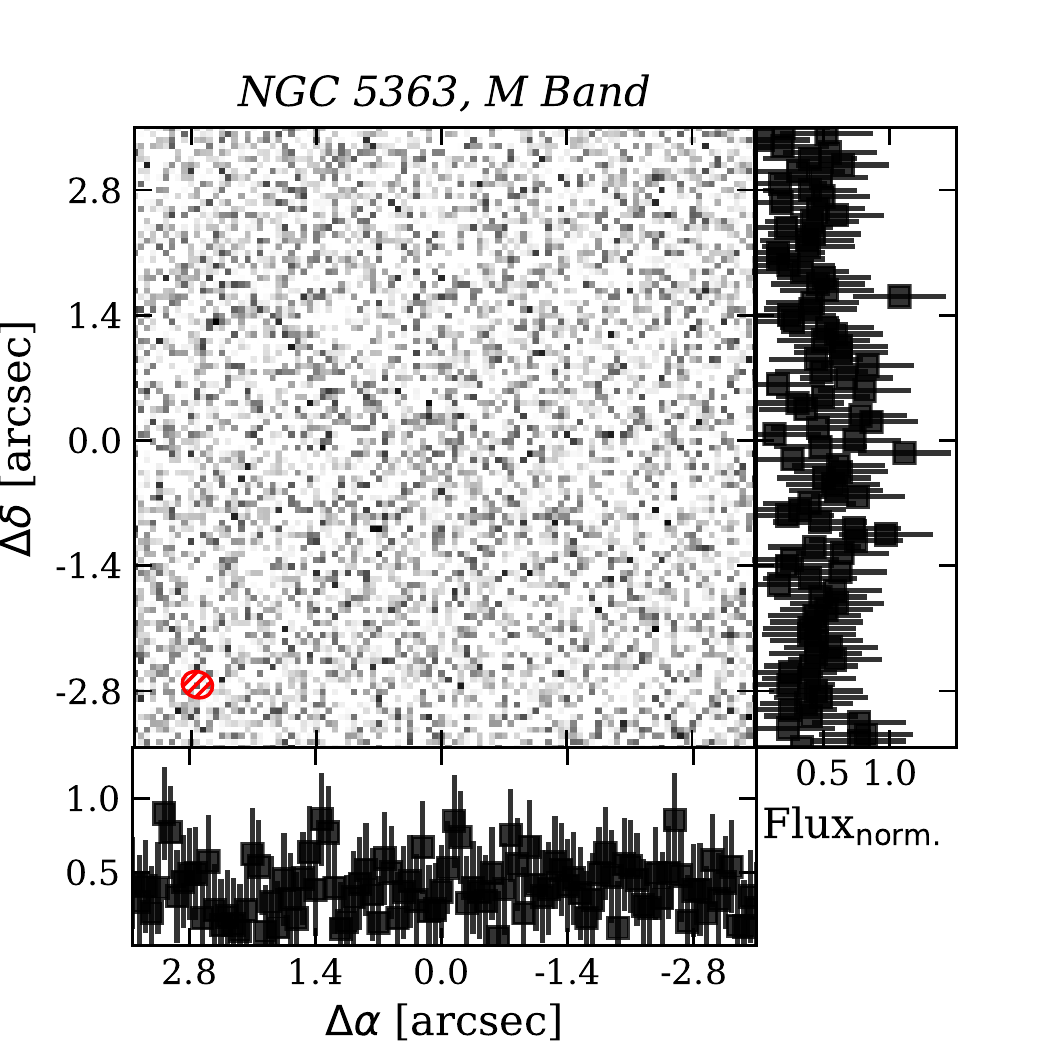}} \\
\subfloat{\includegraphics[width=0.25\hsize]{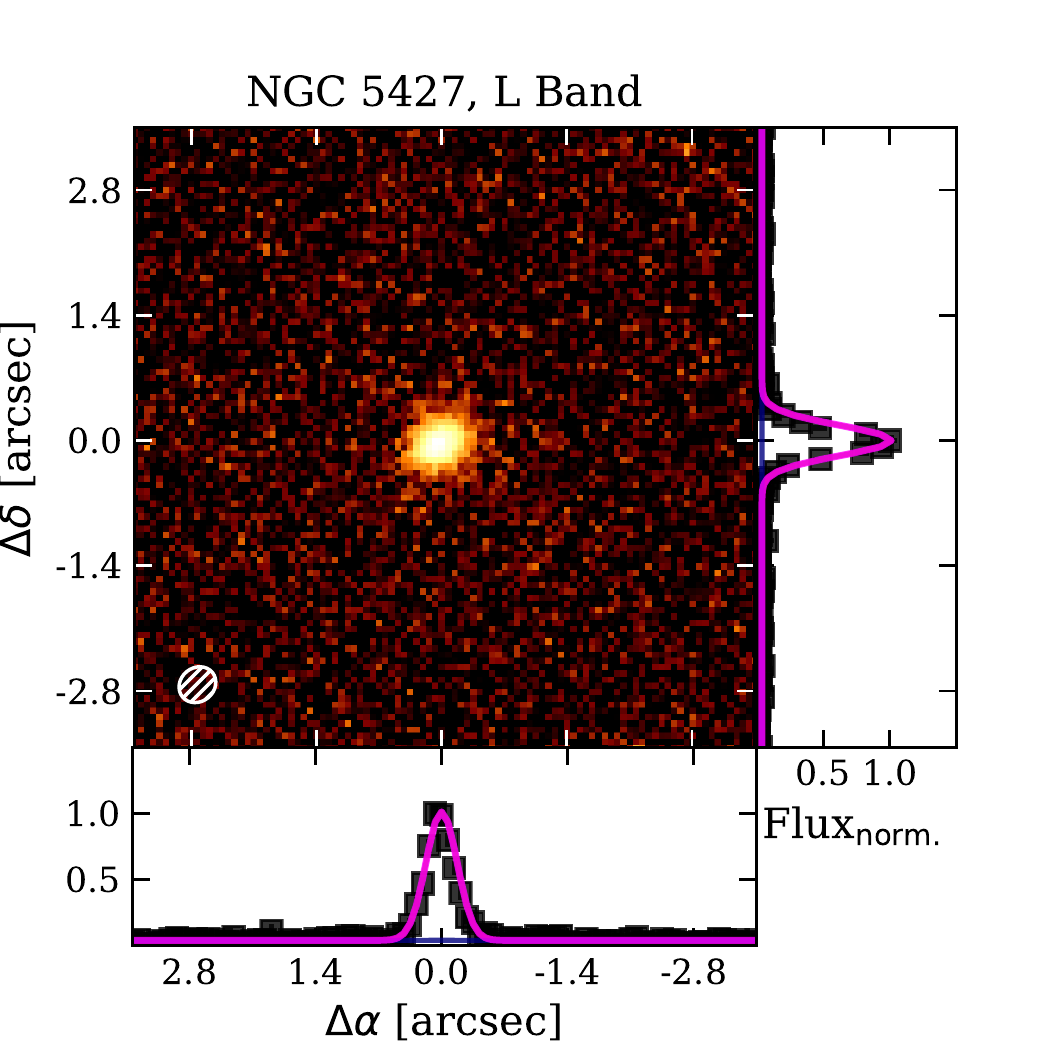}}
\subfloat{\includegraphics[width=0.25\hsize]{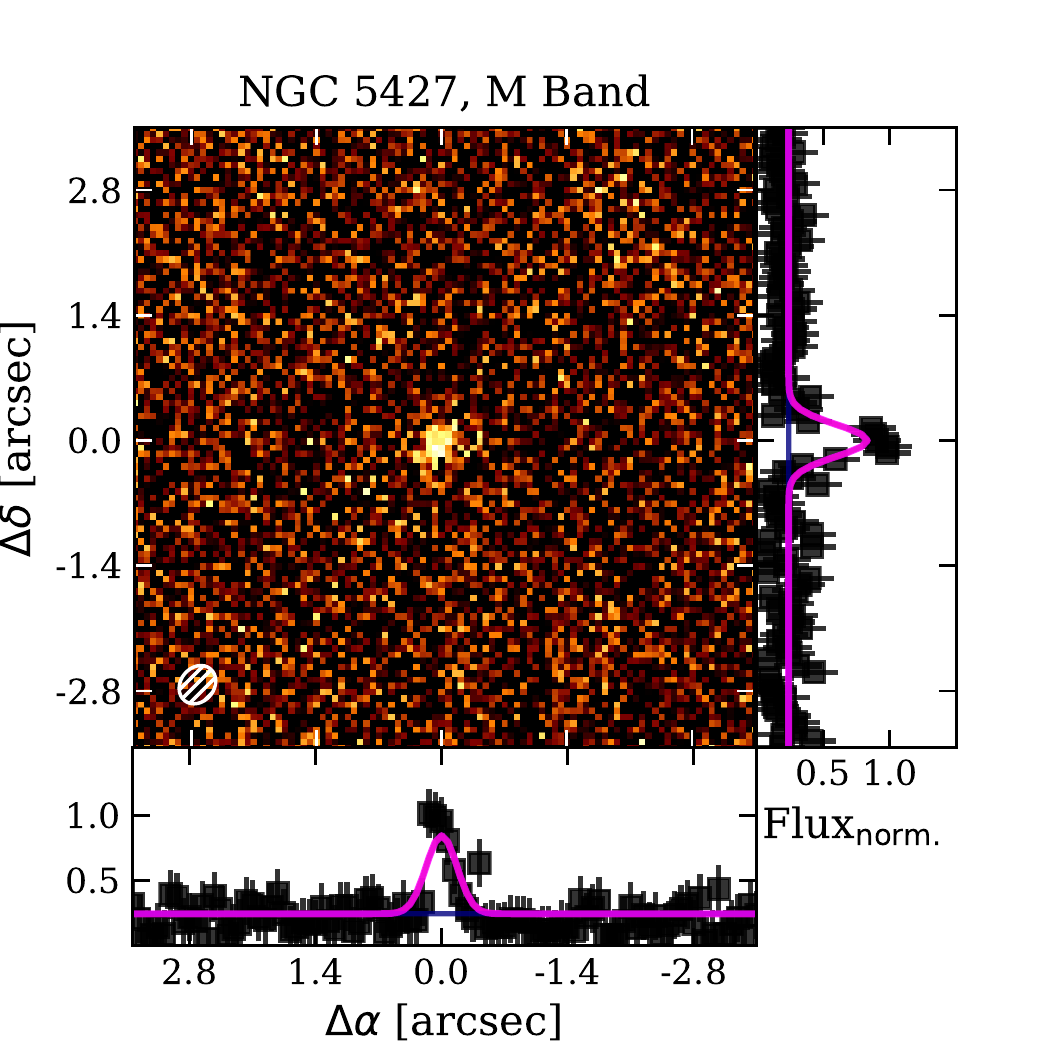}} 
\subfloat{\includegraphics[width=0.25\hsize]{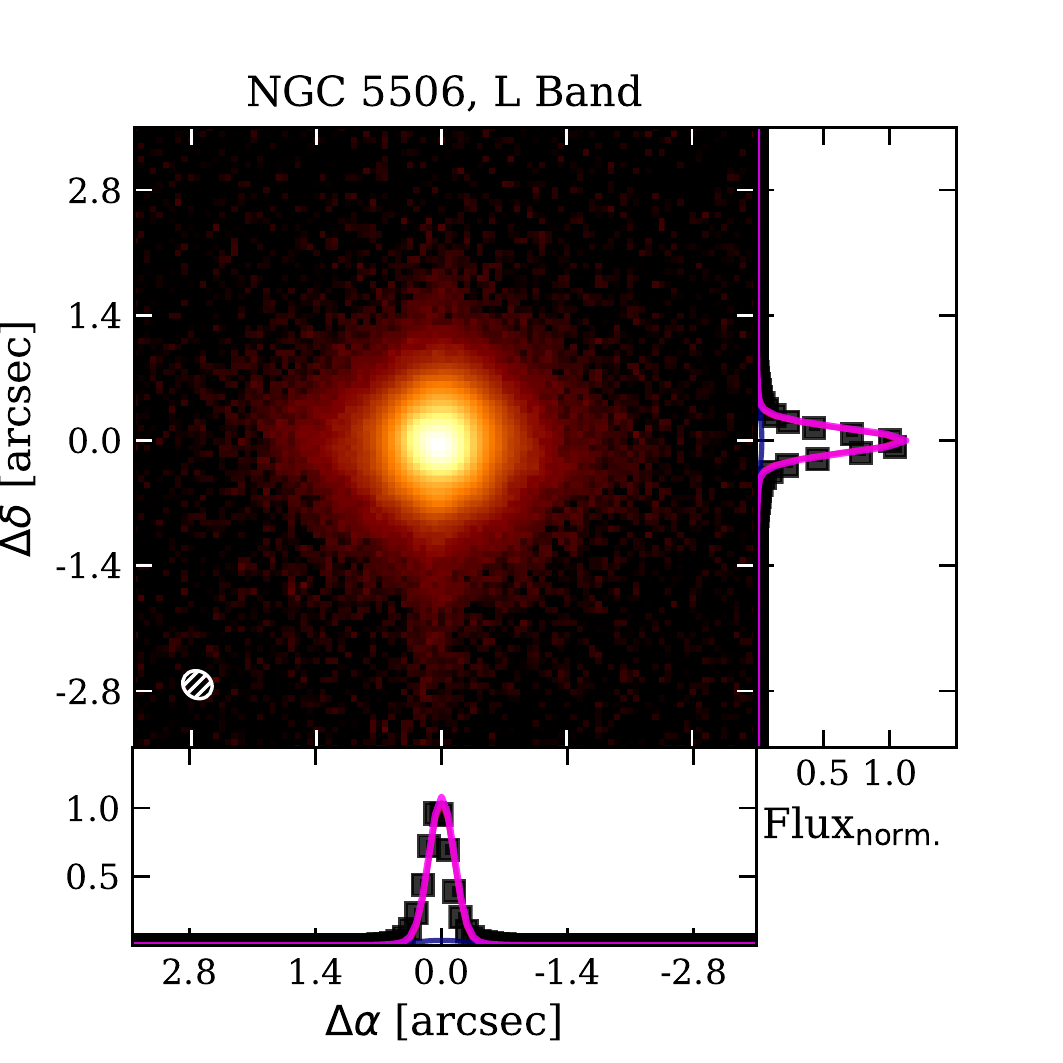}}
\subfloat{\includegraphics[width=0.25\hsize]{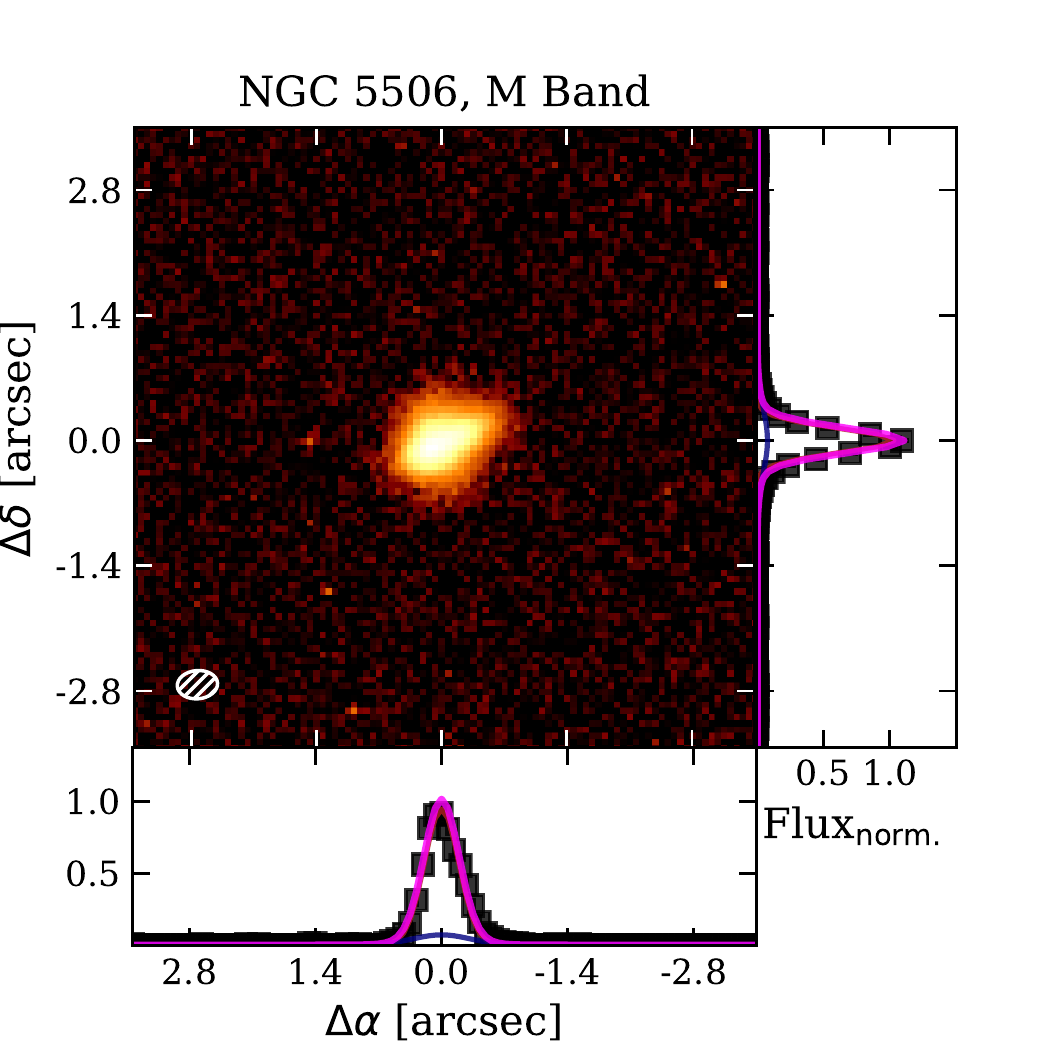}} \\
\caption{ As Fig \ref{fig:cutouts_one} but for all sources.}
\end{figure*}
\begin{figure*}
\subfloat{\includegraphics[width=0.25\hsize]{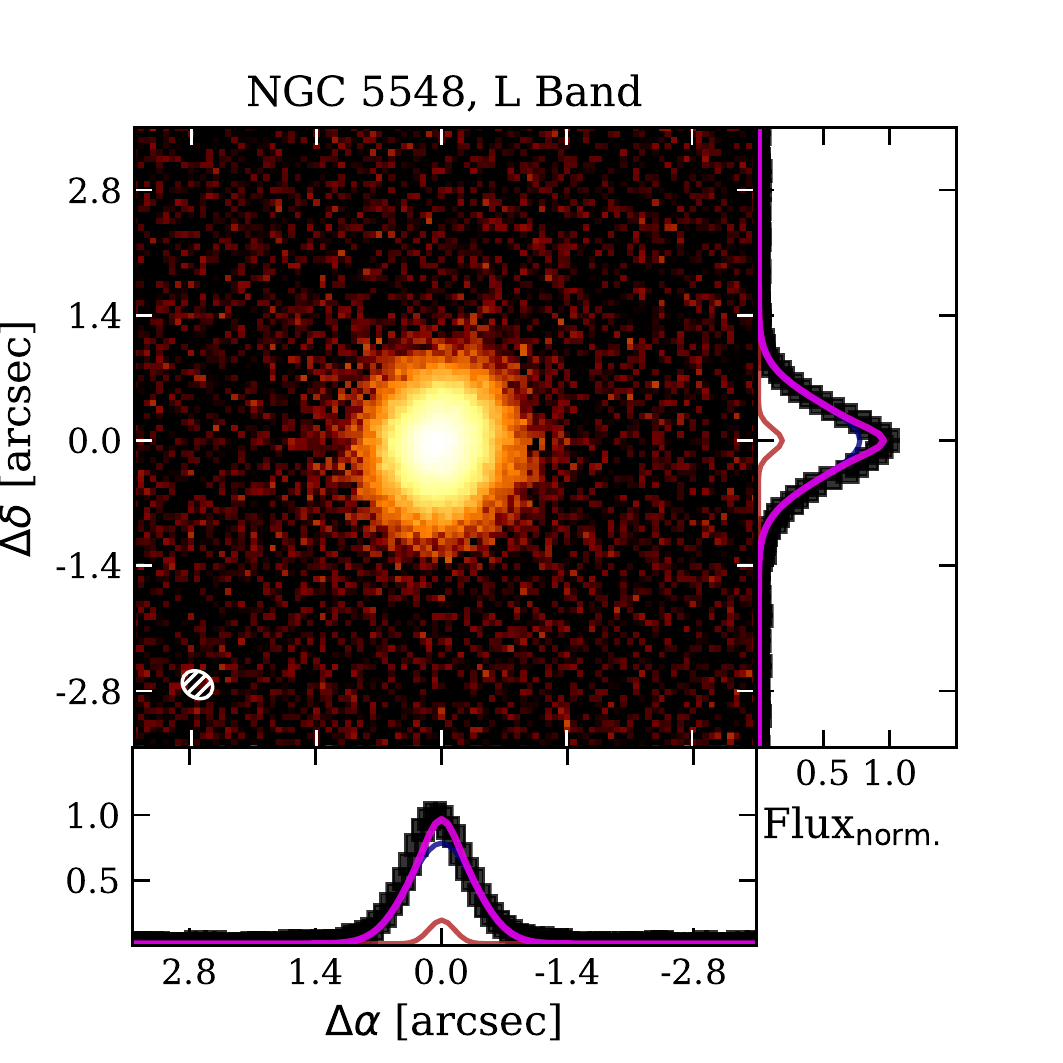}}
\subfloat{\includegraphics[width=0.25\hsize]{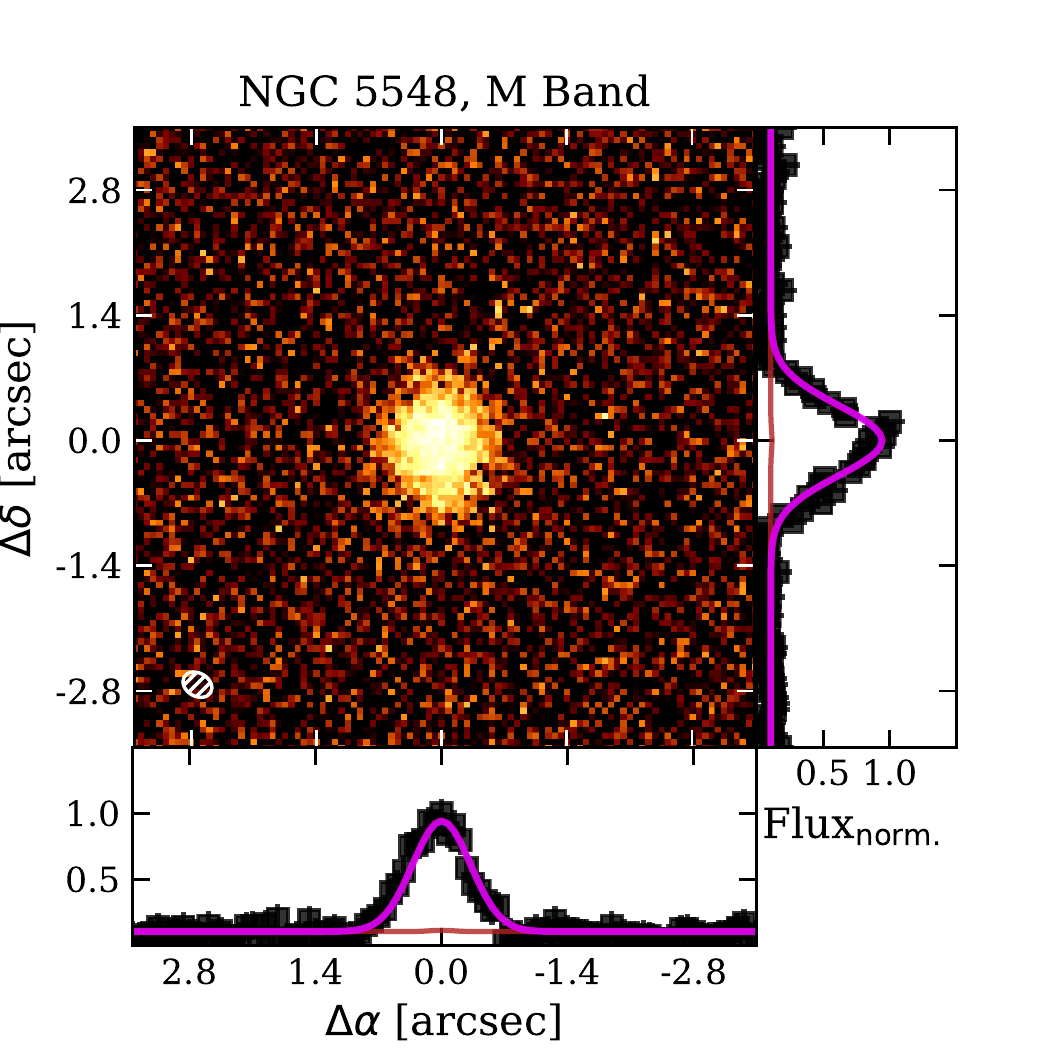}} 
\subfloat{\includegraphics[width=0.25\hsize]{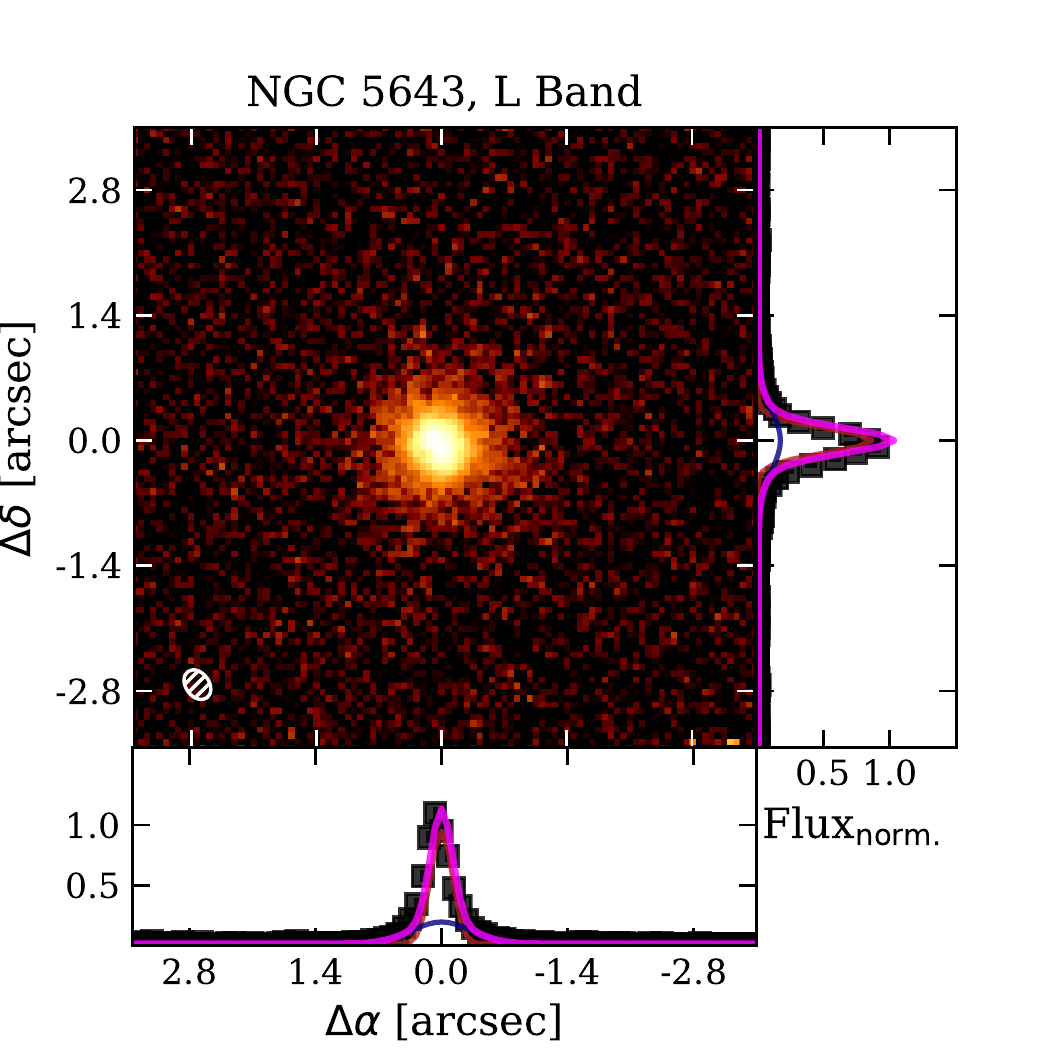}}
\subfloat{\includegraphics[width=0.25\hsize]{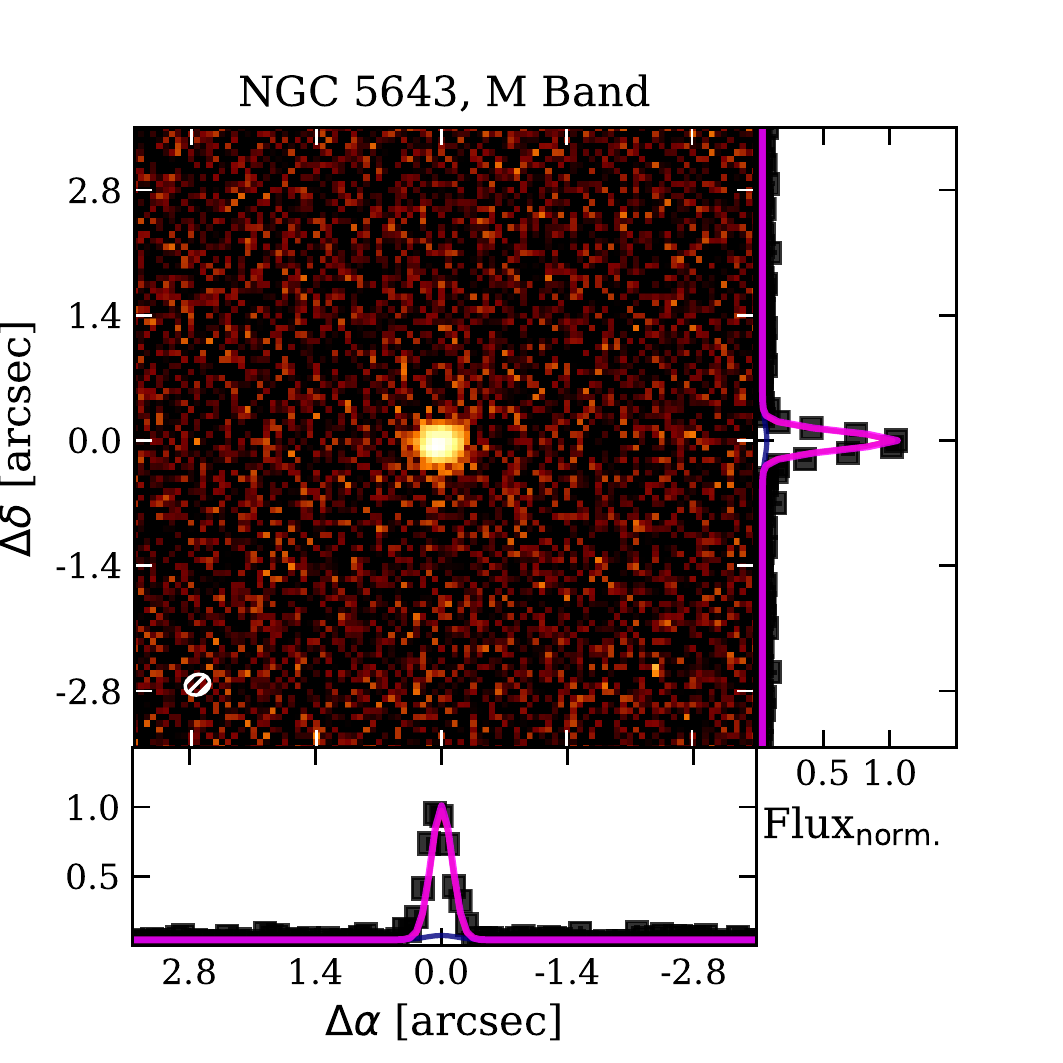}} \\
\subfloat{\includegraphics[width=0.25\hsize]{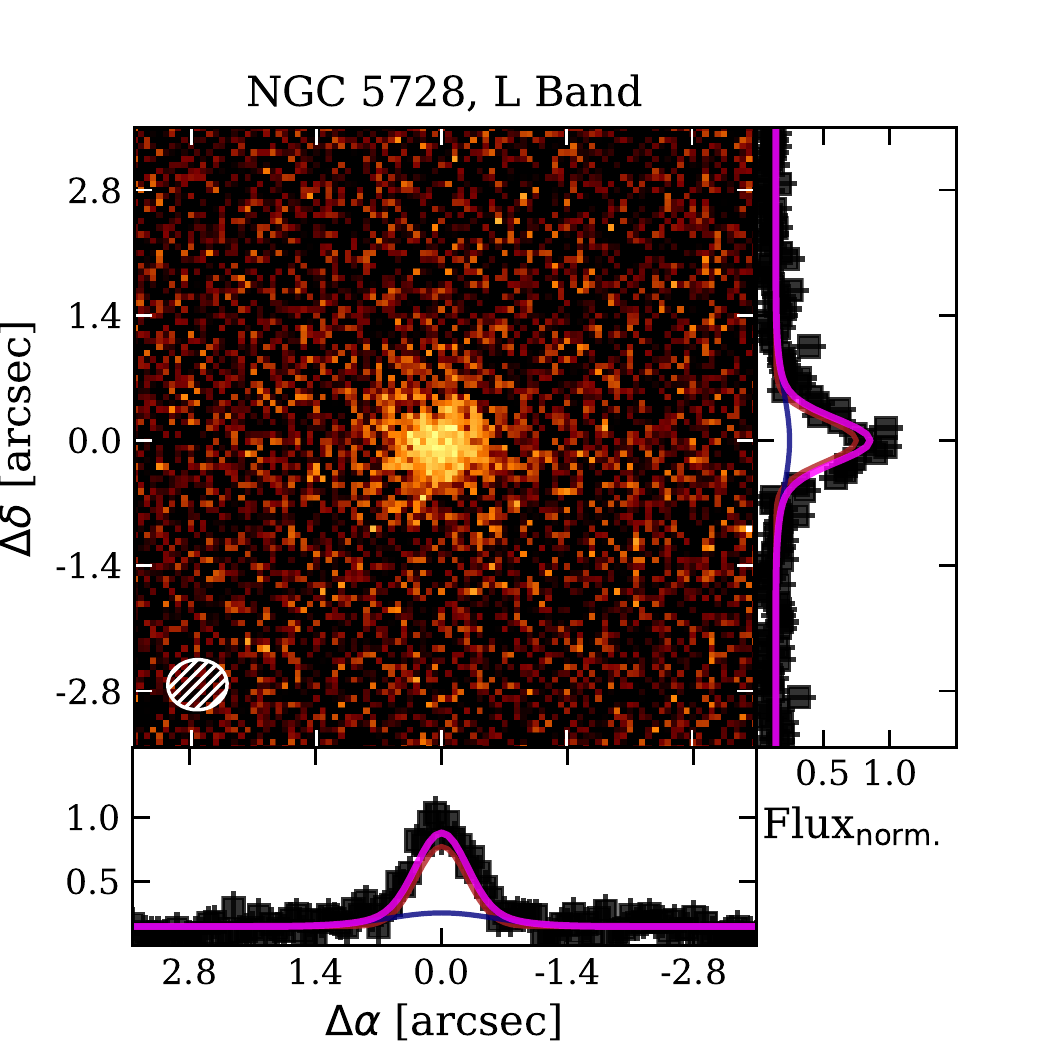}}
\subfloat{\includegraphics[width=0.25\hsize]{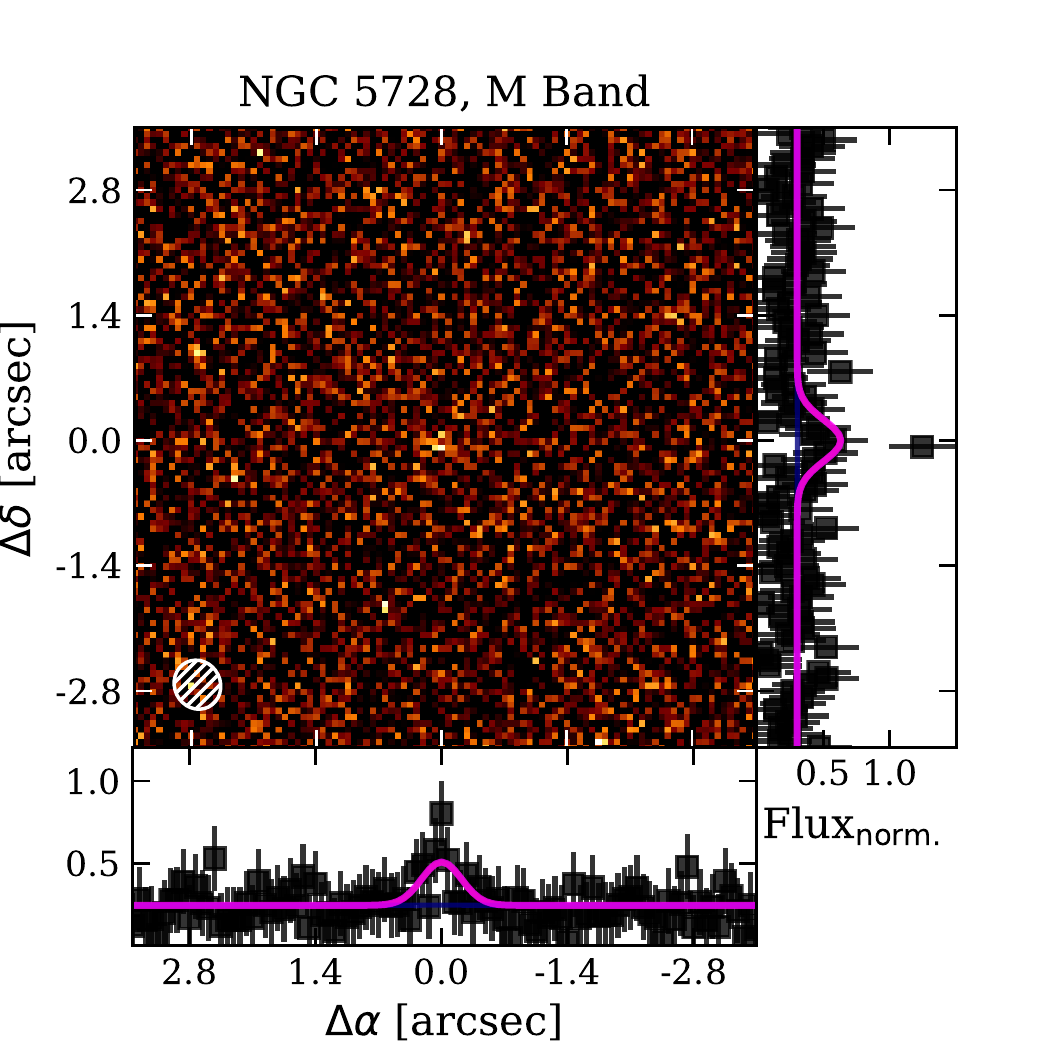}} 
\subfloat{\includegraphics[width=0.25\hsize]{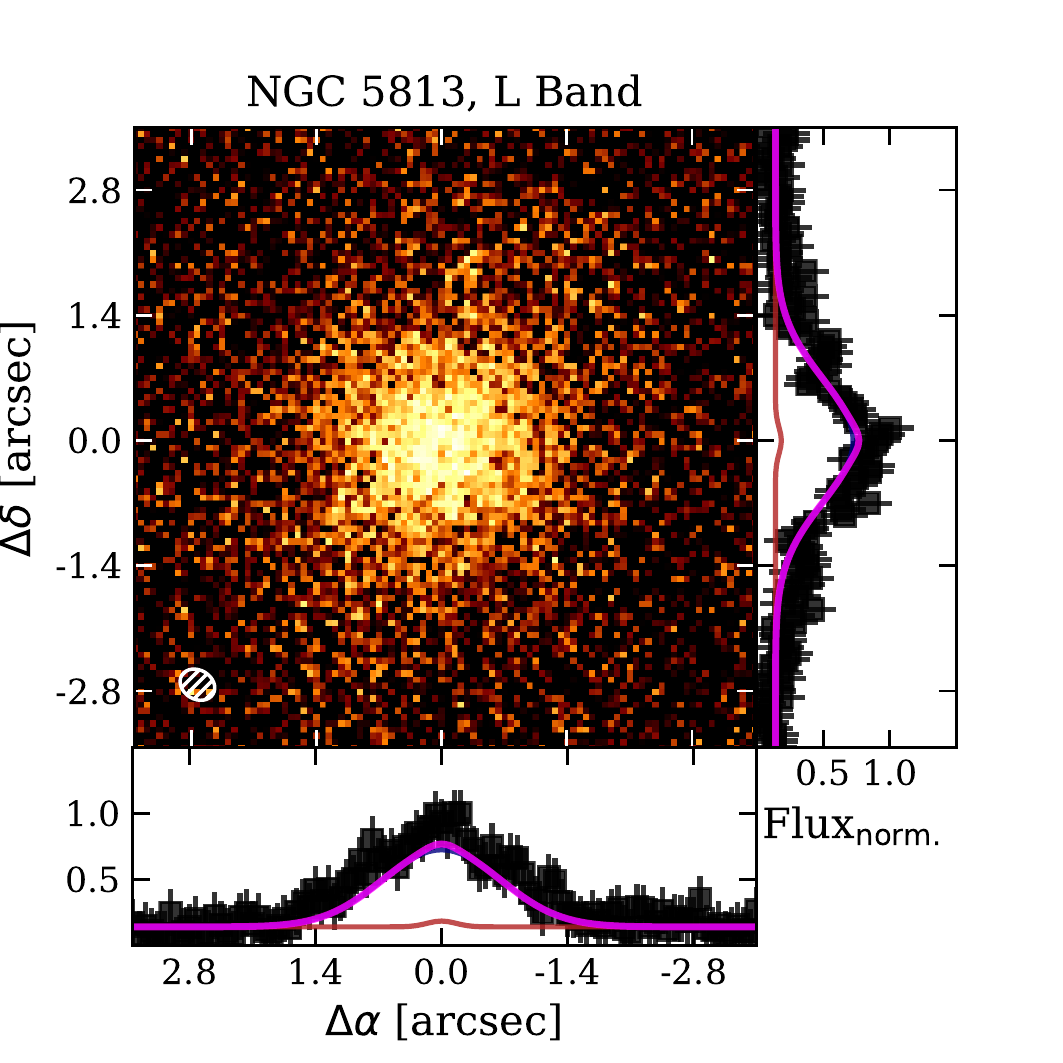}}
\subfloat{\includegraphics[width=0.25\hsize]{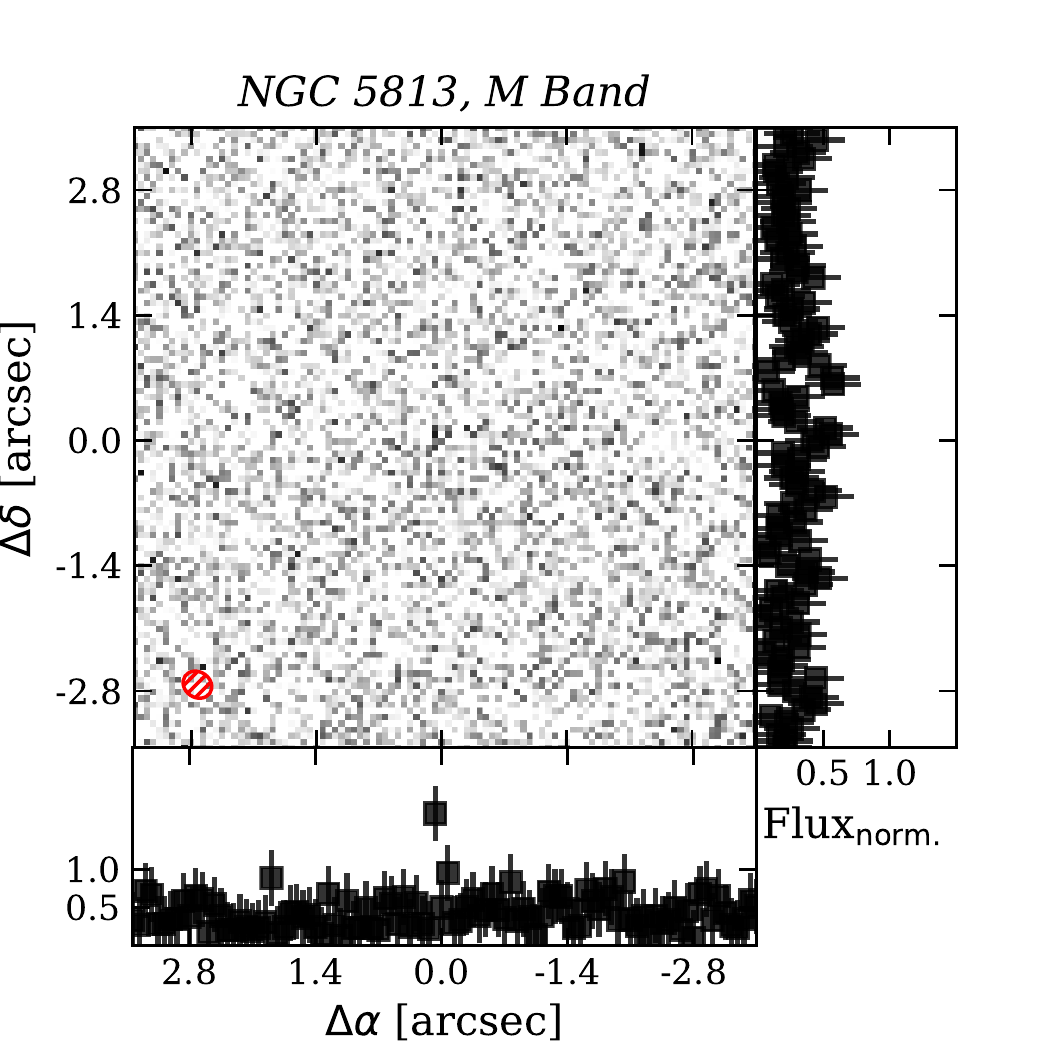}} \\
\subfloat{\includegraphics[width=0.25\hsize]{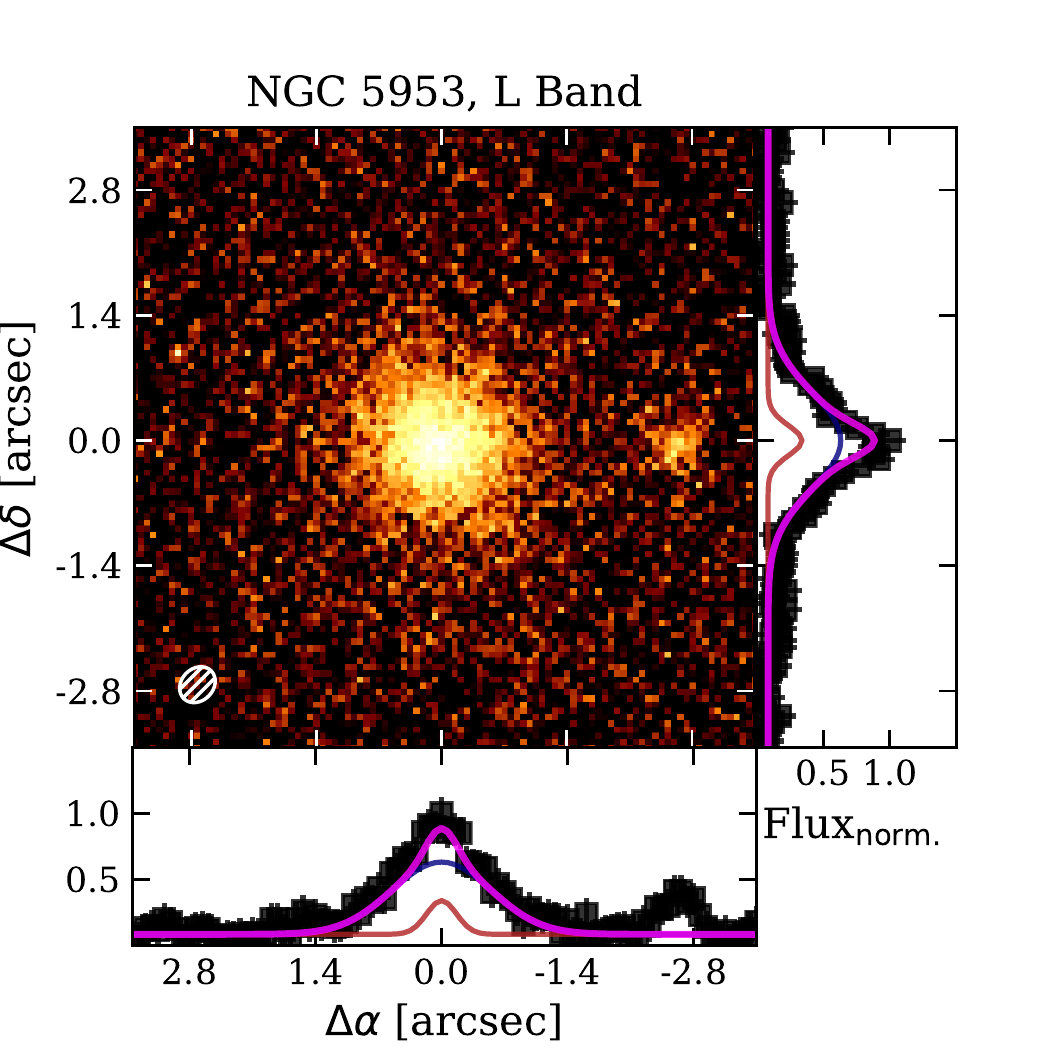}}
\subfloat{\includegraphics[width=0.25\hsize]{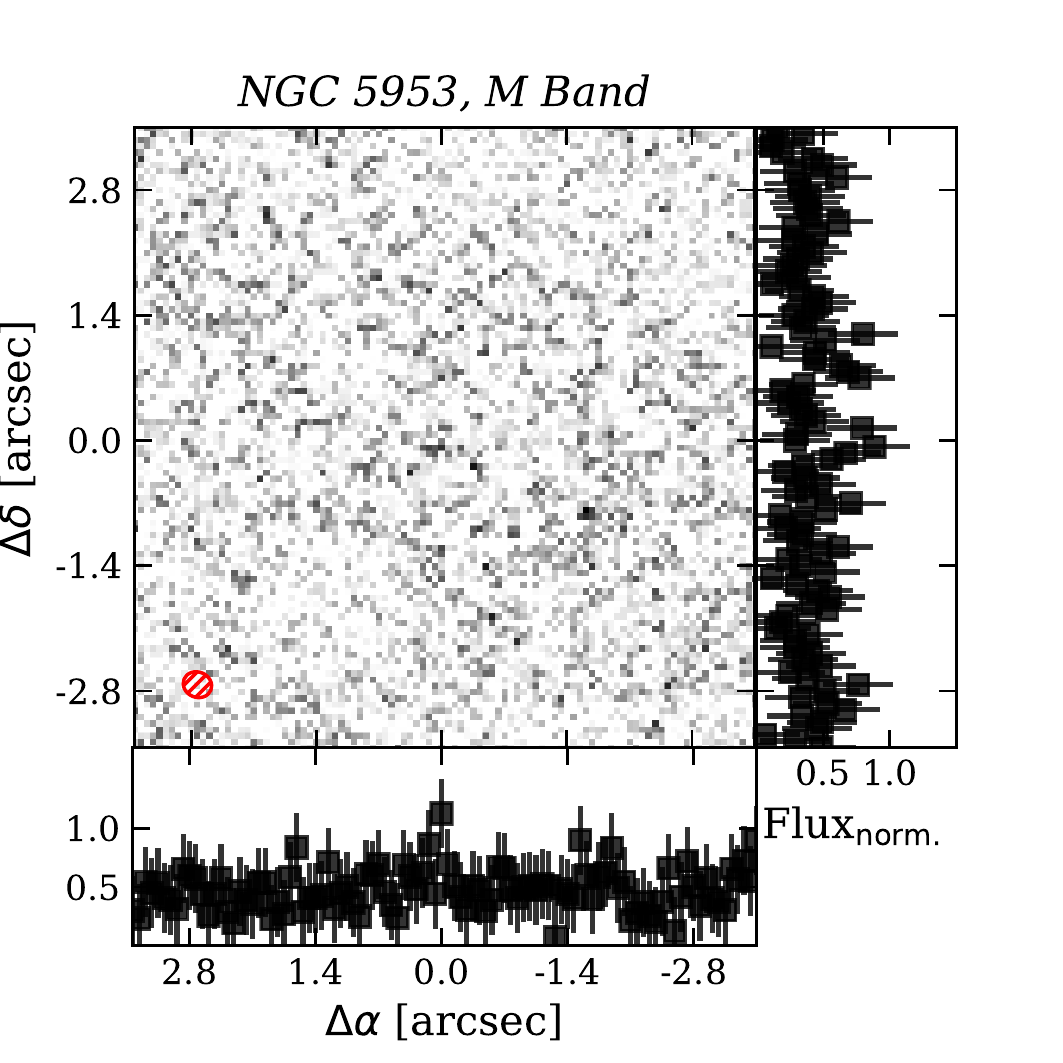}} 
\subfloat{\includegraphics[width=0.25\hsize]{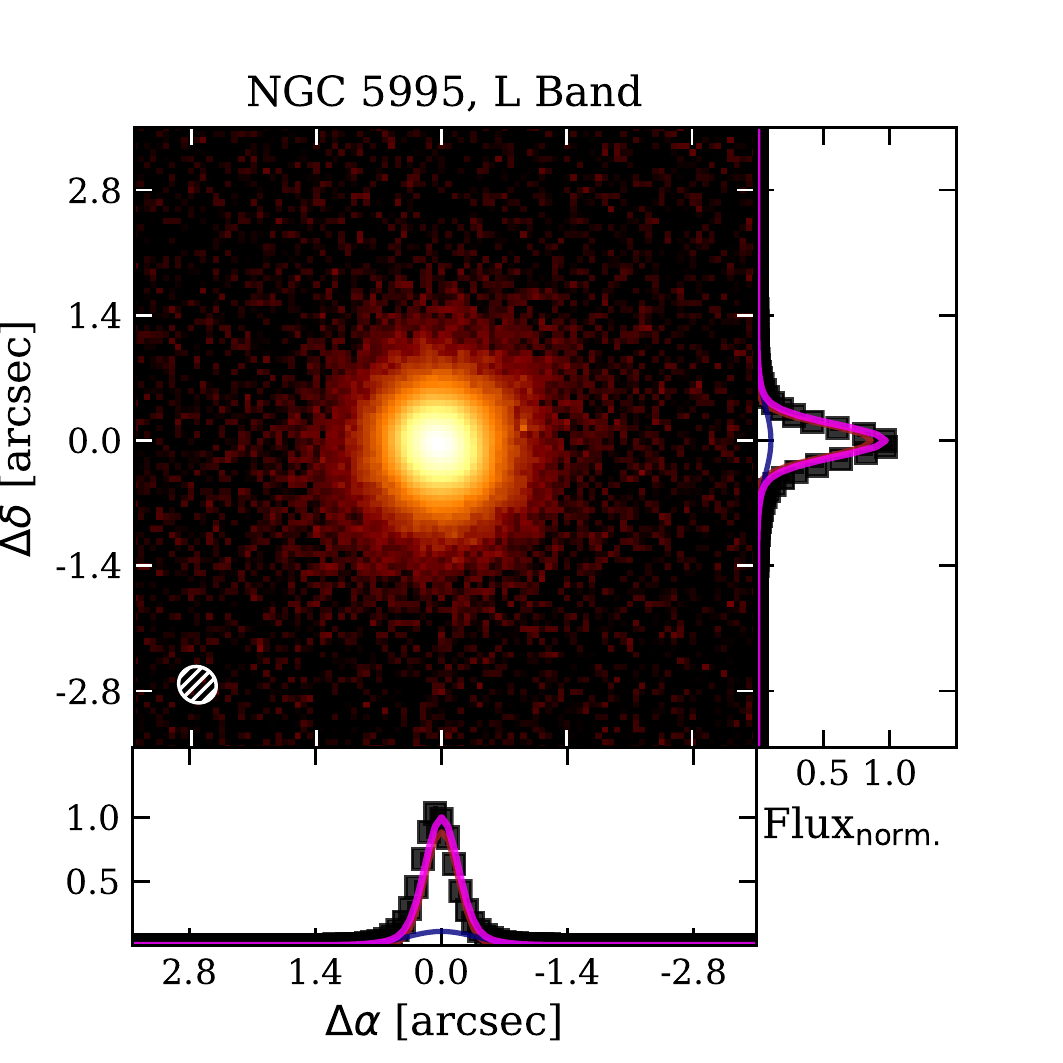}}
\subfloat{\includegraphics[width=0.25\hsize]{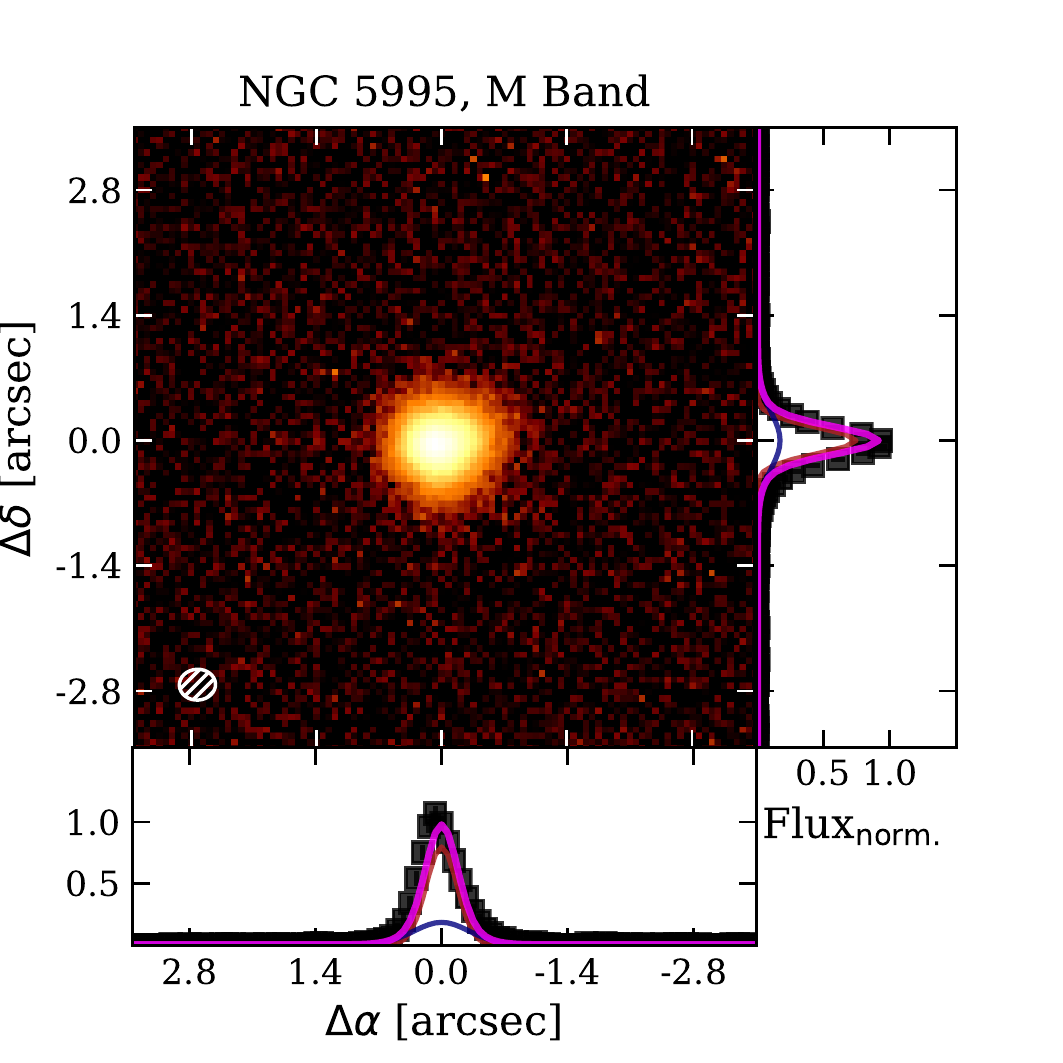}} \\
\subfloat{\includegraphics[width=0.25\hsize]{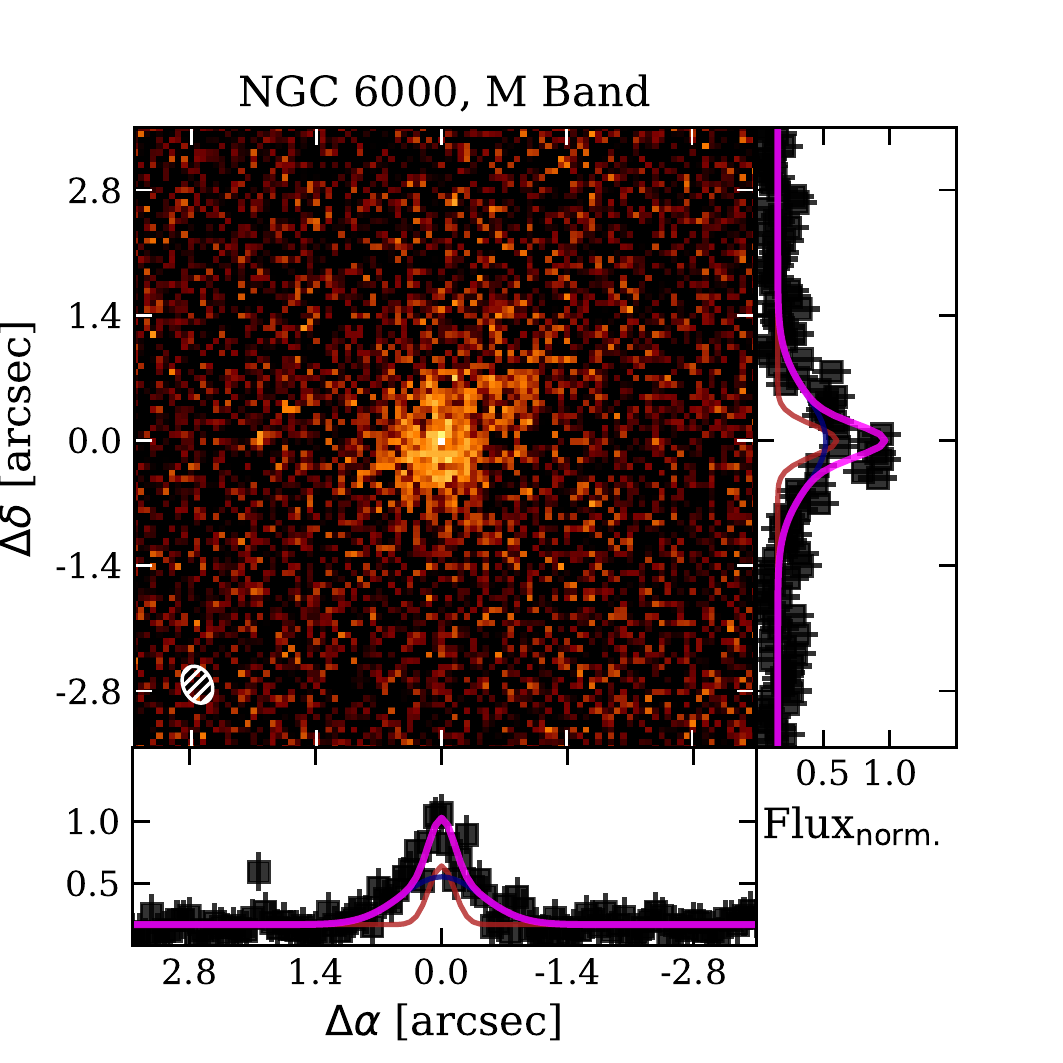}}
\subfloat{\includegraphics[width=0.25\hsize]{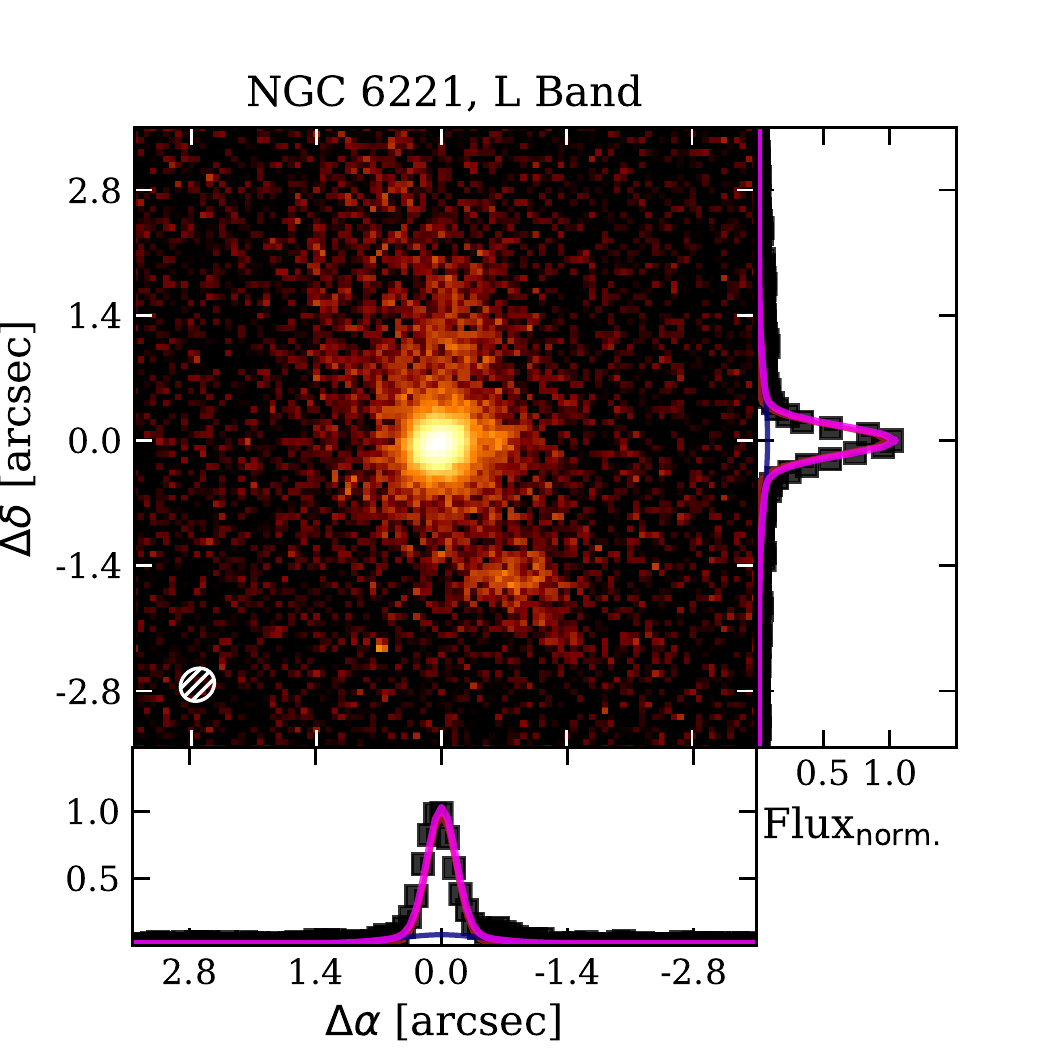}} 
\subfloat{\includegraphics[width=0.25\hsize]{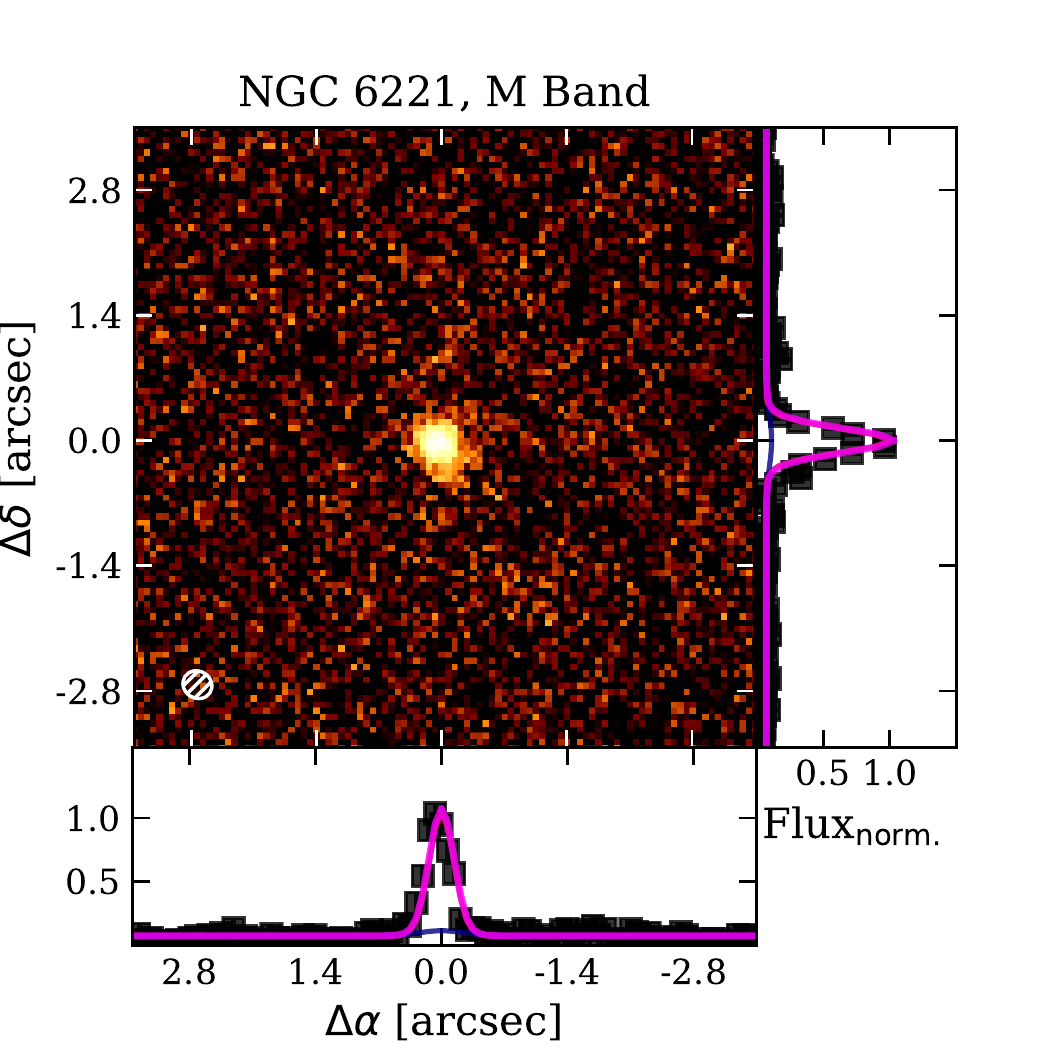}}
\subfloat{\includegraphics[width=0.25\hsize]{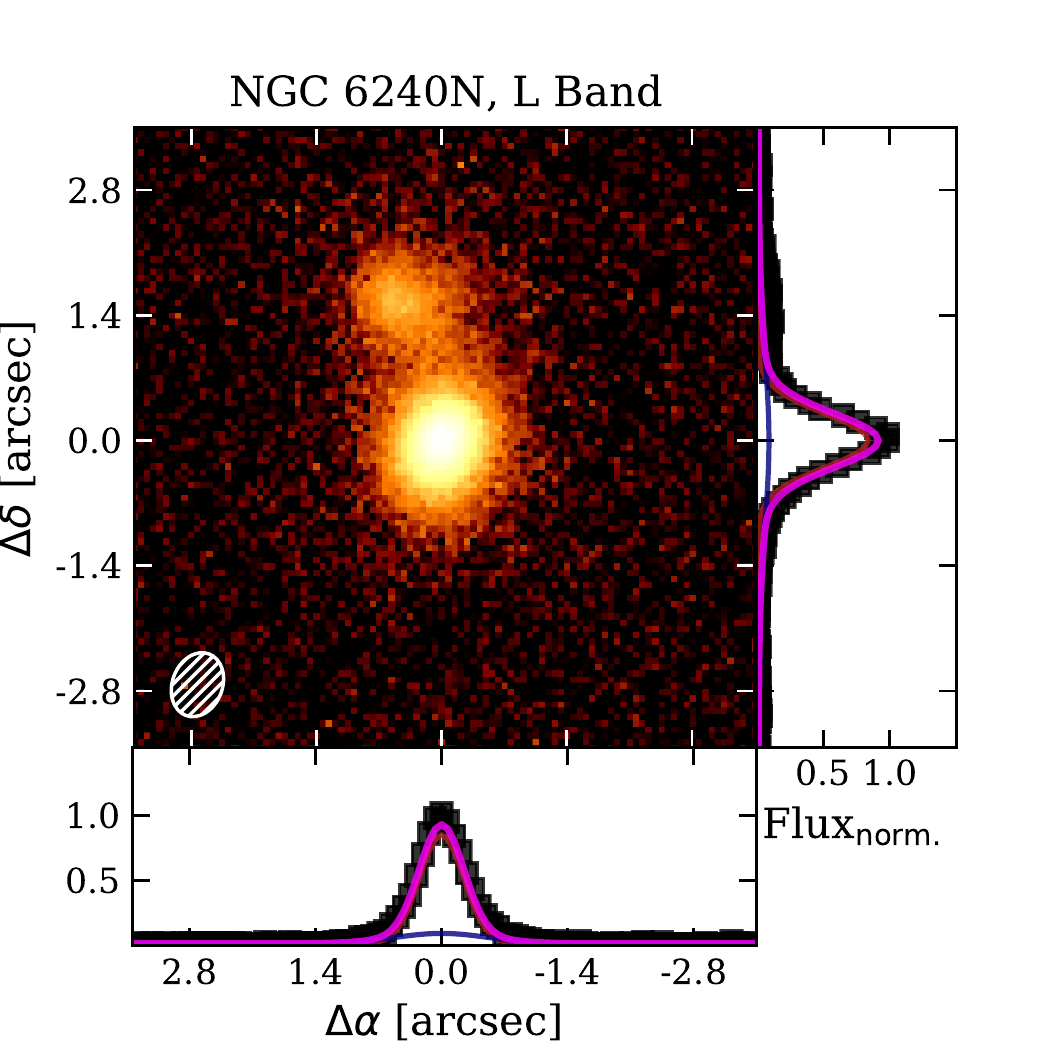}} \\
\subfloat{\includegraphics[width=0.25\hsize]{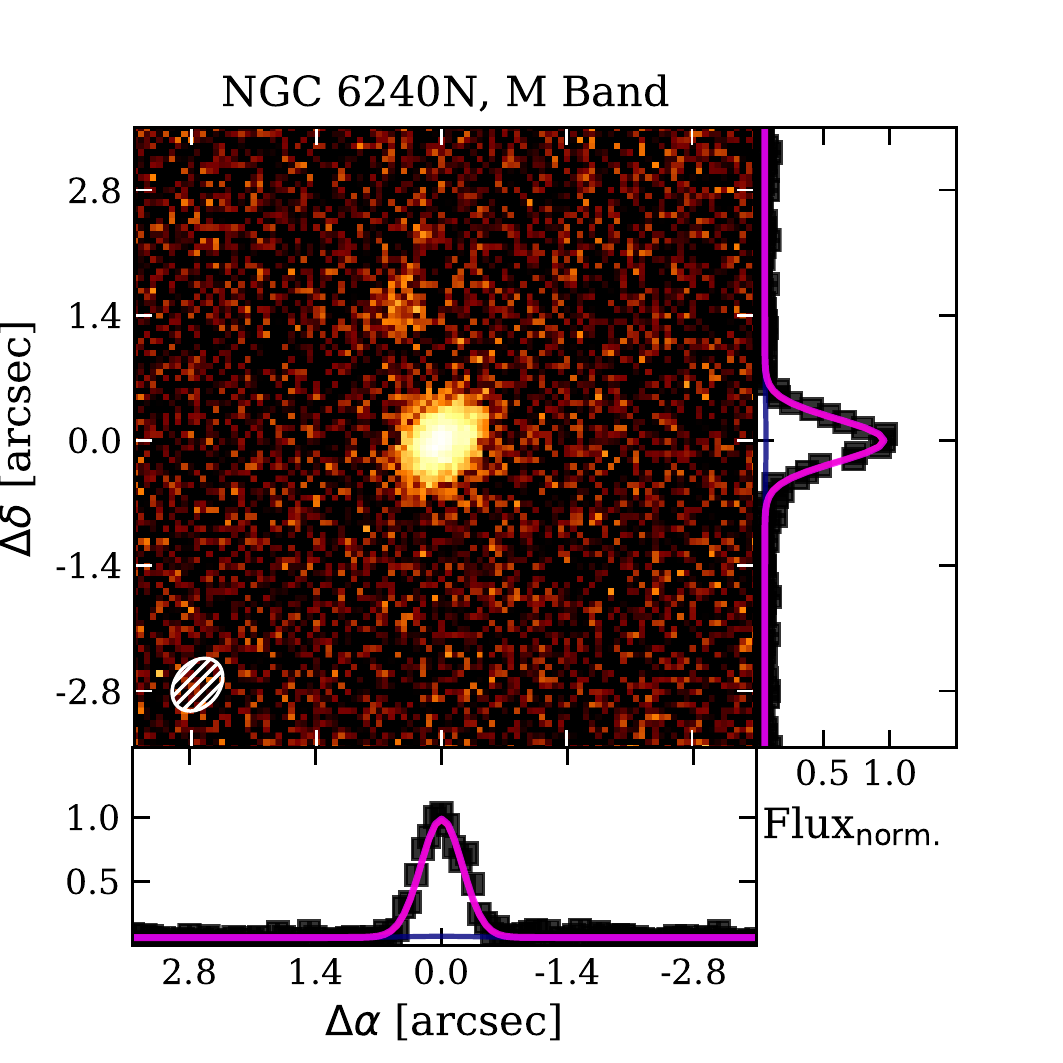}}
\subfloat{\includegraphics[width=0.25\hsize]{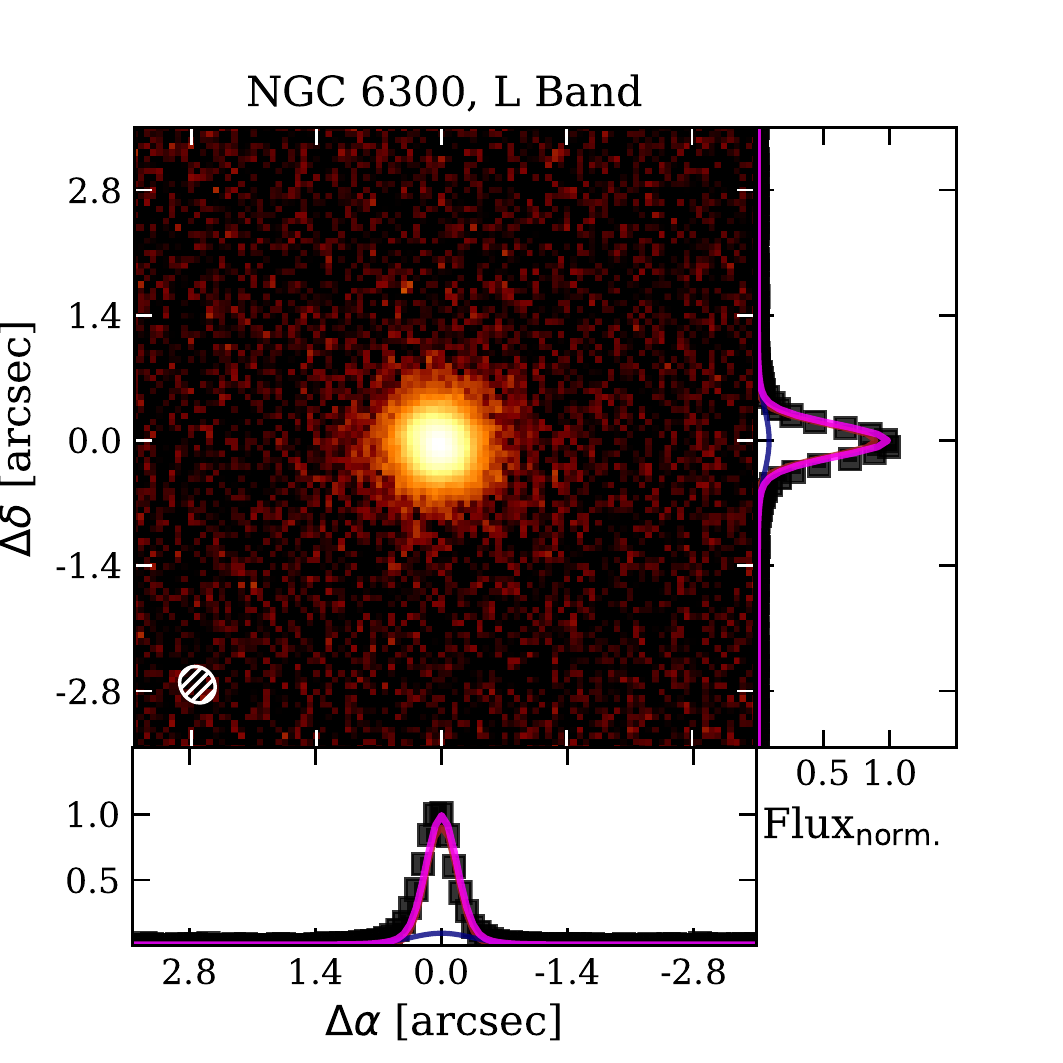}} 
\subfloat{\includegraphics[width=0.25\hsize]{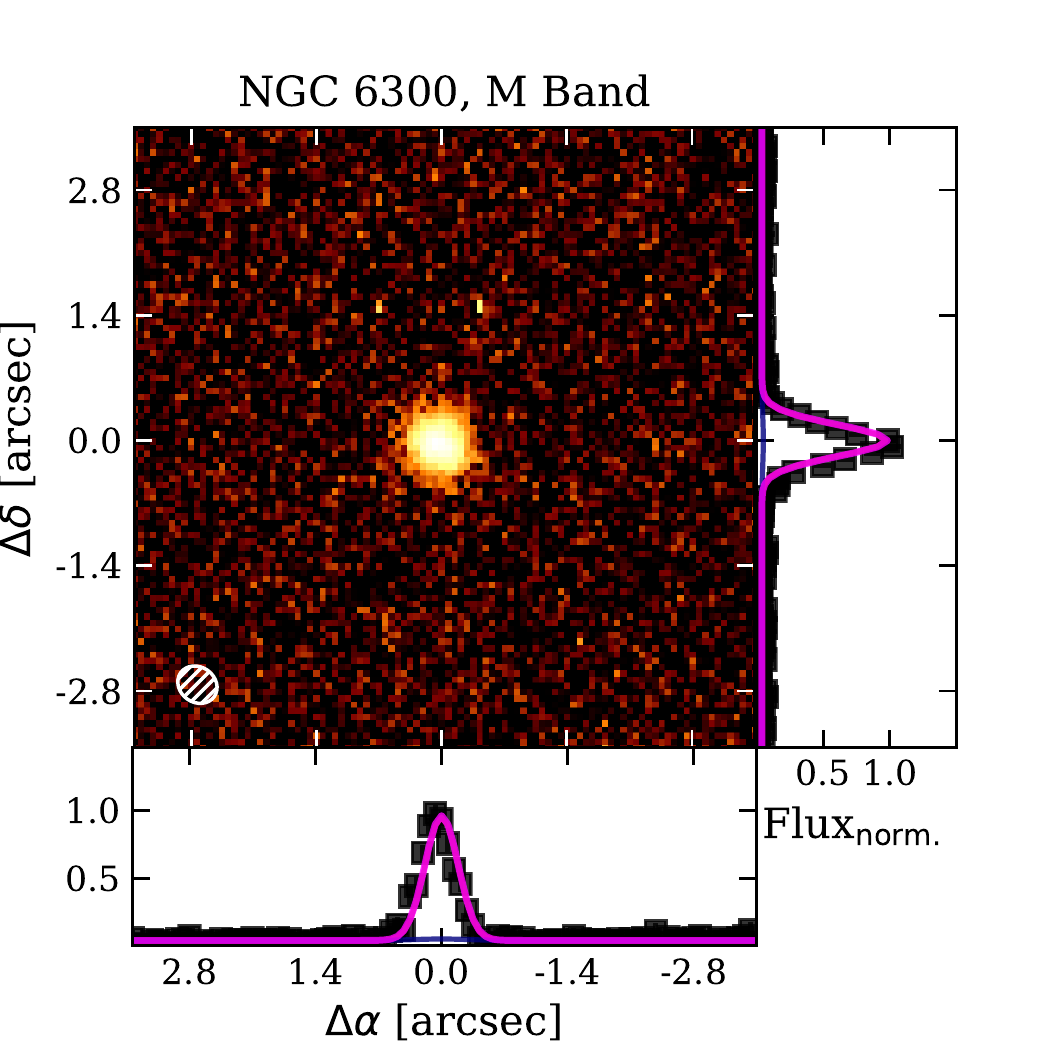}}
\subfloat{\includegraphics[width=0.25\hsize]{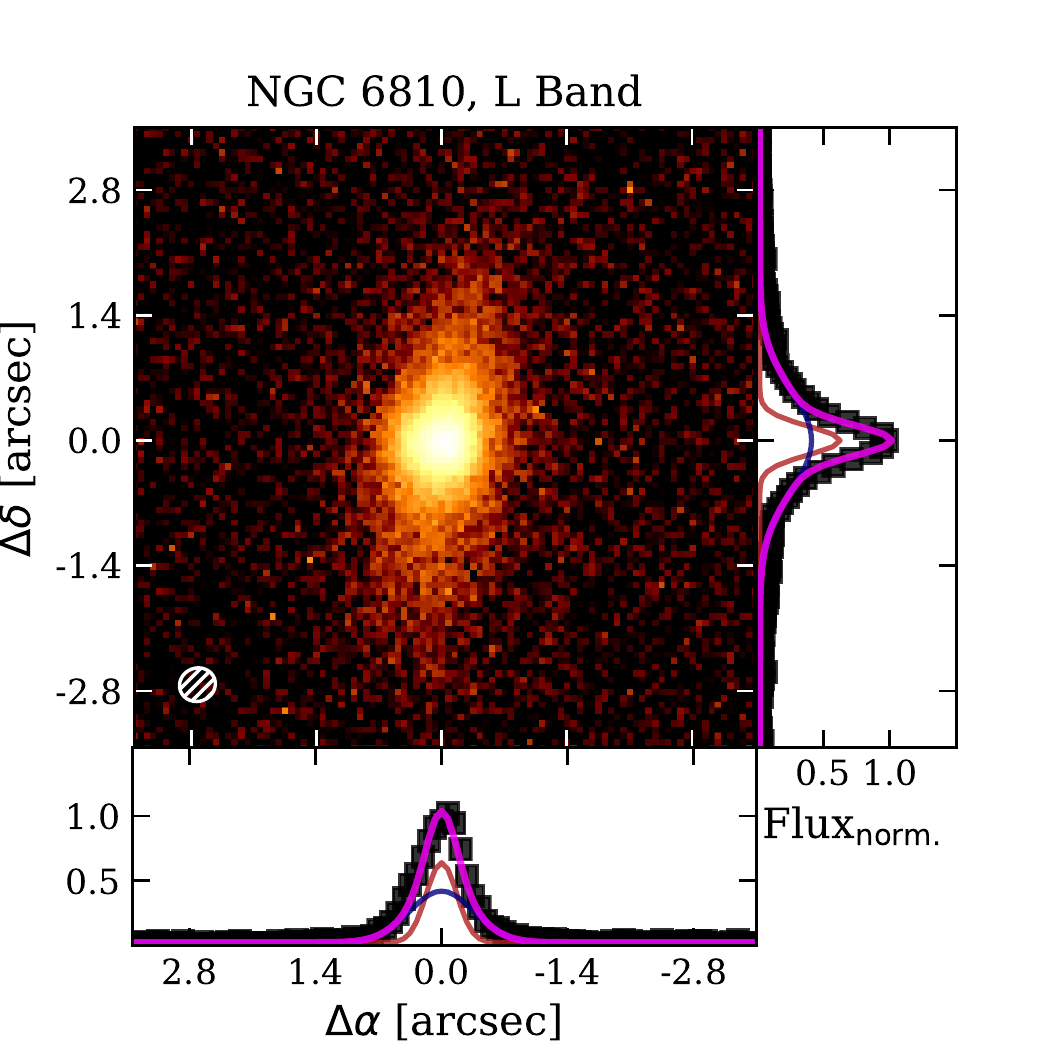}} \\
\caption{ As Fig \ref{fig:cutouts_one} but for all sources.}
\end{figure*}
\begin{figure*}
\subfloat{\includegraphics[width=0.25\hsize]{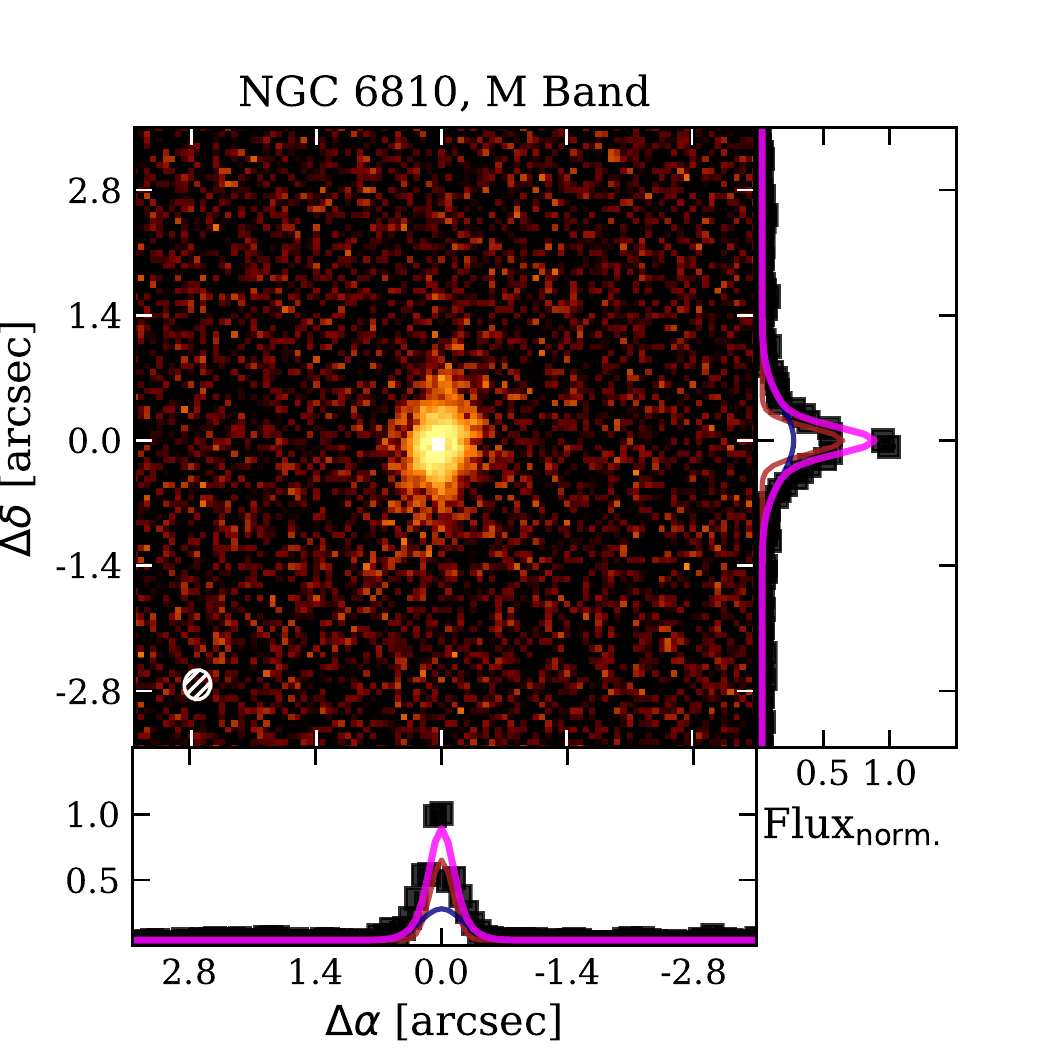}}
\subfloat{\includegraphics[width=0.25\hsize]{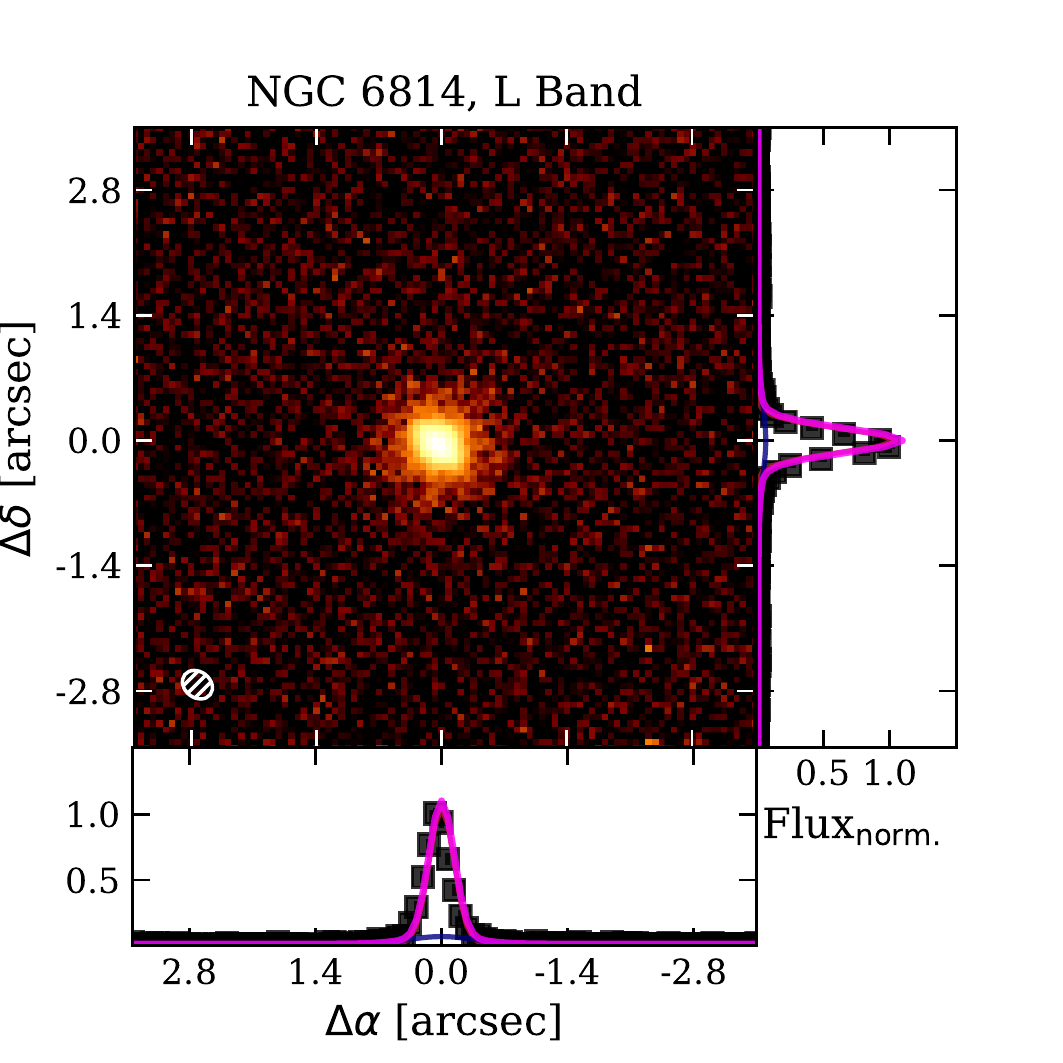}} 
\subfloat{\includegraphics[width=0.25\hsize]{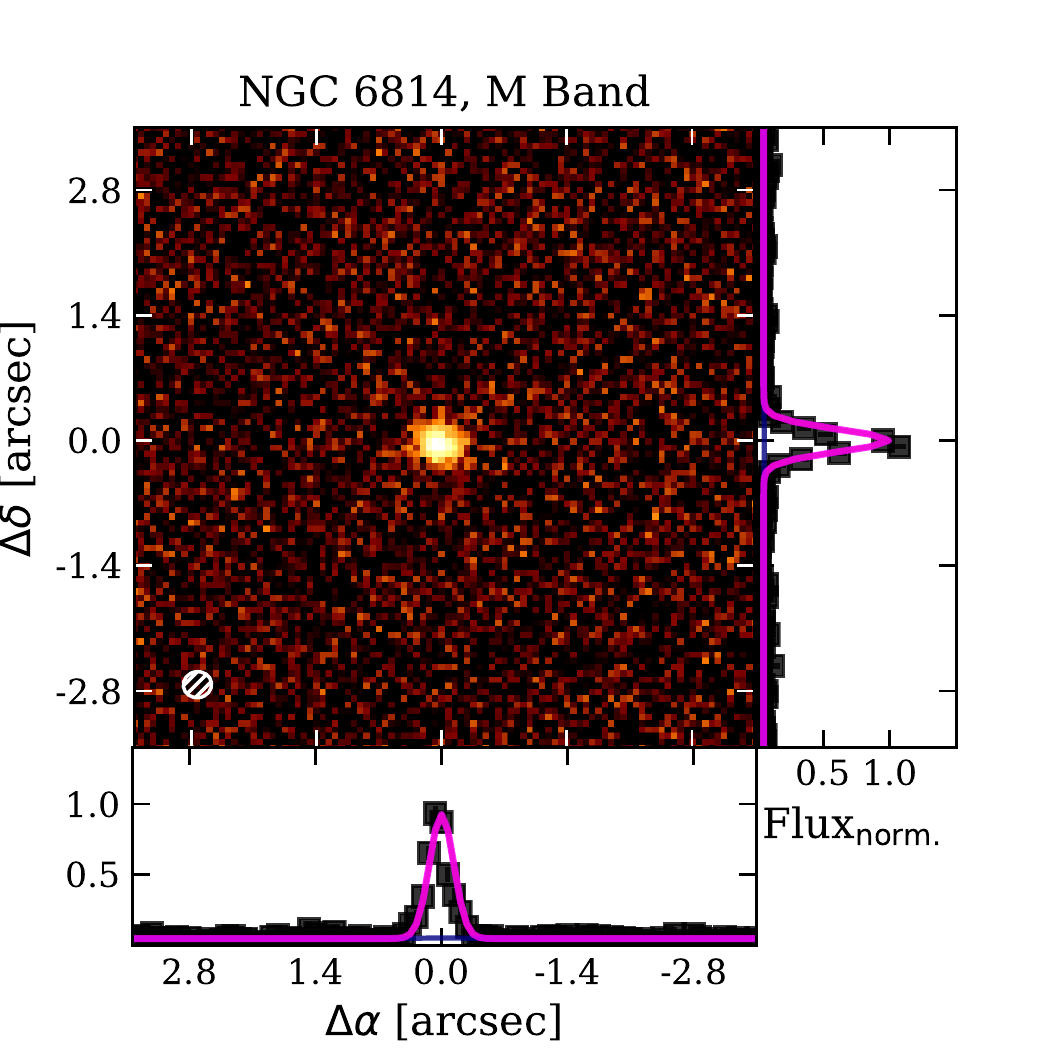}}
\subfloat{\includegraphics[width=0.25\hsize]{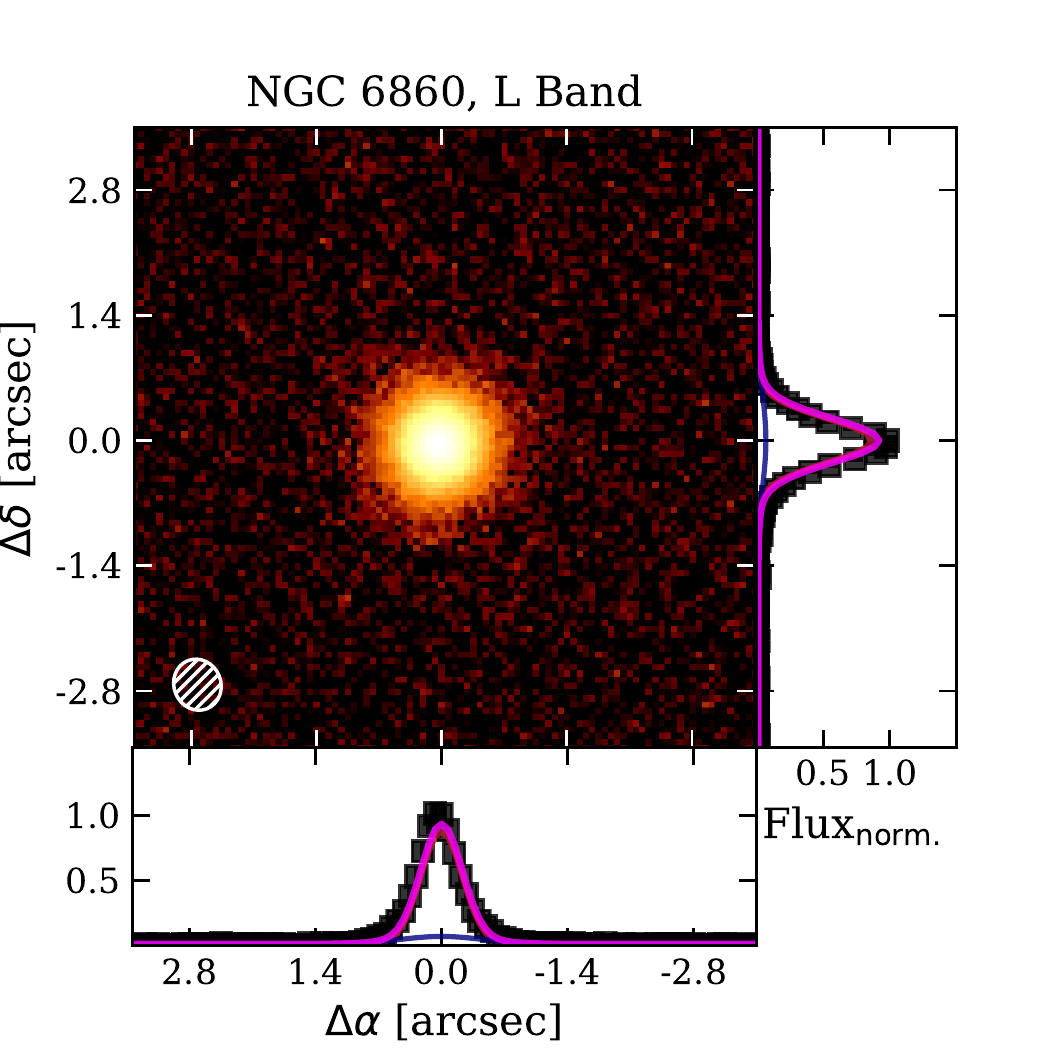}} \\
\subfloat{\includegraphics[width=0.25\hsize]{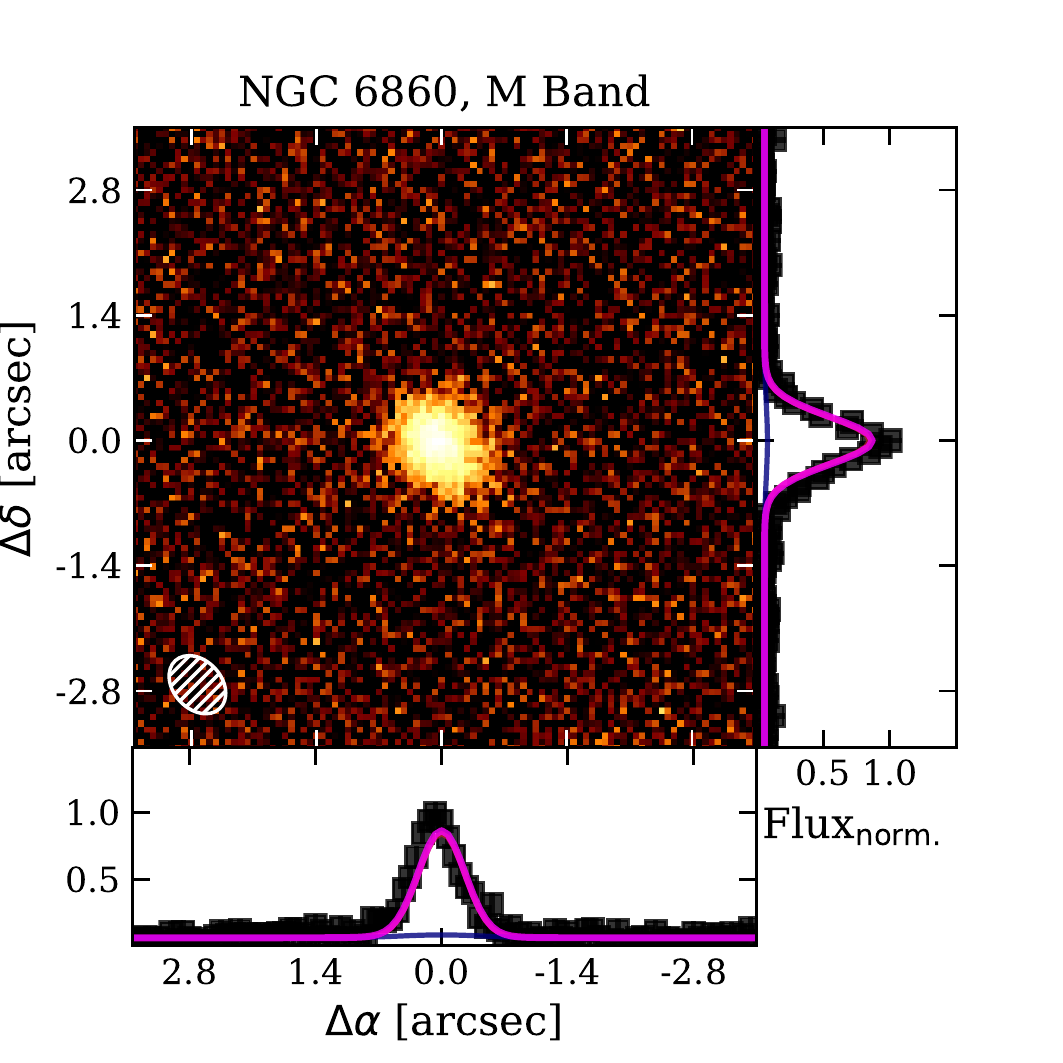}}
\subfloat{\includegraphics[width=0.25\hsize]{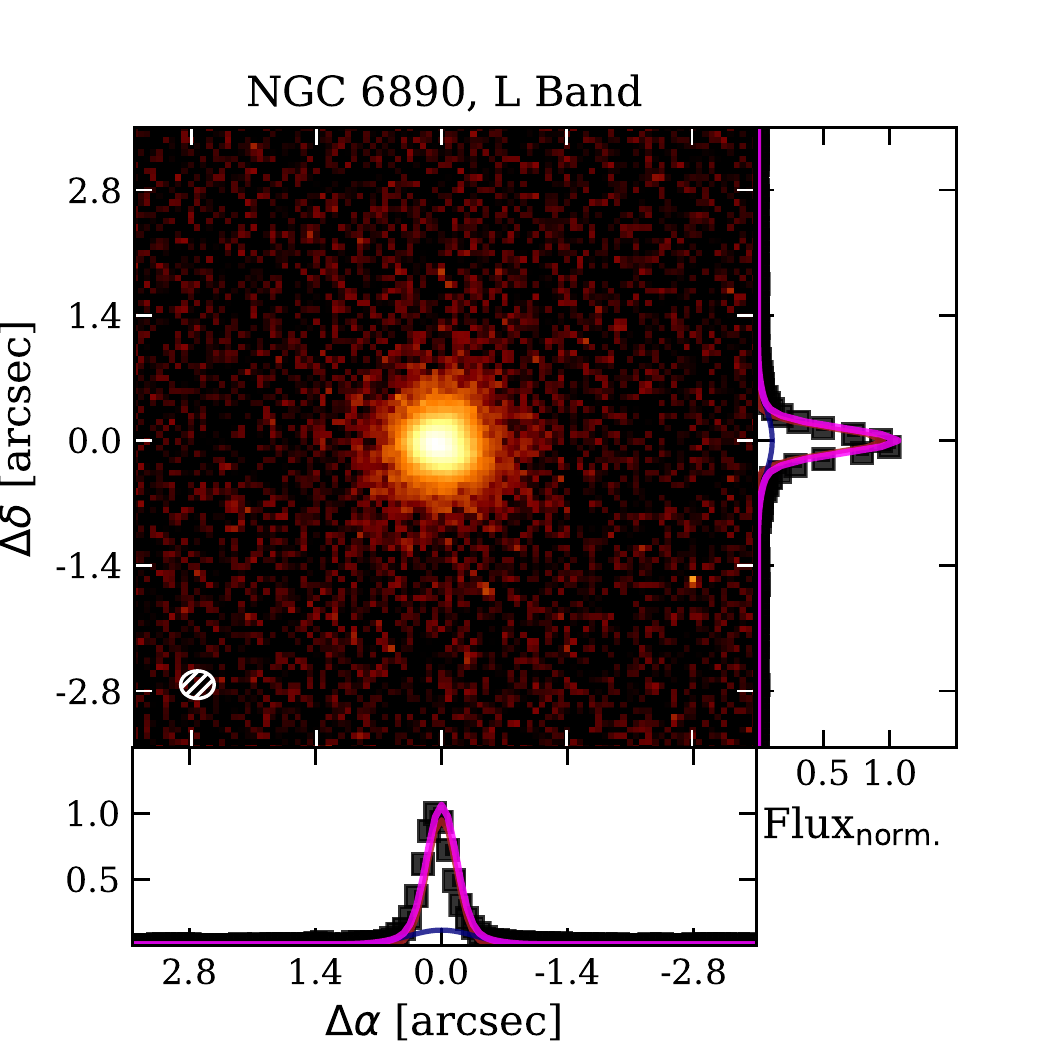}} 
\subfloat{\includegraphics[width=0.25\hsize]{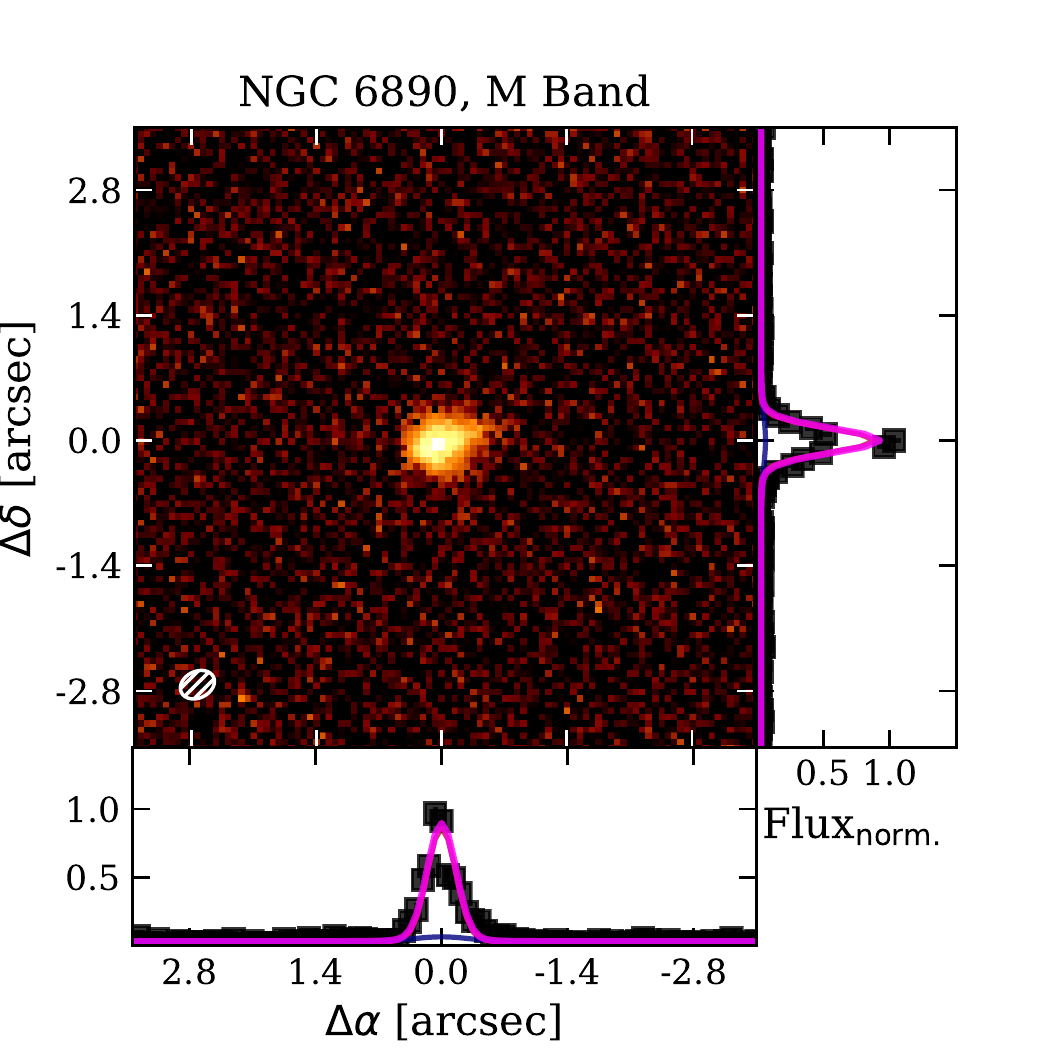}}
\subfloat{\includegraphics[width=0.25\hsize]{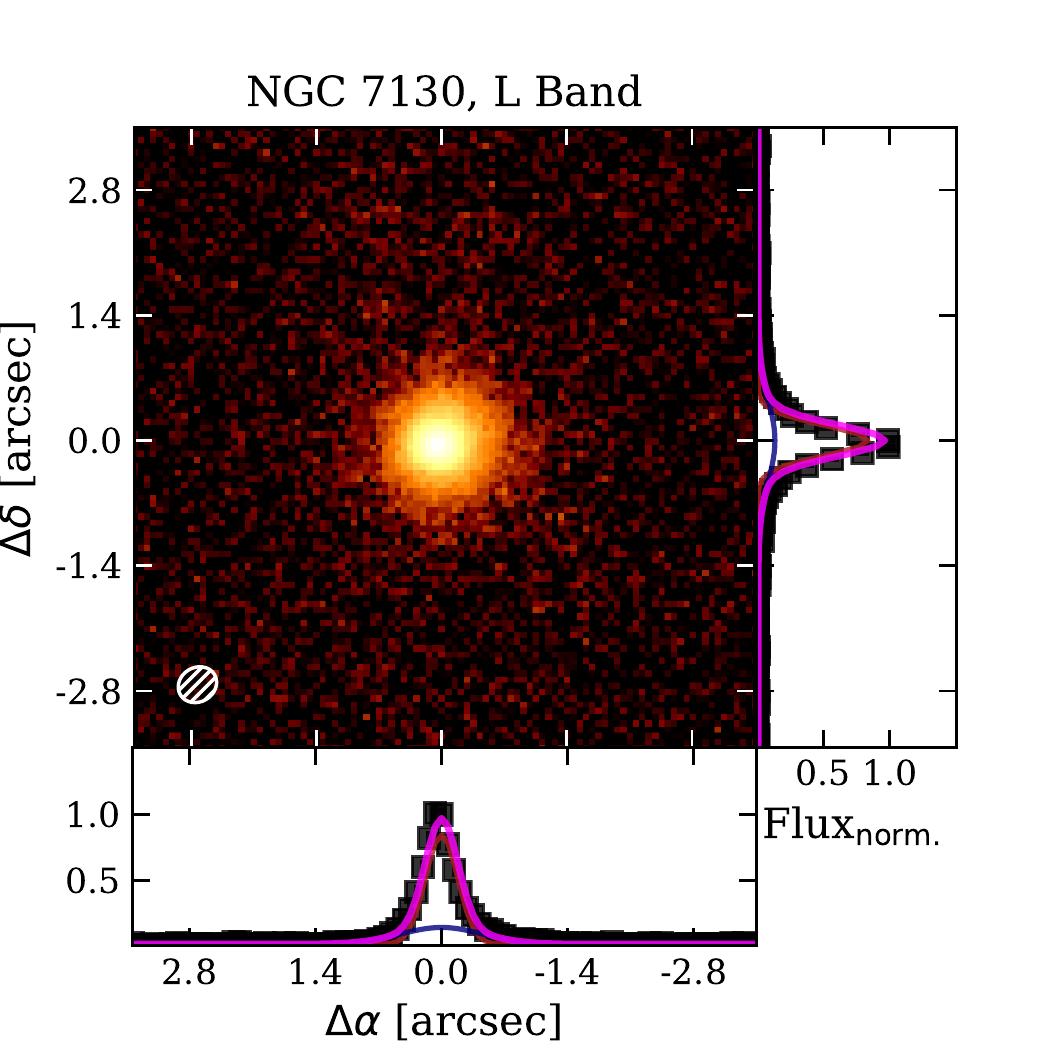}} \\
\subfloat{\includegraphics[width=0.25\hsize]{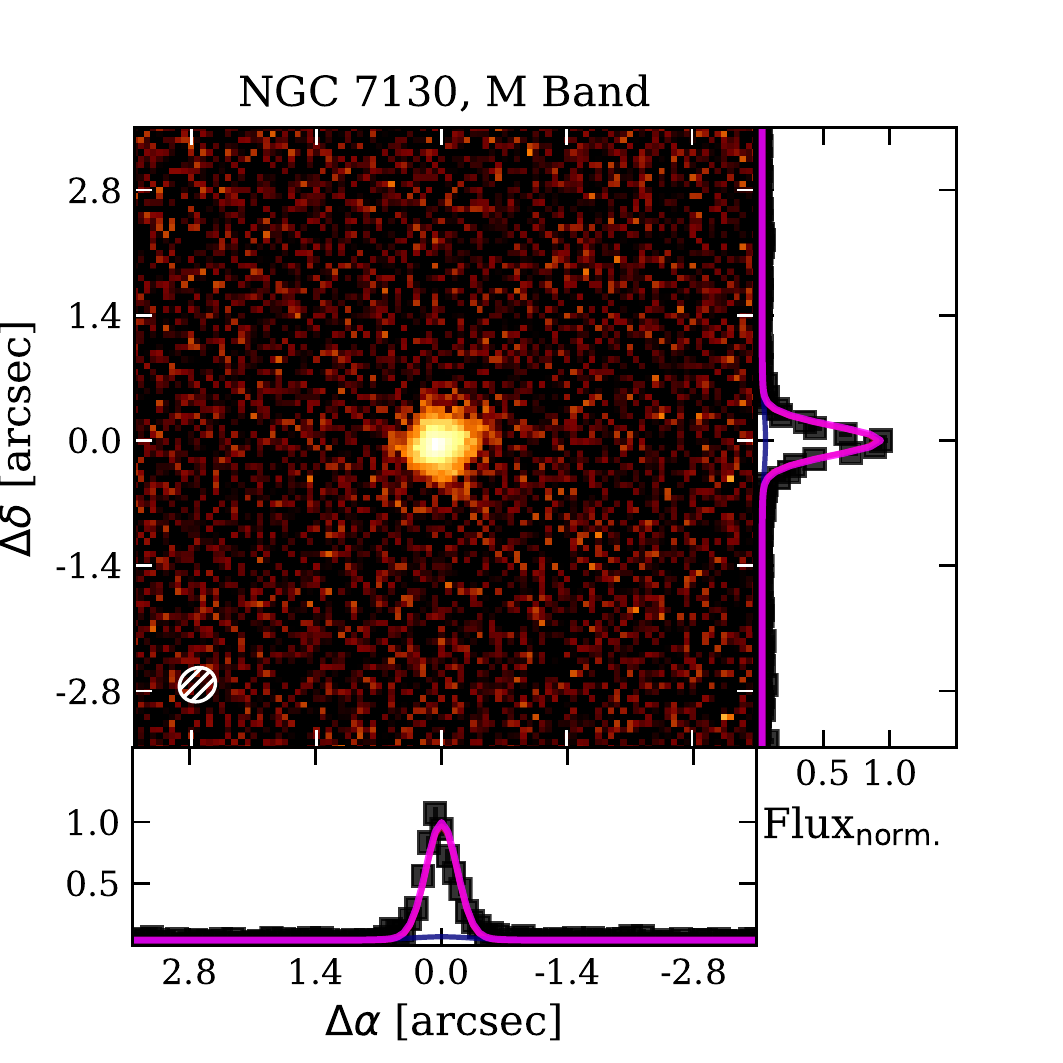}}
\subfloat{\includegraphics[width=0.25\hsize]{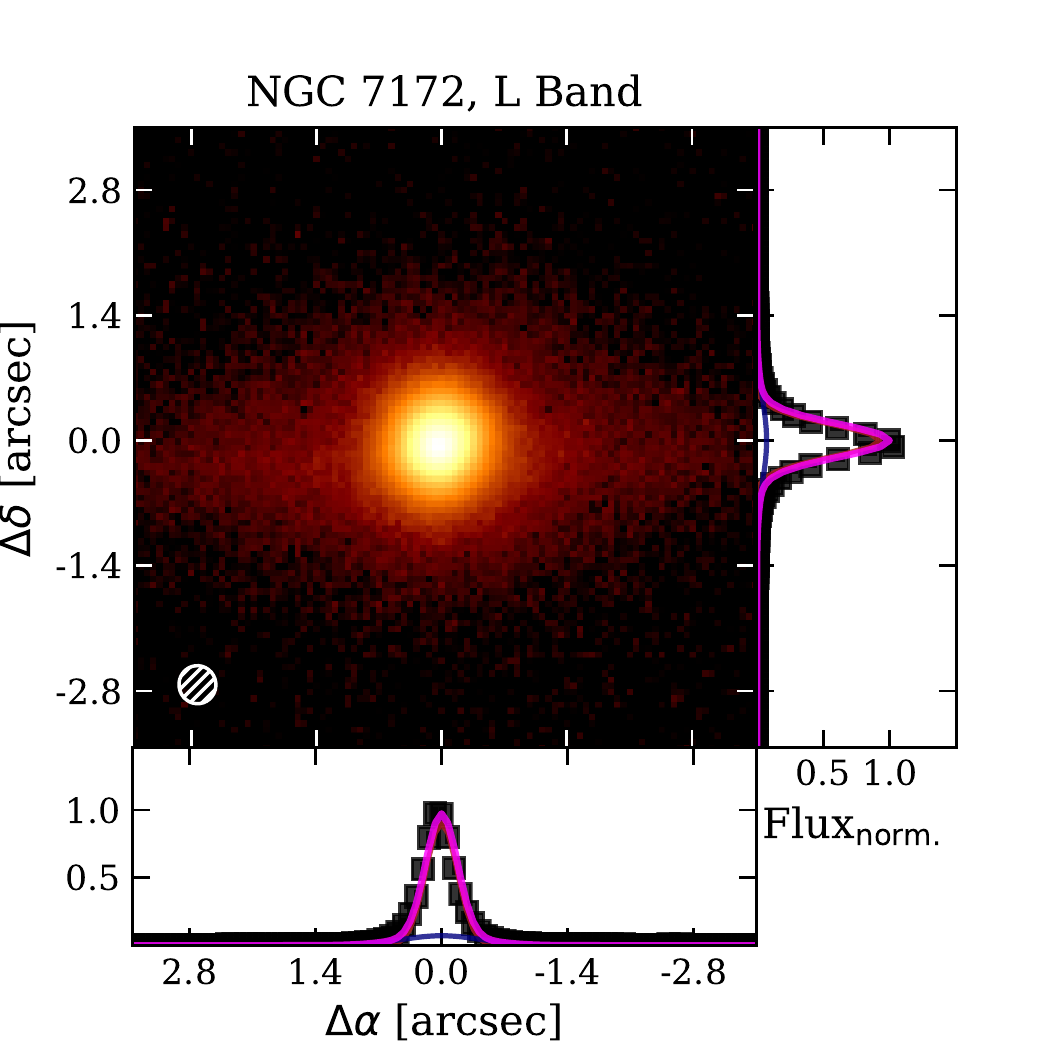}} 
\subfloat{\includegraphics[width=0.25\hsize]{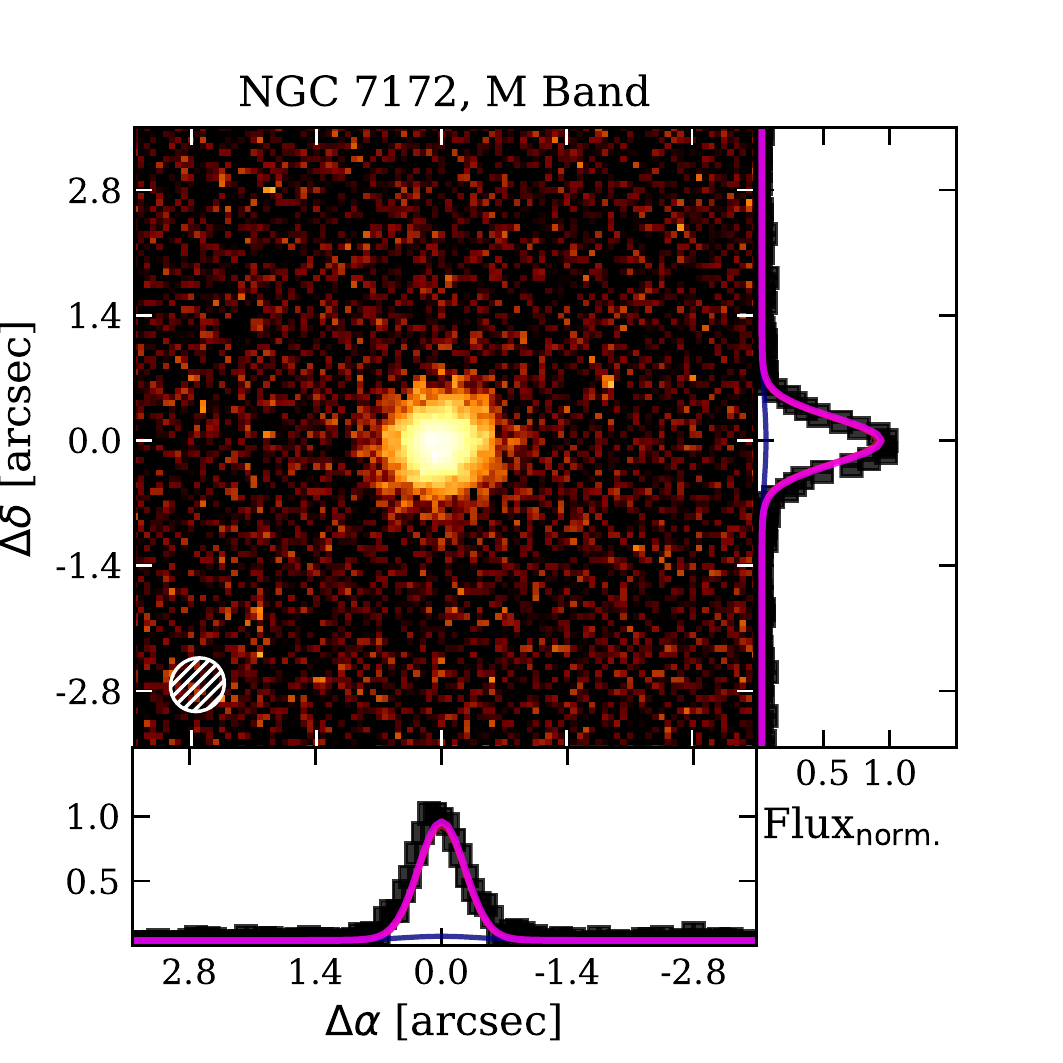}}
\subfloat{\includegraphics[width=0.25\hsize]{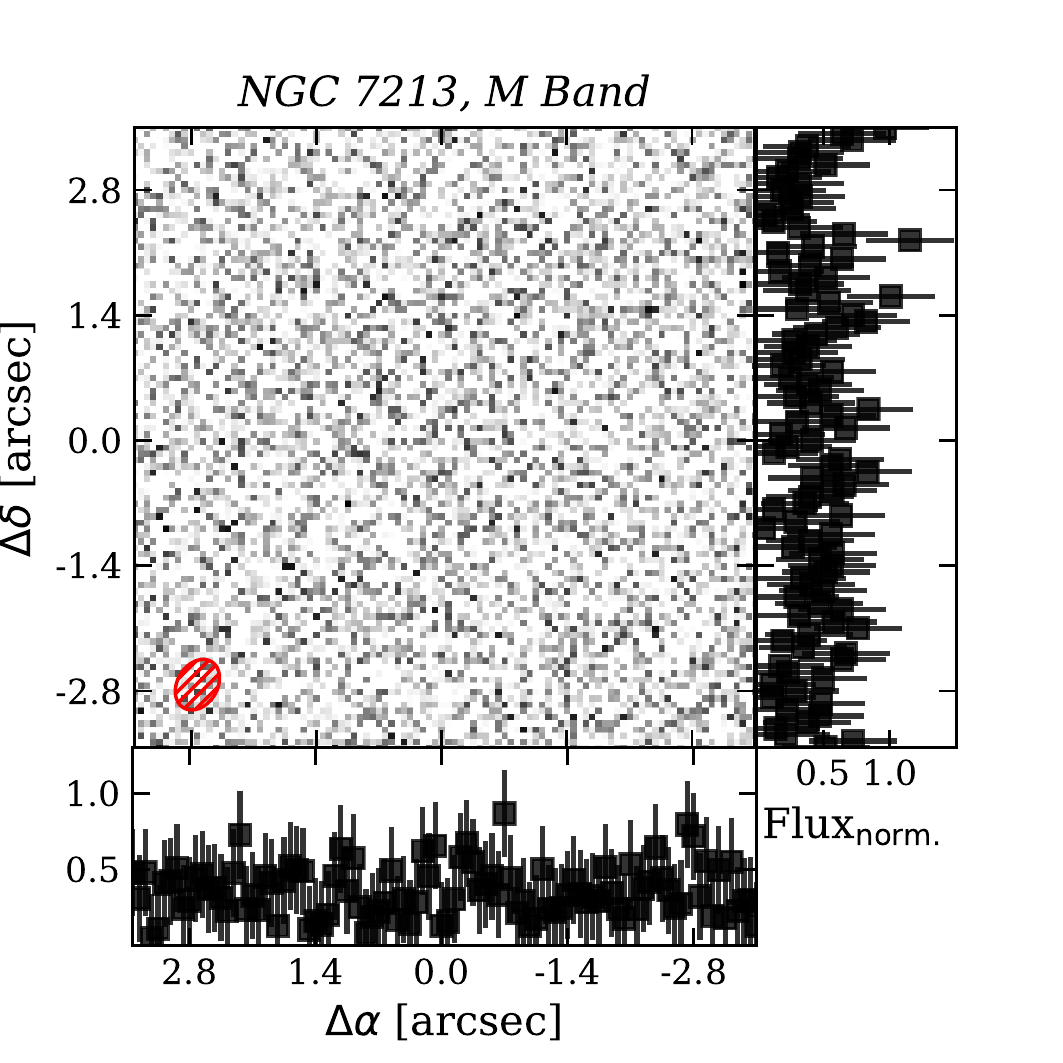}} \\
\subfloat{\includegraphics[width=0.25\hsize]{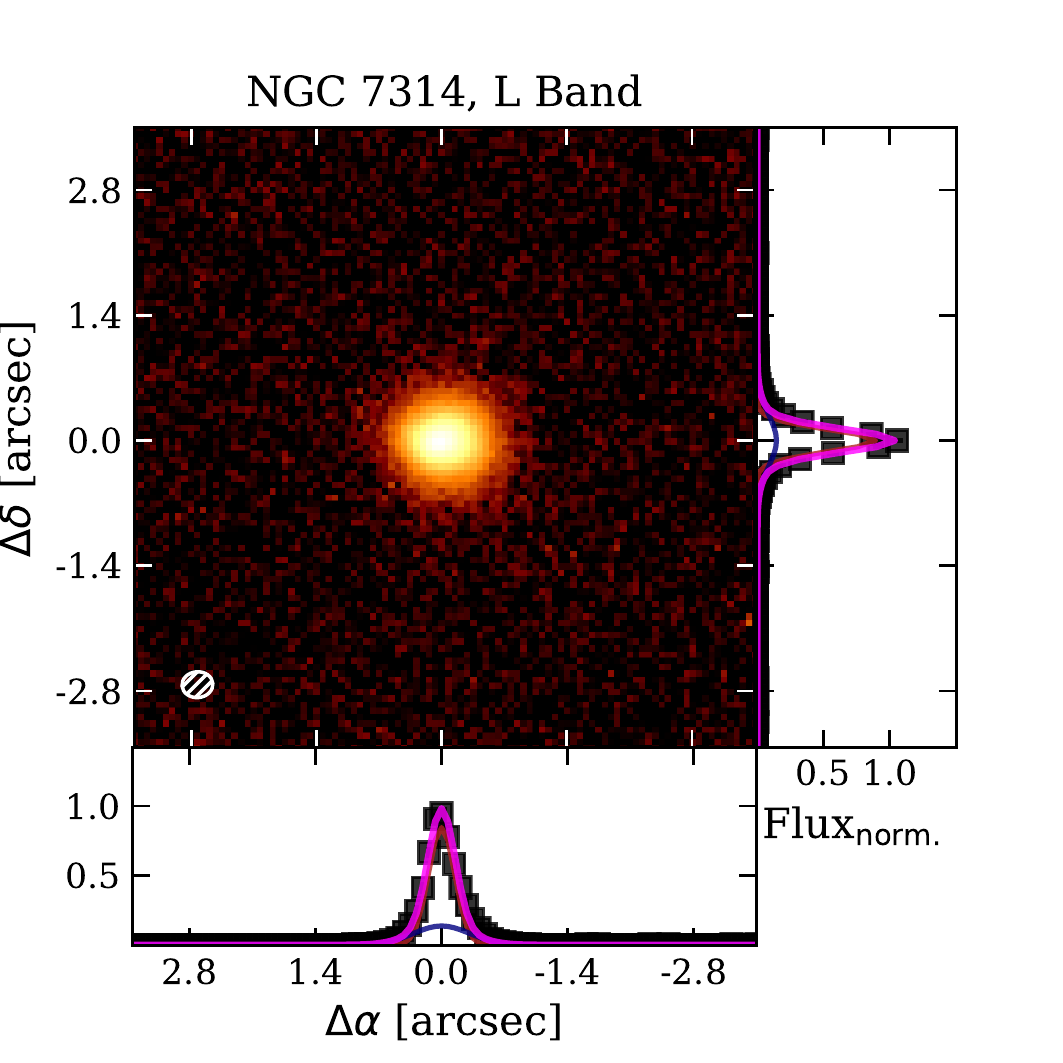}}
\subfloat{\includegraphics[width=0.25\hsize]{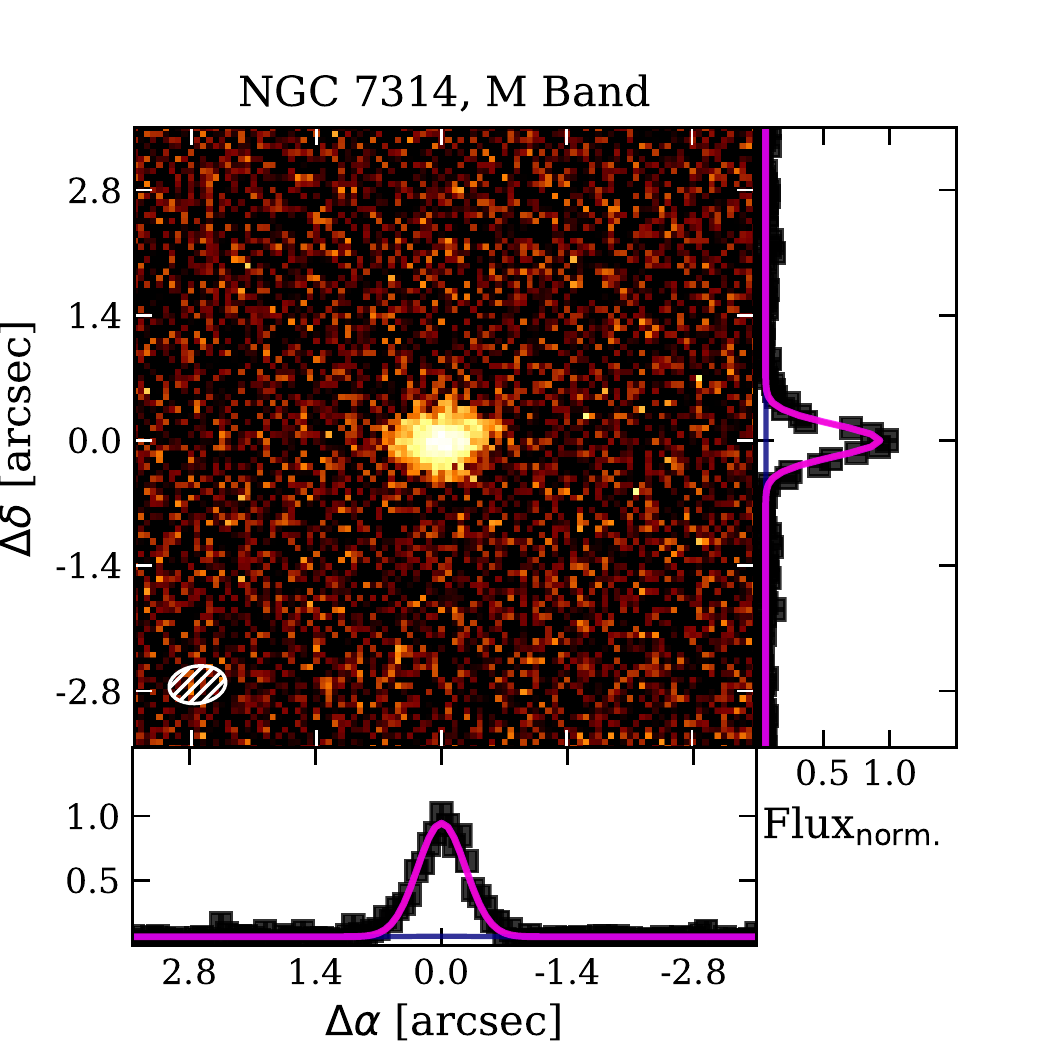}} 
\subfloat{\includegraphics[width=0.25\hsize]{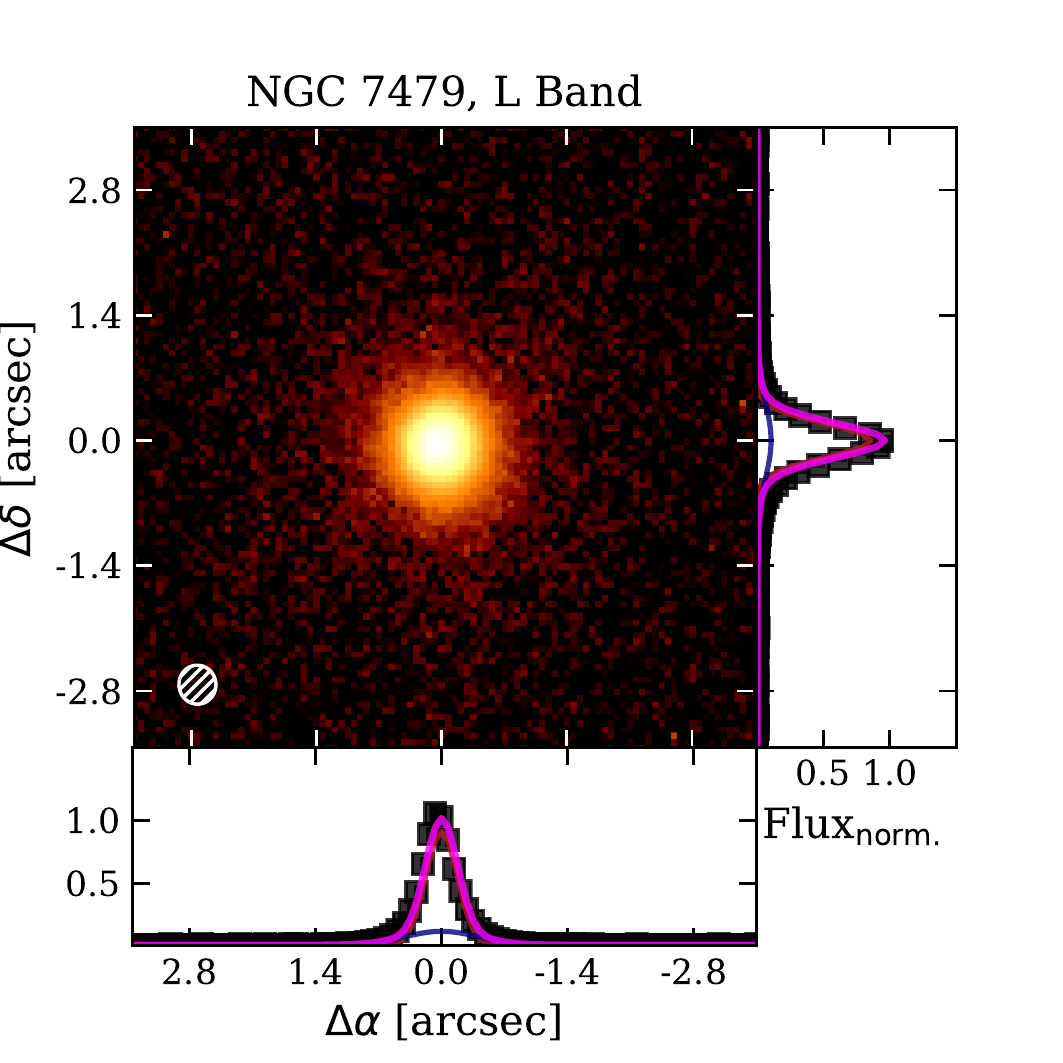}}
\subfloat{\includegraphics[width=0.25\hsize]{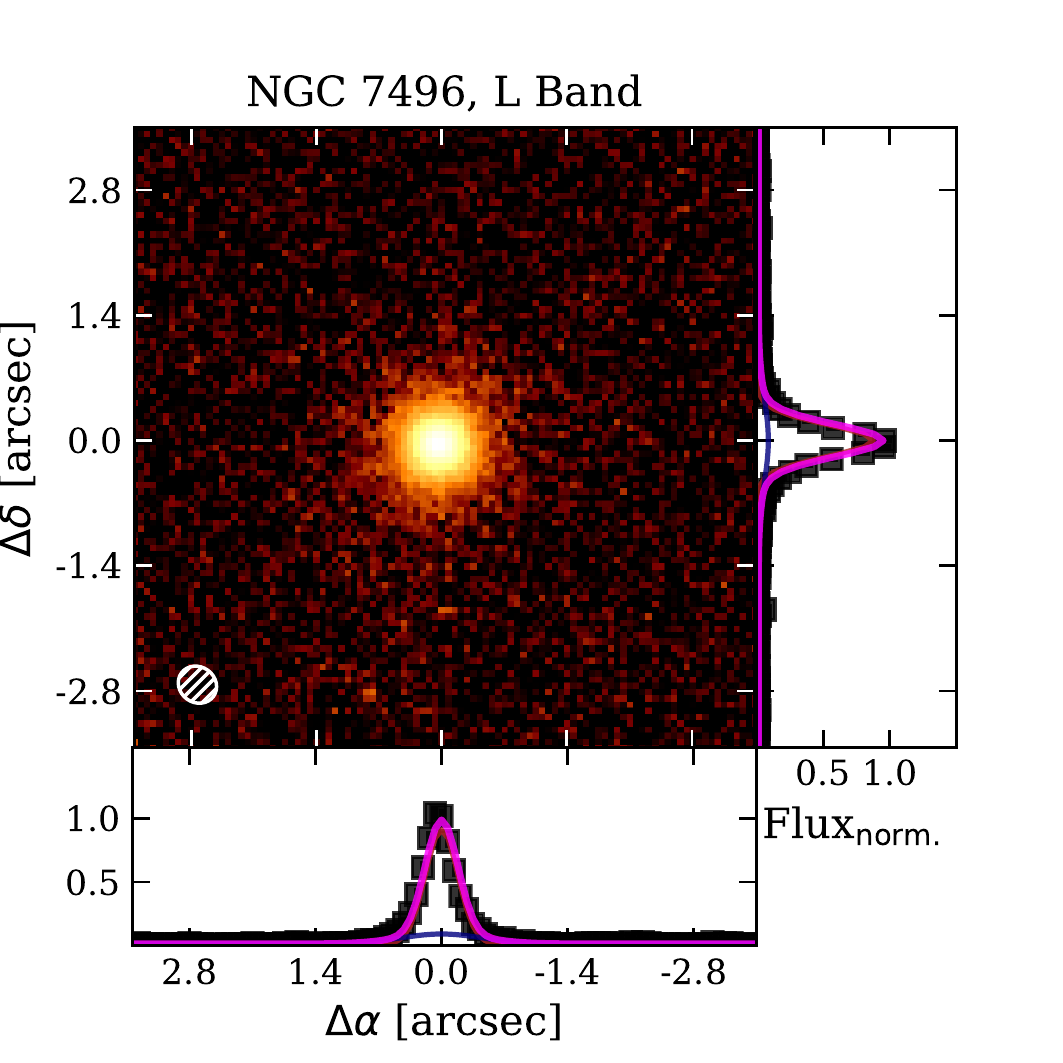}} \\
\subfloat{\includegraphics[width=0.25\hsize]{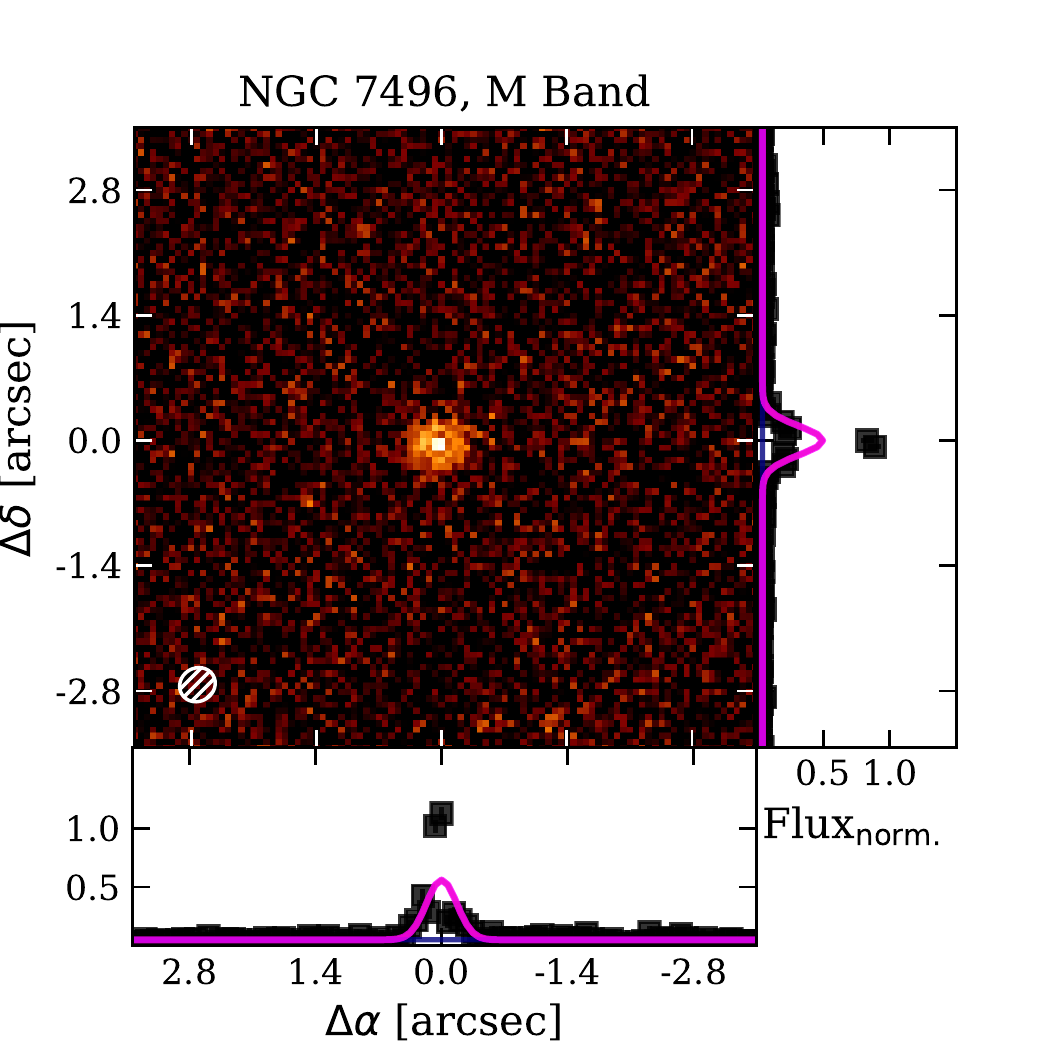}}
\subfloat{\includegraphics[width=0.25\hsize]{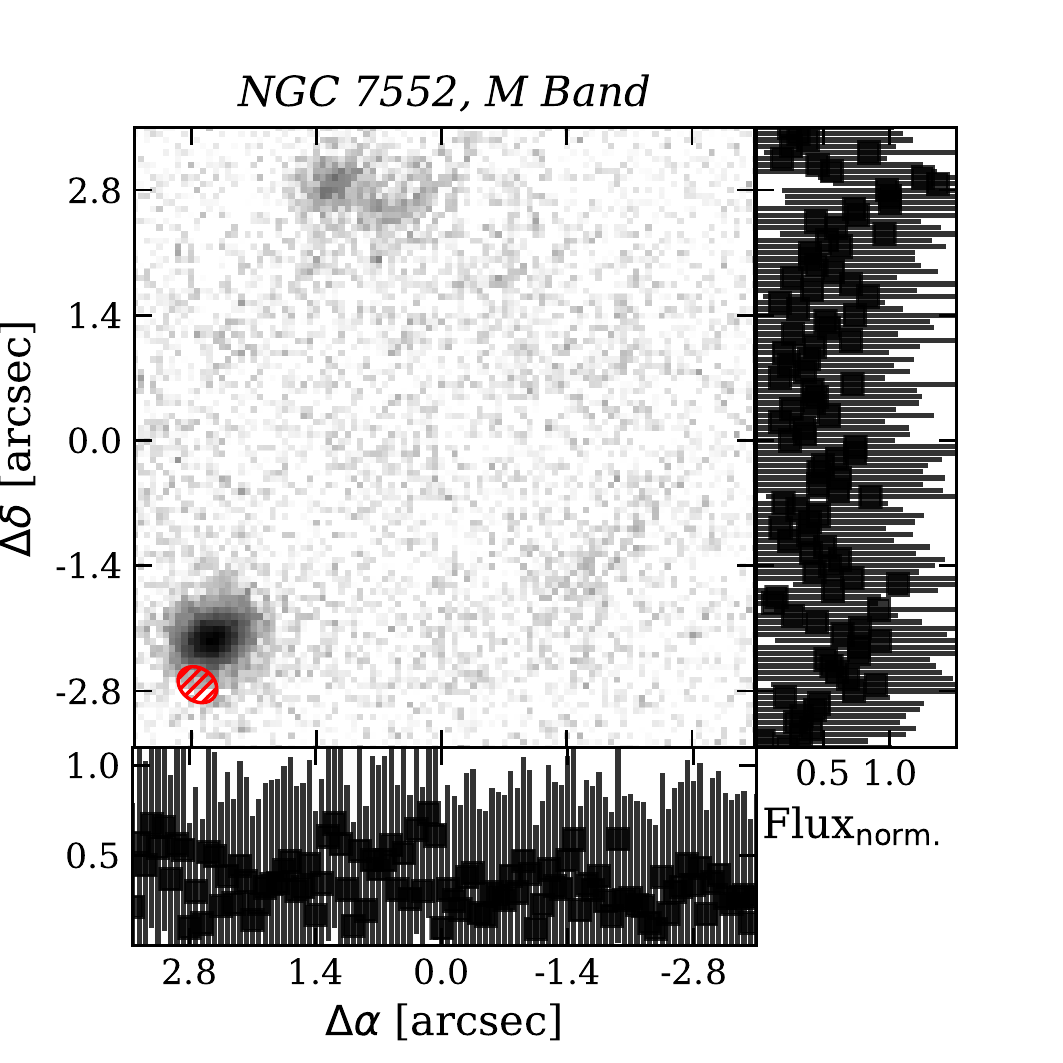}} 
\subfloat{\includegraphics[width=0.25\hsize]{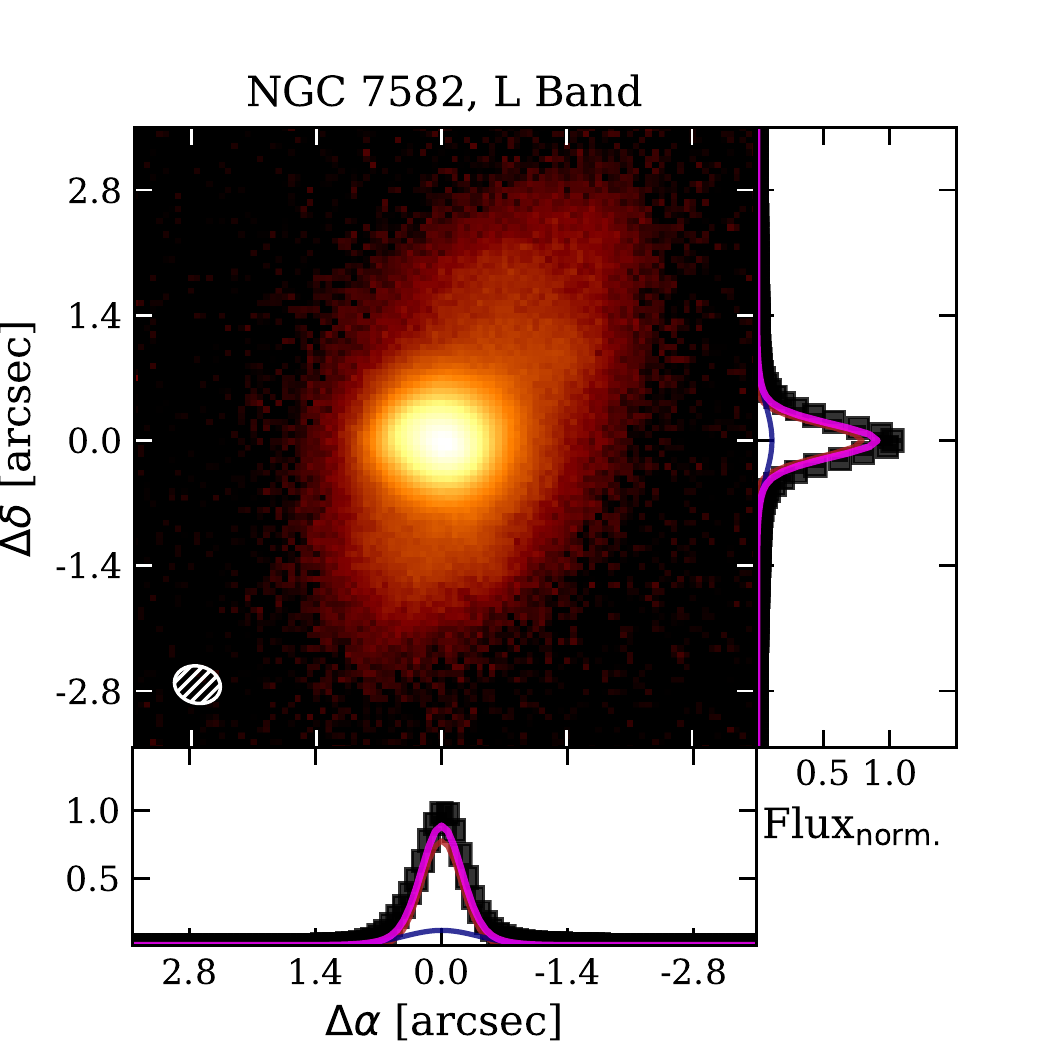}}
\subfloat{\includegraphics[width=0.25\hsize]{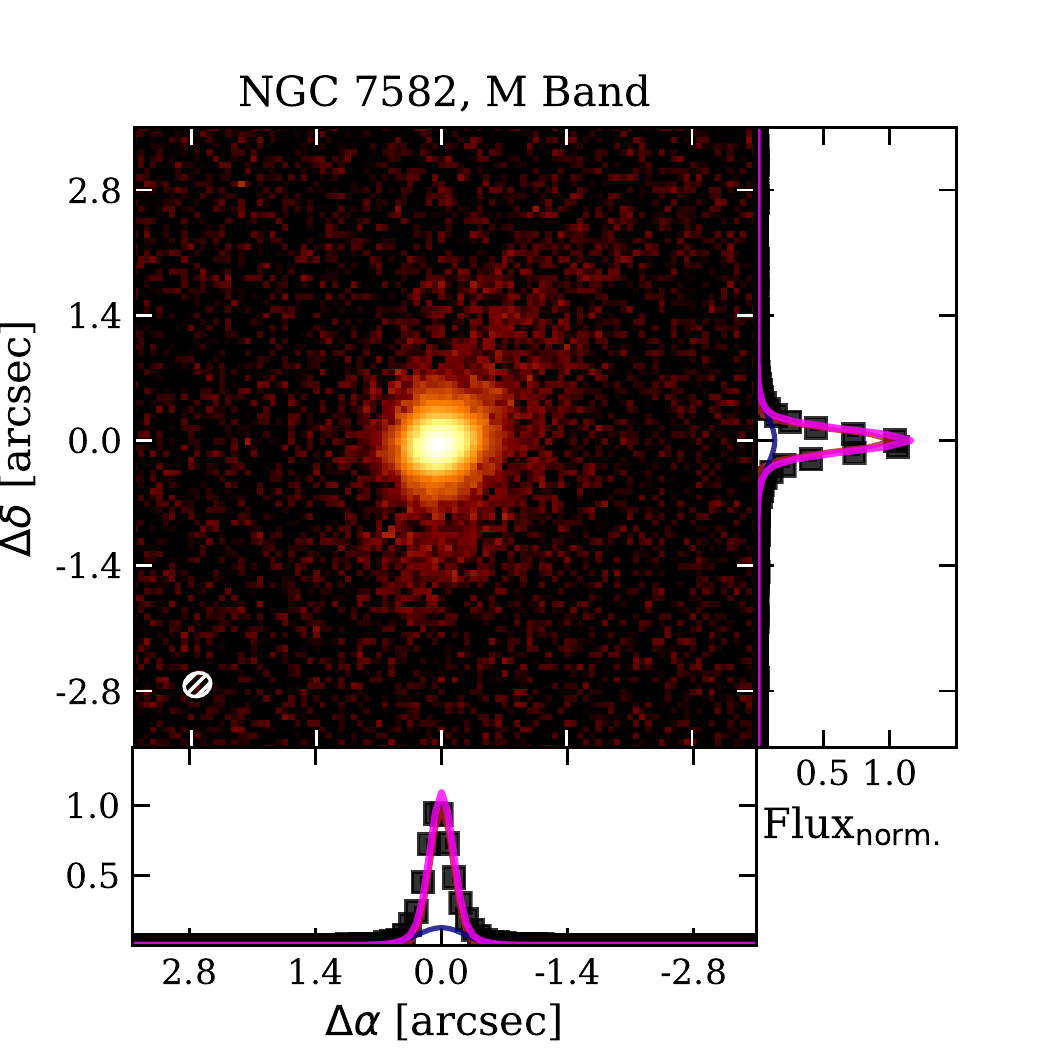}} \\
\caption{ As Fig \ref{fig:cutouts_one} but for all sources.}
\end{figure*}
\begin{figure*}
\subfloat{\includegraphics[width=0.25\hsize]{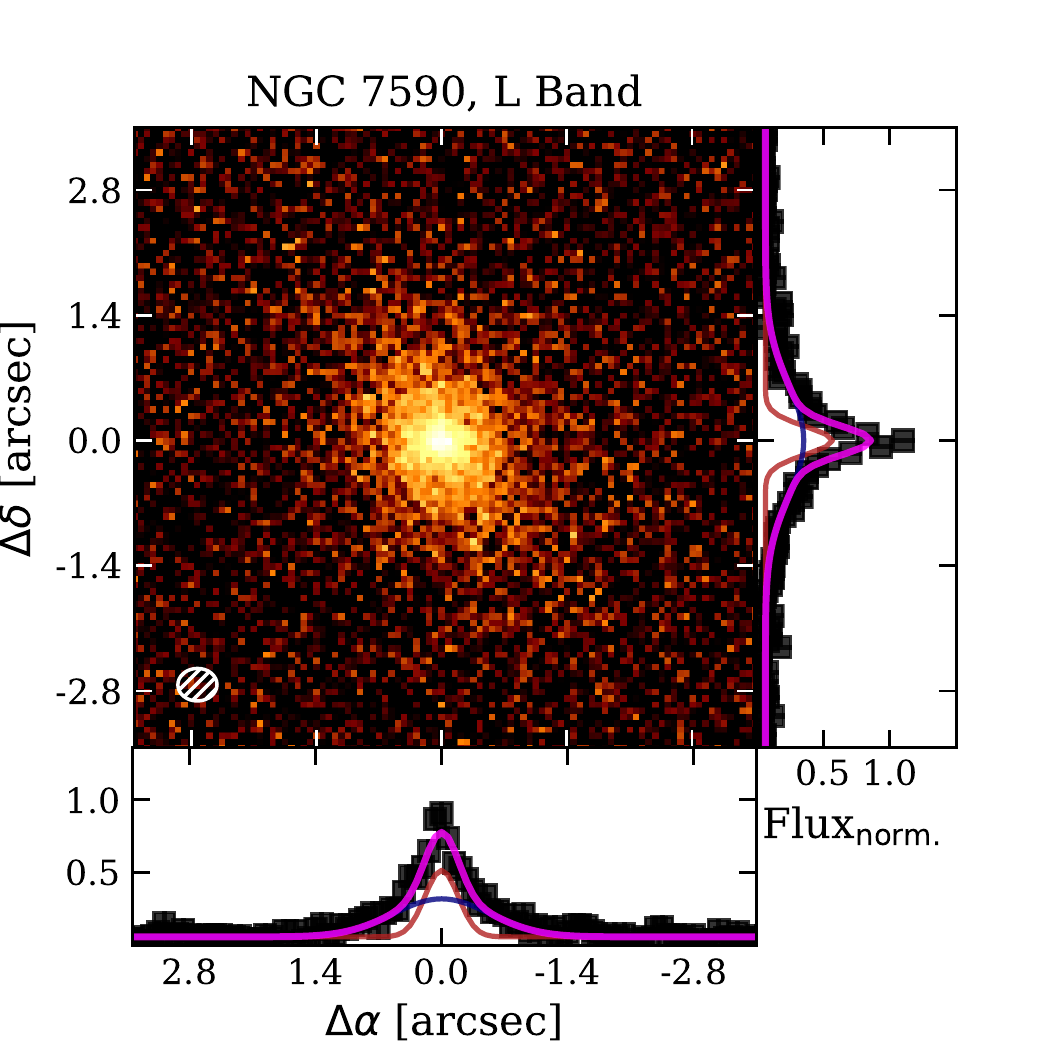}}
\subfloat{\includegraphics[width=0.25\hsize]{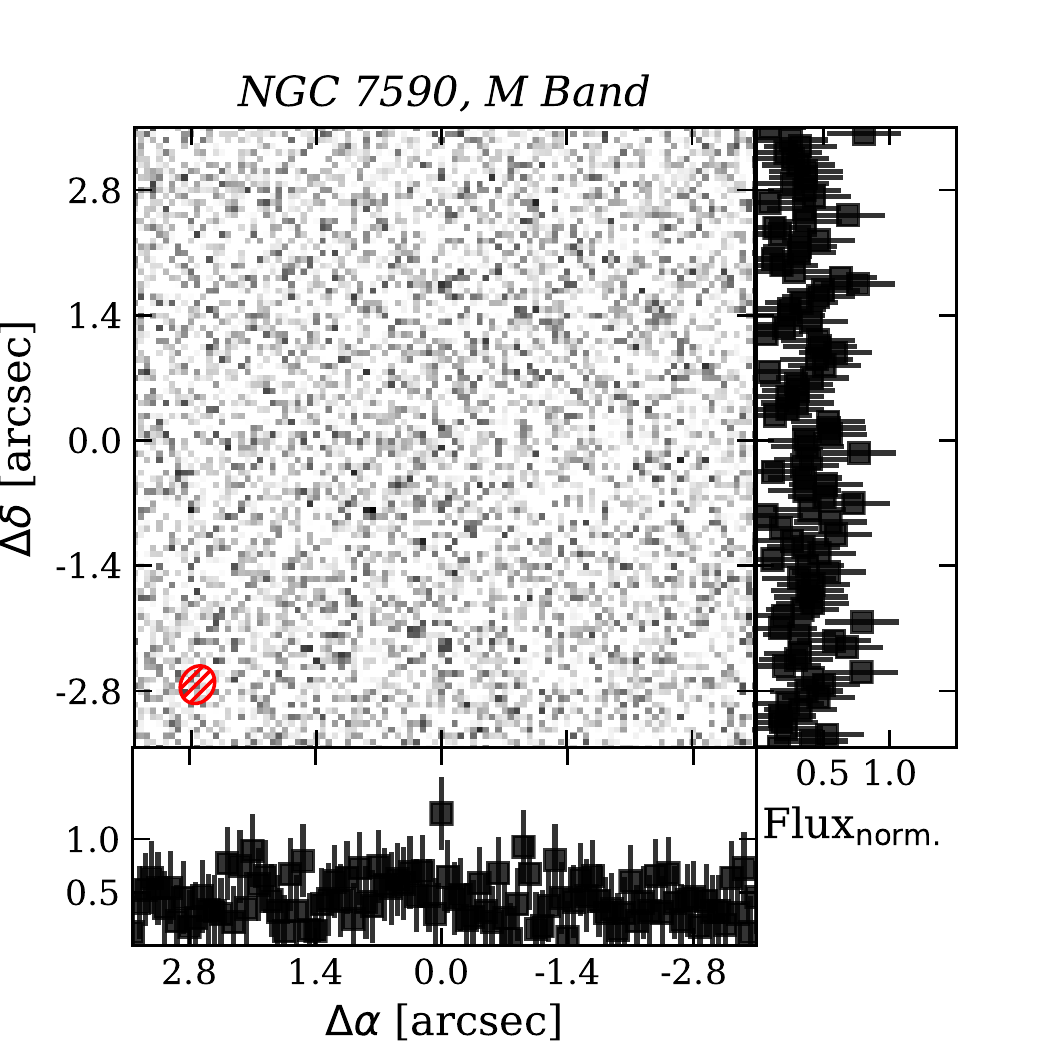}} 
\subfloat{\includegraphics[width=0.25\hsize]{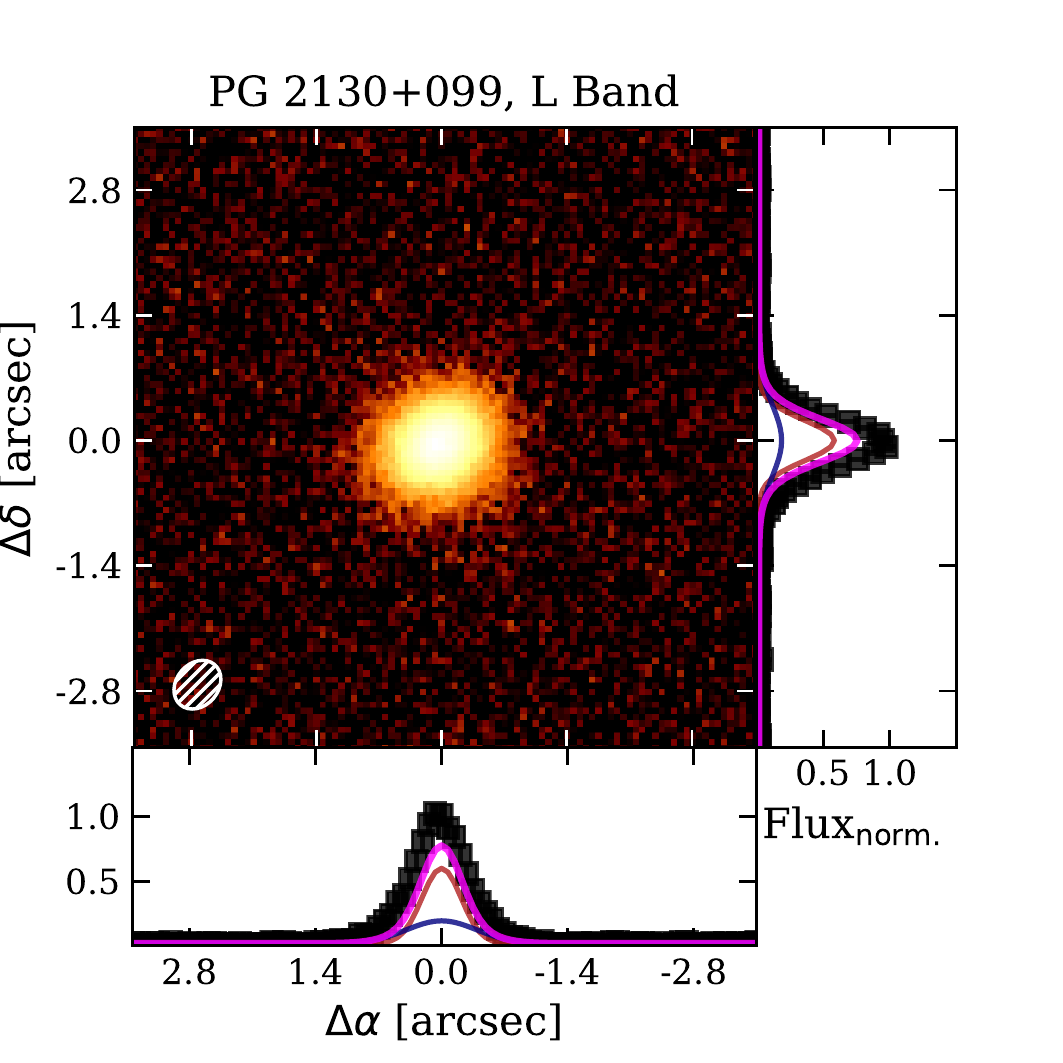}}
\subfloat{\includegraphics[width=0.25\hsize]{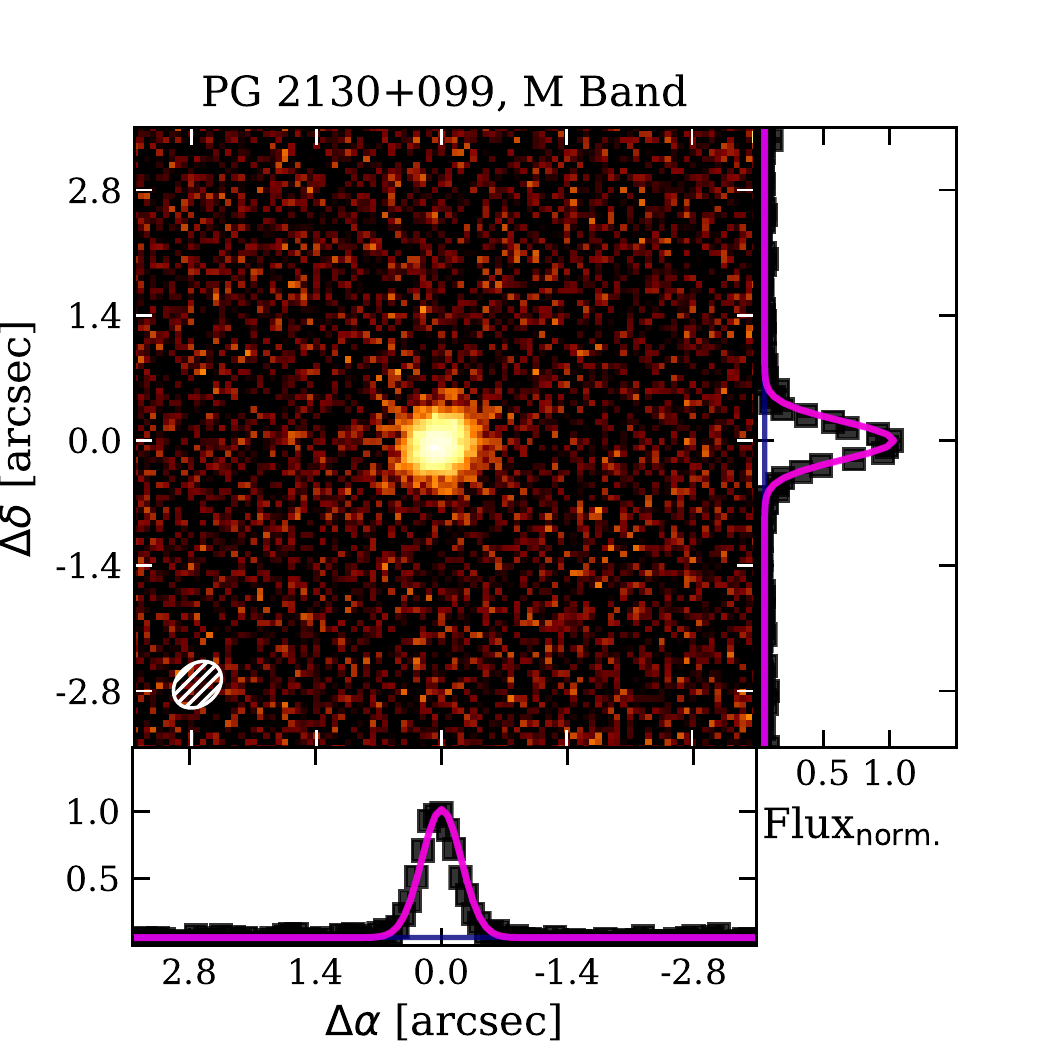}}\\
\subfloat{\includegraphics[width=0.25\hsize]{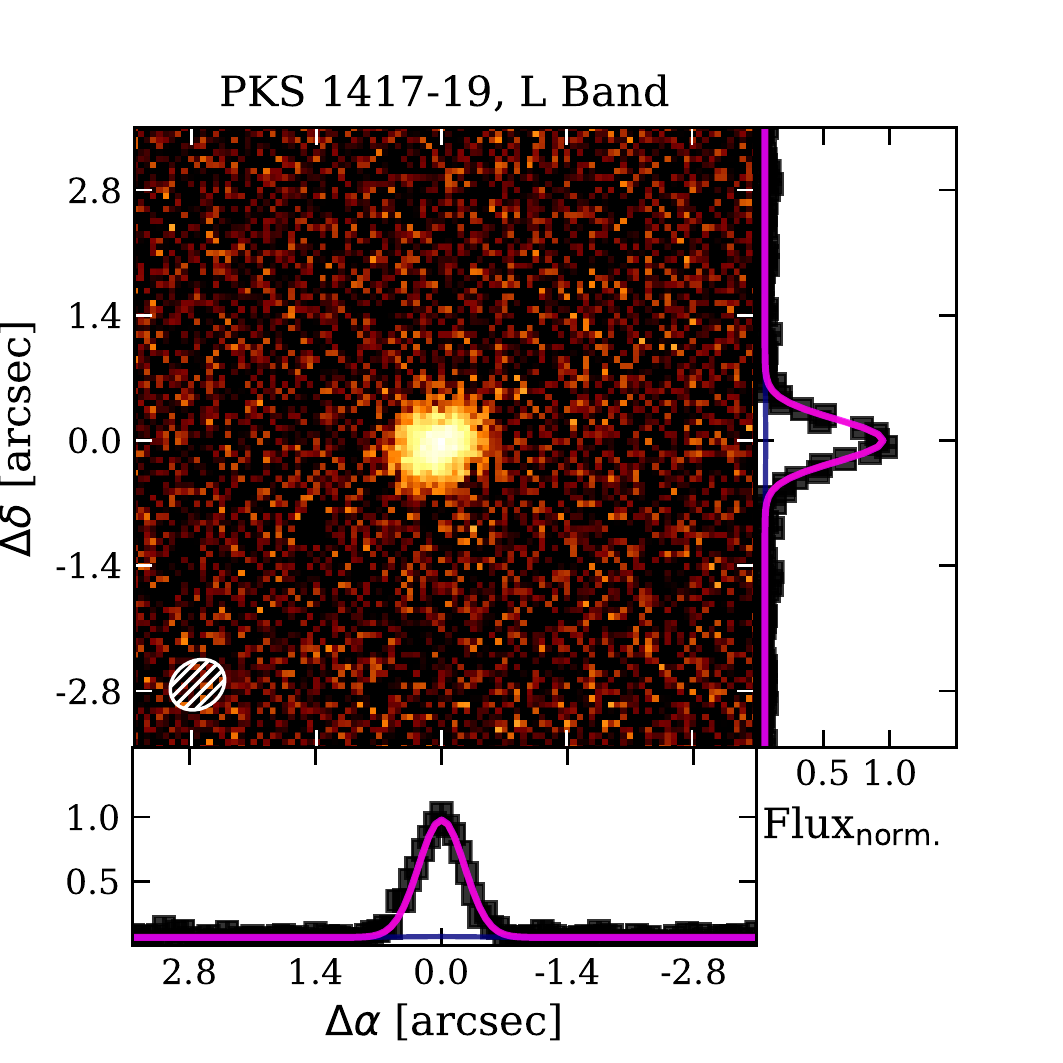}}
\subfloat{\includegraphics[width=0.25\hsize]{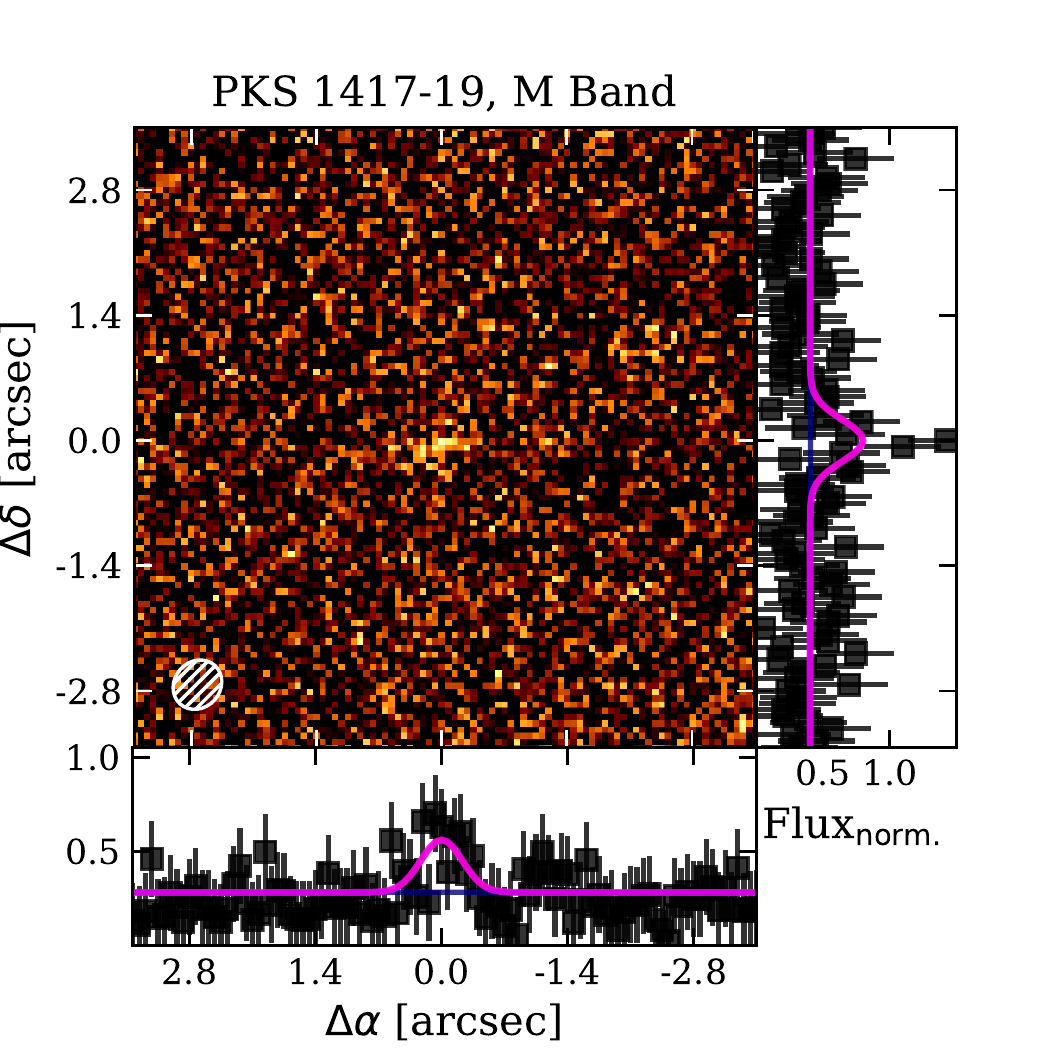}} 
\subfloat{\includegraphics[width=0.25\hsize]{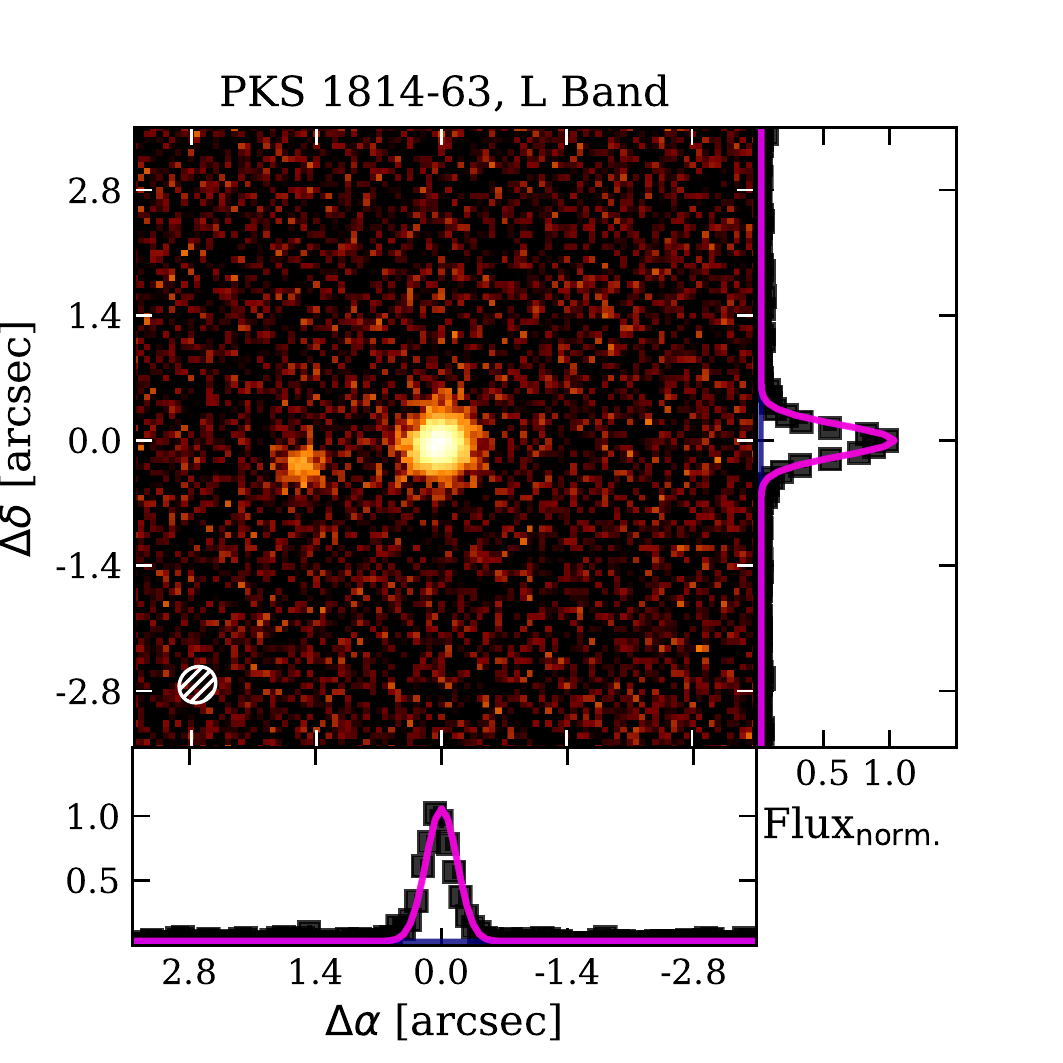}}
\subfloat{\includegraphics[width=0.25\hsize]{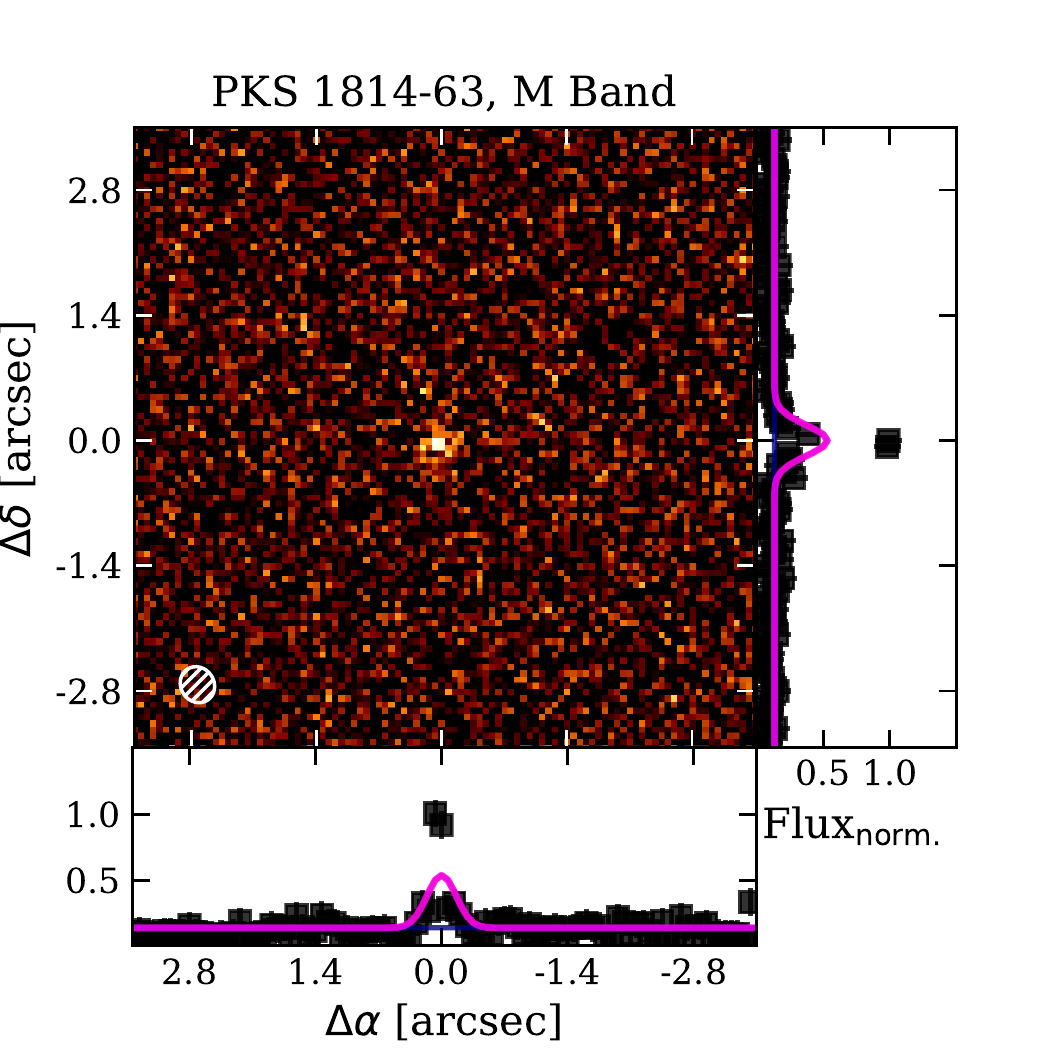}}\\
\subfloat{\includegraphics[width=0.25\hsize]{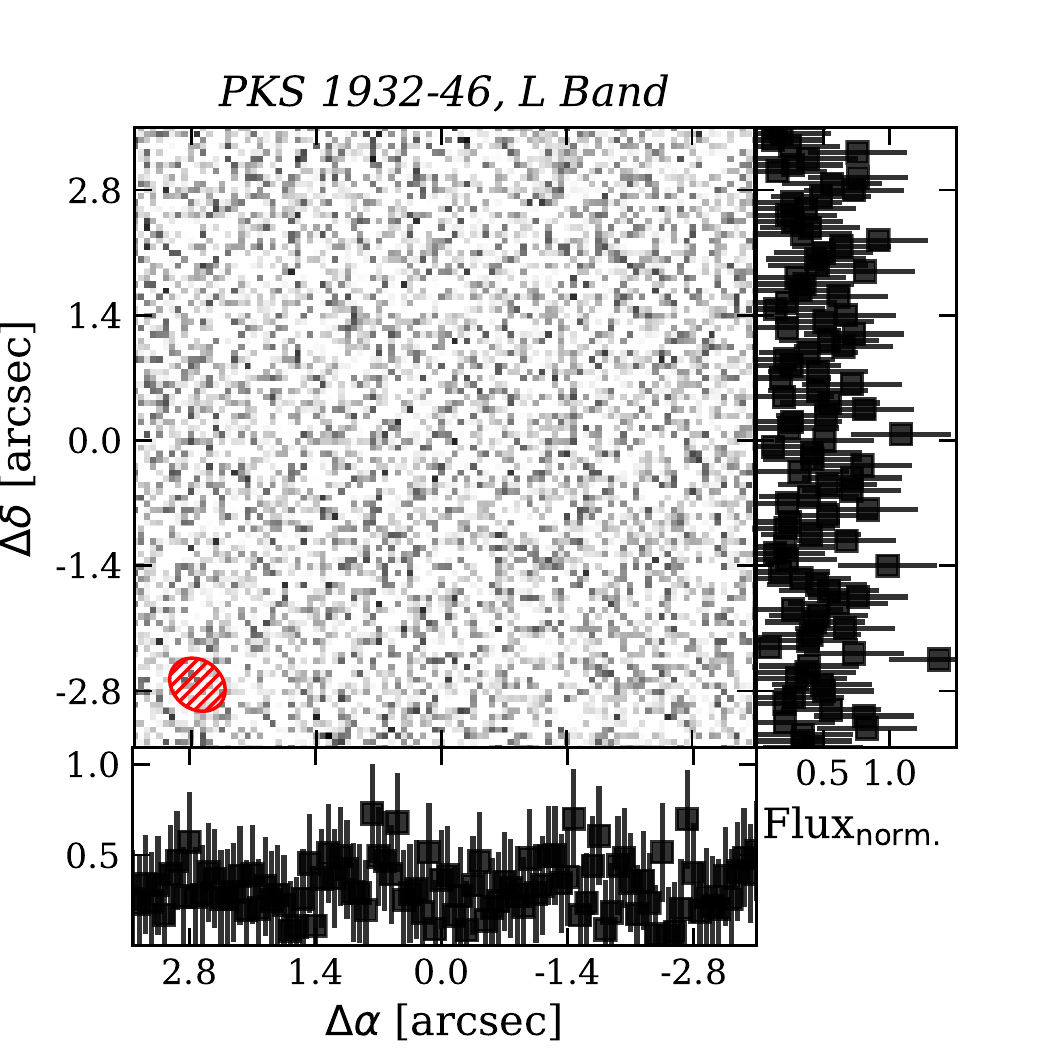}}
\subfloat{\includegraphics[width=0.25\hsize]{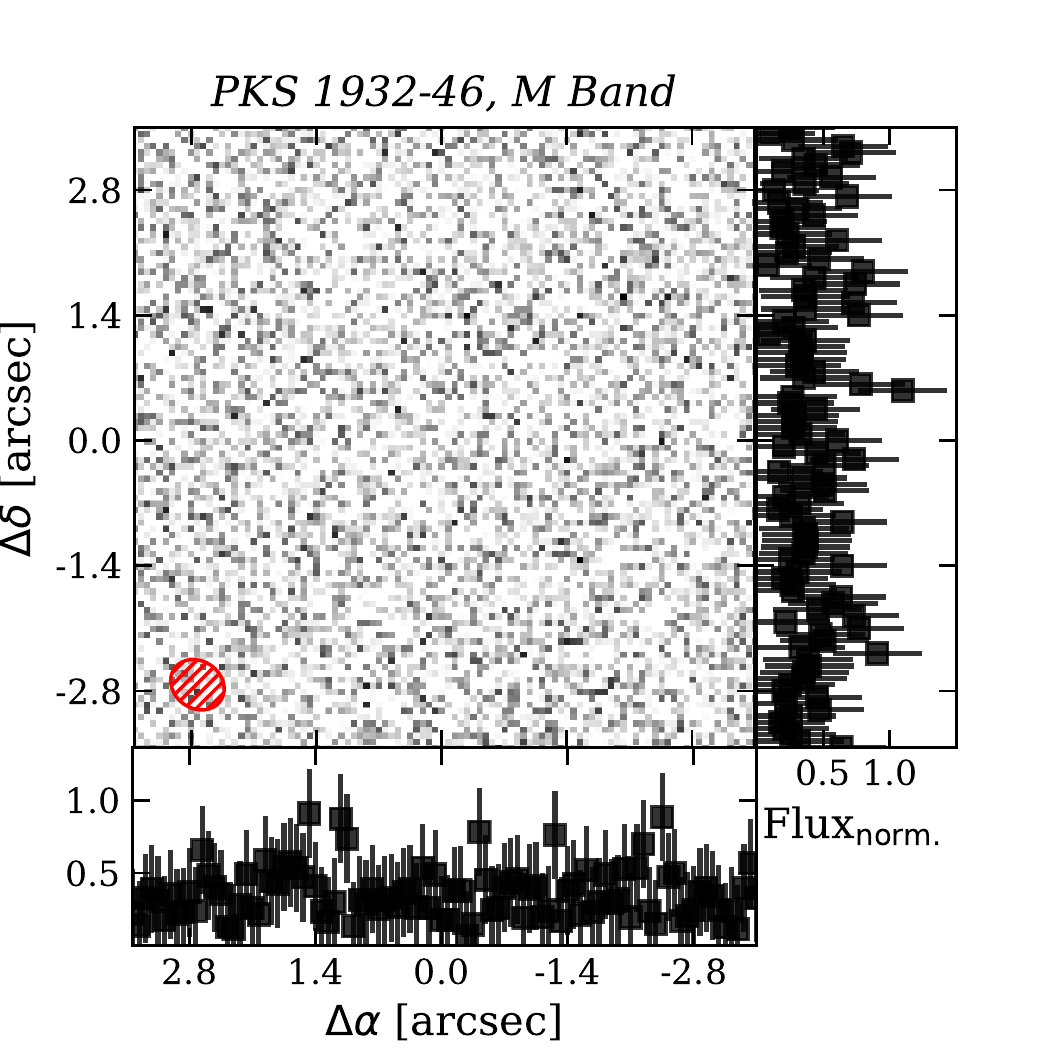}} 
\subfloat{\includegraphics[width=0.25\hsize]{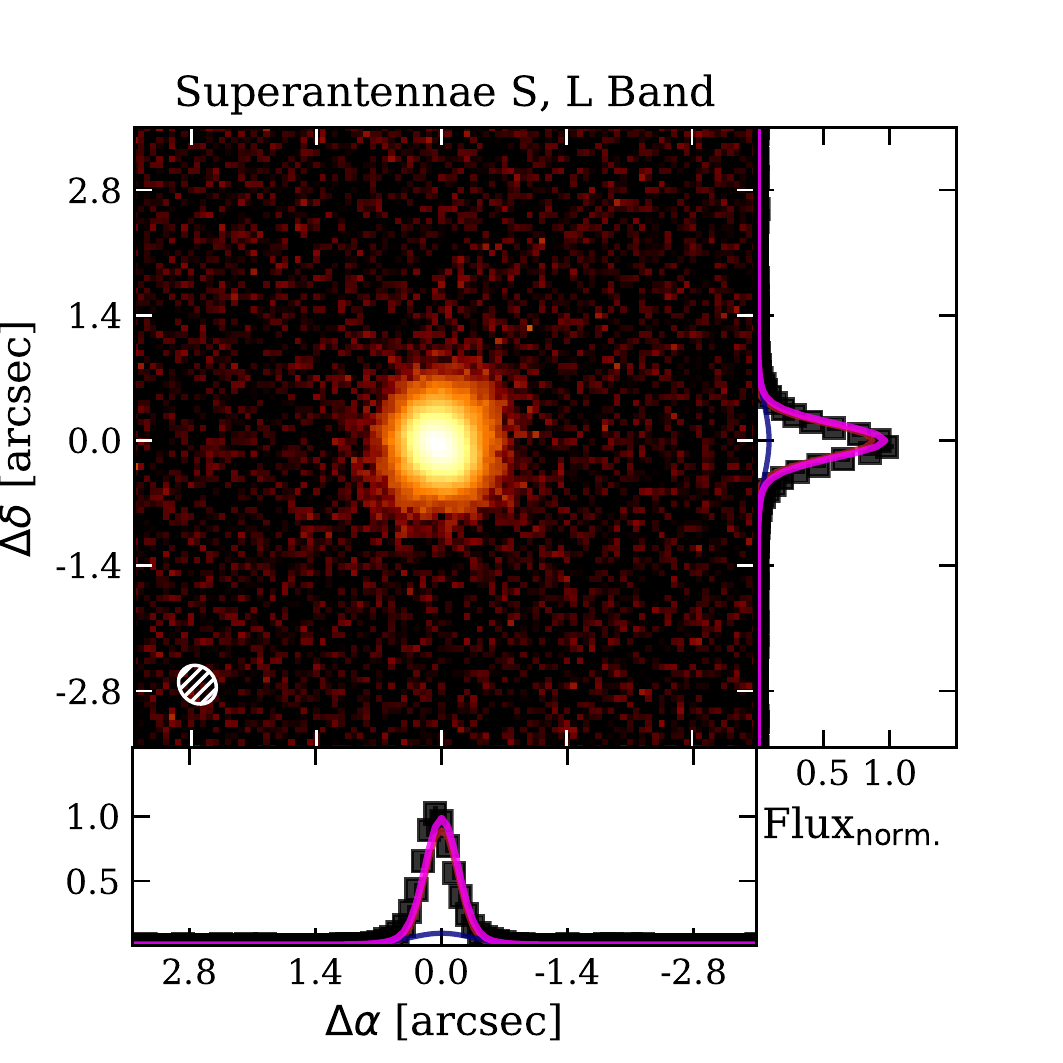}}
\subfloat{\includegraphics[width=0.25\hsize]{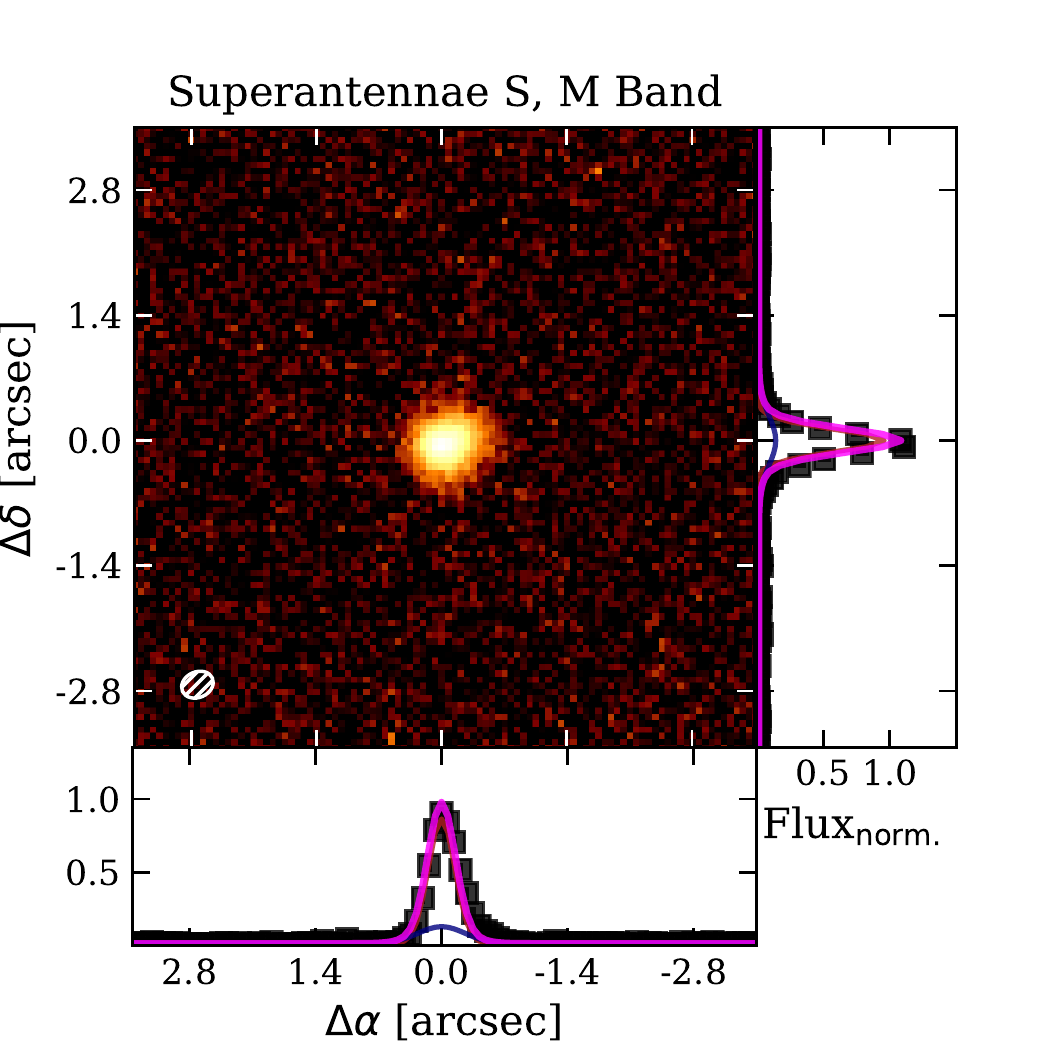}}\\
\subfloat{\includegraphics[width=0.25\hsize]{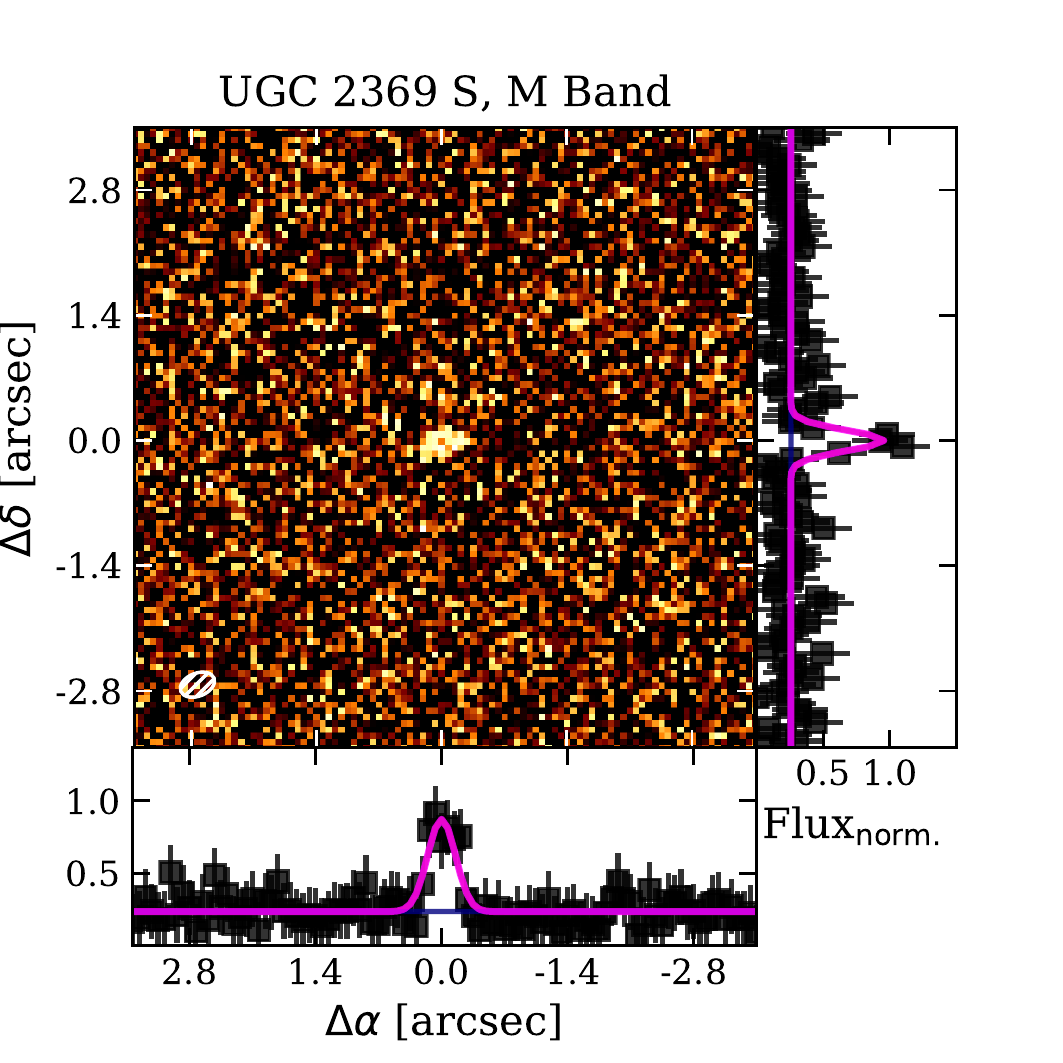}}
\subfloat{\includegraphics[width=0.25\hsize]{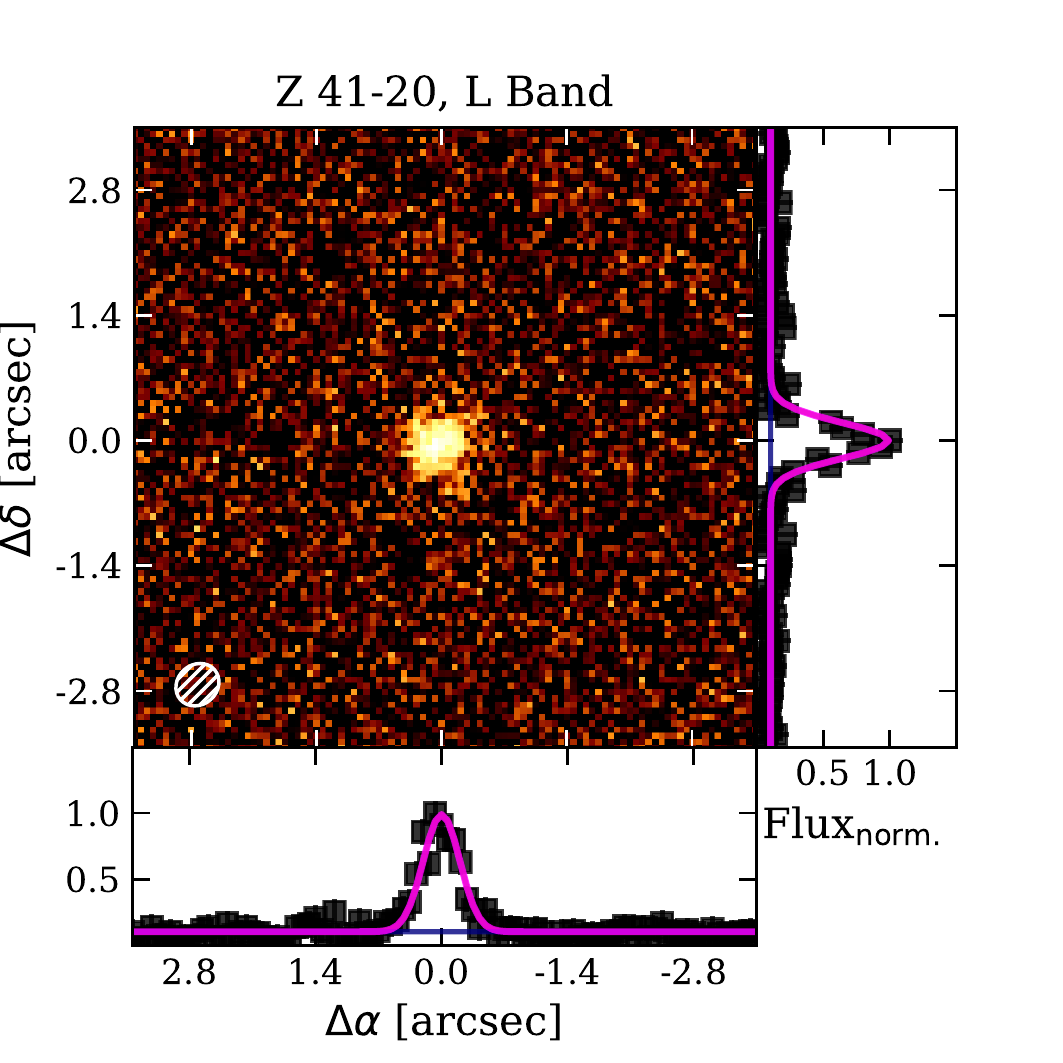}} 
\subfloat{\includegraphics[width=0.25\hsize]{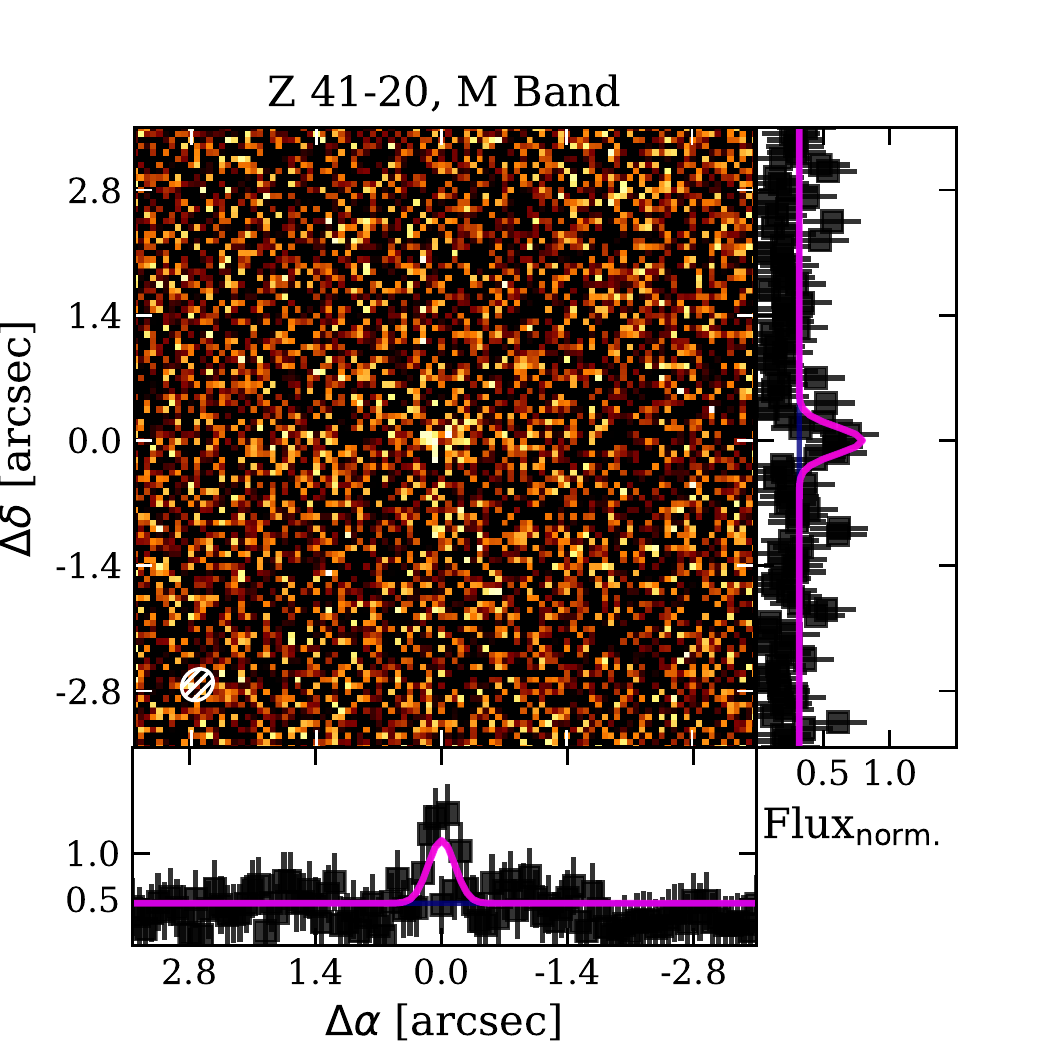}}\\
\caption{ As Fig \ref{fig:cutouts_one} but for all sources.}
\end{figure*}

\end{document}
